# Supplementary material for: The diversity of Type II supernova versus the similarity in their progenitors
Source: arXiv:1603.08953 ancillary file (2016-05-09)
Supplement: Supplementary file 1 [file supplementarytable_final.pdf]

**Table 2:** Sample of SNe type II

| SN | Distance modulus | REF* ($\mu$) | Explosion epoch | m REF* (explosion) | E(B-V) (host) | REF* (E(B-V) host) | $E(B-V)^{x}$ M.W. | Host galaxy |
|---|---|---|---|---|---|---|---|---|
| 2013ai | 32.20 0.15 | a | 2456348.00 5.0 | w | 0.15 0.08 | w | 0.08 | NGC2207 |
| 2013bu | 30.79 0.08 | b | 2456399.80 4.5 | w | 0.00 0.00 | w | 0.08 | NGC7331 |
| 2013fs | 33.45 0.15 | a | 2456571.12 0.5 | ll | 0.00 0.00 | w | 0.04 | NGC7610 |
| lsq13dpa | 35.08 0.15 | a | 2456642.70 2.0 | w | 0.00 0.00 | w | 0.04 | LCSBS1492O |
| 2014cy | 31.87 0.15 | a | 2456900.00 1.0 | w | 0.00 0.00 | w | 0.05 | NGC7742 |
| 2014dw | 32.46 0.15 | a | 2456958.00 10.0 | w | 0.11 0.06 | w | 0.11 | NGC3568 |
| lsq14gv | 35.15 0.15 | a | 2456674.80 2.0 | w | 0.00 0.00 | w | 0.06 | 2MASX J10541092-1501228 |
| ASASSN-14dq | 33.26 0.15 | a | 2456841.50 5.5 | w | 0.00 0.00 | w | 0.07 | UGC11860 |
| ASASSN-14gm | 31.74 0.15 | a | 2456901.00 1.5 | w | 0.00 0.00 | w | 0.10 | NGC0337 |
| ASASSN-14kg | 33.83 0.15 | a | 2456970.00 3.0 | w | 0.25 0.12 | w | 0.04 | CGCG521-075 |
| ASASSN-14ha | 29.53 0.50 | a | 2456910.50 1.5 | w | 0.00 0.00 | w | 0.01 | NGC1566 |
| 2015W | 33.74 0.15 | a | 2457025.00 10.0 | w | 0.00 0.00 | w | 0.15 | UGC03617 |
| 2013ab | 31.90 0.08 | d | 2456340.00 1.0 | d | 0.02 0.07 | d | 0.02 | 1430+101 |
| 2013by | 30.81 0.15 | a | 2456404.00 2.0 | x | 0.00 0.00 | x | 0.23 | ESO138-G010 |
| 2013ej | 29.79 0.20 | c | 2456497.00 1.0 | y | 0.00 0.00 | y | 0.06 | MESSIER074 |
| 2014G | 31.90 0.15 | a | 2456668.35 1.0 | w | 0.20 0.00 | kk | 0.01 | NGC3448 |
| 1986L | 31.72 0.20 | e | 2446708.50 6.0 | m | 0.00 0.02 | m | 0.03 | NGC1559 |
| 1979C | 31.01 0.09 | f | 2443970.00 15.0 | s | 0.16 0.05 | gg | 0.02 | NGC4321 |
| 1990E | 31.71 0.27 | g | 2447932.00 5.0 | z | 0.38 0.00 | z | 0.02 | NGC1035 |
| 1991al | 34.28 0.54 | h | 2448444.00 9.0 | m | 0.04 0.02 | m | 0.05 | 2MASXJ19422191-5506275 |
| 1992af | 34.37 0.15 | a | 2448792.00 6.0 | m | 0.00 0.09 | m | 0.05 | ESO340-G038 |
| 1992ba | 31.07 0.30 | i | 2448889.00 8.0 | m | 0.02 0.01 | m | 0.05 | NGC2082 |
| 1993A | 35.68 0.17 | h | 2448996.00 9.0 | m | 0.00 0.00 | m | 0.15 | 2MASXJ07391822-6203095 |
| 1993K | 32.89 0.15 | a | 2449066.00 9.0 | m | 0.12 0.06 | m | 0.06 | NGC2223 |
| 1993S | 35.32 0.14 | h | 2449131.00 4.0 | m | 0.00 0.08 | m | 0.01 | 2MASXJ22522390-4018432 |
| 1999ca | 32.82 0.15 | a | 2451278.00 7.0 | m | 0.08 0.05 | m | 0.10 | NGC3120 |
| 1999cr | 34.56 0.18 | h | 2451248.00 7.0 | m | 0.10 0.05 | m | 0.09 | ESO576-G034 |
| 1999em | 30.34 0.07 | j | 2451475.00 1.0 | i | 0.06 0.02 | m | 0.04 | NGC1637 |
| 1999gi | 30.34 0.14 | i | 2451518.20 3.1 | hh | 0.19 0.09 | hh | 0.01 | NGC3184 |
| 1999br | 31.60 0.43 | i | 2451278.00 3.0 | jj | 0.00 0.01 | m | 0.02 | SDSSJ130039.25+023002.5 |
| 2000dc | 32.93 0.14 | h | 2451762.00 4.0 | aa | 0.00 0.00 | aa | 0.07 | ESO527-G019 |
| 2001fa | 33.90 0.19 | k | 2452198.00 3.0 | aa | 0.00 0.00 | aa | 0.07 | NGC0673 |
| 2001do | 33.39 0.15 | a | 2452133.00 2.0 | aa | 0.00 0.00 | aa | 0.17 | UGC11459 |
| 2001cy | 33.01 0.12 | h | 2452085.00 6.0 | aa | 0.00 0.00 | aa | 0.19 | UGC11927 |
| 2001X | 31.59 0.11 | h | 2451963.00 5.0 | ee | 0.07 0.04 | ee | 0.04 | NGC5921 |
| 2002gd | 32.90 0.21 | h | 2452552.00 2.0 | dd | 0.00 0.02 | m | 0.06 | NGC7537 |
| 2002gw | 33.07 0.15 | a | 2452560.00 5.0 | m | 0.00 0.02 | m | 0.02 | NGC0922 |
| 2002hj | 34.91 0.15 | a | 2452563.00 7.0 | m | 0.00 0.04 | m | 0.10 | NPM1G+04.0097 |
| 2002hh | 28.36 0.09 | h | 2452577.50 10.0 | ff | 0.70 0.00 | ff | 0.30 | NGC6946 |
| 2002hx | 35.49 0.15 | a | 2452583.00 9.0 | m | 0.00 0.07 | m | 0.05 | PCG23727 |
| 2003B | 30.94 0.15 | a | 2452617.00 11.0 | m | 0.06 0.03 | m | 0.02 | NGC1097 |
| 2003E | 34.01 0.28 | t | 2452635.00 7.0 | m | 0.00 0.00 | m | 0.04 | ESO485-G004 |
| 2003T | 35.36 0.15 | a | 2452655.00 10.0 | m | 0.00 0.00 | m | 0.03 | UGC4864 |
| 2003Z | 31.70 0.15 | a | 2452665.00 4.5 | dd | 0.00 0.00 | dd | 0.03 | NGC2742 |
| 2003bl | 34.07 0.30 | t | 2452700.00 3.0 | m | 0.00 0.09 | m | 0.02 | NGC5374 |
| 2003bn | 33.55 0.15 | a | 2452695.00 3.0 | m | 0.00 0.02 | m | 0.06 | 2MASXJ10023529 |
| 2003cn | 34.81 0.28 | t | 2452720.00 4.0 | m | 0.00 0.04 | m | 0.02 | IC0849 |
| 2003cx | 35.91 0.15 | a | 2452729.00 5.0 | m | 0.00 0.05 | m | 0.08 | – |
| 2003ef | 33.96 0.18 | v | 2452760.00 9.0 | m | 0.00 0.00 | m | 0.04 | NGC4708 |
| 2003fb | 34.36 0.15 | a | 2452777.00 6.0 | m | 0.00 0.06 | m | 0.16 | UGC11522 |
| 2003hd | 36.02 0.15 | a | 2452858.00 5.0 | m | 0.00 0.06 | m | 0.01 | MCG-04-05-010 |
| 2003hf | 35.64 0.15 | a | 2452863.00 2.0 | aa | 0.00 0.00 | aa | 0.02 | UGC10586 |
| 2003hg | 33.31 0.28 | t | 2452866.00 5.0 | m | 0.00 0.00 | m | 0.06 | NGC7771 |
| 2003hl | 32.16 0.10 | h | 2452869.00 5.0 | m | 0.00 0.00 | m | 0.06 | NGC0772 |
| 2003hn | 31.14 0.26 | i | 2452857.00 4.0 | i | 0.12 0.03 | m | 0.01 | 6dFJ0344359-443750 |
| 2003ho | 33.80 0.15 | a | 2452848.00 7.0 | m | 2.36 0.40 | m | 0.03 | ESO235-G58 |

*

a: NED , b: Kanbur et al. 2003, c: Fraser et al. 2014, d: Bose et al. 2015, e: Brown et al. 2010, f: Ferrarese et al. 1996, g: Schmidt, Kirshner & Eastman 1992, h: Poznanski et al. 2009, i: Jones et al. 2009, j: Leonard et al. 2003, k: Wang et al. 2006, l: Takats & Vinko 2006, m: Anderson et al. 2014, n: Takáts & Vinkó 2012, o: Bose & Kumar 2014, p: Freedman et al. 2001, q: Takáts et al. 2014, r: Takats et al. 2015, s: Gall et al. 2015, t: Olivares et al. 2010, u: Mould & Sakai 2008, v: Rest et al. 2014, w: This paper, x: Valenti et al. 2015, y: Valenti et al. 2014, z: Benetti et al. 1994, aa: Faran et al. 2014b, bb: Inserra et al. 2013, cc: Taddia et al. 2013, dd: Spiro et al. 2014, ee: Faran et al. 2014a, ff: Pozzo et al. 2006, gg: de Vaucouleurs et al. 1981, hh: Leonard et al. 2002, jj: Pastorello et al. 2004, kk: Terreran in prep., ll: Yaron in prep., mm: Gandhi et al. 2013, nn: Maguire et al. 2010, oo: Pastorello et al. 2009, pp: Inserra et al. 2011, qq: Tomasella et al. 2013, rr: Barbarino et al. 2015, ss: Inserra et al. 2012, tt: Fraser et al. 2011, uu: Gal-Yam et al. 2011, vv: Elias-Rosa et al. 2011, ww: Dessart et al. 2008, xx: Dall'Ora et al. 2014, zz: Poznanski et al. 2015, ab: Elias-Rosa et al. 2010, ac: Zwitter, Munari & Moretti 2004, ad: Quimby et al. 2007, ae: Andrews et al. 2011,

**Table 2:** continued ..

| SN | Distance modulus | REF* ($\mu$) | Explosion epoch | | m REF* (explosion) | E(B-V) (host) | REF* (E(B-V) host) | $E(B-V)^x$ M.W. | Host galaxy |
|---|---|---|---|---|---|---|---|---|---|
| 2003ib | 35.12 0.15 | a | 2452891.00 | 5.0 | m | 0.00 0.09 | m | 0.04 | MCG-04-48-15 |
| 2003ip | 33.76 0.28 | t | 2452897.00 | 4.0 | m | 0.04 0.03 | m | 0.06 | UGC00327 |
| 2003iq | 32.16 0.10 | h | 2452920.00 | 2.0 | m | 0.00 0.00 | m | 0.06 | NGC0772 |
| 2004du | 33.94 0.02 | h | 2453228.00 | 2.0 | aa | 0.00 0.00 | ee | 0.08 | UGC11683 |
| 2004et | 28.36 0.09 | h | 2453270.50 | 4.0 | nn | 0.11 0.05 | ac | 0.30 | NGC6946 |
| 2004er | 33.83 0.15 | a | 2453272.20 | 2.0 | m | 0.11 0.05 | m | 0.02 | UGCA036 |
| 2004fx | 32.71 0.15 | a | 2453304.00 | 4.0 | m | 0.00 0.03 | m | 0.09 | MCG-02-14-3 |
| 2005J | 34.06 0.15 | a | 2453383.20 | 7.0 | m | 0.07 0.10 | m | 0.02 | NGC4012 |
| 2005K | 35.26 0.15 | a | 2453370.20 | 7.0 | m | 0.00 0.00 | m | 0.03 | NGC2923 |
| 2005af | 27.90 0.10 | u | 2453324.30 | 15.0 | m | 0.00 0.04 | m | 0.16 | NGC4945 |
| 2005dq | 34.77 0.15 | a | 2453608.00 | 4.0 | aa | 0.00 0.00 | aa | 0.07 | UGC12177 |
| 2005cs | 29.26 0.33 | l | 2453549.00 | 0.5 | oo | 0.02 0.01 | oo | 0.03 | NGC5194 |
| 2005dx | 35.16 0.15 | a | 2453616.30 | 7.0 | m | 0.00 0.09 | m | 0.02 | ESO550-G002 |
| 2005dz | 34.44 0.15 | a | 2453620.00 | 4.0 | m | 0.00 0.04 | m | 0.07 | UGC12717 |
| 2006Y | 35.70 0.06 | m | 2453767.00 | 4.0 | m | 0.00 0.04 | m | 0.11 | ESO207-G026 |
| 2006iw | 35.49 0.15 | a | 2454011.10 | 1.0 | m | 0.00 0.04 | m | 0.04 | 2MASXJ23211915+0015329 |
| 2006ai | 34.01 0.14 | m | 2453782.30 | 5.0 | m | 0.00 0.03 | m | 0.11 | ESO005-G009 |
| 2006bp | 31.58 0.18 | n | 2453834.50 | 2.0 | ad | 0.40 0.10 | ww | 0.03 | NGC3953 |
| 2007W | 33.14 0.15 | a | 2454137.30 | 7.0 | m | 0.00 0.03 | m | 0.05 | NGC5105 |
| 2007U | 35.12 0.15 | a | 2454135.10 | 6.0 | m | 0.00 0.12 | m | 0.05 | ESO552-G065 |
| 2007X | 32.62 0.15 | a | 2454144.30 | 5.0 | m | 0.12 0.06 | m | 0.06 | ESO385-G032 |
| 2007ab | 34.97 0.15 | a | 2454124.30 | 10.0 | m | 0.00 0.00 | m | 0.23 | MCG-01-43-2 |
| 2007it | 30.35 0.36 | a | 2454349.00 | 10.0 | ae | 0.00 0.00 | ae | 0.42 | NGC5530 |
| 2007ld | 35.50 0.15 | a | 2454378.00 | 8.0 | m | 0.00 0.05 | m | 0.08 | SDSSJ204929.40+000016.8 |
| 2007od | 31.95 0.15 | a | 2454404.00 | 5.0 | pp | 0.00 0.02 | m | 0.03 | UGC12846 |
| 2008M | 32.42 0.15 | a | 2454472.20 | 9.0 | m | 0.00 0.02 | m | 0.04 | ESO121-26 |
| 2008K | 35.35 0.15 | a | 2454478.20 | 4.0 | m | 0.00 0.02 | m | 0.03 | ESO504-G005 |
| 2008aw | 33.21 0.15 | a | 2454518.20 | 10.0 | m | 0.10 0.05 | m | 0.04 | NGC4939 |
| 2008bu | 34.81 0.15 | a | 2454567.20 | 7.0 | m | 0.00 0.04 | m | 0.37 | ESO586-G2 |
| 2008fq | 33.38 0.15 | a | 2454720.00 | 5.0 | aa | 0.46 0.10 | cc | 0.06 | NGC6907 |
| 2008ho | 33.07 0.15 | a | 2454793.20 | 5.0 | m | 0.05 0.03 | m | 0.02 | NGC0922 |
| 2008if | 33.54 0.15 | a | 2454808.30 | 5.0 | m | 0.07 0.04 | m | 0.03 | MCG-01-24-010 |
| 2008in | 30.45 0.10 | o | 2454825.60 | 1.0 | o | 0.03 0.02 | m | 0.02 | MESSIER061 |
| 2009N | 31.67 0.11 | q | 2454848.10 | 1.2 | q | 0.03 0.02 | m | 0.02 | NGC4487 |
| 2009bw | 31.44 0.15 | a | 2454916.50 | 3.0 | ss | 0.08 0.04 | ss | 0.20 | UGC02890 |
| 2009dd | 30.91 0.15 | a | 2454925.50 | 5.0 | bb | 0.43 0.10 | bb | 0.02 | NGC4088 |
| 2009hd | 29.86 0.08 | p | 2455002.00 | 20.0 | vv | 1.20 0.07 | vv | 0.03 | SDSSJ112017.26+125829.1 |
| 2009ib | 31.48 0.31 | r | 2455041.30 | 2.0 | r | 0.13 0.05 | r | 0.03 | NGC1559 |
| 2009js | 31.57 0.15 | a | 2455110.00 | 5.5 | mm | 0.05 0.16 | mm | 0.31 | NGC0918 |
| 2009kr | 32.09 0.15 | a | 2455140.50 | 2.0 | w | 0.01 0.00 | ab | 0.06 | NGC1832 |
| 2009md | 31.66 0.15 | a | 2455162.00 | 8.0 | tt | 0.10 0.05 | tt | 0.02 | NGC3389 |
| 2010id | 34.15 0.15 | a | 2455452.00 | 2.0 | uu | 0.00 0.00 | uu | 0.05 | NGC7483 |
| 2012A | 29.96 0.15 | a | 2455932.50 | 2.0 | qq | 0.01 0.00 | qq | 0.03 | NGC3239 |
| 2012aw | 29.96 0.09 | o | 2456002.50 | 4.0 | ad | 0.06 0.02 | xx | 0.02 | SDSSJ104357.53+114056.0 |
| 2012ec | 31.32 0.15 | a | 2456143.00 | 5.0 | rr | 0.12 0.05 | rr | 0.02 | NGC1084 |
| lsq13cuw | 36.38 0.13 | s | 2456593.42 | 0.7 | s | 0.00 0.00 | s | 0.02 | SDSSJ023957.37-083123.8 |
| OGLE13-005 | 37.42 0.15 | a | 2456241.70 | 2.9 | zz | 0.00 0.00 | zz | 0.03 | – |
| OGLE13-011 | 36.66 0.15 | a | 2456298.25 | 6.5 | zz | 0.00 0.00 | zz | 0.05 | – |
| OGLE13-045 | 38.25 0.15 | a | 2456483.40 | 2.5 | zz | 0.00 0.00 | zz | 0.03 | – |
| OGLE13-046 | 37.42 0.15 | a | 2456489.90 | 2.0 | zz | 0.00 0.00 | zz | 0.03 | – |
| OGLE13-047 | 37.09 0.15 | a | 2456505.30 | 4.5 | zz | 0.00 0.00 | zz | 0.03 | – |
| OGLE13-048 | 37.09 0.15 | a | 2456489.40 | 1.5 | zz | 0.00 0.00 | zz | 0.04 | – |
| OGLE13-135 | 36.97 0.15 | a | 2456620.65 | 2.0 | zz | 0.00 0.00 | zz | 0.16 | – |
| OGLE13-144 | 36.19 0.15 | a | 2456635.70 | 6.0 | zz | 0.00 0.00 | zz | 0.11 | – |
| OGLE14-004 | 35.54 0.15 | a | 2456660.30 | 2.5 | zz | 0.00 0.00 | zz | 0.07 | – |
| OGLE14-009 | 36.93 0.15 | a | 2456688.20 | 1.5 | zz | 0.00 0.00 | zz | 0.07 | – |

*

a: NED , b: Kanbur et al. 2003, c: Fraser et al. 2014, d: Bose et al. 2015, e: Brown et al. 2010, f: Ferrarese et al. 1996, g: Schmidt, Kirshner & Eastman 1992, h: Poznanski et al. 2009, i: Jones et al. 2009, j: Leonard et al. 2003, k: Wang et al. 2006, l: Takats & Vinko 2006, m: Anderson et al. 2014, n: Takáts & Vinkó 2012, o: Bose & Kumar 2014, p: Freedman et al. 2001, q: Takáts et al. 2014, r: Takats et al. 2015, s: Gall et al. 2015, t: Olivares et al. 2010, u: Mould & Sakai 2008, v: Rest et al. 2014, w: This paper, x: Valenti et al. 2015, y: Valenti et al. 2014, z: Benetti et al. 1994, aa: Faran et al. 2014b, bb: Inserra et al. 2013, cc: Taddia et al. 2013, dd: Spiro et al. 2014, ee: Faran et al. 2014a, ff: Pozzo et al. 2006, gg: de Vaucouleurs et al. 1981, hh: Leonard et al. 2002, jj: Pastorello et al. 2004, kk: Terreran in prep., ll: Yaron in prep., mm: Gandhi et al. 2013, nn: Maguire et al. 2010, oo: Pastorello et al. 2009, pp: Inserra et al. 2011, qq: Tomasella et al. 2013, rr: Barbarino et al. 2015, ss: Inserra et al. 2012, tt: Fraser et al. 2011, uu: Gal-Yam et al. 2011, vv: Elias-Rosa et al. 2011, ww: Dessart et al. 2008, xx: Dall'Ora et al. 2014, zz: Poznanski et al. 2015, ab: Elias-Rosa et al. 2010, ac: Zwitter, Munari & Moretti 2004, ad: Quimby et al. 2007, ae: Andrews et al. 2011,

**Table D1:** SN 2013fs: Photometric Data

| Date | JD | mag[(a)] | Filter | telescope[(b)] | Date | JD | mag[(a)] | Filter | telescope[(b)] |
|---|---|---|---|---|---|---|---|---|---|
| 2013-10-07 | 2456572.503 | 14.267 0.069 | *uw*2 | *Swift* | 2013-10-30 | 2456596.070 | 17.704 0.100 | *uw*1 | *Swift* |
| 2013-10-08 | 2456574.310 | 14.275 0.070 | *uw*2 | *Swift* | 2013-10-09 | 2456575.478 | 14.826 0.050 | *us* | *Swift* |
| 2013-10-09 | 2456575.481 | 14.575 0.070 | *uw*2 | *Swift* | 2013-10-10 | 2456576.412 | 14.922 0.050 | *us* | *Swift* |
| 2013-10-10 | 2456576.414 | 15.028 0.071 | *uw*2 | *Swift* | 2013-10-11 | 2456576.907 | 14.905 0.051 | *us* | *Swift* |
| 2013-10-11 | 2456576.909 | 14.927 0.070 | *uw*2 | *Swift* | 2013-10-12 | 2456577.808 | 14.950 0.053 | *us* | *Swift* |
| 2013-10-12 | 2456577.814 | 15.151 0.071 | *uw*2 | *Swift* | 2013-10-13 | 2456579.216 | 15.094 0.053 | *us* | *Swift* |
| 2013-10-13 | 2456579.223 | 15.577 0.073 | *uw*2 | *Swift* | 2013-10-15 | 2456580.577 | 15.183 0.056 | *us* | *Swift* |
| 2013-10-15 | 2456580.580 | 15.841 0.075 | *uw*2 | *Swift* | 2013-10-18 | 2456584.147 | 15.516 0.057 | *us* | *Swift* |
| 2013-10-18 | 2456584.149 | 16.567 0.079 | *uw*2 | *Swift* | 2013-10-19 | 2456584.849 | 15.575 0.055 | *us* | *Swift* |
| 2013-10-19 | 2456584.853 | 16.802 0.078 | *uw*2 | *Swift* | 2013-10-20 | 2456585.990 | 15.680 0.056 | *us* | *Swift* |
| 2013-10-20 | 2456585.993 | 16.899 0.079 | *uw*2 | *Swift* | 2013-10-21 | 2456586.892 | 15.783 0.056 | *us* | *Swift* |
| 2013-10-21 | 2456586.895 | 17.081 0.080 | *uw*2 | *Swift* | 2013-10-22 | 2456588.087 | 15.895 0.060 | *us* | *Swift* |
| 2013-10-22 | 2456588.093 | 17.241 0.086 | *uw*2 | *Swift* | 2013-10-23 | 2456588.953 | 15.915 0.059 | *us* | *Swift* |
| 2013-10-23 | 2456588.956 | 17.441 0.088 | *uw*2 | *Swift* | 2013-10-24 | 2456589.859 | 16.082 0.060 | *us* | *Swift* |
| 2013-10-24 | 2456589.862 | 17.530 0.089 | *uw*2 | *Swift* | 2013-10-25 | 2456590.997 | 16.122 0.059 | *us* | *Swift* |
| 2013-10-25 | 2456591.000 | 17.678 0.089 | *uw*2 | *Swift* | 2013-10-26 | 2456591.891 | 16.218 0.073 | *us* | *Swift* |
| 2013-10-27 | 2456593.443 | 18.144 0.102 | *uw*2 | *Swift* | 2013-10-27 | 2456593.441 | 16.521 0.065 | *us* | *Swift* |
| 2013-10-28 | 2456593.646 | 18.183 0.104 | *uw*2 | *Swift* | 2013-10-28 | 2456593.644 | 16.552 0.066 | *us* | *Swift* |
| 2013-10-29 | 2456595.211 | 18.254 0.106 | *uw*2 | *Swift* | 2013-10-29 | 2456595.207 | 16.655 0.067 | *us* | *Swift* |
| 2013-10-30 | 2456596.075 | 18.387 0.110 | *uw*2 | *Swift* | 2013-10-30 | 2456596.072 | 16.718 0.069 | *us* | *Swift* |
| 2013-10-07 | 2456572.509 | 14.493 0.060 | *um*2 | *Swift* | 2013-10-07 | 2456572.773 | 15.593 0.019 | *U* | 1m0-08 |
| 2013-10-08 | 2456574.317 | 14.288 0.059 | *um*2 | *Swift* | 2013-10-08 | 2456573.655 | 15.371 0.030 | *U* | 1m0-08 |
| 2013-10-09 | 2456575.426 | 14.492 0.061 | *um*2 | *Swift* | 2013-10-09 | 2456574.651 | 15.340 0.013 | *U* | 1m0-08 |
| 2013-10-10 | 2456576.395 | 14.861 0.062 | *um*2 | *Swift* | 2013-10-10 | 2456575.642 | 15.329 0.022 | *U* | 1m0-08 |
| 2013-10-11 | 2456576.912 | 14.821 0.061 | *um*2 | *Swift* | 2013-10-11 | 2456576.742 | 15.308 0.013 | *U* | 1m0-08 |
| 2013-10-12 | 2456577.824 | 15.021 0.064 | *um*2 | *Swift* | 2013-10-18 | 2456583.609 | 15.725 0.012 | *U* | 1m0-08 |
| 2013-10-13 | 2456579.232 | 15.314 0.068 | *um*2 | *Swift* | 2013-10-20 | 2456585.619 | 15.877 0.033 | *U* | 1m0-08 |
| 2013-10-15 | 2456580.582 | 15.642 0.074 | *um*2 | *Swift* | 2013-10-21 | 2456586.643 | 15.932 0.027 | *U* | 1m0-08 |
| 2013-10-18 | 2456584.151 | 16.450 0.085 | *um*2 | *Swift* | 2013-10-22 | 2456587.729 | 16.042 0.027 | *U* | 1m0-08 |
| 2013-10-19 | 2456584.858 | 16.659 0.078 | *um*2 | *Swift* | 2013-10-23 | 2456588.667 | 16.079 0.041 | *U* | 1m0-08 |
| 2013-10-20 | 2456585.996 | 16.872 0.083 | *um*2 | *Swift* | 2013-10-25 | 2456590.658 | 16.372 0.055 | *U* | 1m0-08 |
| 2013-10-21 | 2456586.899 | 16.992 0.082 | *um*2 | *Swift* | 2013-10-26 | 2456591.703 | 16.344 0.016 | *U* | 1m0-08 |
| 2013-10-22 | 2456588.100 | 17.279 0.098 | *um*2 | *Swift* | 2013-10-27 | 2456592.692 | 16.453 0.042 | *U* | 1m0-08 |
| 2013-10-23 | 2456588.958 | 17.261 0.099 | *um*2 | *Swift* | 2013-10-28 | 2456593.591 | 16.521 0.041 | *U* | 1m0-08 |
| 2013-10-24 | 2456589.867 | 17.534 0.101 | *um*2 | *Swift* | 2013-10-29 | 2456594.649 | 16.552 0.042 | *U* | 1m0-08 |
| 2013-10-25 | 2456591.003 | 17.693 0.104 | *um*2 | *Swift* | 2013-11-02 | 2456598.701 | 17.065 0.035 | *U* | 1m0-08 |
| 2013-10-27 | 2456593.446 | 18.008 0.121 | *um*2 | *Swift* | 2013-11-06 | 2456602.593 | 17.424 0.010 | *U* | 1m0-08 |
| 2013-10-28 | 2456593.648 | 18.141 0.128 | *um*2 | *Swift* | 2013-11-10 | 2456606.672 | 17.497 0.057 | *U* | 1m0-08 |
| 2013-10-29 | 2456595.215 | 18.257 0.136 | *um*2 | *Swift* | 2013-11-21 | 2456617.518 | 18.119 0.095 | *U* | 1m0-05 |
| 2013-10-30 | 2456596.079 | 18.317 0.138 | *um*2 | *Swift* | 2013-12-03 | 2456629.543 | 18.795 0.251 | *U* | 1m0-09 |
| 2013-10-06 | 2456572.491 | 14.699 0.059 | *uw*1 | *Swift* | 2013-12-05 | 2456631.535 | 19.027 0.036 | *U* | 1m0-09 |
| 2013-10-08 | 2456574.292 | 14.447 0.057 | *uw*1 | *Swift* | 2013-12-11 | 2456637.539 | 18.678 0.411 | *U* | 1m0-04 |
| 2013-10-09 | 2456575.476 | 14.594 0.057 | *uw*1 | *Swift* | 2013-12-14 | 2456640.672 | 18.875 0.474 | *U* | 1m0-08 |
| 2013-10-10 | 2456576.410 | 14.824 0.058 | *uw*1 | *Swift* | 2013-10-09 | 2456575.479 | 16.086 0.047 | *bs* | *Swift* |
| 2013-10-11 | 2456576.906 | 14.805 0.058 | *uw*1 | *Swift* | 2013-10-10 | 2456576.413 | 16.105 0.046 | *bs* | *Swift* |
| 2013-10-12 | 2456577.805 | 14.936 0.060 | *uw*1 | *Swift* | 2013-10-11 | 2456576.908 | 16.040 0.047 | *bs* | *Swift* |
| 2013-10-13 | 2456579.242 | 15.205 0.060 | *uw*1 | *Swift* | 2013-10-12 | 2456577.809 | 16.029 0.050 | *bs* | *Swift* |
| 2013-10-15 | 2456580.576 | 15.483 0.065 | *uw*1 | *Swift* | 2013-10-13 | 2456579.218 | 16.094 0.050 | *bs* | *Swift* |
| 2013-10-18 | 2456584.146 | 16.095 0.070 | *uw*1 | *Swift* | 2013-10-15 | 2456580.578 | 16.125 0.053 | *bs* | *Swift* |
| 2013-10-19 | 2456584.848 | 16.217 0.068 | *uw*1 | *Swift* | 2013-10-18 | 2456584.148 | 16.316 0.053 | *bs* | *Swift* |
| 2013-10-20 | 2456585.989 | 16.376 0.069 | *uw*1 | *Swift* | 2013-10-19 | 2456584.850 | 16.429 0.052 | *bs* | *Swift* |
| 2013-10-21 | 2456586.891 | 16.535 0.069 | *uw*1 | *Swift* | 2013-10-20 | 2456585.991 | 16.456 0.052 | *bs* | *Swift* |
| 2013-10-22 | 2456588.085 | 16.601 0.076 | *uw*1 | *Swift* | 2013-10-21 | 2456586.893 | 16.510 0.051 | *bs* | *Swift* |
| 2013-10-23 | 2456588.952 | 16.829 0.078 | *uw*1 | *Swift* | 2013-10-22 | 2456588.089 | 16.523 0.055 | *bs* | *Swift* |
| 2013-10-24 | 2456589.857 | 16.907 0.079 | *uw*1 | *Swift* | 2013-10-23 | 2456588.954 | 16.554 0.054 | *bs* | *Swift* |
| 2013-10-25 | 2456590.996 | 17.080 0.080 | *uw*1 | *Swift* | 2013-10-24 | 2456589.860 | 16.607 0.054 | *bs* | *Swift* |
| 2013-10-26 | 2456591.889 | 17.333 0.115 | *uw*1 | *Swift* | 2013-10-25 | 2456590.998 | 16.572 0.052 | *bs* | *Swift* |
| 2013-10-27 | 2456593.440 | 17.425 0.091 | *uw*1 | *Swift* | 2013-10-26 | 2456591.891 | 16.802 0.207 | *bs* | *Swift* |
| 2013-10-28 | 2456593.643 | 17.529 0.094 | *uw*1 | *Swift* | 2013-10-27 | 2456593.442 | 16.729 0.055 | *bs* | *Swift* |
| 2013-10-29 | 2456595.205 | 17.840 0.105 | *uw*1 | *Swift* | 2013-10-28 | 2456593.644 | 16.748 0.056 | *bs* | *Swift* |

(a) Data have not been corrected for extinction
(b) *Swift* Telescope; LSQ (La Silla Quest, Chile); 1m0-08 (McDonald Observatory, USA); 1m0-10, 1m0-12, 1m0-13 (Sutherland, South Africa), 1m0-04, 1m0-05, 1m0-09 (Cerro Tololo, Chile); 1m0-03, 1m0-11 (Siding Spring, Australia).

**Table D1:** SN 2013fs: Photometric Data

| Date | JD | mag$^{(a)}$ | Filter | telescope$^{(b)}$ | Date | JD | mag$^{(a)}$ | Filter | telescope$^{(b)}$ |
|---|---|---|---|---|---|---|---|---|---|
| 2013-10-29 | 2456595.208 | 16.848 0.056 | *bs* | *Swift* | 2013-12-03 | 2456629.549 | 17.310 0.001 | *g* | 1m0-04 |
| 2013-10-30 | 2456596.073 | 16.898 0.057 | *bs* | *Swift* | 2013-12-04 | 2456631.283 | 17.342 0.014 | *g* | 1m0-13 |
| 2013-10-07 | 2456572.781 | 16.270 0.018 | *B* | 1m0-08 | 2013-12-11 | 2456637.544 | 17.389 0.009 | *g* | 1m0-09 |
| 2013-10-08 | 2456573.665 | 16.103 0.012 | *B* | 1m0-08 | 2013-12-14 | 2456640.922 | 17.566 0.005 | *g* | 1m0-11 |
| 2013-10-09 | 2456574.662 | 16.004 0.028 | *B* | 1m0-08 | 2013-12-18 | 2456644.543 | 17.666 0.013 | *g* | 1m0-08 |
| 2013-10-10 | 2456575.652 | 15.984 0.021 | *B* | 1m0-08 | 2013-12-20 | 2456646.662 | 17.679 0.003 | *g* | 1m0-08 |
| 2013-10-11 | 2456576.752 | 16.068 0.013 | *B* | 1m0-08 | 2014-01-17 | 2456674.581 | 19.365 0.002 | *g* | 1m0-08 |
| 2013-10-18 | 2456583.619 | 16.250 0.034 | *B* | 1m0-08 | 2013-10-09 | 2456575.449 | 16.099 0.060 | *vs* | *Swift* |
| 2013-10-20 | 2456585.630 | 16.357 0.015 | *B* | 1m0-08 | 2013-10-10 | 2456576.394 | 16.058 0.059 | *vs* | *Swift* |
| 2013-10-21 | 2456586.627 | 16.398 0.016 | *B* | 1m0-08 | 2013-10-11 | 2456576.911 | 15.978 0.051 | *vs* | *Swift* |
| 2013-10-22 | 2456587.739 | 16.481 0.015 | *B* | 1m0-08 | 2013-10-12 | 2456577.820 | 15.976 0.048 | *vs* | *Swift* |
| 2013-10-23 | 2456588.678 | 16.477 0.018 | *B* | 1m0-08 | 2013-10-13 | 2456579.228 | 16.000 0.048 | *vs* | *Swift* |
| 2013-10-25 | 2456590.682 | 16.574 0.021 | *B* | 1m0-08 | 2013-10-15 | 2456580.581 | 16.025 0.065 | *vs* | *Swift* |
| 2013-10-26 | 2456591.714 | 16.646 0.012 | *B* | 1m0-08 | 2013-10-18 | 2456584.150 | 16.092 0.063 | *vs* | *Swift* |
| 2013-10-27 | 2456592.703 | 16.624 0.017 | *B* | 1m0-08 | 2013-10-19 | 2456584.856 | 16.277 0.061 | *vs* | *Swift* |
| 2013-10-28 | 2456593.601 | 16.725 0.011 | *B* | 1m0-08 | 2013-10-20 | 2456585.995 | 16.164 0.059 | *vs* | *Swift* |
| 2013-10-29 | 2456594.659 | 16.720 0.035 | *B* | 1m0-08 | 2013-10-21 | 2456586.898 | 16.288 0.059 | *vs* | *Swift* |
| 2013-11-02 | 2456598.711 | 16.931 0.012 | *B* | 1m0-08 | 2013-10-22 | 2456588.097 | 16.318 0.067 | *vs* | *Swift* |
| 2013-11-03 | 2456599.690 | 17.002 0.012 | *B* | 1m0-08 | 2013-10-23 | 2456588.957 | 16.449 0.067 | *vs* | *Swift* |
| 2013-11-06 | 2456602.604 | 17.110 0.022 | *B* | 1m0-08 | 2013-10-24 | 2456589.865 | 16.391 0.065 | *vs* | *Swift* |
| 2013-11-10 | 2456606.683 | 17.252 0.012 | *B* | 1m0-08 | 2013-10-25 | 2456591.001 | 16.428 0.063 | *vs* | *Swift* |
| 2013-11-20 | 2456616.680 | 17.601 0.024 | *B* | 1m0-08 | 2013-10-27 | 2456593.445 | 16.491 0.067 | *vs* | *Swift* |
| 2013-11-21 | 2456617.531 | 17.568 0.023 | *B* | 1m0-05 | 2013-10-28 | 2456593.647 | 16.421 0.066 | *vs* | *Swift* |
| 2013-12-03 | 2456629.550 | 17.807 0.021 | *B* | 1m0-09 | 2013-10-29 | 2456595.213 | 16.551 0.069 | *vs* | *Swift* |
| 2013-12-05 | 2456631.547 | 17.972 0.031 | *B* | 1m0-09 | 2013-10-30 | 2456596.078 | 16.556 0.069 | *vs* | *Swift* |
| 2013-12-11 | 2456637.553 | 17.951 0.039 | *B* | 1m0-04 | 2013-10-07 | 2456572.786 | 16.499 0.016 | *V* | 1m0-08 |
| 2013-12-14 | 2456640.662 | 18.148 0.086 | *B* | 1m0-08 | 2013-10-08 | 2456573.671 | 16.274 0.015 | *V* | 1m0-08 |
| 2013-12-17 | 2456643.609 | 18.223 0.083 | *B* | 1m0-08 | 2013-10-09 | 2456574.667 | 16.103 0.029 | *V* | 1m0-08 |
| 2013-12-20 | 2456646.639 | 18.264 0.040 | *B* | 1m0-08 | 2013-10-10 | 2456575.657 | 16.020 0.025 | *V* | 1m0-08 |
| 2013-12-23 | 2456649.622 | 18.755 0.015 | *B* | 1m0-08 | 2013-10-18 | 2456583.624 | 16.099 0.019 | *V* | 1m0-08 |
| 2014-01-15 | 2456672.566 | 20.103 0.039 | *B* | 1m0-08 | 2013-10-20 | 2456585.635 | 16.223 0.014 | *V* | 1m0-08 |
| 2014-01-19 | 2456676.564 | 20.307 0.043 | *B* | 1m0-08 | 2013-10-21 | 2456586.632 | 16.220 0.017 | *V* | 1m0-08 |
| 2013-10-07 | 2456572.637 | 16.568 0.004 | *g* | 1m0-08 | 2013-10-23 | 2456588.683 | 16.310 0.024 | *V* | 1m0-08 |
| 2013-10-08 | 2456573.692 | 16.263 0.004 | *g* | 1m0-08 | 2013-10-25 | 2456590.716 | 16.397 0.011 | *V* | 1m0-08 |
| 2013-10-09 | 2456574.697 | 16.179 0.003 | *g* | 1m0-08 | 2013-10-26 | 2456591.719 | 16.412 0.043 | *V* | 1m0-08 |
| 2013-10-11 | 2456576.760 | 16.083 0.008 | *g* | 1m0-08 | 2013-10-27 | 2456592.708 | 16.435 0.017 | *V* | 1m0-08 |
| 2013-10-12 | 2456577.761 | 16.023 0.009 | *g* | 1m0-08 | 2013-10-28 | 2456593.606 | 16.416 0.069 | *V* | 1m0-08 |
| 2013-10-18 | 2456583.636 | 16.242 0.011 | *g* | 1m0-08 | 2013-10-29 | 2456594.665 | 16.449 0.020 | *V* | 1m0-08 |
| 2013-10-19 | 2456584.647 | 16.338 0.015 | *g* | 1m0-08 | 2013-11-02 | 2456598.717 | 16.531 0.015 | *V* | 1m0-08 |
| 2013-10-20 | 2456585.599 | 16.313 0.004 | *g* | 1m0-08 | 2013-11-03 | 2456599.696 | 16.619 0.017 | *V* | 1m0-08 |
| 2013-10-21 | 2456586.596 | 16.369 0.003 | *g* | 1m0-08 | 2013-11-06 | 2456602.609 | 16.596 0.014 | *V* | 1m0-08 |
| 2013-10-22 | 2456587.706 | 16.416 0.009 | *g* | 1m0-08 | 2013-11-10 | 2456606.688 | 16.610 0.014 | *V* | 1m0-08 |
| 2013-10-23 | 2456588.734 | 16.486 0.005 | *g* | 1m0-08 | 2013-11-20 | 2456616.686 | 16.736 0.018 | *V* | 1m0-08 |
| 2013-10-26 | 2456591.596 | 16.516 0.001 | *g* | 1m0-08 | 2013-11-21 | 2456617.537 | 16.745 0.013 | *V* | 1m0-05 |
| 2013-10-27 | 2456592.585 | 16.587 0.005 | *g* | 1m0-08 | 2013-12-03 | 2456629.558 | 16.846 0.013 | *V* | 1m0-09 |
| 2013-10-28 | 2456593.630 | 16.593 0.008 | *g* | 1m0-08 | 2013-12-05 | 2456631.554 | 16.865 0.011 | *V* | 1m0-09 |
| 2013-10-29 | 2456594.610 | 16.641 0.002 | *g* | 1m0-08 | 2013-12-11 | 2456637.559 | 17.009 0.014 | *V* | 1m0-04 |
| 2013-11-02 | 2456598.678 | 16.803 0.004 | *g* | 1m0-08 | 2013-12-14 | 2456640.669 | 17.026 0.028 | *V* | 1m0-08 |
| 2013-11-03 | 2456599.669 | 16.778 0.002 | *g* | 1m0-08 | 2013-12-20 | 2456646.645 | 17.098 0.028 | *V* | 1m0-08 |
| 2013-11-06 | 2456602.671 | 16.884 0.005 | *g* | 1m0-08 | 2013-12-23 | 2456649.629 | 17.353 0.029 | *V* | 1m0-08 |
| 2013-11-10 | 2456606.651 | 16.969 0.002 | *g* | 1m0-08 | 2014-01-15 | 2456672.574 | 18.960 0.111 | *V* | 1m0-08 |
| 2013-11-12 | 2456608.686 | 17.007 0.009 | *g* | 1m0-08 | 2014-01-19 | 2456676.570 | 19.023 0.070 | *V* | 1m0-08 |
| 2013-11-15 | 2456611.694 | 17.065 0.010 | *g* | 1m0-08 | 2013-10-07 | 2456572.643 | 16.810 0.005 | *r* | 1m0-08 |
| 2013-11-20 | 2456616.608 | 17.142 0.002 | *g* | 1m0-08 | 2013-10-08 | 2456573.732 | 16.404 0.001 | *r* | 1m0-08 |
| 2013-11-20 | 2456616.911 | 17.164 0.013 | *g* | 1m0-11 | 2013-10-09 | 2456574.702 | 16.276 0.011 | *r* | 1m0-08 |
| 2013-11-25 | 2456621.519 | 17.191 0.010 | *g* | 1m0-09 | 2013-10-11 | 2456576.765 | 16.096 0.011 | *r* | 1m0-08 |
| 2013-11-28 | 2456624.530 | 17.182 0.011 | *g* | 1m0-04 | 2013-10-12 | 2456577.766 | 16.046 0.007 | *r* | 1m0-08 |
| 2013-11-28 | 2456625.272 | 17.245 0.025 | *g* | 1m0-12 | 2013-10-18 | 2456583.641 | 16.102 0.001 | *r* | 1m0-08 |
| 2013-11-30 | 2456626.523 | 17.293 0.003 | *g* | 1m0-04 | 2013-10-19 | 2456584.653 | 16.061 0.005 | *r* | 1m0-08 |
| 2013-12-01 | 2456627.523 | 17.248 0.006 | *g* | 1m0-09 | 2013-10-20 | 2456585.604 | 16.135 0.002 | *r* | 1m0-08 |

(a) Data have not been corrected for extinction
(b) *Swift* Telescope; LSQ (La Silla Quest, Chile); 1m0-08 (McDonald Observatory, USA); 1m0-10, 1m0-12, 1m0-13 (Sutherland, South Africa), 1m0-04, 1m0-05, 1m0-09 (Cerro Tololo, Chile); 1m0-03, 1m0-11 (Siding Spring, Australia).

**Table D1:** SN 2013fs: Photometric Data

| Date | JD | mag$^{(a)}$ | Filter | telescope$^{(b)}$ | Date | JD | mag$^{(a)}$ | Filter | telescope$^{(b)}$ |
|---|---|---|---|---|---|---|---|---|---|
| 2013-10-21 | 2456586.601 | 16.179 0.014 | $r$ | 1m0-08 | 2014-01-17 | 2456674.592 | 18.175 0.080 | $R$ | 1m0-08 |
| 2013-10-22 | 2456587.711 | 16.231 0.000 | $r$ | 1m0-08 | 2013-10-07 | 2456572.646 | 17.048 0.009 | $i$ | 1m0-08 |
| 2013-10-23 | 2456588.740 | 16.300 0.001 | $r$ | 1m0-08 | 2013-10-08 | 2456573.735 | 16.625 0.007 | $i$ | 1m0-08 |
| 2013-10-26 | 2456591.602 | 16.301 0.007 | $r$ | 1m0-08 | 2013-10-09 | 2456574.706 | 16.456 0.012 | $i$ | 1m0-08 |
| 2013-10-27 | 2456592.590 | 16.333 0.002 | $r$ | 1m0-08 | 2013-10-11 | 2456576.768 | 16.232 0.011 | $i$ | 1m0-08 |
| 2013-10-28 | 2456593.635 | 16.331 0.006 | $r$ | 1m0-08 | 2013-10-12 | 2456577.769 | 16.142 0.018 | $i$ | 1m0-08 |
| 2013-10-29 | 2456594.615 | 16.351 0.003 | $r$ | 1m0-08 | 2013-10-18 | 2456583.644 | 16.096 0.005 | $i$ | 1m0-08 |
| 2013-11-02 | 2456598.684 | 16.396 0.002 | $r$ | 1m0-08 | 2013-10-20 | 2456585.607 | 16.173 0.014 | $i$ | 1m0-08 |
| 2013-11-03 | 2456599.674 | 16.409 0.004 | $r$ | 1m0-08 | 2013-10-21 | 2456586.604 | 16.193 0.000 | $i$ | 1m0-08 |
| 2013-11-06 | 2456602.676 | 16.406 0.017 | $r$ | 1m0-08 | 2013-10-22 | 2456587.715 | 16.260 0.018 | $i$ | 1m0-08 |
| 2013-11-10 | 2456606.657 | 16.449 0.001 | $r$ | 1m0-08 | 2013-10-23 | 2456588.743 | 16.318 0.005 | $i$ | 1m0-08 |
| 2013-11-12 | 2456608.692 | 16.463 0.001 | $r$ | 1m0-08 | 2013-10-26 | 2456591.605 | 16.414 0.003 | $i$ | 1m0-08 |
| 2013-11-15 | 2456611.700 | 16.499 0.004 | $r$ | 1m0-08 | 2013-10-27 | 2456592.593 | 16.425 0.003 | $i$ | 1m0-08 |
| 2013-11-20 | 2456616.614 | 16.512 0.002 | $r$ | 1m0-08 | 2013-10-28 | 2456593.638 | 16.426 0.005 | $i$ | 1m0-08 |
| 2013-11-25 | 2456621.525 | 16.499 0.001 | $r$ | 1m0-09 | 2013-10-29 | 2456594.619 | 16.460 0.007 | $i$ | 1m0-08 |
| 2013-11-28 | 2456624.536 | 16.601 0.005 | $r$ | 1m0-04 | 2013-11-02 | 2456598.687 | 16.466 0.009 | $i$ | 1m0-08 |
| 2013-11-28 | 2456625.278 | 16.536 0.002 | $r$ | 1m0-12 | 2013-11-03 | 2456599.677 | 16.446 0.002 | $i$ | 1m0-08 |
| 2013-11-30 | 2456626.530 | 16.606 0.002 | $r$ | 1m0-04 | 2013-11-06 | 2456602.679 | 16.507 0.003 | $i$ | 1m0-08 |
| 2013-12-01 | 2456627.529 | 16.498 0.005 | $r$ | 1m0-09 | 2013-11-10 | 2456606.660 | 16.509 0.019 | $i$ | 1m0-08 |
| 2013-12-03 | 2456629.555 | 16.572 0.021 | $r$ | 1m0-04 | 2013-11-12 | 2456608.695 | 16.486 0.002 | $i$ | 1m0-08 |
| 2013-12-04 | 2456631.290 | 16.559 0.003 | $r$ | 1m0-13 | 2013-11-15 | 2456611.703 | 16.558 0.003 | $i$ | 1m0-08 |
| 2013-12-11 | 2456637.550 | 16.582 0.005 | $r$ | 1m0-09 | 2013-11-20 | 2456616.617 | 16.529 0.005 | $i$ | 1m0-08 |
| 2013-12-14 | 2456640.929 | 16.674 0.005 | $r$ | 1m0-11 | 2013-11-20 | 2456616.920 | 16.523 0.045 | $i$ | 1m0-11 |
| 2013-12-18 | 2456644.550 | 16.805 0.012 | $r$ | 1m0-08 | 2013-11-25 | 2456621.529 | 16.514 0.002 | $i$ | 1m0-09 |
| 2013-12-20 | 2456646.669 | 16.783 0.001 | $r$ | 1m0-08 | 2013-11-28 | 2456624.540 | 16.598 0.007 | $i$ | 1m0-04 |
| 2014-01-17 | 2456674.587 | 18.197 0.011 | $r$ | 1m0-08 | 2013-11-28 | 2456625.282 | 16.487 0.007 | $i$ | 1m0-12 |
| 2014-01-19 | 2456676.576 | 18.321 0.014 | $r$ | 1m0-08 | 2013-11-30 | 2456626.534 | 16.583 0.008 | $i$ | 1m0-04 |
| 2014-01-20 | 2456677.566 | 18.173 0.053 | $r$ | 1m0-08 | 2013-12-01 | 2456627.532 | 16.528 0.013 | $i$ | 1m0-09 |
| 2014-01-22 | 2456679.555 | 18.338 0.023 | $r$ | 1m0-08 | 2013-12-03 | 2456629.560 | 16.563 0.006 | $i$ | 1m0-04 |
| 2013-10-07 | 2456572.789 | 16.567 0.012 | $R$ | 1m0-08 | 2013-12-04 | 2456631.294 | 16.583 0.014 | $i$ | 1m0-13 |
| 2013-10-08 | 2456573.674 | 16.278 0.016 | $R$ | 1m0-08 | 2013-12-11 | 2456637.554 | 16.561 0.009 | $i$ | 1m0-09 |
| 2013-10-09 | 2456574.670 | 16.124 0.014 | $R$ | 1m0-08 | 2013-12-14 | 2456640.933 | 16.716 0.049 | $i$ | 1m0-11 |
| 2013-10-10 | 2456575.661 | 16.024 0.009 | $R$ | 1m0-08 | 2013-12-18 | 2456644.554 | 16.718 0.015 | $i$ | 1m0-08 |
| 2013-10-18 | 2456583.627 | 15.887 0.031 | $R$ | 1m0-08 | 2014-01-19 | 2456676.581 | 18.403 0.035 | $i$ | 1m0-08 |
| 2013-10-20 | 2456585.638 | 15.970 0.013 | $R$ | 1m0-08 | 2014-01-20 | 2456677.571 | 18.352 0.100 | $i$ | 1m0-08 |
| 2013-10-21 | 2456586.636 | 16.008 0.018 | $R$ | 1m0-08 | 2014-01-22 | 2456679.561 | 18.399 0.032 | $i$ | 1m0-08 |
| 2013-10-22 | 2456587.748 | 16.071 0.015 | $R$ | 1m0-08 | 2013-10-07 | 2456572.793 | 16.573 0.023 | $I$ | 1m0-08 |
| 2013-10-23 | 2456588.686 | 16.093 0.021 | $R$ | 1m0-08 | 2013-10-08 | 2456573.677 | 16.265 0.021 | $I$ | 1m0-08 |
| 2013-10-25 | 2456590.719 | 16.154 0.019 | $R$ | 1m0-08 | 2013-10-09 | 2456574.674 | 16.109 0.017 | $I$ | 1m0-08 |
| 2013-10-26 | 2456591.722 | 16.158 0.027 | $R$ | 1m0-08 | 2013-10-10 | 2456575.664 | 15.915 0.025 | $I$ | 1m0-08 |
| 2013-10-27 | 2456592.711 | 16.161 0.017 | $R$ | 1m0-08 | 2013-10-18 | 2456583.631 | 15.679 0.023 | $I$ | 1m0-08 |
| 2013-10-28 | 2456593.610 | 16.192 0.019 | $R$ | 1m0-08 | 2013-10-20 | 2456585.642 | 15.803 0.042 | $I$ | 1m0-08 |
| 2013-10-29 | 2456594.668 | 16.183 0.025 | $R$ | 1m0-08 | 2013-10-21 | 2456586.639 | 15.806 0.031 | $I$ | 1m0-08 |
| 2013-11-02 | 2456598.720 | 16.227 0.020 | $R$ | 1m0-08 | 2013-10-22 | 2456587.751 | 15.827 0.049 | $I$ | 1m0-08 |
| 2013-11-03 | 2456599.699 | 16.236 0.032 | $R$ | 1m0-08 | 2013-10-23 | 2456588.690 | 15.929 0.037 | $I$ | 1m0-08 |
| 2013-11-06 | 2456602.612 | 16.240 0.016 | $R$ | 1m0-08 | 2013-10-26 | 2456591.725 | 15.960 0.011 | $I$ | 1m0-08 |
| 2013-11-10 | 2456606.691 | 16.280 0.011 | $R$ | 1m0-08 | 2013-10-27 | 2456592.714 | 15.955 0.016 | $I$ | 1m0-08 |
| 2013-11-20 | 2456616.690 | 16.307 0.011 | $R$ | 1m0-08 | 2013-10-28 | 2456593.613 | 15.996 0.015 | $I$ | 1m0-08 |
| 2013-11-21 | 2456617.541 | 16.314 0.015 | $R$ | 1m0-05 | 2013-10-29 | 2456594.671 | 16.006 0.020 | $I$ | 1m0-08 |
| 2013-12-03 | 2456629.563 | 16.373 0.021 | $R$ | 1m0-09 | 2013-11-02 | 2456598.723 | 16.043 0.021 | $I$ | 1m0-08 |
| 2013-12-05 | 2456631.558 | 16.400 0.017 | $R$ | 1m0-09 | 2013-11-03 | 2456599.702 | 16.046 0.015 | $I$ | 1m0-08 |
| 2013-12-11 | 2456637.562 | 16.535 0.011 | $R$ | 1m0-04 | 2013-11-06 | 2456602.616 | 16.070 0.012 | $I$ | 1m0-08 |
| 2013-12-14 | 2456640.673 | 16.548 0.024 | $R$ | 1m0-08 | 2013-11-10 | 2456606.695 | 16.064 0.015 | $I$ | 1m0-08 |
| 2013-12-17 | 2456643.619 | 16.456 0.037 | $R$ | 1m0-08 | 2013-11-20 | 2456616.694 | 16.123 0.036 | $I$ | 1m0-08 |
| 2013-12-20 | 2456646.649 | 16.570 0.021 | $R$ | 1m0-08 | 2013-11-21 | 2456617.545 | 16.080 0.027 | $I$ | 1m0-05 |
| 2013-12-22 | 2456648.624 | 16.741 0.025 | $R$ | 1m0-08 | 2013-12-03 | 2456629.566 | 16.114 0.017 | $I$ | 1m0-09 |
| 2013-12-23 | 2456649.633 | 16.812 0.019 | $R$ | 1m0-08 | 2013-12-05 | 2456631.562 | 16.172 0.037 | $I$ | 1m0-09 |
| 2014-01-01 | 2456658.580 | 17.560 0.038 | $R$ | 1m0-08 | 2013-12-11 | 2456637.566 | 16.248 0.018 | $I$ | 1m0-04 |
| 2014-01-07 | 2456664.553 | 17.948 0.011 | $R$ | 1m0-08 | 2013-12-14 | 2456640.677 | 16.230 0.032 | $I$ | 1m0-08 |
| 2014-01-15 | 2456672.556 | 18.122 0.056 | $R$ | 1m0-08 | 2013-12-17 | 2456643.623 | 16.054 0.012 | $I$ | 1m0-08 |

(a) Data have not been corrected for extinction
(b) *Swift* Telescope; LSQ (La Silla Quest, Chile); 1m0-08 (McDonald Observatory, USA); 1m0-10, 1m0-12, 1m0-13 (Sutherland, South Africa), 1m0-04, 1m0-05, 1m0-09 (Cerro Tololo, Chile); 1m0-03, 1m0-11 (Siding Spring, Australia).

**Table D1:** SN 2013fs: Photometric Data

| Date | JD | mag[(a)] | Filter | telescope[(b)] | Date | JD | mag[(a)] | Filter | telescope[(b)] |
|---|---|---|---|---|---|---|---|---|---|
| 2013-12-22 | 2456648.628 | 16.343 0.054 | $I$ | 1m0-08 | 2013-10-29 | 2456594.623 | 16.415 0.001 | $z$ | 1m0-08 |
| 2013-12-23 | 2456649.637 | 16.491 0.034 | $I$ | 1m0-08 | 2013-11-02 | 2456598.691 | 16.481 0.004 | $z$ | 1m0-08 |
| 2014-01-01 | 2456658.583 | 16.883 0.046 | $I$ | 1m0-08 | 2013-11-03 | 2456599.680 | 16.434 0.021 | $z$ | 1m0-08 |
| 2014-01-07 | 2456664.557 | 17.575 0.138 | $I$ | 1m0-08 | 2013-11-06 | 2456602.683 | 16.473 0.006 | $z$ | 1m0-08 |
| 2014-01-15 | 2456672.560 | 17.596 0.104 | $I$ | 1m0-08 | 2013-11-10 | 2456606.664 | 16.481 0.004 | $z$ | 1m0-08 |
| 2014-01-17 | 2456674.596 | 17.576 0.102 | $I$ | 1m0-08 | 2013-11-12 | 2456608.699 | 16.482 0.007 | $z$ | 1m0-08 |
| 2013-10-07 | 2456572.650 | 17.282 0.009 | $z$ | 1m0-08 | 2013-11-15 | 2456611.707 | 16.571 0.037 | $z$ | 1m0-08 |
| 2013-10-08 | 2456573.739 | 16.796 0.000 | $z$ | 1m0-08 | 2013-11-20 | 2456616.621 | 16.553 0.026 | $z$ | 1m0-08 |
| 2013-10-09 | 2456574.710 | 16.589 0.015 | $z$ | 1m0-08 | 2013-11-25 | 2456621.534 | 16.524 0.006 | $z$ | 1m0-09 |
| 2013-10-11 | 2456576.772 | 16.307 0.026 | $z$ | 1m0-08 | 2013-11-28 | 2456624.545 | 16.527 0.024 | $z$ | 1m0-04 |
| 2013-10-12 | 2456577.772 | 16.208 0.024 | $z$ | 1m0-08 | 2013-11-28 | 2456625.287 | 16.492 0.037 | $z$ | 1m0-12 |
| 2013-10-18 | 2456583.648 | 16.117 0.000 | $z$ | 1m0-08 | 2013-11-30 | 2456626.539 | 16.538 0.027 | $z$ | 1m0-04 |
| 2013-10-20 | 2456585.611 | 16.172 0.002 | $z$ | 1m0-08 | 2013-12-01 | 2456627.538 | 16.511 0.000 | $z$ | 1m0-09 |
| 2013-10-21 | 2456586.608 | 16.203 0.010 | $z$ | 1m0-08 | 2013-12-03 | 2456629.565 | 16.600 0.028 | $z$ | 1m0-04 |
| 2013-10-22 | 2456587.719 | 16.263 0.019 | $z$ | 1m0-08 | 2013-12-04 | 2456631.299 | 16.522 0.027 | $z$ | 1m0-13 |
| 2013-10-23 | 2456588.747 | 16.306 0.025 | $z$ | 1m0-08 | 2013-12-11 | 2456637.559 | 16.526 0.011 | $z$ | 1m0-09 |
| 2013-10-26 | 2456591.609 | 16.368 0.018 | $z$ | 1m0-08 | 2013-12-14 | 2456640.938 | 16.750 0.026 | $z$ | 1m0-11 |
| 2013-10-27 | 2456592.597 | 16.392 0.004 | $z$ | 1m0-08 | 2013-12-18 | 2456644.558 | 16.190 0.310 | $z$ | 1m0-08 |
| 2013-10-28 | 2456593.642 | 16.374 0.014 | $z$ | 1m0-08 | 2013-12-20 | 2456646.677 | 17.019 0.050 | $z$ | 1m0-08 |

(a) Data have not been corrected for extinction
(b) *Swift* Telescope; LSQ (La Silla Quest, Chile); 1m0-08 (McDonald Observatory, USA); 1m0-10, 1m0-12, 1m0-13 (Sutherland, South Africa), 1m0-04, 1m0-05, 1m0-09 (Cerro Tololo, Chile); 1m0-03, 1m0-11 (Siding Spring, Australia).

**Table D1:** SN 2013bu: Photometric Data

| Date | JD | mag$^{(a)}$ | Filter | telescope$^{(b)}$ |
|---|---|---|---|---|
| 2013-04-21 | 2456404.259 | 16.600 0.000 | $B$ | Atel/CBAT |
| 2013-04-23 | 2456405.952 | 16.503 0.024 | $B$ | 1m0-08 |
| 2013-04-30 | 2456412.952 | 16.622 0.027 | $B$ | 1m0-08 |
| 2013-04-30 | 2456412.954 | 16.674 0.024 | $B$ | 1m0-08 |
| 2013-05-06 | 2456418.949 | 16.954 0.023 | $B$ | 1m0-08 |
| 2013-05-08 | 2456420.949 | 17.006 0.021 | $B$ | 1m0-08 |
| 2013-05-18 | 2456430.910 | 17.395 0.027 | $B$ | 1m0-08 |
| 2013-05-18 | 2456430.913 | 17.405 0.021 | $B$ | 1m0-08 |
| 2013-05-20 | 2456432.910 | 17.433 0.030 | $B$ | 1m0-08 |
| 2013-05-20 | 2456432.913 | 17.468 0.024 | $B$ | 1m0-08 |
| 2013-05-22 | 2456434.875 | 17.536 0.034 | $B$ | 1m0-08 |
| 2013-05-22 | 2456434.878 | 17.473 0.027 | $B$ | 1m0-08 |
| 2013-05-31 | 2456443.875 | 17.735 0.030 | $B$ | 1m0-08 |
| 2013-05-31 | 2456443.878 | 17.748 0.032 | $B$ | 1m0-08 |
| 2013-06-04 | 2456447.889 | 17.848 0.041 | $B$ | 1m0-08 |
| 2013-06-04 | 2456447.892 | 17.707 0.039 | $B$ | 1m0-08 |
| 2013-06-10 | 2456453.896 | 17.820 0.033 | $B$ | 1m0-08 |
| 2013-06-10 | 2456453.899 | 17.904 0.047 | $B$ | 1m0-08 |
| 2013-06-11 | 2456454.896 | 17.946 0.044 | $B$ | 1m0-08 |
| 2013-06-11 | 2456454.899 | 17.958 0.052 | $B$ | 1m0-08 |
| 2013-06-13 | 2456456.896 | 17.934 0.046 | $B$ | 1m0-08 |
| 2013-06-13 | 2456456.899 | 17.901 0.028 | $B$ | 1m0-08 |
| 2013-06-15 | 2456458.891 | 17.820 0.037 | $B$ | 1m0-08 |
| 2013-06-16 | 2456459.886 | 17.911 0.050 | $B$ | 1m0-08 |
| 2013-06-16 | 2456459.889 | 17.931 0.032 | $B$ | 1m0-08 |
| 2013-06-17 | 2456460.893 | 17.752 0.039 | $B$ | 1m0-08 |
| 2013-06-17 | 2456460.896 | 17.799 0.040 | $B$ | 1m0-08 |
| 2013-06-18 | 2456461.889 | 17.969 0.045 | $B$ | 1m0-08 |
| 2013-06-19 | 2456462.886 | 17.948 0.033 | $B$ | 1m0-08 |
| 2013-06-19 | 2456462.889 | 17.931 0.043 | $B$ | 1m0-08 |
| 2013-07-04 | 2456477.851 | 18.265 0.051 | $B$ | 1m0-08 |
| 2013-07-04 | 2456477.853 | 18.363 0.079 | $B$ | 1m0-08 |
| 2013-07-05 | 2456478.851 | 18.300 0.067 | $B$ | 1m0-08 |
| 2013-07-05 | 2456478.853 | 18.338 0.047 | $B$ | 1m0-08 |
| 2013-07-07 | 2456480.851 | 18.284 0.060 | $B$ | 1m0-08 |
| 2013-07-07 | 2456480.853 | 18.336 0.042 | $B$ | 1m0-08 |
| 2013-07-08 | 2456481.834 | 18.392 0.042 | $B$ | 1m0-08 |
| 2013-07-08 | 2456481.835 | 18.413 0.076 | $B$ | 1m0-08 |
| 2013-07-12 | 2456485.834 | 18.504 0.048 | $B$ | 1m0-08 |
| 2013-07-12 | 2456485.835 | 18.532 0.058 | $B$ | 1m0-08 |
| 2013-07-14 | 2456487.834 | 18.696 0.099 | $B$ | 1m0-08 |
| 2013-07-14 | 2456487.835 | 18.650 0.066 | $B$ | 1m0-08 |
| 2013-07-25 | 2456498.884 | 19.381 0.113 | $B$ | 1m0-08 |
| 2013-07-25 | 2456498.886 | 19.109 0.102 | $B$ | 1m0-08 |
| 2013-08-01 | 2456505.806 | 20.057 0.324 | $B$ | 1m0-08 |
| 2013-08-01 | 2456505.808 | 20.032 0.306 | $B$ | 1m0-08 |
| 2013-08-02 | 2456506.865 | 20.081 0.203 | $B$ | 1m0-08 |
| 2013-08-02 | 2456506.866 | 20.156 0.221 | $B$ | 1m0-08 |
| 2013-08-04 | 2456508.923 | 20.563 0.342 | $B$ | 1m0-08 |
| 2013-08-06 | 2456510.903 | 20.923 0.427 | $B$ | 1m0-08 |
| 2013-08-06 | 2456510.932 | 20.674 0.423 | $B$ | 1m0-08 |
| 2013-08-09 | 2456513.916 | 21.114 0.320 | $B$ | 1m0-08 |
| 2013-08-09 | 2456513.945 | 21.405 0.331 | $B$ | 1m0-08 |
| 2013-08-10 | 2456515.232 | 20.332 0.166 | $B$ | 1m0-11 |
| 2013-08-11 | 2456515.701 | 20.294 0.280 | $B$ | 1m0-08 |
| 2013-08-11 | 2456515.705 | 20.144 0.298 | $B$ | 1m0-08 |
| 2013-08-12 | 2456516.688 | 20.524 0.351 | $B$ | 1m0-08 |
| 2013-08-12 | 2456516.692 | 20.692 0.485 | $B$ | 1m0-08 |
| 2013-08-13 | 2456517.752 | $<$ 20.643 | $B$ | 1m0-08 |
| 2013-08-13 | 2456517.756 | $<$ 20.624 | $B$ | 1m0-08 |
| 2013-08-15 | 2456519.708 | $<$ 20.136 | $B$ | 1m0-08 |
| 2013-08-15 | 2456519.712 | $<$ 20.342 | $B$ | 1m0-08 |
| 2013-04-23 | 2456405.958 | 16.034 0.021 | $g$ | 1m0-08 |
| 2013-04-23 | 2456405.960 | 15.988 0.025 | $g$ | 1m0-08 |
| 2013-04-26 | 2456408.958 | 16.268 0.054 | $g$ | 1m0-08 |
| 2013-04-26 | 2456408.959 | 16.308 0.047 | $g$ | 1m0-08 |
| 2013-04-29 | 2456411.960 | 16.139 0.041 | $g$ | 1m0-08 |
| 2013-04-30 | 2456412.958 | 16.170 0.028 | $g$ | 1m0-08 |
| 2013-04-30 | 2456412.960 | 16.228 0.037 | $g$ | 1m0-08 |
| 2013-05-08 | 2456420.953 | 16.358 0.031 | $g$ | 1m0-08 |
| 2013-05-08 | 2456420.955 | 16.330 0.036 | $g$ | 1m0-08 |
| 2013-05-16 | 2456428.917 | 16.495 0.021 | $g$ | 1m0-08 |
| 2013-05-16 | 2456428.921 | 16.501 0.017 | $g$ | 1m0-08 |
| 2013-05-18 | 2456430.920 | 16.547 0.035 | $g$ | 1m0-08 |
| 2013-05-18 | 2456430.923 | 16.540 0.035 | $g$ | 1m0-08 |
| 2013-05-20 | 2456432.920 | 16.559 0.017 | $g$ | 1m0-08 |
| 2013-05-20 | 2456432.923 | 16.585 0.016 | $g$ | 1m0-08 |
| 2013-05-22 | 2456434.885 | 16.660 0.015 | $g$ | 1m0-08 |
| 2013-05-22 | 2456434.888 | 16.598 0.015 | $g$ | 1m0-08 |
| 2013-05-31 | 2456443.885 | 16.665 0.015 | $g$ | 1m0-08 |
| 2013-05-31 | 2456443.888 | 16.679 0.012 | $g$ | 1m0-08 |
| 2013-06-04 | 2456447.899 | 16.698 0.016 | $g$ | 1m0-08 |
| 2013-06-04 | 2456447.902 | 16.699 0.016 | $g$ | 1m0-08 |
| 2013-06-10 | 2456453.906 | 16.756 0.013 | $g$ | 1m0-08 |
| 2013-06-10 | 2456453.909 | 16.777 0.015 | $g$ | 1m0-08 |
| 2013-06-11 | 2456454.906 | 16.747 0.042 | $g$ | 1m0-08 |
| 2013-06-11 | 2456454.910 | 16.773 0.043 | $g$ | 1m0-08 |
| 2013-06-13 | 2456456.906 | 16.801 0.015 | $g$ | 1m0-08 |
| 2013-06-13 | 2456456.909 | 16.820 0.015 | $g$ | 1m0-08 |
| 2013-06-16 | 2456459.896 | 16.807 0.013 | $g$ | 1m0-08 |
| 2013-06-16 | 2456459.899 | 16.811 0.013 | $g$ | 1m0-08 |
| 2013-06-18 | 2456461.896 | 16.778 0.030 | $g$ | 1m0-08 |
| 2013-06-18 | 2456461.899 | 16.780 0.024 | $g$ | 1m0-08 |
| 2013-06-19 | 2456462.896 | 16.862 0.017 | $g$ | 1m0-08 |
| 2013-06-19 | 2456462.899 | 16.862 0.014 | $g$ | 1m0-08 |
| 2013-07-04 | 2456477.857 | 17.073 0.023 | $g$ | 1m0-08 |
| 2013-07-04 | 2456477.859 | 17.109 0.029 | $g$ | 1m0-08 |
| 2013-07-05 | 2456478.857 | 17.120 0.020 | $g$ | 1m0-08 |
| 2013-07-05 | 2456478.858 | 17.110 0.018 | $g$ | 1m0-08 |
| 2013-07-07 | 2456480.857 | 17.171 0.012 | $g$ | 1m0-08 |
| 2013-07-07 | 2456480.859 | 17.149 0.015 | $g$ | 1m0-08 |
| 2013-07-08 | 2456481.839 | 17.230 0.025 | $g$ | 1m0-08 |
| 2013-07-08 | 2456481.841 | 17.188 0.019 | $g$ | 1m0-08 |
| 2013-07-12 | 2456485.840 | 17.350 0.024 | $g$ | 1m0-08 |
| 2013-07-12 | 2456485.841 | 17.342 0.019 | $g$ | 1m0-08 |
| 2013-07-14 | 2456487.839 | 17.412 0.020 | $g$ | 1m0-08 |
| 2013-07-14 | 2456487.841 | 17.460 0.017 | $g$ | 1m0-08 |
| 2013-07-25 | 2456498.890 | 18.378 0.052 | $g$ | 1m0-08 |
| 2013-07-25 | 2456498.892 | 18.275 0.032 | $g$ | 1m0-08 |
| 2013-08-01 | 2456505.811 | 19.700 0.099 | $g$ | 1m0-08 |
| 2013-08-01 | 2456505.813 | 19.693 0.120 | $g$ | 1m0-08 |
| 2013-08-02 | 2456506.870 | 20.554 0.232 | $g$ | 1m0-08 |
| 2013-08-02 | 2456506.872 | 20.216 0.169 | $g$ | 1m0-08 |
| 2013-08-06 | 2456510.887 | 20.796 0.338 | $g$ | 1m0-08 |
| 2013-08-06 | 2456510.891 | 20.689 0.237 | $g$ | 1m0-08 |
| 2013-08-09 | 2456513.924 | 20.918 0.394 | $g$ | 1m0-08 |
| 2013-08-09 | 2456513.957 | 21.053 0.462 | $g$ | 1m0-08 |
| 2013-08-10 | 2456515.244 | 21.405 0.366 | $g$ | 1m0-11 |
| 2013-08-11 | 2456515.716 | 21.136 0.344 | $g$ | 1m0-08 |
| 2013-08-12 | 2456516.700 | 20.965 0.280 | $g$ | 1m0-08 |

(a) Data have not been corrected for extinction
(b) *Swift* Telescope; LSQ (La Silla Quest, Chile); 1m0-08 (McDonald Observatory, USA); 1m0-10, 1m0-12, 1m0-13 (Sutherland, South Africa), 1m0-04, 1m0-05, 1m0-09 (Cerro Tololo, Chile); 1m0-03, 1m0-11 (Siding Spring, Australia).

**Table D1:** SN 2013bu: Photometric Data

| Date | JD | mag[(a)] | Filter | telescope[(b)] | Date | JD | mag[(a)] | Filter | telescope[(b)] |
|---|---|---|---|---|---|---|---|---|---|
| 2013-08-12 | 2456516.703 | 20.977 0.268 | *g* | 1m0-08 | 2013-07-12 | 2456485.838 | 17.088 0.017 | *V* | 1m0-08 |
| 2013-08-13 | 2456517.793 | 21.314 0.312 | *g* | 1m0-08 | 2013-07-14 | 2456487.837 | 17.399 0.040 | *V* | 1m0-08 |
| 2013-08-13 | 2456517.797 | 21.420 0.355 | *g* | 1m0-08 | 2013-07-14 | 2456487.838 | 17.166 0.021 | *V* | 1m0-08 |
| 2013-08-13 | 2456517.813 | 21.515 0.425 | *g* | 1m0-08 | 2013-07-25 | 2456498.888 | 17.866 0.032 | *V* | 1m0-08 |
| 2013-08-13 | 2456517.817 | 21.358 0.377 | *g* | 1m0-08 | 2013-07-25 | 2456498.889 | 17.855 0.033 | *V* | 1m0-08 |
| 2013-08-15 | 2456519.722 | 21.174 0.410 | *g* | 1m0-08 | 2013-08-01 | 2456505.809 | 19.178 0.100 | *V* | 1m0-08 |
| 2013-08-15 | 2456519.787 | 21.201 0.426 | *g* | 1m0-08 | 2013-08-01 | 2456505.810 | 19.314 0.115 | *V* | 1m0-08 |
| 2013-08-15 | 2456519.791 | 21.130 0.393 | *g* | 1m0-08 | 2013-08-02 | 2456506.868 | 19.365 0.118 | *V* | 1m0-08 |
| 2013-08-15 | 2456519.947 | 21.412 0.446 | *g* | 1m0-08 | 2013-08-02 | 2456506.869 | 19.497 0.110 | *V* | 1m0-08 |
| 2013-08-15 | 2456519.957 | 21.172 0.304 | *g* | 1m0-08 | 2013-08-03 | 2456507.946 | 20.266 0.190 | *V* | 1m0-08 |
| 2013-08-22 | 2456526.834 | 21.148 0.204 | *g* | 1m0-08 | 2013-08-04 | 2456508.962 | 20.160 0.207 | *V* | 1m0-08 |
| 2013-08-22 | 2456526.873 | 21.344 0.363 | *g* | 1m0-08 | 2013-08-04 | 2456508.964 | 20.113 0.209 | *V* | 1m0-08 |
| 2013-08-22 | 2456526.878 | 21.227 0.344 | *g* | 1m0-08 | 2013-08-06 | 2456510.885 | 20.504 0.141 | *V* | 1m0-08 |
| 2013-08-29 | 2456533.870 | 21.038 0.367 | *g* | 1m0-08 | 2013-08-09 | 2456513.949 | 20.544 0.135 | *V* | 1m0-08 |
| 2013-08-29 | 2456533.875 | 21.276 0.493 | *g* | 1m0-08 | 2013-08-11 | 2456515.708 | 19.948 0.177 | *V* | 1m0-08 |
| 2013-04-12 | 2456395.263 | $<$ 19.000 | *V* | Atel/CBAT | 2013-08-11 | 2456515.710 | 20.130 0.203 | *V* | 1m0-08 |
| 2013-04-23 | 2456405.955 | 16.294 0.014 | *V* | 1m0-08 | 2013-08-12 | 2456516.696 | 20.065 0.219 | *V* | 1m0-08 |
| 2013-04-23 | 2456405.957 | 16.237 0.013 | *V* | 1m0-08 | 2013-08-12 | 2456516.698 | 20.145 0.218 | *V* | 1m0-08 |
| 2013-04-26 | 2456408.955 | 16.401 0.030 | *V* | 1m0-08 | 2013-08-13 | 2456517.761 | $<$ 20.206 | *V* | 1m0-08 |
| 2013-04-27 | 2456409.955 | 16.473 0.021 | *V* | 1m0-08 | 2013-08-13 | 2456517.763 | $<$ 20.050 | *V* | 1m0-08 |
| 2013-04-27 | 2456409.957 | 16.558 0.036 | *V* | 1m0-08 | 2013-08-15 | 2456519.717 | $<$ 19.969 | *V* | 1m0-08 |
| 2013-04-29 | 2456411.956 | 16.407 0.022 | *V* | 1m0-08 | 2013-08-15 | 2456519.719 | $<$ 20.191 | *V* | 1m0-08 |
| 2013-04-29 | 2456411.957 | 16.512 0.023 | *V* | 1m0-08 | 2013-04-23 | 2456405.961 | 15.547 0.014 | *r* | 1m0-08 |
| 2013-04-30 | 2456412.956 | 16.352 0.021 | *V* | 1m0-08 | 2013-04-23 | 2456405.963 | 15.597 0.015 | *r* | 1m0-08 |
| 2013-04-30 | 2456412.957 | 16.316 0.017 | *V* | 1m0-08 | 2013-04-26 | 2456408.961 | 15.574 0.032 | *r* | 1m0-08 |
| 2013-05-06 | 2456418.952 | 16.356 0.022 | *V* | 1m0-08 | 2013-04-26 | 2456408.962 | 15.653 0.034 | *r* | 1m0-08 |
| 2013-05-06 | 2456418.954 | 16.428 0.019 | *V* | 1m0-08 | 2013-04-27 | 2456409.961 | 15.775 0.059 | *r* | 1m0-08 |
| 2013-05-08 | 2456420.951 | 16.384 0.015 | *V* | 1m0-08 | 2013-04-29 | 2456411.962 | 15.628 0.022 | *r* | 1m0-08 |
| 2013-05-08 | 2456420.952 | 16.360 0.015 | *V* | 1m0-08 | 2013-04-29 | 2456411.964 | 15.603 0.017 | *r* | 1m0-08 |
| 2013-05-15 | 2456427.953 | 16.599 0.027 | *V* | 1m0-08 | 2013-04-30 | 2456412.961 | 15.576 0.034 | *r* | 1m0-08 |
| 2013-05-15 | 2456427.954 | 16.669 0.025 | *V* | 1m0-08 | 2013-04-30 | 2456412.962 | 15.585 0.027 | *r* | 1m0-08 |
| 2013-05-18 | 2456430.917 | 16.478 0.011 | *V* | 1m0-08 | 2013-05-08 | 2456420.957 | 15.584 0.027 | *r* | 1m0-08 |
| 2013-05-18 | 2456430.918 | 16.474 0.015 | *V* | 1m0-08 | 2013-05-08 | 2456420.958 | 15.596 0.023 | *r* | 1m0-08 |
| 2013-05-20 | 2456432.917 | 16.500 0.011 | *V* | 1m0-08 | 2013-05-15 | 2456427.960 | 15.643 0.033 | *r* | 1m0-08 |
| 2013-05-20 | 2456432.918 | 16.497 0.015 | *V* | 1m0-08 | 2013-05-15 | 2456427.962 | 15.740 0.027 | *r* | 1m0-08 |
| 2013-05-22 | 2456434.882 | 16.420 0.015 | *V* | 1m0-08 | 2013-05-16 | 2456428.924 | 15.674 0.011 | *r* | 1m0-08 |
| 2013-05-22 | 2456434.884 | 16.532 0.016 | *V* | 1m0-08 | 2013-05-16 | 2456428.927 | 15.657 0.010 | *r* | 1m0-08 |
| 2013-05-31 | 2456443.882 | 16.613 0.028 | *V* | 1m0-08 | 2013-05-18 | 2456430.927 | 15.661 0.023 | *r* | 1m0-08 |
| 2013-05-31 | 2456443.883 | 16.541 0.012 | *V* | 1m0-08 | 2013-05-18 | 2456430.928 | 15.663 0.018 | *r* | 1m0-08 |
| 2013-06-04 | 2456447.896 | 16.549 0.015 | *V* | 1m0-08 | 2013-05-20 | 2456432.926 | 15.711 0.010 | *r* | 1m0-08 |
| 2013-06-04 | 2456447.897 | 16.587 0.013 | *V* | 1m0-08 | 2013-05-20 | 2456432.928 | 15.651 0.009 | *r* | 1m0-08 |
| 2013-06-10 | 2456453.903 | 16.593 0.016 | *V* | 1m0-08 | 2013-05-22 | 2456434.892 | 15.690 0.009 | *r* | 1m0-08 |
| 2013-06-10 | 2456453.904 | 16.566 0.011 | *V* | 1m0-08 | 2013-05-22 | 2456434.894 | 15.680 0.013 | *r* | 1m0-08 |
| 2013-06-11 | 2456454.903 | 16.569 0.014 | *V* | 1m0-08 | 2013-05-31 | 2456443.892 | 15.665 0.010 | *r* | 1m0-08 |
| 2013-06-11 | 2456454.904 | 16.595 0.015 | *V* | 1m0-08 | 2013-05-31 | 2456443.893 | 15.668 0.009 | *r* | 1m0-08 |
| 2013-06-13 | 2456456.904 | 16.578 0.013 | *V* | 1m0-08 | 2013-06-04 | 2456447.906 | 15.664 0.011 | *r* | 1m0-08 |
| 2013-06-16 | 2456459.892 | 16.607 0.014 | *V* | 1m0-08 | 2013-06-04 | 2456447.907 | 15.661 0.012 | *r* | 1m0-08 |
| 2013-06-16 | 2456459.894 | 16.622 0.011 | *V* | 1m0-08 | 2013-06-10 | 2456453.913 | 15.662 0.011 | *r* | 1m0-08 |
| 2013-06-18 | 2456461.892 | 16.622 0.014 | *V* | 1m0-08 | 2013-06-10 | 2456453.914 | 15.667 0.010 | *r* | 1m0-08 |
| 2013-06-18 | 2456461.894 | 16.588 0.019 | *V* | 1m0-08 | 2013-06-11 | 2456454.913 | 15.644 0.046 | *r* | 1m0-08 |
| 2013-06-19 | 2456462.892 | 16.631 0.014 | *V* | 1m0-08 | 2013-06-11 | 2456454.915 | 15.670 0.025 | *r* | 1m0-08 |
| 2013-07-04 | 2456477.855 | 16.887 0.016 | *V* | 1m0-08 | 2013-06-13 | 2456456.913 | 15.691 0.012 | *r* | 1m0-08 |
| 2013-07-04 | 2456477.856 | 16.823 0.015 | *V* | 1m0-08 | 2013-06-13 | 2456456.914 | 15.709 0.011 | *r* | 1m0-08 |
| 2013-07-05 | 2456478.855 | 16.828 0.017 | *V* | 1m0-08 | 2013-06-16 | 2456459.902 | 15.699 0.010 | *r* | 1m0-08 |
| 2013-07-05 | 2456478.856 | 16.841 0.016 | *V* | 1m0-08 | 2013-06-16 | 2456459.904 | 15.695 0.010 | *r* | 1m0-08 |
| 2013-07-07 | 2456480.855 | 16.901 0.014 | *V* | 1m0-08 | 2013-06-18 | 2456461.902 | 15.677 0.014 | *r* | 1m0-08 |
| 2013-07-07 | 2456480.856 | 16.893 0.021 | *V* | 1m0-08 | 2013-06-18 | 2456461.904 | 15.679 0.014 | *r* | 1m0-08 |
| 2013-07-08 | 2456481.837 | 16.993 0.017 | *V* | 1m0-08 | 2013-06-19 | 2456462.902 | 15.711 0.010 | *r* | 1m0-08 |
| 2013-07-08 | 2456481.838 | 16.973 0.018 | *V* | 1m0-08 | 2013-06-19 | 2456462.904 | 15.724 0.010 | *r* | 1m0-08 |
| 2013-07-12 | 2456485.837 | 17.252 0.025 | *V* | 1m0-08 | 2013-07-04 | 2456477.860 | 15.861 0.013 | *r* | 1m0-08 |

(a) Data have not been corrected for extinction
(b) *Swift* Telescope; LSQ (La Silla Quest, Chile); 1m0-08 (McDonald Observatory, USA); 1m0-10, 1m0-12, 1m0-13 (Sutherland, South Africa), 1m0-04, 1m0-05, 1m0-09 (Cerro Tololo, Chile); 1m0-03, 1m0-11 (Siding Spring, Australia).

**Table D1:** SN 2013bu: Photometric Data

| Date | JD | mag$^{(a)}$ | Filter | telescope$^{(b)}$ | Date | JD | mag$^{(a)}$ | Filter | telescope$^{(b)}$ |
|---|---|---|---|---|---|---|---|---|---|
| 2013-07-04 | 2456477.862 | 15.843 0.019 | $r$ | 1m0-08 | 2013-05-20 | 2456432.932 | 15.556 0.008 | $i$ | 1m0-08 |
| 2013-07-05 | 2456478.860 | 15.881 0.012 | $r$ | 1m0-08 | 2013-05-22 | 2456434.895 | 15.579 0.009 | $i$ | 1m0-08 |
| 2013-07-05 | 2456478.861 | 15.876 0.012 | $r$ | 1m0-08 | 2013-05-22 | 2456434.897 | 15.529 0.008 | $i$ | 1m0-08 |
| 2013-07-07 | 2456480.860 | 15.935 0.009 | $r$ | 1m0-08 | 2013-05-31 | 2456443.895 | 15.493 0.007 | $i$ | 1m0-08 |
| 2013-07-07 | 2456480.861 | 15.914 0.010 | $r$ | 1m0-08 | 2013-05-31 | 2456443.897 | 15.483 0.008 | $i$ | 1m0-08 |
| 2013-07-08 | 2456481.843 | 15.936 0.013 | $r$ | 1m0-08 | 2013-06-04 | 2456447.909 | 15.509 0.009 | $i$ | 1m0-08 |
| 2013-07-08 | 2456481.844 | 15.935 0.014 | $r$ | 1m0-08 | 2013-06-04 | 2456447.911 | 15.498 0.008 | $i$ | 1m0-08 |
| 2013-07-12 | 2456485.843 | 16.072 0.013 | $r$ | 1m0-08 | 2013-06-10 | 2456453.916 | 15.476 0.007 | $i$ | 1m0-08 |
| 2013-07-12 | 2456485.844 | 16.060 0.012 | $r$ | 1m0-08 | 2013-06-10 | 2456453.918 | 15.487 0.008 | $i$ | 1m0-08 |
| 2013-07-14 | 2456487.843 | 16.141 0.012 | $r$ | 1m0-08 | 2013-06-11 | 2456454.916 | 15.472 0.015 | $i$ | 1m0-08 |
| 2013-07-14 | 2456487.844 | 16.142 0.013 | $r$ | 1m0-08 | 2013-06-11 | 2456454.918 | 15.468 0.018 | $i$ | 1m0-08 |
| 2013-07-25 | 2456498.893 | 16.779 0.019 | $r$ | 1m0-08 | 2013-06-13 | 2456456.916 | 15.495 0.008 | $i$ | 1m0-08 |
| 2013-07-25 | 2456498.895 | 16.833 0.017 | $r$ | 1m0-08 | 2013-06-13 | 2456456.918 | 15.505 0.008 | $i$ | 1m0-08 |
| 2013-08-01 | 2456505.814 | 18.008 0.048 | $r$ | 1m0-08 | 2013-06-16 | 2456459.906 | 15.490 0.006 | $i$ | 1m0-08 |
| 2013-08-01 | 2456505.815 | 17.972 0.046 | $r$ | 1m0-08 | 2013-06-16 | 2456459.908 | 15.487 0.007 | $i$ | 1m0-08 |
| 2013-08-02 | 2456506.873 | 18.375 0.053 | $r$ | 1m0-08 | 2013-06-18 | 2456461.906 | 15.513 0.007 | $i$ | 1m0-08 |
| 2013-08-02 | 2456506.874 | 18.355 0.053 | $r$ | 1m0-08 | 2013-06-18 | 2456461.908 | 15.484 0.009 | $i$ | 1m0-08 |
| 2013-08-06 | 2456510.895 | 19.799 0.181 | $r$ | 1m0-08 | 2013-06-19 | 2456462.906 | 15.509 0.007 | $i$ | 1m0-08 |
| 2013-08-06 | 2456510.897 | 19.576 0.163 | $r$ | 1m0-08 | 2013-06-19 | 2456462.908 | 15.516 0.009 | $i$ | 1m0-08 |
| 2013-08-06 | 2456510.923 | 19.712 0.180 | $r$ | 1m0-08 | 2013-07-04 | 2456477.863 | 15.646 0.014 | $i$ | 1m0-08 |
| 2013-08-06 | 2456510.925 | 19.862 0.241 | $r$ | 1m0-08 | 2013-07-04 | 2456477.864 | 15.651 0.010 | $i$ | 1m0-08 |
| 2013-08-06 | 2456510.951 | 19.914 0.280 | $r$ | 1m0-08 | 2013-07-05 | 2456478.863 | 15.685 0.009 | $i$ | 1m0-08 |
| 2013-08-06 | 2456510.954 | 19.867 0.218 | $r$ | 1m0-08 | 2013-07-05 | 2456478.864 | 15.667 0.010 | $i$ | 1m0-08 |
| 2013-08-09 | 2456513.932 | 19.874 0.280 | $r$ | 1m0-08 | 2013-07-07 | 2456480.863 | 15.714 0.008 | $i$ | 1m0-08 |
| 2013-08-09 | 2456513.934 | 19.992 0.251 | $r$ | 1m0-08 | 2013-07-07 | 2456480.864 | 15.718 0.009 | $i$ | 1m0-08 |
| 2013-08-09 | 2456513.961 | 19.607 0.183 | $r$ | 1m0-08 | 2013-07-08 | 2456481.845 | 15.714 0.010 | $i$ | 1m0-08 |
| 2013-08-09 | 2456513.963 | 19.618 0.180 | $r$ | 1m0-08 | 2013-07-08 | 2456481.846 | 15.732 0.009 | $i$ | 1m0-08 |
| 2013-08-11 | 2456515.720 | 19.137 0.126 | $r$ | 1m0-08 | 2013-07-12 | 2456485.845 | 15.878 0.010 | $i$ | 1m0-08 |
| 2013-08-11 | 2456515.722 | $<$ 18.961 | $r$ | 1m0-08 | 2013-07-12 | 2456485.846 | 15.866 0.011 | $i$ | 1m0-08 |
| 2013-08-12 | 2456516.707 | 19.195 0.101 | $r$ | 1m0-08 | 2013-07-14 | 2456487.845 | 16.070 0.015 | $i$ | 1m0-08 |
| 2013-08-12 | 2456516.709 | 19.110 0.094 | $r$ | 1m0-08 | 2013-07-14 | 2456487.846 | 15.948 0.010 | $i$ | 1m0-08 |
| 2013-08-13 | 2456517.802 | $<$ 19.167 | $r$ | 1m0-08 | 2013-07-25 | 2456498.896 | 16.595 0.018 | $i$ | 1m0-08 |
| 2013-08-13 | 2456517.804 | $<$ 19.088 | $r$ | 1m0-08 | 2013-07-25 | 2456498.897 | 16.567 0.012 | $i$ | 1m0-08 |
| 2013-08-13 | 2456517.822 | $<$ 19.310 | $r$ | 1m0-08 | 2013-08-01 | 2456505.816 | 17.778 0.043 | $i$ | 1m0-08 |
| 2013-08-13 | 2456517.824 | $<$ 19.201 | $r$ | 1m0-08 | 2013-08-01 | 2456505.817 | 17.872 0.046 | $i$ | 1m0-08 |
| 2013-08-15 | 2456519.736 | $<$ 19.286 | $r$ | 1m0-08 | 2013-08-02 | 2456506.875 | 18.208 0.074 | $i$ | 1m0-08 |
| 2013-08-15 | 2456519.738 | $<$ 19.188 | $r$ | 1m0-08 | 2013-08-02 | 2456506.876 | 18.165 0.076 | $i$ | 1m0-08 |
| 2013-04-23 | 2456405.964 | 15.559 0.014 | $i$ | 1m0-08 | 2013-08-11 | 2456515.724 | 18.768 0.120 | $i$ | 1m0-08 |
| 2013-04-23 | 2456405.965 | 15.581 0.010 | $i$ | 1m0-08 | 2013-08-11 | 2456515.726 | 18.744 0.104 | $i$ | 1m0-08 |
| 2013-04-26 | 2456408.963 | 15.628 0.030 | $i$ | 1m0-08 | 2013-08-12 | 2456516.711 | 18.706 0.100 | $i$ | 1m0-08 |
| 2013-04-26 | 2456408.964 | 15.596 0.025 | $i$ | 1m0-08 | 2013-08-12 | 2456516.713 | 18.885 0.125 | $i$ | 1m0-08 |
| 2013-04-29 | 2456411.965 | 15.590 0.018 | $i$ | 1m0-08 | 2013-08-13 | 2456517.806 | 18.730 0.099 | $i$ | 1m0-08 |
| 2013-04-29 | 2456411.966 | 15.581 0.020 | $i$ | 1m0-08 | 2013-08-13 | 2456517.809 | 18.771 0.102 | $i$ | 1m0-08 |
| 2013-04-30 | 2456412.964 | 15.559 0.030 | $i$ | 1m0-08 | 2013-08-13 | 2456517.826 | 18.745 0.093 | $i$ | 1m0-08 |
| 2013-04-30 | 2456412.965 | 15.596 0.021 | $i$ | 1m0-08 | 2013-08-13 | 2456517.828 | 18.790 0.100 | $i$ | 1m0-08 |
| 2013-05-06 | 2456418.961 | 15.566 0.037 | $i$ | 1m0-08 | 2013-08-15 | 2456519.800 | 18.616 0.109 | $i$ | 1m0-08 |
| 2013-05-06 | 2456418.963 | 15.625 0.034 | $i$ | 1m0-08 | 2013-08-15 | 2456519.966 | 18.781 0.114 | $i$ | 1m0-08 |
| 2013-05-08 | 2456420.959 | 15.588 0.015 | $i$ | 1m0-08 | 2013-08-15 | 2456519.968 | 18.704 0.112 | $i$ | 1m0-08 |
| 2013-05-08 | 2456420.960 | 15.560 0.016 | $i$ | 1m0-08 | 2013-08-20 | 2456524.695 | 18.852 0.147 | $i$ | 1m0-08 |
| 2013-05-15 | 2456427.963 | 15.534 0.030 | $i$ | 1m0-08 | 2013-08-20 | 2456524.697 | 19.028 0.197 | $i$ | 1m0-08 |
| 2013-05-15 | 2456427.964 | 15.648 0.021 | $i$ | 1m0-08 | 2013-08-22 | 2456526.888 | 18.625 0.121 | $i$ | 1m0-08 |
| 2013-05-16 | 2456428.929 | 15.581 0.006 | $i$ | 1m0-08 | 2013-08-22 | 2456526.891 | 18.771 0.140 | $i$ | 1m0-08 |
| 2013-05-16 | 2456428.931 | 15.555 0.008 | $i$ | 1m0-08 | 2013-08-29 | 2456533.885 | 18.732 0.132 | $i$ | 1m0-08 |
| 2013-05-18 | 2456430.930 | 15.560 0.011 | $i$ | 1m0-08 | 2013-08-29 | 2456533.887 | 18.829 0.156 | $i$ | 1m0-08 |
| 2013-05-18 | 2456430.932 | 15.527 0.015 | $i$ | 1m0-08 | 2013-09-01 | 2456536.738 | 18.941 0.143 | $i$ | 1m0-08 |
| 2013-05-20 | 2456432.930 | 15.555 0.009 | $i$ | 1m0-08 | 2013-09-01 | 2456536.741 | 18.947 0.150 | $i$ | 1m0-08 |

(a) Data have not been corrected for extinction
(b) *Swift* Telescope; LSQ (La Silla Quest, Chile); 1m0-08 (McDonald Observatory, USA); 1m0-10, 1m0-12, 1m0-13 (Sutherland, South Africa), 1m0-04, 1m0-05, 1m0-09 (Cerro Tololo, Chile); 1m0-03, 1m0-11 (Siding Spring, Australia).

**Table D1:** ASASSN-14ha: Photometric Data

| Date | JD | mag$^{(a)}$ | Filter | telescope$^{(b)}$ | Date | JD | mag$^{(a)}$ | Filter | telescope$^{(b)}$ |
|---|---|---|---|---|---|---|---|---|---|
| 2014-09-12 | 2456912.959 | 12.678 0.093 | *uw*2 | *Swift* | 2014-09-12 | 2456912.963 | 12.509 0.061 | *um*2 | *Swift* |
| 2014-09-12 | 2456912.960 | 12.687 0.071 | *uw*2 | *Swift* | 2014-09-12 | 2456912.967 | 12.511 0.058 | *um*2 | *Swift* |
| 2014-09-11 | 2456912.355 | 12.478 0.092 | *uw*2 | *Swift* | 2014-09-11 | 2456912.358 | 12.336 0.084 | *um*2 | *Swift* |
| 2014-09-11 | 2456912.356 | 12.442 0.071 | *uw*2 | *Swift* | 2014-09-11 | 2456912.359 | 12.380 0.061 | *um*2 | *Swift* |
| 2014-09-12 | 2456912.959 | 12.678 0.093 | *uw*2 | *Swift* | 2014-09-11 | 2456912.366 | 12.348 0.058 | *um*2 | *Swift* |
| 2014-09-12 | 2456912.960 | 12.687 0.071 | *uw*2 | *Swift* | 2014-09-12 | 2456912.962 | 12.543 0.087 | *um*2 | *Swift* |
| 2014-09-13 | 2456913.840 | 12.887 0.093 | *uw*2 | *Swift* | 2014-09-12 | 2456912.963 | 12.509 0.061 | *um*2 | *Swift* |
| 2014-09-13 | 2456913.840 | 13.017 0.072 | *uw*2 | *Swift* | 2014-09-12 | 2456912.967 | 12.511 0.058 | *um*2 | *Swift* |
| 2014-09-13 | 2456913.906 | 13.155 0.097 | *uw*2 | *Swift* | 2014-09-13 | 2456914.309 | 12.769 0.090 | *um*2 | *Swift* |
| 2014-09-13 | 2456913.907 | 13.121 0.072 | *uw*2 | *Swift* | 2014-09-13 | 2456914.309 | 12.795 0.069 | *um*2 | *Swift* |
| 2014-09-13 | 2456913.958 | 13.095 0.096 | *uw*2 | *Swift* | 2014-09-14 | 2456915.300 | 12.979 0.094 | *um*2 | *Swift* |
| 2014-09-13 | 2456913.958 | 13.056 0.072 | *uw*2 | *Swift* | 2014-09-14 | 2456915.300 | 13.025 0.063 | *um*2 | *Swift* |
| 2014-09-13 | 2456914.305 | 13.084 0.096 | *uw*2 | *Swift* | 2014-09-14 | 2456915.302 | 13.019 0.061 | *um*2 | *Swift* |
| 2014-09-13 | 2456914.306 | 13.071 0.072 | *uw*2 | *Swift* | 2014-09-14 | 2456915.366 | 12.954 0.094 | *um*2 | *Swift* |
| 2014-09-13 | 2456914.372 | 13.238 0.098 | *uw*2 | *Swift* | 2014-09-14 | 2456915.367 | 12.978 0.063 | *um*2 | *Swift* |
| 2014-09-13 | 2456914.373 | 13.216 0.072 | *uw*2 | *Swift* | 2014-09-14 | 2456915.369 | 13.043 0.061 | *um*2 | *Swift* |
| 2014-09-14 | 2456915.296 | 13.414 0.100 | *uw*2 | *Swift* | 2014-09-15 | 2456915.566 | 12.955 0.093 | *um*2 | *Swift* |
| 2014-09-14 | 2456915.297 | 13.498 0.073 | *uw*2 | *Swift* | 2014-09-15 | 2456915.567 | 13.087 0.063 | *um*2 | *Swift* |
| 2014-09-14 | 2456915.363 | 13.352 0.099 | *uw*2 | *Swift* | 2014-09-15 | 2456915.569 | 13.091 0.060 | *um*2 | *Swift* |
| 2014-09-14 | 2456915.363 | 13.805 0.075 | *uw*2 | *Swift* | 2014-09-15 | 2456915.902 | 13.496 0.108 | *um*2 | *Swift* |
| 2014-09-15 | 2456915.563 | 13.457 0.102 | *uw*2 | *Swift* | 2014-09-15 | 2456915.902 | 13.425 0.066 | *um*2 | *Swift* |
| 2014-09-15 | 2456915.563 | 13.511 0.073 | *uw*2 | *Swift* | 2014-09-14 | 2456915.425 | 13.064 0.063 | *um*2 | *Swift* |
| 2014-09-15 | 2456915.898 | 13.864 0.111 | *uw*2 | *Swift* | 2014-09-15 | 2456915.692 | 13.190 0.064 | *um*2 | *Swift* |
| 2014-09-15 | 2456915.899 | 13.932 0.075 | *uw*2 | *Swift* | 2014-09-15 | 2456915.759 | 13.167 0.067 | *um*2 | *Swift* |
| 2014-09-15 | 2456915.703 | 13.590 0.078 | *uw*2 | *Swift* | 2014-09-15 | 2456915.826 | 13.154 0.072 | *um*2 | *Swift* |
| 2014-09-15 | 2456915.766 | 13.681 0.085 | *uw*2 | *Swift* | 2014-09-15 | 2456915.959 | 13.217 0.065 | *um*2 | *Swift* |
| 2014-09-15 | 2456915.832 | 13.526 0.082 | *uw*2 | *Swift* | 2014-09-15 | 2456916.027 | 13.247 0.065 | *um*2 | *Swift* |
| 2014-09-15 | 2456915.969 | 13.672 0.079 | *uw*2 | *Swift* | 2014-09-15 | 2456916.368 | 13.287 0.077 | *um*2 | *Swift* |
| 2014-09-15 | 2456916.037 | 13.753 0.080 | *uw*2 | *Swift* | 2014-09-15 | 2456916.426 | 13.231 0.064 | *um*2 | *Swift* |
| 2014-09-15 | 2456916.371 | 13.790 0.105 | *uw*2 | *Swift* | 2014-09-17 | 2456918.097 | 13.422 0.105 | *um*2 | *Swift* |
| 2014-09-15 | 2456916.437 | 13.717 0.078 | *uw*2 | *Swift* | 2014-09-17 | 2456918.098 | 13.693 0.067 | *um*2 | *Swift* |
| 2014-09-17 | 2456918.094 | 14.020 0.116 | *uw*2 | *Swift* | 2014-09-17 | 2456918.101 | 13.638 0.060 | *um*2 | *Swift* |
| 2014-09-17 | 2456918.094 | 14.091 0.076 | *uw*2 | *Swift* | 2014-09-19 | 2456920.427 | 14.295 0.140 | *um*2 | *Swift* |
| 2014-09-19 | 2456920.424 | 14.870 0.152 | *uw*2 | *Swift* | 2014-09-19 | 2456920.428 | 14.380 0.074 | *um*2 | *Swift* |
| 2014-09-19 | 2456920.425 | 14.750 0.082 | *uw*2 | *Swift* | 2014-09-19 | 2456920.431 | 14.311 0.061 | *um*2 | *Swift* |
| 2014-09-21 | 2456922.421 | 14.738 0.145 | *uw*2 | *Swift* | 2014-09-21 | 2456922.425 | 14.604 0.158 | *um*2 | *Swift* |
| 2014-09-21 | 2456922.422 | 14.859 0.083 | *uw*2 | *Swift* | 2014-09-21 | 2456922.426 | 14.506 0.076 | *um*2 | *Swift* |
| 2014-09-23 | 2456923.549 | 15.257 0.140 | *uw*2 | *Swift* | 2014-09-21 | 2456922.429 | 14.516 0.062 | *um*2 | *Swift* |
| 2014-09-23 | 2456923.550 | 15.068 0.077 | *uw*2 | *Swift* | 2014-09-23 | 2456923.555 | 14.799 0.133 | *um*2 | *Swift* |
| 2014-09-30 | 2456931.022 | 16.488 0.308 | *uw*2 | *Swift* | 2014-09-23 | 2456923.557 | 14.771 0.068 | *um*2 | *Swift* |
| 2014-09-30 | 2456931.023 | 16.911 0.153 | *uw*2 | *Swift* | 2014-09-30 | 2456931.092 | 17.007 0.520 | *um*2 | *Swift* |
| 2014-09-30 | 2456931.089 | 16.833 0.376 | *uw*2 | *Swift* | 2014-10-02 | 2456932.548 | 17.509 0.707 | *um*2 | *Swift* |
| 2014-09-30 | 2456931.089 | 17.055 0.165 | *uw*2 | *Swift* | 2014-10-02 | 2456932.548 | 17.252 0.220 | *um*2 | *Swift* |
| 2014-10-02 | 2456932.544 | 17.470 0.534 | *uw*2 | *Swift* | 2014-10-02 | 2456932.551 | 17.207 0.113 | *um*2 | *Swift* |
| 2014-10-02 | 2456932.545 | 17.104 0.167 | *uw*2 | *Swift* | 2014-10-04 | 2456935.356 | 17.573 0.723 | *um*2 | *Swift* |
| 2014-10-04 | 2456935.352 | 17.627 0.623 | *uw*2 | *Swift* | 2014-10-04 | 2456935.357 | 17.712 0.291 | *um*2 | *Swift* |
| 2014-10-04 | 2456935.353 | 17.668 0.233 | *uw*2 | *Swift* | 2014-10-04 | 2456935.358 | 17.812 0.242 | *um*2 | *Swift* |
| 2014-10-06 | 2456937.475 | 17.407 0.535 | *uw*2 | *Swift* | 2014-10-06 | 2456937.479 | 17.485 0.659 | *um*2 | *Swift* |
| 2014-10-06 | 2456937.476 | 18.035 0.299 | *uw*2 | *Swift* | 2014-10-06 | 2456937.479 | 18.349 0.469 | *um*2 | *Swift* |
| 2014-10-08 | 2456939.081 | 17.849 0.258 | *uw*2 | *Swift* | 2014-10-06 | 2456937.482 | 18.162 0.185 | *um*2 | *Swift* |
| 2014-10-10 | 2456941.143 | 17.800 0.658 | *uw*2 | *Swift* | 2014-10-08 | 2456939.084 | 18.814 0.628 | *um*2 | *Swift* |
| 2014-10-10 | 2456941.144 | 18.368 0.368 | *uw*2 | *Swift* | 2014-10-08 | 2456939.087 | 18.467 0.226 | *um*2 | *Swift* |
| 2014-10-15 | 2456945.540 | 18.473 0.232 | *uw*2 | *Swift* | 2014-10-10 | 2456941.148 | 18.198 0.406 | *um*2 | *Swift* |
| 2014-10-15 | 2456945.608 | 17.873 0.650 | *uw*2 | *Swift* | 2014-10-10 | 2456941.151 | 18.531 0.214 | *um*2 | *Swift* |
| 2014-10-15 | 2456945.610 | 18.104 0.176 | *uw*2 | *Swift* | 2014-10-15 | 2456945.543 | 18.157 0.990 | *um*2 | *Swift* |
| 2014-10-19 | 2456949.541 | 18.508 0.275 | *uw*2 | *Swift* | 2014-10-15 | 2456945.544 | 18.587 0.305 | *um*2 | *Swift* |
| 2014-10-20 | 2456950.673 | 18.108 0.193 | *uw*2 | *Swift* | 2014-10-15 | 2456945.614 | 18.227 0.228 | *um*2 | *Swift* |
| 2014-10-25 | 2456955.981 | 18.240 0.582 | *uw*2 | *Swift* | 2014-10-19 | 2456949.544 | 18.161 0.258 | *um*2 | *Swift* |
| 2014-10-25 | 2456955.984 | 18.676 0.191 | *uw*2 | *Swift* | 2014-10-19 | 2456950.409 | 19.279 0.687 | *um*2 | *Swift* |
| 2014-09-12 | 2456912.962 | 12.543 0.087 | *um*2 | *Swift* | 2014-10-25 | 2456955.991 | 18.791 0.247 | *um*2 | *Swift* |

(a) Data have not been corrected for extinction
(b) *Swift* Telescope; LSQ (La Silla Quest, Chile); 1m0-08 (McDonald Observatory, USA); 1m0-10, 1m0-12, 1m0-13 (Sutherland, South Africa), 1m0-04, 1m0-05, 1m0-09 (Cerro Tololo, Chile); 1m0-03, 1m0-11 (Siding Spring, Australia).

**Table D1:** ASASSN-14ha: Photometric Data

| Date | JD | mag[(a)] | Filter | telescope[(b)] | Date | JD | mag[(a)] | Filter | telescope[(b)] |
|---|---|---|---|---|---|---|---|---|---|
| 2014-09-12 | 2456912.773 | 12.704 0.081 | *uw*1 | *Swift* | 2014-09-30 | 2456931.018 | 15.814 0.092 | *uw*1 | *Swift* |
| 2014-09-12 | 2456912.774 | 12.680 0.058 | *uw*1 | *Swift* | 2014-09-30 | 2456931.084 | 16.112 0.249 | *uw*1 | *Swift* |
| 2014-09-12 | 2456912.903 | 12.948 0.085 | *uw*1 | *Swift* | 2014-09-30 | 2456931.084 | 15.845 0.093 | *uw*1 | *Swift* |
| 2014-09-12 | 2456912.903 | 12.785 0.058 | *uw*1 | *Swift* | 2014-10-02 | 2456932.539 | 16.529 0.320 | *uw*1 | *Swift* |
| 2014-09-12 | 2456912.954 | 12.814 0.082 | *uw*1 | *Swift* | 2014-10-02 | 2456932.540 | 16.297 0.110 | *uw*1 | *Swift* |
| 2014-09-12 | 2456912.955 | 12.791 0.058 | *uw*1 | *Swift* | 2014-10-04 | 2456935.347 | 16.500 0.306 | *uw*1 | *Swift* |
| 2014-09-11 | 2456912.350 | 12.745 0.084 | *uw*1 | *Swift* | 2014-10-04 | 2456935.348 | 16.463 0.119 | *uw*1 | *Swift* |
| 2014-09-11 | 2456912.350 | 12.636 0.058 | *uw*1 | *Swift* | 2014-10-06 | 2456937.470 | 16.372 0.289 | *uw*1 | *Swift* |
| 2014-09-12 | 2456912.773 | 12.704 0.081 | *uw*1 | *Swift* | 2014-10-06 | 2456937.471 | 16.735 0.135 | *uw*1 | *Swift* |
| 2014-09-12 | 2456912.774 | 12.680 0.058 | *uw*1 | *Swift* | 2014-10-08 | 2456939.075 | 16.919 0.395 | *uw*1 | *Swift* |
| 2014-09-12 | 2456912.903 | 12.948 0.085 | *uw*1 | *Swift* | 2014-10-08 | 2456939.075 | 17.012 0.157 | *uw*1 | *Swift* |
| 2014-09-12 | 2456912.903 | 12.785 0.058 | *uw*1 | *Swift* | 2014-10-10 | 2456941.138 | 17.235 0.495 | *uw*1 | *Swift* |
| 2014-09-12 | 2456912.954 | 12.814 0.082 | *uw*1 | *Swift* | 2014-10-10 | 2456941.139 | 17.021 0.158 | *uw*1 | *Swift* |
| 2014-09-12 | 2456912.955 | 12.791 0.058 | *uw*1 | *Swift* | 2014-10-15 | 2456945.546 | 17.955 0.745 | *uw*1 | *Swift* |
| 2014-09-13 | 2456913.834 | 12.944 0.084 | *uw*1 | *Swift* | 2014-10-15 | 2456945.548 | 17.583 0.158 | *uw*1 | *Swift* |
| 2014-09-13 | 2456913.835 | 12.887 0.058 | *uw*1 | *Swift* | 2014-10-15 | 2456945.616 | 17.096 0.403 | *uw*1 | *Swift* |
| 2014-09-13 | 2456913.901 | 12.853 0.083 | *uw*1 | *Swift* | 2014-10-15 | 2456945.618 | 17.473 0.145 | *uw*1 | *Swift* |
| 2014-09-13 | 2456913.902 | 12.998 0.059 | *uw*1 | *Swift* | 2014-10-19 | 2456949.546 | 17.526 0.138 | *uw*1 | *Swift* |
| 2014-09-13 | 2456913.953 | 12.915 0.084 | *uw*1 | *Swift* | 2014-10-19 | 2456950.411 | 17.589 0.150 | *uw*1 | *Swift* |
| 2014-09-13 | 2456913.953 | 12.941 0.059 | *uw*1 | *Swift* | 2014-10-20 | 2456950.678 | 18.221 0.955 | *uw*1 | *Swift* |
| 2014-09-13 | 2456914.285 | 12.896 0.083 | *uw*1 | *Swift* | 2014-10-20 | 2456950.679 | 17.465 0.236 | *uw*1 | *Swift* |
| 2014-09-13 | 2456914.286 | 12.976 0.059 | *uw*1 | *Swift* | 2014-10-25 | 2456955.995 | 17.974 0.519 | *uw*1 | *Swift* |
| 2014-09-13 | 2456914.300 | 13.142 0.088 | *uw*1 | *Swift* | 2014-10-25 | 2456955.998 | 17.701 0.113 | *uw*1 | *Swift* |
| 2014-09-13 | 2456914.301 | 12.956 0.059 | *uw*1 | *Swift* | 2014-09-12 | 2456912.905 | 13.327 0.051 | *us* | *Swift* |
| 2014-09-13 | 2456914.352 | 13.069 0.087 | *uw*1 | *Swift* | 2014-09-12 | 2456912.956 | 13.305 0.050 | *us* | *Swift* |
| 2014-09-13 | 2456914.353 | 13.107 0.059 | *uw*1 | *Swift* | 2014-09-11 | 2456912.352 | 13.193 0.050 | *us* | *Swift* |
| 2014-09-13 | 2456914.367 | 13.144 0.086 | *uw*1 | *Swift* | 2014-09-12 | 2456912.905 | 13.327 0.051 | *us* | *Swift* |
| 2014-09-13 | 2456914.368 | 13.072 0.059 | *uw*1 | *Swift* | 2014-09-12 | 2456912.956 | 13.305 0.050 | *us* | *Swift* |
| 2014-09-14 | 2456915.291 | 13.153 0.088 | *uw*1 | *Swift* | 2014-09-13 | 2456913.837 | 13.427 0.051 | *us* | *Swift* |
| 2014-09-14 | 2456915.292 | 13.181 0.059 | *uw*1 | *Swift* | 2014-09-13 | 2456913.903 | 13.462 0.051 | *us* | *Swift* |
| 2014-09-14 | 2456915.358 | 13.147 0.087 | *uw*1 | *Swift* | 2014-09-13 | 2456913.955 | 13.415 0.051 | *us* | *Swift* |
| 2014-09-14 | 2456915.358 | 13.171 0.059 | *uw*1 | *Swift* | 2014-09-13 | 2456914.303 | 13.441 0.051 | *us* | *Swift* |
| 2014-09-15 | 2456915.557 | 13.382 0.094 | *uw*1 | *Swift* | 2014-09-13 | 2456914.355 | 13.491 0.051 | *us* | *Swift* |
| 2014-09-15 | 2456915.558 | 13.234 0.059 | *uw*1 | *Swift* | 2014-09-13 | 2456914.369 | 13.500 0.051 | *us* | *Swift* |
| 2014-09-15 | 2456915.893 | 13.466 0.095 | *uw*1 | *Swift* | 2014-09-14 | 2456915.293 | 13.523 0.051 | *us* | *Swift* |
| 2014-09-15 | 2456915.894 | 13.353 0.060 | *uw*1 | *Swift* | 2014-09-14 | 2456915.360 | 13.542 0.051 | *us* | *Swift* |
| 2014-09-15 | 2456915.690 | 13.222 0.057 | *uw*1 | *Swift* | 2014-09-15 | 2456915.560 | 13.503 0.051 | *us* | *Swift* |
| 2014-09-15 | 2456915.757 | 13.241 0.057 | *uw*1 | *Swift* | 2014-09-15 | 2456915.896 | 13.572 0.051 | *us* | *Swift* |
| 2014-09-15 | 2456915.823 | 13.259 0.057 | *uw*1 | *Swift* | 2014-09-17 | 2456918.091 | 13.673 0.051 | *us* | *Swift* |
| 2014-09-15 | 2456915.956 | 13.237 0.057 | *uw*1 | *Swift* | 2014-09-19 | 2456920.421 | 13.835 0.052 | *us* | *Swift* |
| 2014-09-15 | 2456916.025 | 13.279 0.057 | *uw*1 | *Swift* | 2014-09-21 | 2456922.419 | 13.905 0.052 | *us* | *Swift* |
| 2014-09-15 | 2456916.366 | 13.350 0.057 | *uw*1 | *Swift* | 2014-09-23 | 2456923.563 | 13.927 0.050 | *us* | *Swift* |
| 2014-09-15 | 2456916.424 | 13.391 0.057 | *uw*1 | *Swift* | 2014-09-30 | 2456931.019 | 14.529 0.055 | *us* | *Swift* |
| 2014-09-14 | 2456915.426 | 13.147 0.065 | *uw*1 | *Swift* | 2014-09-30 | 2456931.086 | 14.510 0.055 | *us* | *Swift* |
| 2014-09-15 | 2456915.693 | 13.190 0.066 | *uw*1 | *Swift* | 2014-10-02 | 2456932.542 | 14.698 0.056 | *us* | *Swift* |
| 2014-09-15 | 2456915.759 | 13.261 0.073 | *uw*1 | *Swift* | 2014-10-04 | 2456935.350 | 14.959 0.058 | *us* | *Swift* |
| 2014-09-15 | 2456915.826 | 13.189 0.072 | *uw*1 | *Swift* | 2014-10-06 | 2456937.472 | 15.182 0.061 | *us* | *Swift* |
| 2014-09-15 | 2456915.960 | 13.323 0.069 | *uw*1 | *Swift* | 2014-10-08 | 2456939.077 | 15.416 0.064 | *us* | *Swift* |
| 2014-09-15 | 2456916.028 | 13.268 0.068 | *uw*1 | *Swift* | 2014-10-10 | 2456941.141 | 15.674 0.068 | *us* | *Swift* |
| 2014-09-15 | 2456916.368 | 13.489 0.090 | *uw*1 | *Swift* | 2014-10-15 | 2456945.862 | 15.911 0.069 | *us* | *Swift* |
| 2014-09-15 | 2456916.427 | 13.288 0.067 | *uw*1 | *Swift* | 2014-10-20 | 2456951.271 | 16.164 0.075 | *us* | *Swift* |
| 2014-09-17 | 2456918.088 | 13.783 0.102 | *uw*1 | *Swift* | 2014-10-25 | 2456956.053 | 16.380 0.082 | *us* | *Swift* |
| 2014-09-17 | 2456918.089 | 13.581 0.061 | *uw*1 | *Swift* | 2014-09-20 | 2456920.808 | 14.217 0.023 | *U* | 1m0-05 |
| 2014-09-19 | 2456920.419 | 14.132 0.110 | *uw*1 | *Swift* | 2014-09-20 | 2456920.811 | 14.230 0.021 | *U* | 1m0-05 |
| 2014-09-19 | 2456920.419 | 13.991 0.063 | *uw*1 | *Swift* | 2014-09-22 | 2456922.845 | 14.275 0.025 | *U* | 1m0-09 |
| 2014-09-21 | 2456922.416 | 14.338 0.119 | *uw*1 | *Swift* | 2014-09-22 | 2456922.848 | 14.285 0.021 | *U* | 1m0-09 |
| 2014-09-21 | 2456922.417 | 14.307 0.065 | *uw*1 | *Swift* | 2014-09-25 | 2456925.869 | 14.407 0.023 | *U* | 1m0-04 |
| 2014-09-23 | 2456923.558 | 14.375 0.096 | *uw*1 | *Swift* | 2014-09-25 | 2456925.872 | 14.393 0.020 | *U* | 1m0-04 |
| 2014-09-23 | 2456923.560 | 14.489 0.061 | *uw*1 | *Swift* | 2014-09-26 | 2456926.627 | 14.385 0.041 | *U* | 1m0-12 |
| 2014-09-30 | 2456931.017 | 15.626 0.198 | *uw*1 | *Swift* | 2014-09-26 | 2456926.628 | 14.450 0.047 | *U* | 1m0-12 |

(a) Data have not been corrected for extinction
(b) *Swift* Telescope; LSQ (La Silla Quest, Chile); 1m0-08 (McDonald Observatory, USA); 1m0-10, 1m0-12, 1m0-13 (Sutherland, South Africa), 1m0-04, 1m0-05, 1m0-09 (Cerro Tololo, Chile); 1m0-03, 1m0-11 (Siding Spring, Australia).

**Table D1:** ASASSN-14ha: Photometric Data

| Date | JD | mag$^{(a)}$ | Filter | telescope$^{(b)}$ | Date | JD | mag$^{(a)}$ | Filter | telescope$^{(b)}$ |
|---|---|---|---|---|---|---|---|---|---|
| 2014-09-28 | 2456929.251 | 14.626 0.047 | *U* | 1m0-03 | 2014-09-13 | 2456913.547 | 14.643 0.016 | *B* | 1m0-12 |
| 2014-09-28 | 2456929.253 | 14.669 0.052 | *U* | 1m0-03 | 2014-09-13 | 2456913.549 | 14.599 0.017 | *B* | 1m0-12 |
| 2014-09-30 | 2456931.165 | 14.443 0.057 | *U* | 1m0-11 | 2014-09-13 | 2456913.614 | 14.653 0.012 | *B* | 1m0-12 |
| 2014-10-02 | 2456933.060 | 14.915 0.070 | *U* | 1m0-11 | 2014-09-13 | 2456913.617 | 14.603 0.014 | *B* | 1m0-12 |
| 2014-10-04 | 2456934.542 | 14.874 0.060 | *U* | 1m0-12 | 2014-09-13 | 2456914.278 | 14.930 0.057 | *B* | 1m0-03 |
| 2014-10-04 | 2456934.544 | 14.833 0.059 | *U* | 1m0-12 | 2014-09-14 | 2456914.590 | 14.691 0.028 | *B* | 1m0-10 |
| 2014-10-05 | 2456936.259 | 14.992 0.038 | *U* | 1m0-11 | 2014-09-14 | 2456914.592 | 14.681 0.022 | *B* | 1m0-10 |
| 2014-10-05 | 2456936.260 | 14.944 0.045 | *U* | 1m0-11 | 2014-09-14 | 2456914.875 | 14.715 0.010 | *B* | 1m0-05 |
| 2014-10-07 | 2456938.038 | 15.179 0.075 | *U* | 1m0-11 | 2014-09-14 | 2456914.878 | 14.710 0.010 | *B* | 1m0-05 |
| 2014-10-07 | 2456938.040 | 15.115 0.077 | *U* | 1m0-11 | 2014-09-14 | 2456915.098 | 14.783 0.013 | *B* | 1m0-03 |
| 2014-10-08 | 2456939.221 | 15.274 0.085 | *U* | 1m0-03 | 2014-09-14 | 2456915.100 | 14.796 0.014 | *B* | 1m0-03 |
| 2014-10-08 | 2456939.221 | 15.147 0.079 | *U* | 1m0-11 | 2014-09-14 | 2456915.255 | 14.755 0.015 | *B* | 1m0-11 |
| 2014-10-08 | 2456939.223 | 15.233 0.077 | *U* | 1m0-03 | 2014-09-14 | 2456915.258 | 14.725 0.013 | *B* | 1m0-11 |
| 2014-10-08 | 2456939.223 | 15.138 0.072 | *U* | 1m0-11 | 2014-09-14 | 2456915.278 | 14.634 0.019 | *B* | 1m0-11 |
| 2014-10-09 | 2456940.030 | 15.430 0.062 | *U* | 1m0-03 | 2014-09-14 | 2456915.280 | 14.674 0.017 | *B* | 1m0-11 |
| 2014-10-11 | 2456942.024 | 15.295 0.058 | *U* | 1m0-03 | 2014-09-15 | 2456916.235 | 14.806 0.013 | *B* | 1m0-11 |
| 2014-10-16 | 2456947.227 | 15.698 0.062 | *U* | 1m0-11 | 2014-09-15 | 2456916.237 | 14.768 0.012 | *B* | 1m0-11 |
| 2014-10-16 | 2456947.229 | 15.661 0.085 | *U* | 1m0-11 | 2014-09-15 | 2456916.480 | 14.782 0.014 | *B* | 1m0-12 |
| 2014-10-17 | 2456948.011 | 16.006 0.125 | *U* | 1m0-03 | 2014-09-15 | 2456916.482 | 14.764 0.018 | *B* | 1m0-12 |
| 2014-10-17 | 2456948.012 | 16.036 0.129 | *U* | 1m0-03 | 2014-09-16 | 2456916.810 | 14.849 0.013 | *B* | 1m0-09 |
| 2014-10-22 | 2456953.348 | 16.313 0.202 | *U* | 1m0-12 | 2014-09-16 | 2456916.812 | 15.023 0.023 | *B* | 1m0-09 |
| 2014-11-21 | 2456982.718 | 16.836 0.083 | *U* | 1m0-05 | 2014-09-16 | 2456917.240 | 14.817 0.016 | *B* | 1m0-11 |
| 2014-11-21 | 2456982.720 | 17.026 0.090 | *U* | 1m0-05 | 2014-09-16 | 2456917.242 | 14.897 0.018 | *B* | 1m0-11 |
| 2014-11-27 | 2456989.410 | 16.902 0.123 | *U* | 1m0-10 | 2014-09-17 | 2456917.602 | 14.770 0.058 | *B* | 1m0-12 |
| 2014-12-11 | 2457002.742 | 17.317 0.157 | *U* | 1m0-05 | 2014-09-17 | 2456917.604 | 14.764 0.028 | *B* | 1m0-12 |
| 2014-12-11 | 2457002.743 | 17.286 0.163 | *U* | 1m0-05 | 2014-09-18 | 2456918.748 | 14.879 0.012 | *B* | 1m0-04 |
| 2014-12-16 | 2457008.449 | 17.103 0.127 | *U* | 1m0-12 | 2014-09-18 | 2456918.751 | 14.908 0.011 | *B* | 1m0-04 |
| 2014-12-16 | 2457008.450 | 17.450 0.154 | *U* | 1m0-12 | 2014-09-20 | 2456920.814 | 14.877 0.012 | *B* | 1m0-05 |
| 2014-12-22 | 2457014.288 | 17.598 0.241 | *U* | 1m0-10 | 2014-09-20 | 2456920.816 | 14.908 0.012 | *B* | 1m0-05 |
| 2014-12-22 | 2457014.290 | 17.630 0.230 | *U* | 1m0-10 | 2014-09-20 | 2456920.873 | 14.938 0.012 | *B* | 1m0-09 |
| 2014-09-12 | 2456912.907 | 14.763 0.049 | *bs* | *Swift* | 2014-09-20 | 2456920.876 | 14.907 0.011 | *B* | 1m0-09 |
| 2014-09-12 | 2456912.958 | 14.721 0.048 | *bs* | *Swift* | 2014-09-22 | 2456922.851 | 15.062 0.016 | *B* | 1m0-09 |
| 2014-09-11 | 2456912.354 | 14.665 0.048 | *bs* | *Swift* | 2014-09-22 | 2456922.853 | 14.939 0.012 | *B* | 1m0-09 |
| 2014-09-12 | 2456912.907 | 14.763 0.049 | *bs* | *Swift* | 2014-09-25 | 2456925.875 | 15.002 0.012 | *B* | 1m0-04 |
| 2014-09-12 | 2456912.958 | 14.721 0.048 | *bs* | *Swift* | 2014-09-25 | 2456925.878 | 14.998 0.013 | *B* | 1m0-04 |
| 2014-09-13 | 2456913.838 | 14.788 0.049 | *bs* | *Swift* | 2014-09-26 | 2456926.630 | 15.135 0.023 | *B* | 1m0-12 |
| 2014-09-13 | 2456913.905 | 14.882 0.049 | *bs* | *Swift* | 2014-09-26 | 2456926.631 | 15.171 0.025 | *B* | 1m0-12 |
| 2014-09-13 | 2456913.957 | 14.896 0.049 | *bs* | *Swift* | 2014-09-28 | 2456929.256 | 15.223 0.044 | *B* | 1m0-03 |
| 2014-09-13 | 2456914.304 | 14.878 0.049 | *bs* | *Swift* | 2014-09-30 | 2456931.168 | 15.281 0.027 | *B* | 1m0-11 |
| 2014-09-13 | 2456914.356 | 14.831 0.055 | *bs* | *Swift* | 2014-09-30 | 2456931.169 | 15.309 0.027 | *B* | 1m0-11 |
| 2014-09-13 | 2456914.371 | 14.879 0.049 | *bs* | *Swift* | 2014-10-02 | 2456933.064 | 15.310 0.026 | *B* | 1m0-11 |
| 2014-09-14 | 2456915.295 | 14.898 0.049 | *bs* | *Swift* | 2014-10-02 | 2456933.065 | 15.369 0.030 | *B* | 1m0-11 |
| 2014-09-14 | 2456915.362 | 14.850 0.049 | *bs* | *Swift* | 2014-10-04 | 2456934.545 | 15.216 0.024 | *B* | 1m0-12 |
| 2014-09-15 | 2456915.562 | 14.929 0.049 | *bs* | *Swift* | 2014-10-04 | 2456934.547 | 15.239 0.021 | *B* | 1m0-12 |
| 2014-09-15 | 2456915.897 | 14.872 0.049 | *bs* | *Swift* | 2014-10-05 | 2456936.262 | 15.232 0.017 | *B* | 1m0-11 |
| 2014-09-17 | 2456918.093 | 14.957 0.049 | *bs* | *Swift* | 2014-10-05 | 2456936.263 | 15.328 0.014 | *B* | 1m0-11 |
| 2014-09-19 | 2456920.423 | 15.038 0.050 | *bs* | *Swift* | 2014-10-07 | 2456938.041 | 15.397 0.031 | *B* | 1m0-11 |
| 2014-09-21 | 2456922.420 | 15.013 0.050 | *bs* | *Swift* | 2014-10-07 | 2456938.043 | 15.392 0.024 | *B* | 1m0-11 |
| 2014-09-30 | 2456931.088 | 15.269 0.052 | *bs* | *Swift* | 2014-10-09 | 2456940.033 | 15.498 0.025 | *B* | 1m0-03 |
| 2014-09-30 | 2456931.021 | 15.203 0.051 | *bs* | *Swift* | 2014-10-09 | 2456940.033 | 15.495 0.024 | *B* | 1m0-11 |
| 2014-10-02 | 2456932.543 | 15.200 0.051 | *bs* | *Swift* | 2014-10-09 | 2456940.115 | 15.431 0.024 | *B* | 1m0-03 |
| 2014-10-04 | 2456935.351 | 15.291 0.052 | *bs* | *Swift* | 2014-10-11 | 2456942.026 | 15.521 0.025 | *B* | 1m0-03 |
| 2014-10-06 | 2456937.474 | 15.369 0.053 | *bs* | *Swift* | 2014-10-11 | 2456942.027 | 15.511 0.021 | *B* | 1m0-03 |
| 2014-10-08 | 2456939.079 | 15.430 0.053 | *bs* | *Swift* | 2014-10-16 | 2456947.231 | 15.626 0.019 | *B* | 1m0-11 |
| 2014-10-10 | 2456941.142 | 15.429 0.053 | *bs* | *Swift* | 2014-10-17 | 2456948.014 | 15.819 0.029 | *B* | 1m0-03 |
| 2014-10-15 | 2456945.864 | 15.557 0.052 | *bs* | *Swift* | 2014-10-17 | 2456948.015 | 15.665 0.028 | *B* | 1m0-03 |
| 2014-10-20 | 2456951.273 | 15.615 0.053 | *bs* | *Swift* | 2014-10-22 | 2456953.351 | 15.896 0.038 | *B* | 1m0-12 |
| 2014-10-25 | 2456956.055 | 15.865 0.056 | *bs* | *Swift* | 2014-10-22 | 2456953.352 | 15.759 0.034 | *B* | 1m0-12 |
| 2014-09-11 | 2456912.270 | 14.547 0.020 | *B* | 1m0-11 | 2014-10-28 | 2456959.101 | 15.877 0.024 | *B* | 1m0-11 |
| 2014-09-11 | 2456912.272 | 14.506 0.014 | *B* | 1m0-11 | 2014-10-28 | 2456959.102 | 15.985 0.027 | *B* | 1m0-11 |

(a) Data have not been corrected for extinction
(b) *Swift* Telescope; LSQ (La Silla Quest, Chile); 1m0-08 (McDonald Observatory, USA); 1m0-10, 1m0-12, 1m0-13 (Sutherland, South Africa), 1m0-04, 1m0-05, 1m0-09 (Cerro Tololo, Chile); 1m0-03, 1m0-11 (Siding Spring, Australia).

**Table D1:** ASASSN-14ha: Photometric Data

| Date | JD | mag[(a)] | Filter | telescope[(b)] |
|---|---|---|---|---|
| 2014-11-03 | 2456965.028 | 16.089 0.032 | *B* | 1m0-11 |
| 2014-11-03 | 2456965.029 | 16.108 0.033 | *B* | 1m0-11 |
| 2014-11-09 | 2456970.946 | 16.310 0.114 | *B* | 1m0-11 |
| 2014-11-21 | 2456982.722 | 16.278 0.019 | *B* | 1m0-05 |
| 2014-11-21 | 2456982.723 | 16.300 0.022 | *B* | 1m0-05 |
| 2014-11-27 | 2456989.413 | 16.386 0.023 | *B* | 1m0-10 |
| 2014-11-27 | 2456989.415 | 16.363 0.021 | *B* | 1m0-10 |
| 2014-12-04 | 2456996.184 | 16.419 0.054 | *B* | 1m0-03 |
| 2014-12-04 | 2456996.185 | 16.546 0.035 | *B* | 1m0-03 |
| 2014-12-10 | 2457001.819 | 16.442 0.024 | *B* | 1m0-05 |
| 2014-12-10 | 2457001.820 | 16.415 0.026 | *B* | 1m0-05 |
| 2014-12-11 | 2457002.745 | 16.418 0.025 | *B* | 1m0-05 |
| 2014-12-11 | 2457002.746 | 16.454 0.026 | *B* | 1m0-05 |
| 2014-12-16 | 2457008.452 | 16.469 0.025 | *B* | 1m0-12 |
| 2014-12-16 | 2457008.453 | 16.512 0.025 | *B* | 1m0-12 |
| 2014-12-22 | 2457014.292 | 16.637 0.041 | *B* | 1m0-10 |
| 2014-12-22 | 2457014.293 | 16.386 0.051 | *B* | 1m0-10 |
| 2014-12-22 | 2457014.318 | 16.377 0.049 | *B* | 1m0-13 |
| 2014-12-22 | 2457014.320 | 16.541 0.048 | *B* | 1m0-13 |
| 2014-12-23 | 2457015.317 | 16.528 0.019 | *B* | 1m0-12 |
| 2014-12-23 | 2457015.319 | 16.504 0.019 | *B* | 1m0-12 |
| 2014-12-25 | 2457017.329 | 16.670 0.018 | *B* | 1m0-12 |
| 2014-12-25 | 2457017.332 | 16.652 0.017 | *B* | 1m0-12 |
| 2014-12-25 | 2457017.355 | 16.373 0.037 | *B* | 1m0-12 |
| 2014-12-25 | 2457017.358 | 16.561 0.021 | *B* | 1m0-12 |
| 2014-12-27 | 2457019.370 | 16.689 0.015 | *B* | 1m0-10 |
| 2014-12-27 | 2457019.373 | 16.718 0.017 | *B* | 1m0-10 |
| 2014-12-29 | 2457021.042 | 16.571 0.021 | *B* | 1m0-11 |
| 2014-12-31 | 2457022.747 | 16.755 0.022 | *B* | 1m0-05 |
| 2014-12-31 | 2457022.750 | 16.723 0.025 | *B* | 1m0-05 |
| 2015-01-02 | 2457025.046 | 16.717 0.028 | *B* | 1m0-11 |
| 2015-01-03 | 2457026.462 | 16.833 0.021 | *B* | 1m0-12 |
| 2015-01-03 | 2457026.465 | 16.869 0.021 | *B* | 1m0-12 |
| 2015-01-05 | 2457028.329 | 16.845 0.022 | *B* | 1m0-10 |
| 2015-01-05 | 2457028.351 | 16.886 0.028 | *B* | 1m0-12 |
| 2015-01-05 | 2457028.354 | 16.889 0.030 | *B* | 1m0-12 |
| 2015-01-09 | 2457031.966 | 16.723 0.037 | *B* | 1m0-03 |
| 2015-01-09 | 2457031.969 | 16.861 0.032 | *B* | 1m0-03 |
| 2015-01-11 | 2457034.317 | 17.029 0.024 | *B* | 1m0-12 |
| 2015-01-11 | 2457034.320 | 17.002 0.020 | *B* | 1m0-12 |
| 2015-01-13 | 2457036.458 | 17.343 0.042 | *B* | 1m0-13 |
| 2015-01-13 | 2457036.460 | 17.244 0.041 | *B* | 1m0-13 |
| 2015-01-15 | 2457038.096 | 17.425 0.029 | *B* | 1m0-11 |
| 2015-01-15 | 2457038.098 | 17.378 0.037 | *B* | 1m0-11 |
| 2015-01-17 | 2457039.718 | 17.327 0.027 | *B* | 1m0-05 |
| 2015-01-17 | 2457039.721 | 17.366 0.026 | *B* | 1m0-05 |
| 2015-01-18 | 2457041.455 | 17.426 0.026 | *B* | 1m0-12 |
| 2015-01-18 | 2457041.458 | 17.469 0.024 | *B* | 1m0-12 |
| 2015-01-20 | 2457043.295 | 17.574 0.026 | *B* | 1m0-10 |
| 2015-01-20 | 2457043.297 | 17.571 0.028 | *B* | 1m0-10 |
| 2015-01-22 | 2457045.308 | 17.983 0.038 | *B* | 1m0-10 |
| 2015-01-22 | 2457045.312 | 17.809 0.030 | *B* | 1m0-10 |
| 2015-01-25 | 2457047.958 | 19.079 0.080 | *B* | 1m0-11 |
| 2015-01-25 | 2457047.962 | 19.488 0.155 | *B* | 1m0-11 |
| 2015-01-27 | 2457049.613 | 20.065 0.011 | *B* | 1m0-05 |
| 2015-01-27 | 2457049.617 | 20.742 0.166 | *B* | 1m0-05 |
| 2015-02-03 | 2457056.684 | $< 20.358$ | *B* | 1m0-05 |
| 2015-02-03 | 2457056.688 | $< 19.973$ | *B* | 1m0-05 |
| 2015-02-11 | 2457064.600 | 20.880 0.127 | *B* | 1m0-33 |
| 2014-09-11 | 2456912.278 | 14.555 0.027 | *g* | 1m0-11 |
| 2014-09-11 | 2456912.281 | 14.579 0.026 | *g* | 1m0-11 |
| 2014-09-13 | 2456913.555 | 14.684 0.039 | *g* | 1m0-12 |
| 2014-09-13 | 2456913.558 | 14.690 0.042 | *g* | 1m0-12 |
| 2014-09-13 | 2456913.623 | 14.587 0.034 | *g* | 1m0-12 |
| 2014-09-13 | 2456913.625 | 14.685 0.033 | *g* | 1m0-12 |
| 2014-09-14 | 2456914.598 | 14.799 0.026 | *g* | 1m0-10 |
| 2014-09-14 | 2456914.601 | 14.794 0.027 | *g* | 1m0-10 |
| 2014-09-14 | 2456914.885 | 14.695 0.009 | *g* | 1m0-05 |
| 2014-09-14 | 2456914.888 | 14.705 0.007 | *g* | 1m0-05 |
| 2014-09-14 | 2456915.106 | 14.764 0.035 | *g* | 1m0-03 |
| 2014-09-14 | 2456915.109 | 14.748 0.030 | *g* | 1m0-03 |
| 2014-09-14 | 2456915.263 | 14.675 0.034 | *g* | 1m0-11 |
| 2014-09-14 | 2456915.266 | 14.698 0.033 | *g* | 1m0-11 |
| 2014-09-14 | 2456915.289 | 14.484 0.049 | *g* | 1m0-11 |
| 2014-09-15 | 2456916.243 | 14.803 0.031 | *g* | 1m0-11 |
| 2014-09-15 | 2456916.246 | 14.796 0.029 | *g* | 1m0-11 |
| 2014-09-15 | 2456916.488 | 14.768 0.034 | *g* | 1m0-12 |
| 2014-09-15 | 2456916.491 | 14.792 0.115 | *g* | 1m0-12 |
| 2014-09-16 | 2456916.819 | 14.871 0.010 | *g* | 1m0-09 |
| 2014-09-16 | 2456916.822 | 14.897 0.011 | *g* | 1m0-09 |
| 2014-09-16 | 2456917.248 | 14.812 0.024 | *g* | 1m0-11 |
| 2014-09-16 | 2456917.251 | 14.788 0.028 | *g* | 1m0-11 |
| 2014-09-18 | 2456918.758 | 14.974 0.011 | *g* | 1m0-04 |
| 2014-09-18 | 2456918.761 | 14.967 0.014 | *g* | 1m0-04 |
| 2014-09-20 | 2456920.822 | 14.994 0.033 | *g* | 1m0-05 |
| 2014-09-20 | 2456920.824 | 14.982 0.028 | *g* | 1m0-05 |
| 2014-09-20 | 2456920.883 | 14.862 0.010 | *g* | 1m0-09 |
| 2014-09-20 | 2456920.886 | 14.871 0.011 | *g* | 1m0-09 |
| 2014-09-22 | 2456922.858 | 14.879 0.010 | *g* | 1m0-09 |
| 2014-09-22 | 2456922.860 | 14.902 0.011 | *g* | 1m0-09 |
| 2014-09-25 | 2456925.884 | 14.965 0.012 | *g* | 1m0-04 |
| 2014-09-25 | 2456925.886 | 14.964 0.011 | *g* | 1m0-04 |
| 2014-09-26 | 2456926.634 | 14.998 0.029 | *g* | 1m0-12 |
| 2014-09-26 | 2456926.635 | 14.995 0.027 | *g* | 1m0-12 |
| 2014-09-30 | 2456931.172 | 15.016 0.025 | *g* | 1m0-11 |
| 2014-09-30 | 2456931.174 | 15.078 0.023 | *g* | 1m0-11 |
| 2014-10-02 | 2456933.068 | 15.120 0.024 | *g* | 1m0-11 |
| 2014-10-02 | 2456933.069 | 15.254 0.026 | *g* | 1m0-11 |
| 2014-10-04 | 2456934.550 | 15.093 0.036 | *g* | 1m0-12 |
| 2014-10-04 | 2456934.551 | 15.232 0.037 | *g* | 1m0-12 |
| 2014-10-05 | 2456936.266 | 15.186 0.027 | *g* | 1m0-11 |
| 2014-10-05 | 2456936.267 | 15.100 0.028 | *g* | 1m0-11 |
| 2014-10-07 | 2456938.046 | 15.168 0.028 | *g* | 1m0-11 |
| 2014-10-07 | 2456938.047 | 15.180 0.028 | *g* | 1m0-11 |
| 2014-10-09 | 2456940.038 | 15.236 0.031 | *g* | 1m0-03 |
| 2014-10-09 | 2456940.038 | 15.192 0.060 | *g* | 1m0-11 |
| 2014-10-09 | 2456940.119 | 15.210 0.028 | *g* | 1m0-03 |
| 2014-10-11 | 2456942.030 | 15.240 0.028 | *g* | 1m0-03 |
| 2014-10-11 | 2456942.030 | 15.275 0.028 | *g* | 1m0-03 |
| 2014-10-17 | 2456948.018 | 15.412 0.030 | *g* | 1m0-03 |
| 2014-10-17 | 2456948.019 | 15.456 0.034 | *g* | 1m0-03 |
| 2014-10-22 | 2456953.355 | 15.482 0.028 | *g* | 1m0-12 |
| 2014-10-22 | 2456953.356 | 15.508 0.030 | *g* | 1m0-12 |
| 2014-10-28 | 2456959.105 | 15.401 0.028 | *g* | 1m0-11 |
| 2014-11-03 | 2456965.032 | 15.549 0.030 | *g* | 1m0-11 |
| 2014-11-03 | 2456965.033 | 15.486 0.027 | *g* | 1m0-11 |
| 2014-11-21 | 2456982.726 | 15.588 0.030 | *g* | 1m0-05 |
| 2014-11-21 | 2456982.727 | 15.554 0.032 | *g* | 1m0-05 |
| 2014-11-27 | 2456989.417 | 15.604 0.028 | *g* | 1m0-10 |
| 2014-11-27 | 2456989.418 | 15.621 0.027 | *g* | 1m0-10 |

(a) Data have not been corrected for extinction
(b) *Swift* Telescope; LSQ (La Silla Quest, Chile); 1m0-08 (McDonald Observatory, USA); 1m0-10, 1m0-12, 1m0-13 (Sutherland, South Africa), 1m0-04, 1m0-05, 1m0-09 (Cerro Tololo, Chile); 1m0-03, 1m0-11 (Siding Spring, Australia).

**Table D1:** ASASSN-14ha: Photometric Data

| Date | JD | mag[(a)] | Filter | telescope[(b)] | Date | JD | mag[(a)] | Filter | telescope[(b)] |
|---|---|---|---|---|---|---|---|---|---|
| 2014-12-04 | 2456996.188 | 15.728 0.029 | *g* | 1m0-03 | 2014-09-30 | 2456931.091 | 14.938 0.059 | *vs* | *Swift* |
| 2014-12-04 | 2456996.189 | 15.577 0.031 | *g* | 1m0-03 | 2014-10-02 | 2456932.547 | 14.870 0.057 | *vs* | *Swift* |
| 2014-12-10 | 2457001.823 | 15.688 0.029 | *g* | 1m0-05 | 2014-10-04 | 2456935.355 | 14.949 0.059 | *vs* | *Swift* |
| 2014-12-10 | 2457001.824 | 15.658 0.028 | *g* | 1m0-05 | 2014-10-06 | 2456937.478 | 14.879 0.058 | *vs* | *Swift* |
| 2014-12-11 | 2457002.749 | 15.706 0.028 | *g* | 1m0-05 | 2014-10-08 | 2456939.082 | 14.892 0.058 | *vs* | *Swift* |
| 2014-12-11 | 2457002.750 | 15.668 0.028 | *g* | 1m0-05 | 2014-10-10 | 2456941.146 | 14.965 0.059 | *vs* | *Swift* |
| 2014-12-16 | 2457008.456 | 15.683 0.034 | *g* | 1m0-12 | 2014-10-15 | 2456945.867 | 14.987 0.051 | *vs* | *Swift* |
| 2014-12-16 | 2457008.457 | 15.659 0.036 | *g* | 1m0-12 | 2014-10-20 | 2456951.276 | 14.994 0.045 | *vs* | *Swift* |
| 2014-12-22 | 2457014.296 | 15.669 0.027 | *g* | 1m0-10 | 2014-10-25 | 2456956.058 | 15.048 0.044 | *vs* | *Swift* |
| 2014-12-22 | 2457014.297 | 15.715 0.062 | *g* | 1m0-10 | 2014-09-08 | 2456908.834 | $< 16.000$ | *V* | Atel/CBAT |
| 2014-12-23 | 2457015.325 | 15.836 0.039 | *g* | 1m0-12 | 2014-09-11 | 2456912.275 | 14.729 0.019 | *V* | 1m0-11 |
| 2014-12-23 | 2457015.328 | 15.818 0.083 | *g* | 1m0-12 | 2014-09-11 | 2456912.277 | 14.716 0.019 | *V* | 1m0-11 |
| 2014-12-25 | 2457017.338 | 15.823 0.041 | *g* | 1m0-12 | 2014-09-13 | 2456913.552 | 14.867 0.016 | *V* | 1m0-12 |
| 2014-12-25 | 2457017.340 | 15.812 0.042 | *g* | 1m0-12 | 2014-09-13 | 2456913.554 | 14.851 0.015 | *V* | 1m0-12 |
| 2014-12-25 | 2457017.364 | 15.703 0.030 | *g* | 1m0-12 | 2014-09-13 | 2456913.621 | 14.869 0.015 | *V* | 1m0-12 |
| 2014-12-25 | 2457017.366 | 15.728 0.031 | *g* | 1m0-12 | 2014-09-14 | 2456914.595 | 14.882 0.026 | *V* | 1m0-10 |
| 2014-12-27 | 2457019.379 | 15.755 0.028 | *g* | 1m0-10 | 2014-09-14 | 2456914.597 | 14.904 0.026 | *V* | 1m0-10 |
| 2014-12-27 | 2457019.381 | 15.784 0.028 | *g* | 1m0-10 | 2014-09-14 | 2456914.881 | 14.880 0.010 | *V* | 1m0-05 |
| 2014-12-29 | 2457021.048 | 15.847 0.090 | *g* | 1m0-11 | 2014-09-14 | 2456914.883 | 14.867 0.009 | *V* | 1m0-05 |
| 2014-12-31 | 2457022.756 | 15.870 0.036 | *g* | 1m0-05 | 2014-09-14 | 2456915.103 | 14.890 0.014 | *V* | 1m0-03 |
| 2014-12-31 | 2457022.758 | 15.787 0.039 | *g* | 1m0-05 | 2014-09-14 | 2456915.104 | 14.882 0.014 | *V* | 1m0-03 |
| 2015-01-02 | 2457025.052 | 15.884 0.031 | *g* | 1m0-11 | 2014-09-14 | 2456915.260 | 14.888 0.013 | *V* | 1m0-11 |
| 2015-01-02 | 2457025.055 | 15.873 0.032 | *g* | 1m0-11 | 2014-09-14 | 2456915.262 | 14.895 0.014 | *V* | 1m0-11 |
| 2015-01-03 | 2457026.471 | 15.974 0.042 | *g* | 1m0-12 | 2014-09-14 | 2456915.283 | 14.833 0.015 | *V* | 1m0-11 |
| 2015-01-03 | 2457026.473 | 15.979 0.042 | *g* | 1m0-12 | 2014-09-14 | 2456915.285 | 14.802 0.013 | *V* | 1m0-11 |
| 2015-01-05 | 2457028.338 | 15.964 0.033 | *g* | 1m0-10 | 2014-09-15 | 2456916.240 | 14.906 0.015 | *V* | 1m0-11 |
| 2015-01-05 | 2457028.360 | 15.889 0.037 | *g* | 1m0-12 | 2014-09-15 | 2456916.241 | 14.903 0.013 | *V* | 1m0-11 |
| 2015-01-05 | 2457028.362 | 15.959 0.035 | *g* | 1m0-12 | 2014-09-15 | 2456916.485 | 14.922 0.014 | *V* | 1m0-12 |
| 2015-01-09 | 2457031.975 | 16.074 0.044 | *g* | 1m0-03 | 2014-09-15 | 2456916.486 | 14.891 0.014 | *V* | 1m0-12 |
| 2015-01-11 | 2457034.329 | 16.077 0.062 | *g* | 1m0-12 | 2014-09-16 | 2456916.815 | 15.005 0.016 | *V* | 1m0-09 |
| 2015-01-15 | 2457038.104 | 16.191 0.039 | *g* | 1m0-11 | 2014-09-16 | 2456916.817 | 15.010 0.016 | *V* | 1m0-09 |
| 2015-01-15 | 2457038.107 | 16.216 0.040 | *g* | 1m0-11 | 2014-09-16 | 2456917.247 | 14.954 0.015 | *V* | 1m0-11 |
| 2015-01-17 | 2457039.727 | 16.316 0.038 | *g* | 1m0-05 | 2014-09-20 | 2456920.818 | 14.981 0.015 | *V* | 1m0-05 |
| 2015-01-17 | 2457039.729 | 16.295 0.037 | *g* | 1m0-05 | 2014-09-20 | 2456920.820 | 14.957 0.014 | *V* | 1m0-05 |
| 2015-01-18 | 2457041.464 | 16.309 0.033 | *g* | 1m0-12 | 2014-09-20 | 2456920.879 | 14.965 0.010 | *V* | 1m0-09 |
| 2015-01-18 | 2457041.467 | 16.397 0.031 | *g* | 1m0-12 | 2014-09-20 | 2456920.881 | 14.976 0.012 | *V* | 1m0-09 |
| 2015-01-20 | 2457043.303 | 16.547 0.030 | *g* | 1m0-10 | 2014-09-22 | 2456922.855 | 14.966 0.015 | *V* | 1m0-09 |
| 2015-01-20 | 2457043.306 | 16.539 0.029 | *g* | 1m0-10 | 2014-09-22 | 2456922.857 | 14.962 0.015 | *V* | 1m0-09 |
| 2015-01-22 | 2457045.322 | 16.881 0.062 | *g* | 1m0-10 | 2014-09-25 | 2456925.880 | 15.023 0.012 | *V* | 1m0-04 |
| 2015-01-22 | 2457045.326 | 16.851 0.030 | *g* | 1m0-10 | 2014-09-25 | 2456925.882 | 15.041 0.012 | *V* | 1m0-04 |
| 2015-01-25 | 2457047.972 | 18.207 0.047 | *g* | 1m0-11 | 2014-09-26 | 2456926.632 | 15.050 0.018 | *V* | 1m0-12 |
| 2015-01-25 | 2457047.975 | 18.548 0.067 | *g* | 1m0-11 | 2014-09-26 | 2456926.633 | 15.012 0.018 | *V* | 1m0-12 |
| 2015-02-01 | 2457055.028 | 20.144 0.183 | *g* | 1m0-11 | 2014-09-30 | 2456931.171 | 15.069 0.024 | *V* | 1m0-11 |
| 2015-02-10 | 2457064.345 | 20.163 0.152 | *g* | 1m0-10 | 2014-09-30 | 2456931.171 | 14.970 0.025 | *V* | 1m0-11 |
| 2014-09-12 | 2456912.961 | 14.723 0.055 | *vs* | *Swift* | 2014-10-02 | 2456933.066 | 15.085 0.024 | *V* | 1m0-11 |
| 2014-09-11 | 2456912.357 | 14.645 0.053 | *vs* | *Swift* | 2014-10-02 | 2456933.067 | 15.078 0.024 | *V* | 1m0-11 |
| 2014-09-12 | 2456912.961 | 14.723 0.055 | *vs* | *Swift* | 2014-10-04 | 2456934.548 | 15.074 0.022 | *V* | 1m0-12 |
| 2014-09-13 | 2456913.842 | 14.670 0.057 | *vs* | *Swift* | 2014-10-04 | 2456934.549 | 15.066 0.022 | *V* | 1m0-12 |
| 2014-09-13 | 2456913.909 | 14.722 0.057 | *vs* | *Swift* | 2014-10-05 | 2456936.264 | 15.118 0.017 | *V* | 1m0-11 |
| 2014-09-13 | 2456914.308 | 14.686 0.055 | *vs* | *Swift* | 2014-10-05 | 2456936.265 | 15.111 0.017 | *V* | 1m0-11 |
| 2014-09-13 | 2456914.374 | 14.773 0.062 | *vs* | *Swift* | 2014-10-07 | 2456938.044 | 15.090 0.027 | *V* | 1m0-11 |
| 2014-09-14 | 2456915.299 | 14.754 0.055 | *vs* | *Swift* | 2014-10-07 | 2456938.045 | 15.091 0.028 | *V* | 1m0-11 |
| 2014-09-14 | 2456915.365 | 14.748 0.055 | *vs* | *Swift* | 2014-10-09 | 2456940.035 | 15.187 0.022 | *V* | 1m0-03 |
| 2014-09-15 | 2456915.565 | 14.779 0.056 | *vs* | *Swift* | 2014-10-09 | 2456940.035 | 15.189 0.023 | *V* | 1m0-11 |
| 2014-09-15 | 2456915.901 | 14.710 0.055 | *vs* | *Swift* | 2014-10-09 | 2456940.116 | 15.148 0.023 | *V* | 1m0-03 |
| 2014-09-17 | 2456918.096 | 14.800 0.056 | *vs* | *Swift* | 2014-10-11 | 2456942.028 | 15.186 0.022 | *V* | 1m0-03 |
| 2014-09-19 | 2456920.426 | 14.848 0.057 | *vs* | *Swift* | 2014-10-11 | 2456942.029 | 15.156 0.023 | *V* | 1m0-03 |
| 2014-09-21 | 2456922.424 | 14.803 0.056 | *vs* | *Swift* | 2014-10-17 | 2456948.017 | 15.195 0.024 | *V* | 1m0-03 |
| 2014-09-23 | 2456923.553 | 14.902 0.047 | *vs* | *Swift* | 2014-10-22 | 2456953.354 | 15.132 0.033 | *V* | 1m0-12 |
| 2014-09-30 | 2456931.024 | 14.912 0.093 | *vs* | *Swift* | 2014-10-28 | 2456959.104 | 15.187 0.020 | *V* | 1m0-11 |

(a) Data have not been corrected for extinction
(b) *Swift* Telescope; LSQ (La Silla Quest, Chile); 1m0-08 (McDonald Observatory, USA); 1m0-10, 1m0-12, 1m0-13 (Sutherland, South Africa), 1m0-04, 1m0-05, 1m0-09 (Cerro Tololo, Chile); 1m0-03, 1m0-11 (Siding Spring, Australia).

**Table D1:** ASASSN-14ha: Photometric Data

| Date | JD | mag[(a)] | Filter | telescope[(b)] | Date | JD | mag[(a)] | Filter | telescope[(b)] |
|---|---|---|---|---|---|---|---|---|---|
| 2014-10-28 | 2456959.104 | 15.185 0.021 | $V$ | 1m0-11 | 2015-03-08 | 2457089.531 | < 19.043 | $V$ | 1m0-04 |
| 2014-11-03 | 2456965.031 | 15.193 0.025 | $V$ | 1m0-11 | 2015-02-11 | 2457064.600 | 19.307 0.100 | $V$ | 1m0-33 |
| 2014-11-03 | 2456965.032 | 15.221 0.026 | $V$ | 1m0-11 | 2014-09-11 | 2456912.284 | 14.851 0.015 | $r$ | 1m0-11 |
| 2014-11-09 | 2456970.950 | 15.230 0.115 | $V$ | 1m0-11 | 2014-09-11 | 2456912.285 | 14.876 0.015 | $r$ | 1m0-11 |
| 2014-11-15 | 2456977.198 | 15.177 0.128 | $V$ | 1m0-03 | 2014-09-13 | 2456913.561 | 14.916 0.019 | $r$ | 1m0-12 |
| 2014-11-21 | 2456982.724 | 15.242 0.019 | $V$ | 1m0-05 | 2014-09-13 | 2456913.562 | 14.900 0.019 | $r$ | 1m0-12 |
| 2014-11-21 | 2456982.725 | 15.268 0.018 | $V$ | 1m0-05 | 2014-09-13 | 2456913.628 | 14.941 0.020 | $r$ | 1m0-12 |
| 2014-11-27 | 2456989.416 | 15.334 0.018 | $V$ | 1m0-10 | 2014-09-13 | 2456913.630 | 14.953 0.018 | $r$ | 1m0-12 |
| 2014-11-27 | 2456989.417 | 15.341 0.018 | $V$ | 1m0-10 | 2014-09-14 | 2456914.604 | 15.021 0.016 | $r$ | 1m0-10 |
| 2014-12-04 | 2456996.187 | 15.256 0.030 | $V$ | 1m0-03 | 2014-09-14 | 2456914.605 | 14.900 0.016 | $r$ | 1m0-10 |
| 2014-12-04 | 2456996.187 | 15.290 0.030 | $V$ | 1m0-03 | 2014-09-14 | 2456914.891 | 15.000 0.010 | $r$ | 1m0-05 |
| 2014-12-10 | 2457001.821 | 15.312 0.017 | $V$ | 1m0-05 | 2014-09-14 | 2456914.893 | 15.021 0.007 | $r$ | 1m0-05 |
| 2014-12-10 | 2457001.822 | 15.322 0.017 | $V$ | 1m0-05 | 2014-09-14 | 2456915.111 | 14.940 0.021 | $r$ | 1m0-03 |
| 2014-12-11 | 2457002.748 | 15.305 0.019 | $V$ | 1m0-05 | 2014-09-14 | 2456915.113 | 14.904 0.021 | $r$ | 1m0-03 |
| 2014-12-11 | 2457002.749 | 15.253 0.018 | $V$ | 1m0-05 | 2014-09-14 | 2456915.269 | 14.884 0.021 | $r$ | 1m0-11 |
| 2014-12-16 | 2457008.454 | 15.274 0.019 | $V$ | 1m0-12 | 2014-09-14 | 2456915.270 | 14.903 0.019 | $r$ | 1m0-11 |
| 2014-12-16 | 2457008.455 | 15.301 0.018 | $V$ | 1m0-12 | 2014-09-14 | 2456915.292 | 14.879 0.018 | $r$ | 1m0-11 |
| 2014-12-22 | 2457014.294 | 15.315 0.021 | $V$ | 1m0-10 | 2014-09-14 | 2456915.293 | 14.899 0.021 | $r$ | 1m0-11 |
| 2014-12-22 | 2457014.295 | 15.357 0.028 | $V$ | 1m0-10 | 2014-09-15 | 2456916.250 | 14.978 0.034 | $r$ | 1m0-11 |
| 2014-12-22 | 2457014.321 | 15.275 0.020 | $V$ | 1m0-13 | 2014-09-15 | 2456916.493 | 14.911 0.019 | $r$ | 1m0-12 |
| 2014-12-23 | 2457015.322 | 15.319 0.016 | $V$ | 1m0-12 | 2014-09-15 | 2456916.495 | 14.953 0.017 | $r$ | 1m0-12 |
| 2014-12-23 | 2457015.324 | 15.390 0.018 | $V$ | 1m0-12 | 2014-09-16 | 2456916.825 | 15.106 0.019 | $r$ | 1m0-09 |
| 2014-12-25 | 2457017.334 | 15.402 0.014 | $V$ | 1m0-12 | 2014-09-16 | 2456916.827 | 15.181 0.023 | $r$ | 1m0-09 |
| 2014-12-25 | 2457017.336 | 15.391 0.013 | $V$ | 1m0-12 | 2014-09-16 | 2456917.255 | 15.101 0.033 | $r$ | 1m0-11 |
| 2014-12-25 | 2457017.361 | 15.358 0.014 | $V$ | 1m0-12 | 2014-09-18 | 2456918.764 | 15.115 0.010 | $r$ | 1m0-04 |
| 2014-12-25 | 2457017.362 | 15.259 0.020 | $V$ | 1m0-12 | 2014-09-18 | 2456918.766 | 15.179 0.015 | $r$ | 1m0-04 |
| 2014-12-27 | 2457019.375 | 15.412 0.011 | $V$ | 1m0-10 | 2014-09-20 | 2456920.889 | 14.970 0.008 | $r$ | 1m0-09 |
| 2014-12-27 | 2457019.377 | 15.417 0.012 | $V$ | 1m0-10 | 2014-09-20 | 2456920.891 | 15.005 0.009 | $r$ | 1m0-09 |
| 2014-12-29 | 2457021.047 | 15.441 0.022 | $V$ | 1m0-11 | 2014-09-22 | 2456922.862 | 15.012 0.007 | $r$ | 1m0-09 |
| 2014-12-31 | 2457022.752 | 15.409 0.015 | $V$ | 1m0-05 | 2014-09-22 | 2456922.864 | 14.999 0.010 | $r$ | 1m0-09 |
| 2014-12-31 | 2457022.754 | 15.434 0.018 | $V$ | 1m0-05 | 2014-09-25 | 2456925.888 | 15.020 0.010 | $r$ | 1m0-04 |
| 2015-01-02 | 2457025.049 | 15.459 0.030 | $V$ | 1m0-11 | 2014-09-25 | 2456925.889 | 15.012 0.009 | $r$ | 1m0-04 |
| 2015-01-02 | 2457025.051 | 15.457 0.031 | $V$ | 1m0-11 | 2014-09-26 | 2456926.637 | 15.022 0.017 | $r$ | 1m0-12 |
| 2015-01-03 | 2457026.468 | 15.467 0.019 | $V$ | 1m0-12 | 2014-09-30 | 2456931.175 | 15.098 0.017 | $r$ | 1m0-11 |
| 2015-01-03 | 2457026.469 | 15.488 0.019 | $V$ | 1m0-12 | 2014-09-30 | 2456931.176 | 15.033 0.017 | $r$ | 1m0-11 |
| 2015-01-05 | 2457028.333 | 15.517 0.015 | $V$ | 1m0-10 | 2014-10-02 | 2456933.070 | 15.141 0.018 | $r$ | 1m0-11 |
| 2015-01-05 | 2457028.356 | 15.588 0.018 | $V$ | 1m0-12 | 2014-10-02 | 2456933.071 | 14.962 0.015 | $r$ | 1m0-11 |
| 2015-01-05 | 2457028.358 | 15.564 0.015 | $V$ | 1m0-12 | 2014-10-04 | 2456934.552 | 15.006 0.018 | $r$ | 1m0-12 |
| 2015-01-09 | 2457031.971 | 15.588 0.018 | $V$ | 1m0-03 | 2014-10-04 | 2456934.553 | 14.997 0.018 | $r$ | 1m0-12 |
| 2015-01-09 | 2457031.973 | 15.443 0.023 | $V$ | 1m0-03 | 2014-10-05 | 2456936.269 | 14.931 0.020 | $r$ | 1m0-11 |
| 2015-01-11 | 2457034.323 | 15.686 0.015 | $V$ | 1m0-12 | 2014-10-05 | 2456936.269 | 14.961 0.018 | $r$ | 1m0-11 |
| 2015-01-11 | 2457034.324 | 15.675 0.016 | $V$ | 1m0-12 | 2014-10-07 | 2456938.048 | 15.039 0.016 | $r$ | 1m0-11 |
| 2015-01-13 | 2457036.465 | 15.822 0.029 | $V$ | 1m0-13 | 2014-10-07 | 2456938.049 | 14.987 0.017 | $r$ | 1m0-11 |
| 2015-01-17 | 2457039.723 | 15.792 0.016 | $V$ | 1m0-05 | 2014-10-09 | 2456940.039 | 15.075 0.018 | $r$ | 1m0-03 |
| 2015-01-17 | 2457039.725 | 15.801 0.018 | $V$ | 1m0-05 | 2014-10-09 | 2456940.039 | 14.998 0.019 | $r$ | 1m0-11 |
| 2015-01-18 | 2457041.461 | 15.908 0.015 | $V$ | 1m0-12 | 2014-10-09 | 2456940.120 | 15.084 0.017 | $r$ | 1m0-03 |
| 2015-01-18 | 2457041.462 | 15.923 0.015 | $V$ | 1m0-12 | 2014-10-11 | 2456942.031 | 14.873 0.030 | $r$ | 1m0-03 |
| 2015-01-20 | 2457043.300 | 16.002 0.018 | $V$ | 1m0-10 | 2014-10-11 | 2456942.032 | 14.871 0.034 | $r$ | 1m0-03 |
| 2015-01-20 | 2457043.301 | 16.000 0.017 | $V$ | 1m0-10 | 2014-10-16 | 2456947.237 | 14.986 0.026 | $r$ | 1m0-11 |
| 2015-01-22 | 2457045.316 | 16.360 0.016 | $V$ | 1m0-10 | 2014-10-16 | 2456947.238 | 15.004 0.025 | $r$ | 1m0-11 |
| 2015-01-22 | 2457045.318 | 16.556 0.018 | $V$ | 1m0-10 | 2014-10-17 | 2456948.020 | 15.181 0.022 | $r$ | 1m0-03 |
| 2015-01-25 | 2457047.966 | 17.557 0.050 | $V$ | 1m0-11 | 2014-10-17 | 2456948.021 | 15.038 0.021 | $r$ | 1m0-03 |
| 2015-01-25 | 2457047.968 | 17.481 0.042 | $V$ | 1m0-11 | 2014-10-22 | 2456953.357 | 14.960 0.022 | $r$ | 1m0-12 |
| 2015-01-27 | 2457049.621 | 19.126 0.069 | $V$ | 1m0-05 | 2014-10-22 | 2456953.357 | 14.970 0.024 | $r$ | 1m0-12 |
| 2015-01-27 | 2457049.623 | 19.274 0.089 | $V$ | 1m0-05 | 2014-10-28 | 2456959.107 | 14.835 0.020 | $r$ | 1m0-11 |
| 2015-01-30 | 2457053.017 | 18.999 0.083 | $V$ | 1m0-03 | 2014-10-28 | 2456959.108 | 14.907 0.027 | $r$ | 1m0-11 |
| 2015-02-03 | 2457056.691 | 19.367 0.181 | $V$ | 1m0-05 | 2014-11-03 | 2456965.034 | 14.915 0.016 | $r$ | 1m0-11 |
| 2015-02-04 | 2457058.400 | < 18.962 | $V$ | 1m0-12 | 2014-11-03 | 2456965.035 | 14.940 0.017 | $r$ | 1m0-11 |
| 2015-02-04 | 2457058.402 | 19.380 0.157 | $V$ | 1m0-12 | 2014-11-09 | 2456970.952 | 14.951 0.085 | $r$ | 1m0-11 |
| 2015-03-03 | 2457084.534 | < 18.895 | $V$ | 1m0-04 | 2014-11-15 | 2456977.201 | 15.092 0.033 | $r$ | 1m0-03 |

(a) Data have not been corrected for extinction
(b) *Swift* Telescope; LSQ (La Silla Quest, Chile); 1m0-08 (McDonald Observatory, USA); 1m0-10, 1m0-12, 1m0-13 (Sutherland, South Africa), 1m0-04, 1m0-05, 1m0-09 (Cerro Tololo, Chile); 1m0-03, 1m0-11 (Siding Spring, Australia).

**Table D1:** ASASSN-14ha: Photometric Data

| Date | JD | mag[(a)] | Filter | telescope[(b)] | Date | JD | mag[(a)] | Filter | telescope[(b)] |
|---|---|---|---|---|---|---|---|---|---|
| 2014-11-21 | 2456982.728 | 14.958 0.029 | $r$ | 1m0-05 | 2015-02-08 | 2457062.049 | 18.706 0.095 | $r$ | 1m0-03 |
| 2014-11-21 | 2456982.728 | 14.944 0.027 | $r$ | 1m0-05 | 2015-02-10 | 2457064.366 | 18.712 0.081 | $r$ | 1m0-12 |
| 2014-11-27 | 2456989.419 | 14.905 0.020 | $r$ | 1m0-10 | 2015-02-10 | 2457064.368 | 18.618 0.057 | $r$ | 1m0-12 |
| 2014-11-27 | 2456989.420 | 14.942 0.021 | $r$ | 1m0-10 | 2015-02-11 | 2457065.011 | 18.544 0.041 | $r$ | 1m0-11 |
| 2014-12-04 | 2456996.190 | 14.957 0.016 | $r$ | 1m0-03 | 2015-02-11 | 2457065.014 | 18.619 0.065 | $r$ | 1m0-11 |
| 2014-12-04 | 2456996.190 | 14.987 0.017 | $r$ | 1m0-03 | 2015-02-16 | 2457069.944 | 18.531 0.107 | $r$ | 1m0-11 |
| 2014-12-10 | 2457001.824 | 14.941 0.028 | $r$ | 1m0-05 | 2015-02-16 | 2457069.946 | 18.496 0.110 | $r$ | 1m0-11 |
| 2014-12-10 | 2457001.825 | 14.936 0.029 | $r$ | 1m0-05 | 2015-03-03 | 2457084.535 | 18.739 0.057 | $r$ | 1m0-09 |
| 2014-12-11 | 2457002.751 | 14.936 0.019 | $r$ | 1m0-05 | 2015-03-03 | 2457084.539 | 18.707 0.066 | $r$ | 1m0-09 |
| 2014-12-11 | 2457002.752 | 14.941 0.018 | $r$ | 1m0-05 | 2015-03-08 | 2457089.551 | 18.598 0.041 | $r$ | 1m0-04 |
| 2014-12-16 | 2457008.458 | 14.918 0.018 | $r$ | 1m0-12 | 2015-03-08 | 2457089.555 | 18.754 0.060 | $r$ | 1m0-04 |
| 2014-12-16 | 2457008.458 | 14.904 0.018 | $r$ | 1m0-12 | 2015-03-09 | 2457090.558 | 18.700 0.046 | $r$ | 1m0-09 |
| 2014-12-22 | 2457014.297 | 14.960 0.024 | $r$ | 1m0-10 | 2015-03-09 | 2457090.563 | 18.574 0.050 | $r$ | 1m0-09 |
| 2014-12-22 | 2457014.298 | 14.853 0.029 | $r$ | 1m0-10 | 2015-03-11 | 2457092.518 | 18.687 0.055 | $r$ | 1m0-09 |
| 2014-12-22 | 2457014.324 | 14.970 0.017 | $r$ | 1m0-13 | 2015-03-11 | 2457092.523 | 18.904 0.067 | $r$ | 1m0-09 |
| 2014-12-22 | 2457014.325 | 14.883 0.037 | $r$ | 1m0-13 | 2014-09-11 | 2456912.287 | 15.161 0.016 | $i$ | 1m0-11 |
| 2014-12-23 | 2457015.330 | 14.797 0.032 | $r$ | 1m0-12 | 2014-09-11 | 2456912.288 | 15.098 0.017 | $i$ | 1m0-11 |
| 2014-12-23 | 2457015.332 | 15.014 0.044 | $r$ | 1m0-12 | 2014-09-13 | 2456913.564 | 15.213 0.024 | $i$ | 1m0-12 |
| 2014-12-25 | 2457017.343 | 14.905 0.023 | $r$ | 1m0-12 | 2014-09-13 | 2456913.566 | 15.211 0.020 | $i$ | 1m0-12 |
| 2014-12-25 | 2457017.344 | 14.880 0.024 | $r$ | 1m0-12 | 2014-09-13 | 2456913.631 | 15.243 0.021 | $i$ | 1m0-12 |
| 2014-12-25 | 2457017.369 | 14.807 0.021 | $r$ | 1m0-12 | 2014-09-13 | 2456913.633 | 15.244 0.019 | $i$ | 1m0-12 |
| 2014-12-25 | 2457017.371 | 14.996 0.018 | $r$ | 1m0-12 | 2014-09-14 | 2456914.607 | 15.121 0.019 | $i$ | 1m0-10 |
| 2014-12-27 | 2457019.384 | 15.001 0.017 | $r$ | 1m0-10 | 2014-09-14 | 2456914.608 | 15.196 0.017 | $i$ | 1m0-10 |
| 2014-12-27 | 2457019.385 | 14.964 0.018 | $r$ | 1m0-10 | 2014-09-14 | 2456914.895 | 15.234 0.008 | $i$ | 1m0-05 |
| 2014-12-31 | 2457022.761 | 14.984 0.024 | $r$ | 1m0-05 | 2014-09-14 | 2456914.897 | 15.259 0.008 | $i$ | 1m0-05 |
| 2014-12-31 | 2457022.762 | 15.037 0.021 | $r$ | 1m0-05 | 2014-09-14 | 2456915.114 | 15.225 0.024 | $i$ | 1m0-03 |
| 2015-01-02 | 2457025.058 | 15.069 0.019 | $r$ | 1m0-11 | 2014-09-14 | 2456915.116 | 15.197 0.024 | $i$ | 1m0-03 |
| 2015-01-02 | 2457025.059 | 15.030 0.020 | $r$ | 1m0-11 | 2014-09-14 | 2456915.272 | 15.156 0.022 | $i$ | 1m0-11 |
| 2015-01-03 | 2457026.476 | 15.127 0.020 | $r$ | 1m0-12 | 2014-09-14 | 2456915.273 | 15.153 0.021 | $i$ | 1m0-11 |
| 2015-01-03 | 2457026.478 | 15.118 0.020 | $r$ | 1m0-12 | 2014-09-14 | 2456915.295 | 15.091 0.023 | $i$ | 1m0-11 |
| 2015-01-05 | 2457028.341 | 15.064 0.018 | $r$ | 1m0-10 | 2014-09-14 | 2456915.297 | 15.140 0.021 | $i$ | 1m0-11 |
| 2015-01-05 | 2457028.342 | 15.099 0.018 | $r$ | 1m0-10 | 2014-09-15 | 2456916.497 | 15.193 0.018 | $i$ | 1m0-12 |
| 2015-01-05 | 2457028.365 | 15.088 0.019 | $r$ | 1m0-12 | 2014-09-15 | 2456916.498 | 15.187 0.018 | $i$ | 1m0-12 |
| 2015-01-05 | 2457028.366 | 15.084 0.019 | $r$ | 1m0-12 | 2014-09-16 | 2456916.829 | 15.152 0.011 | $i$ | 1m0-09 |
| 2015-01-09 | 2457031.980 | 15.237 0.023 | $r$ | 1m0-03 | 2014-09-16 | 2456917.257 | 15.074 0.036 | $i$ | 1m0-11 |
| 2015-01-09 | 2457031.981 | 15.167 0.025 | $r$ | 1m0-03 | 2014-09-18 | 2456918.768 | 15.054 0.011 | $i$ | 1m0-04 |
| 2015-01-11 | 2457034.331 | 15.199 0.019 | $r$ | 1m0-12 | 2014-09-20 | 2456920.831 | 15.325 0.043 | $i$ | 1m0-05 |
| 2015-01-11 | 2457034.333 | 15.252 0.018 | $r$ | 1m0-12 | 2014-09-20 | 2456920.893 | 15.218 0.010 | $i$ | 1m0-09 |
| 2015-01-13 | 2457036.473 | 15.326 0.030 | $r$ | 1m0-13 | 2014-09-22 | 2456922.866 | 15.075 0.025 | $i$ | 1m0-09 |
| 2015-01-13 | 2457036.475 | 15.362 0.017 | $r$ | 1m0-13 | 2014-09-22 | 2456922.867 | 15.164 0.009 | $i$ | 1m0-09 |
| 2015-01-15 | 2457038.110 | 15.303 0.024 | $r$ | 1m0-11 | 2014-09-25 | 2456925.893 | 15.121 0.011 | $i$ | 1m0-04 |
| 2015-01-15 | 2457038.111 | 15.299 0.022 | $r$ | 1m0-11 | 2014-09-26 | 2456926.638 | 15.174 0.020 | $i$ | 1m0-12 |
| 2015-01-17 | 2457039.732 | 15.352 0.022 | $r$ | 1m0-05 | 2014-09-26 | 2456926.639 | 15.160 0.022 | $i$ | 1m0-12 |
| 2015-01-17 | 2457039.733 | 15.341 0.021 | $r$ | 1m0-05 | 2014-09-30 | 2456931.176 | 15.039 0.019 | $i$ | 1m0-11 |
| 2015-01-18 | 2457041.469 | 15.443 0.019 | $r$ | 1m0-12 | 2014-09-30 | 2456931.177 | 15.115 0.020 | $i$ | 1m0-11 |
| 2015-01-18 | 2457041.471 | 15.389 0.020 | $r$ | 1m0-12 | 2014-10-02 | 2456933.072 | 14.975 0.019 | $i$ | 1m0-11 |
| 2015-01-20 | 2457043.308 | 15.515 0.018 | $r$ | 1m0-10 | 2014-10-02 | 2456933.073 | 15.098 0.018 | $i$ | 1m0-11 |
| 2015-01-20 | 2457043.310 | 15.442 0.020 | $r$ | 1m0-10 | 2014-10-04 | 2456934.554 | 15.123 0.019 | $i$ | 1m0-12 |
| 2015-01-22 | 2457045.329 | 15.802 0.019 | $r$ | 1m0-10 | 2014-10-04 | 2456934.555 | 15.126 0.021 | $i$ | 1m0-12 |
| 2015-01-22 | 2457045.332 | 15.912 0.020 | $r$ | 1m0-10 | 2014-10-05 | 2456936.270 | 15.041 0.021 | $i$ | 1m0-11 |
| 2015-01-25 | 2457047.979 | 17.046 0.030 | $r$ | 1m0-11 | 2014-10-05 | 2456936.271 | 15.087 0.028 | $i$ | 1m0-11 |
| 2015-01-25 | 2457047.982 | 16.945 0.031 | $r$ | 1m0-11 | 2014-10-07 | 2456938.050 | 15.028 0.019 | $i$ | 1m0-11 |
| 2015-01-28 | 2457051.418 | 18.374 0.052 | $r$ | 1m0-10 | 2014-10-07 | 2456938.050 | 15.069 0.021 | $i$ | 1m0-11 |
| 2015-01-28 | 2457051.421 | 18.457 0.055 | $r$ | 1m0-10 | 2014-10-09 | 2456940.041 | 15.135 0.020 | $i$ | 1m0-03 |
| 2015-01-30 | 2457053.025 | 18.480 0.078 | $r$ | 1m0-11 | 2014-10-09 | 2456940.041 | 15.104 0.021 | $i$ | 1m0-11 |
| 2015-01-30 | 2457053.028 | 18.535 0.072 | $r$ | 1m0-11 | 2014-10-11 | 2456942.033 | 15.092 0.029 | $i$ | 1m0-03 |
| 2015-02-01 | 2457055.031 | 18.625 0.090 | $r$ | 1m0-11 | 2014-10-11 | 2456942.034 | 15.050 0.031 | $i$ | 1m0-03 |
| 2015-02-04 | 2457058.402 | 18.771 0.098 | $r$ | 1m0-10 | 2014-10-17 | 2456948.021 | 14.999 0.023 | $i$ | 1m0-03 |
| 2015-02-06 | 2457060.313 | 18.482 0.059 | $r$ | 1m0-12 | 2014-10-17 | 2456948.022 | 15.033 0.026 | $i$ | 1m0-03 |
| 2015-02-06 | 2457060.315 | 18.544 0.056 | $r$ | 1m0-12 | 2014-10-22 | 2456953.358 | 14.883 0.023 | $i$ | 1m0-12 |

(a) Data have not been corrected for extinction
(b) *Swift* Telescope; LSQ (La Silla Quest, Chile); 1m0-08 (McDonald Observatory, USA); 1m0-10, 1m0-12, 1m0-13 (Sutherland, South Africa), 1m0-04, 1m0-05, 1m0-09 (Cerro Tololo, Chile); 1m0-03, 1m0-11 (Siding Spring, Australia).

**Table D1:** ASASSN-14ha: Photometric Data

| Date | JD | mag$^{(a)}$ | Filter | telescope$^{(b)}$ | Date | JD | mag$^{(a)}$ | Filter | telescope$^{(b)}$ |
|---|---|---|---|---|---|---|---|---|---|
| 2014-10-22 | 2456953.359 | 14.890 0.024 | $i$ | 1m0-12 | 2015-01-13 | 2457036.479 | 15.242 0.030 | $i$ | 1m0-13 |
| 2014-10-28 | 2456959.109 | 14.924 0.020 | $i$ | 1m0-11 | 2015-01-15 | 2457038.113 | 15.309 0.021 | $i$ | 1m0-11 |
| 2014-11-03 | 2456965.036 | 14.946 0.019 | $i$ | 1m0-11 | 2015-01-15 | 2457038.114 | 15.301 0.022 | $i$ | 1m0-11 |
| 2014-11-03 | 2456965.036 | 14.842 0.020 | $i$ | 1m0-11 | 2015-01-17 | 2457039.735 | 15.281 0.024 | $i$ | 1m0-05 |
| 2014-11-09 | 2456970.954 | 15.028 0.145 | $i$ | 1m0-11 | 2015-01-17 | 2457039.737 | 15.265 0.024 | $i$ | 1m0-05 |
| 2014-11-15 | 2456977.202 | 15.053 0.033 | $i$ | 1m0-03 | 2015-01-18 | 2457041.472 | 15.228 0.023 | $i$ | 1m0-12 |
| 2014-11-15 | 2456977.203 | 14.998 0.033 | $i$ | 1m0-03 | 2015-01-18 | 2457041.474 | 15.270 0.021 | $i$ | 1m0-12 |
| 2014-11-21 | 2456982.729 | 14.848 0.031 | $i$ | 1m0-05 | 2015-01-20 | 2457043.312 | 15.393 0.017 | $i$ | 1m0-10 |
| 2014-11-21 | 2456982.730 | 14.886 0.028 | $i$ | 1m0-05 | 2015-01-20 | 2457043.313 | 15.491 0.019 | $i$ | 1m0-10 |
| 2014-11-27 | 2456989.421 | 14.871 0.021 | $i$ | 1m0-10 | 2015-01-22 | 2457045.335 | 15.722 0.026 | $i$ | 1m0-10 |
| 2014-11-27 | 2456989.422 | 14.885 0.020 | $i$ | 1m0-10 | 2015-01-22 | 2457045.337 | 15.753 0.021 | $i$ | 1m0-10 |
| 2014-12-04 | 2456996.191 | 14.820 0.019 | $i$ | 1m0-03 | 2015-01-25 | 2457047.984 | 16.973 0.074 | $i$ | 1m0-11 |
| 2014-12-04 | 2456996.192 | 14.873 0.018 | $i$ | 1m0-03 | 2015-01-25 | 2457047.987 | 16.911 0.065 | $i$ | 1m0-11 |
| 2014-12-11 | 2457002.753 | 14.887 0.019 | $i$ | 1m0-05 | 2015-01-28 | 2457051.423 | 17.866 0.041 | $i$ | 1m0-10 |
| 2014-12-11 | 2457002.753 | 14.891 0.020 | $i$ | 1m0-05 | 2015-01-28 | 2457051.426 | 17.910 0.048 | $i$ | 1m0-10 |
| 2014-12-16 | 2457008.459 | 14.819 0.019 | $i$ | 1m0-12 | 2015-01-30 | 2457053.030 | 17.939 0.054 | $i$ | 1m0-11 |
| 2014-12-16 | 2457008.460 | 14.862 0.020 | $i$ | 1m0-12 | 2015-01-30 | 2457053.033 | 17.992 0.069 | $i$ | 1m0-11 |
| 2014-12-22 | 2457014.300 | 14.929 0.020 | $i$ | 1m0-10 | 2015-02-01 | 2457055.036 | 17.856 0.080 | $i$ | 1m0-11 |
| 2014-12-22 | 2457014.326 | 14.989 0.026 | $i$ | 1m0-13 | 2015-02-01 | 2457055.039 | 17.737 0.070 | $i$ | 1m0-11 |
| 2014-12-22 | 2457014.327 | 15.062 0.025 | $i$ | 1m0-13 | 2015-02-03 | 2457056.930 | 17.837 0.062 | $i$ | 1m0-03 |
| 2014-12-23 | 2457015.334 | 14.862 0.021 | $i$ | 1m0-12 | 2015-02-03 | 2457056.932 | 17.971 0.067 | $i$ | 1m0-03 |
| 2014-12-23 | 2457015.335 | 14.921 0.019 | $i$ | 1m0-12 | 2015-02-04 | 2457058.405 | 18.027 0.062 | $i$ | 1m0-10 |
| 2014-12-25 | 2457017.372 | 14.962 0.019 | $i$ | 1m0-12 | 2015-02-04 | 2457058.407 | 18.213 0.100 | $i$ | 1m0-10 |
| 2014-12-25 | 2457017.374 | 14.941 0.019 | $i$ | 1m0-12 | 2015-02-06 | 2457060.318 | 18.137 0.066 | $i$ | 1m0-12 |
| 2014-12-27 | 2457019.387 | 14.955 0.016 | $i$ | 1m0-10 | 2015-02-06 | 2457060.320 | 18.098 0.066 | $i$ | 1m0-12 |
| 2014-12-27 | 2457019.389 | 14.929 0.015 | $i$ | 1m0-10 | 2015-02-08 | 2457062.054 | 18.187 0.074 | $i$ | 1m0-03 |
| 2014-12-31 | 2457022.764 | 14.952 0.026 | $i$ | 1m0-05 | 2015-02-08 | 2457062.057 | 18.129 0.084 | $i$ | 1m0-03 |
| 2014-12-31 | 2457022.766 | 14.954 0.027 | $i$ | 1m0-05 | 2015-02-10 | 2457064.371 | 17.964 0.060 | $i$ | 1m0-12 |
| 2015-01-02 | 2457025.061 | 14.979 0.020 | $i$ | 1m0-11 | 2015-02-10 | 2457064.373 | 18.010 0.042 | $i$ | 1m0-12 |
| 2015-01-02 | 2457025.063 | 14.982 0.020 | $i$ | 1m0-11 | 2015-02-11 | 2457065.017 | 18.043 0.058 | $i$ | 1m0-11 |
| 2015-01-03 | 2457026.479 | 15.071 0.022 | $i$ | 1m0-12 | 2015-02-11 | 2457065.019 | 18.030 0.056 | $i$ | 1m0-11 |
| 2015-01-03 | 2457026.481 | 15.053 0.022 | $i$ | 1m0-12 | 2015-02-16 | 2457069.949 | 17.848 0.130 | $i$ | 1m0-11 |
| 2015-01-05 | 2457028.346 | 15.087 0.018 | $i$ | 1m0-10 | 2015-03-03 | 2457084.543 | 18.241 0.041 | $i$ | 1m0-09 |
| 2015-01-05 | 2457028.368 | 15.039 0.017 | $i$ | 1m0-12 | 2015-03-03 | 2457084.547 | 18.211 0.046 | $i$ | 1m0-09 |
| 2015-01-09 | 2457031.983 | 15.133 0.023 | $i$ | 1m0-03 | 2015-03-08 | 2457089.559 | 18.196 0.042 | $i$ | 1m0-04 |
| 2015-01-09 | 2457031.985 | 15.107 0.021 | $i$ | 1m0-03 | 2015-03-08 | 2457089.563 | 18.345 0.068 | $i$ | 1m0-04 |
| 2015-01-11 | 2457034.335 | 15.183 0.020 | $i$ | 1m0-12 | 2015-03-09 | 2457090.568 | 18.109 0.038 | $i$ | 1m0-09 |
| 2015-01-11 | 2457034.336 | 15.115 0.020 | $i$ | 1m0-12 | 2015-03-09 | 2457090.573 | 18.199 0.044 | $i$ | 1m0-09 |
| 2015-01-13 | 2457036.477 | 15.177 0.030 | $i$ | 1m0-13 | 2015-03-11 | 2457092.529 | 18.217 0.029 | $i$ | 1m0-09 |

(a) Data have not been corrected for extinction
(b) *Swift* Telescope; LSQ (La Silla Quest, Chile); 1m0-08 (McDonald Observatory, USA); 1m0-10, 1m0-12, 1m0-13 (Sutherland, South Africa), 1m0-04, 1m0-05, 1m0-09 (Cerro Tololo, Chile); 1m0-03, 1m0-11 (Siding Spring, Australia).

**Table D1:** ASASSN-14dq: Photometric Data

| Date | JD | mag[(a)] | Filter | telescope[(b)] | Date | JD | mag[(a)] | Filter | telescope[(b)] |
|---|---|---|---|---|---|---|---|---|---|
| 2014-07-10 | 2456849.241 | 15.966 0.039 | *B* | 1m0-11 | 2014-11-20 | 2456981.628 | 20.588 0.110 | *B* | 1m0-08 |
| 2014-07-10 | 2456849.244 | 15.984 0.040 | *B* | 1m0-11 | 2014-11-25 | 2456986.643 | 20.410 0.109 | *B* | 1m0-08 |
| 2014-07-12 | 2456850.577 | 15.957 0.018 | *B* | 1m0-12 | 2014-11-25 | 2456986.650 | 20.494 0.123 | *B* | 1m0-08 |
| 2014-07-12 | 2456850.579 | 15.996 0.017 | *B* | 1m0-12 | 2014-11-28 | 2456989.536 | 20.527 0.116 | *B* | 1m0-08 |
| 2014-07-22 | 2456860.554 | 16.192 0.015 | *B* | 1m0-13 | 2014-11-28 | 2456989.543 | 20.607 0.109 | *B* | 1m0-08 |
| 2014-07-22 | 2456860.556 | 16.355 0.017 | *B* | 1m0-13 | 2014-11-28 | 2456989.649 | 20.277 0.099 | *B* | 1m0-08 |
| 2014-07-24 | 2456862.554 | 16.257 0.035 | *B* | 1m0-10 | 2014-11-28 | 2456989.656 | 20.461 0.175 | *B* | 1m0-08 |
| 2014-07-24 | 2456862.557 | 16.231 0.035 | *B* | 1m0-10 | 2014-11-30 | 2456991.622 | 20.546 0.201 | *B* | 1m0-08 |
| 2014-07-26 | 2456864.830 | 16.470 0.024 | *B* | 1m0-08 | 2014-11-30 | 2456991.629 | 20.559 0.170 | *B* | 1m0-08 |
| 2014-07-26 | 2456864.833 | 16.475 0.018 | *B* | 1m0-08 | 2014-12-02 | 2456993.633 | 20.506 0.245 | *B* | 1m0-08 |
| 2014-07-28 | 2456867.188 | 16.604 0.015 | *B* | 1m0-11 | 2014-12-14 | 2457005.551 | 20.480 0.143 | *B* | 1m0-08 |
| 2014-07-28 | 2456867.191 | 16.609 0.036 | *B* | 1m0-11 | 2014-12-14 | 2457005.558 | 20.966 0.161 | *B* | 1m0-08 |
| 2014-07-30 | 2456869.163 | 16.776 0.013 | *B* | 1m0-03 | 2014-12-15 | 2457006.551 | 20.520 0.152 | *B* | 1m0-08 |
| 2014-07-30 | 2456869.165 | 16.703 0.016 | *B* | 1m0-03 | 2014-12-15 | 2457006.558 | 20.633 0.165 | *B* | 1m0-08 |
| 2014-08-01 | 2456871.179 | 16.919 0.018 | *B* | 1m0-11 | 2014-12-16 | 2457007.537 | 20.540 0.181 | *B* | 1m0-08 |
| 2014-08-01 | 2456871.182 | 16.864 0.016 | *B* | 1m0-11 | 2014-12-16 | 2457007.544 | 20.582 0.148 | *B* | 1m0-08 |
| 2014-08-02 | 2456872.181 | 16.883 0.017 | *B* | 1m0-03 | 2014-12-29 | 2457020.565 | 20.919 0.353 | *B* | 1m0-08 |
| 2014-08-02 | 2456872.183 | 16.901 0.017 | *B* | 1m0-03 | 2014-12-30 | 2457021.559 | 21.098 0.430 | *B* | 1m0-08 |
| 2014-08-03 | 2456873.466 | 16.968 0.020 | *B* | 1m0-10 | 2014-07-12 | 2456850.585 | 15.879 0.015 | *g* | 1m0-12 |
| 2014-08-03 | 2456873.468 | 16.969 0.023 | *B* | 1m0-10 | 2014-07-12 | 2456850.588 | 15.845 0.014 | *g* | 1m0-12 |
| 2014-08-05 | 2456875.072 | 17.027 0.018 | *B* | 1m0-03 | 2014-07-22 | 2456860.562 | 16.009 0.016 | *g* | 1m0-13 |
| 2014-08-05 | 2456875.075 | 17.015 0.018 | *B* | 1m0-03 | 2014-07-22 | 2456860.565 | 16.060 0.009 | *g* | 1m0-13 |
| 2014-08-09 | 2456879.153 | 17.090 0.026 | *B* | 1m0-11 | 2014-07-24 | 2456862.563 | 16.138 0.013 | *g* | 1m0-10 |
| 2014-08-09 | 2456879.156 | 17.105 0.028 | *B* | 1m0-11 | 2014-07-24 | 2456862.565 | 16.119 0.010 | *g* | 1m0-10 |
| 2014-08-14 | 2456884.457 | 17.216 0.029 | *B* | 1m0-13 | 2014-07-26 | 2456864.839 | 16.227 0.015 | *g* | 1m0-08 |
| 2014-08-14 | 2456884.459 | 17.242 0.033 | *B* | 1m0-13 | 2014-07-26 | 2456864.841 | 16.205 0.015 | *g* | 1m0-08 |
| 2014-08-20 | 2456890.069 | 17.346 0.021 | *B* | 1m0-11 | 2014-07-28 | 2456867.197 | 16.289 0.011 | *g* | 1m0-11 |
| 2014-08-20 | 2456890.071 | 17.403 0.021 | *B* | 1m0-11 | 2014-07-30 | 2456869.171 | 16.331 0.015 | *g* | 1m0-03 |
| 2014-08-20 | 2456890.154 | 17.410 0.022 | *B* | 1m0-03 | 2014-07-30 | 2456869.174 | 16.352 0.015 | *g* | 1m0-03 |
| 2014-08-20 | 2456890.156 | 17.385 0.020 | *B* | 1m0-03 | 2014-08-01 | 2456871.188 | 16.501 0.010 | *g* | 1m0-11 |
| 2014-08-26 | 2456896.470 | 17.558 0.034 | *B* | 1m0-10 | 2014-08-01 | 2456871.190 | 16.485 0.010 | *g* | 1m0-11 |
| 2014-08-26 | 2456896.472 | 17.594 0.025 | *B* | 1m0-10 | 2014-08-02 | 2456872.189 | 16.523 0.010 | *g* | 1m0-03 |
| 2014-09-07 | 2456908.090 | 17.899 0.077 | *B* | 1m0-03 | 2014-08-02 | 2456872.192 | 16.519 0.011 | *g* | 1m0-03 |
| 2014-09-07 | 2456908.092 | 17.734 0.072 | *B* | 1m0-03 | 2014-08-03 | 2456873.475 | 16.571 0.024 | *g* | 1m0-10 |
| 2014-09-10 | 2456911.419 | 17.778 0.033 | *B* | 1m0-12 | 2014-08-03 | 2456873.477 | 16.587 0.018 | *g* | 1m0-10 |
| 2014-09-10 | 2456911.422 | 17.727 0.046 | *B* | 1m0-12 | 2014-08-05 | 2456875.081 | 16.552 0.013 | *g* | 1m0-03 |
| 2014-09-17 | 2456918.045 | 17.947 0.023 | *B* | 1m0-03 | 2014-08-05 | 2456875.083 | 16.559 0.012 | *g* | 1m0-03 |
| 2014-09-17 | 2456918.049 | 17.953 0.025 | *B* | 1m0-03 | 2014-08-09 | 2456879.162 | 16.625 0.018 | *g* | 1m0-11 |
| 2014-09-29 | 2456930.051 | 17.941 0.216 | *B* | 1m0-11 | 2014-08-09 | 2456879.164 | 16.598 0.018 | *g* | 1m0-11 |
| 2014-10-03 | 2456934.252 | 18.482 0.058 | *B* | 1m0-10 | 2014-08-14 | 2456884.465 | 16.754 0.016 | *g* | 1m0-13 |
| 2014-10-03 | 2456934.258 | 18.566 0.062 | *B* | 1m0-10 | 2014-08-14 | 2456884.468 | 16.799 0.016 | *g* | 1m0-13 |
| 2014-10-06 | 2456936.971 | 18.648 0.123 | *B* | 1m0-03 | 2014-08-20 | 2456890.077 | 16.838 0.013 | *g* | 1m0-11 |
| 2014-10-06 | 2456936.976 | 18.841 0.126 | *B* | 1m0-03 | 2014-08-20 | 2456890.080 | 16.851 0.013 | *g* | 1m0-11 |
| 2014-10-10 | 2456940.601 | 19.121 0.071 | *B* | 1m0-08 | 2014-08-20 | 2456890.162 | 16.858 0.011 | *g* | 1m0-03 |
| 2014-10-10 | 2456940.606 | 19.092 0.089 | *B* | 1m0-08 | 2014-08-20 | 2456890.165 | 16.883 0.011 | *g* | 1m0-03 |
| 2014-10-12 | 2456942.699 | 19.410 0.073 | *B* | 1m0-08 | 2014-08-26 | 2456896.478 | 16.961 0.012 | *g* | 1m0-10 |
| 2014-10-12 | 2456942.704 | 19.422 0.064 | *B* | 1m0-08 | 2014-08-26 | 2456896.481 | 16.971 0.011 | *g* | 1m0-10 |
| 2014-10-15 | 2456945.632 | 19.773 0.055 | *B* | 1m0-08 | 2014-09-07 | 2456908.098 | 17.117 0.171 | *g* | 1m0-03 |
| 2014-10-15 | 2456945.637 | 19.628 0.055 | *B* | 1m0-08 | 2014-09-07 | 2456908.430 | 17.012 0.044 | *g* | 1m0-10 |
| 2014-10-18 | 2456948.598 | 19.999 0.070 | *B* | 1m0-08 | 2014-09-07 | 2456908.433 | 17.143 0.056 | *g* | 1m0-10 |
| 2014-10-18 | 2456948.603 | 19.996 0.076 | *B* | 1m0-08 | 2014-09-10 | 2456911.431 | 17.160 0.026 | *g* | 1m0-12 |
| 2014-10-21 | 2456951.991 | 20.229 0.250 | *B* | 1m0-11 | 2014-09-10 | 2456911.435 | 17.164 0.026 | *g* | 1m0-12 |
| 2014-10-21 | 2456951.995 | 20.078 0.246 | *B* | 1m0-11 | 2014-09-17 | 2456918.058 | 17.339 0.013 | *g* | 1m0-03 |
| 2014-10-23 | 2456954.331 | 20.085 0.086 | *B* | 1m0-13 | 2014-09-17 | 2456918.061 | 17.331 0.013 | *g* | 1m0-03 |
| 2014-10-24 | 2456955.287 | 20.074 0.163 | *B* | 1m0-13 | 2014-09-23 | 2456924.071 | 17.427 0.016 | *g* | 1m0-11 |
| 2014-11-08 | 2456969.696 | 20.772 0.400 | *B* | 1m0-08 | 2014-09-23 | 2456924.074 | 17.409 0.019 | *g* | 1m0-11 |
| 2014-11-08 | 2456969.703 | 20.510 0.308 | *B* | 1m0-08 | 2014-09-29 | 2456930.063 | 17.445 0.038 | *g* | 1m0-11 |
| 2014-11-19 | 2456980.659 | 20.842 0.188 | *B* | 1m0-08 | 2014-09-29 | 2456930.067 | 17.537 0.048 | *g* | 1m0-11 |
| 2014-11-19 | 2456980.666 | 20.686 0.158 | *B* | 1m0-08 | 2014-10-03 | 2456934.298 | 17.848 0.027 | *g* | 1m0-10 |
| 2014-11-20 | 2456981.621 | 20.631 0.150 | *B* | 1m0-08 | 2014-10-03 | 2456934.303 | 17.656 0.030 | *g* | 1m0-10 |

(a) Data have not been corrected for extinction
(b) *Swift* Telescope; LSQ (La Silla Quest, Chile); 1m0-08 (McDonald Observatory, USA); 1m0-10, 1m0-12, 1m0-13 (Sutherland, South Africa), 1m0-04, 1m0-05, 1m0-09 (Cerro Tololo, Chile); 1m0-03, 1m0-11 (Siding Spring, Australia).

**Table D1:** ASASSN-14dq: Photometric Data

| Date | JD | mag[(a)] | Filter | telescope[(b)] | Date | JD | mag[(a)] | Filter | telescope[(b)] |
|---|---|---|---|---|---|---|---|---|---|
| 2014-10-06 | 2456936.972 | 17.911 0.054 | *g* | 1m0-11 | 2014-07-24 | 2456862.561 | 16.081 0.022 | *V* | 1m0-10 |
| 2014-10-06 | 2456936.977 | 17.910 0.042 | *g* | 1m0-11 | 2014-07-26 | 2456864.835 | 16.096 0.022 | *V* | 1m0-08 |
| 2014-10-10 | 2456940.619 | 18.262 0.022 | *g* | 1m0-08 | 2014-07-26 | 2456864.837 | 16.069 0.016 | *V* | 1m0-08 |
| 2014-10-10 | 2456940.624 | 18.317 0.024 | *g* | 1m0-08 | 2014-07-28 | 2456867.193 | 16.089 0.015 | *V* | 1m0-11 |
| 2014-10-12 | 2456942.965 | 18.507 0.032 | *g* | 1m0-11 | 2014-07-28 | 2456867.195 | 16.089 0.015 | *V* | 1m0-11 |
| 2014-10-12 | 2456942.970 | 18.502 0.032 | *g* | 1m0-11 | 2014-07-30 | 2456869.168 | 16.154 0.016 | *V* | 1m0-03 |
| 2014-10-15 | 2456945.686 | 18.895 0.022 | *g* | 1m0-08 | 2014-07-30 | 2456869.170 | 16.131 0.016 | *V* | 1m0-03 |
| 2014-10-15 | 2456945.690 | 18.897 0.025 | *g* | 1m0-08 | 2014-08-01 | 2456871.184 | 16.282 0.013 | *V* | 1m0-11 |
| 2014-10-18 | 2456948.616 | 19.216 0.030 | *g* | 1m0-08 | 2014-08-01 | 2456871.186 | 16.244 0.014 | *V* | 1m0-11 |
| 2014-10-18 | 2456948.621 | 19.250 0.026 | *g* | 1m0-08 | 2014-08-02 | 2456872.186 | 16.248 0.015 | *V* | 1m0-03 |
| 2014-10-21 | 2456952.264 | 19.207 0.040 | *g* | 1m0-13 | 2014-08-02 | 2456872.188 | 16.272 0.014 | *V* | 1m0-03 |
| 2014-10-21 | 2456952.269 | 19.207 0.042 | *g* | 1m0-13 | 2014-08-03 | 2456873.471 | 16.282 0.013 | *V* | 1m0-10 |
| 2014-10-24 | 2456954.753 | 19.449 0.031 | *g* | 1m0-08 | 2014-08-03 | 2456873.473 | 16.262 0.016 | *V* | 1m0-10 |
| 2014-10-27 | 2456957.749 | 19.480 0.031 | *g* | 1m0-08 | 2014-08-05 | 2456875.078 | 16.279 0.015 | *V* | 1m0-03 |
| 2014-10-27 | 2456957.754 | 19.490 0.036 | *g* | 1m0-08 | 2014-08-05 | 2456875.079 | 16.281 0.015 | *V* | 1m0-03 |
| 2014-10-30 | 2456960.890 | 19.429 0.066 | *g* | 1m0-03 | 2014-08-09 | 2456879.158 | 16.413 0.015 | *V* | 1m0-11 |
| 2014-10-30 | 2456960.895 | 19.492 0.053 | *g* | 1m0-03 | 2014-08-09 | 2456879.160 | 16.288 0.016 | *V* | 1m0-11 |
| 2014-11-05 | 2456966.922 | 19.280 0.179 | *g* | 1m0-11 | 2014-08-14 | 2456884.462 | 16.434 0.019 | *V* | 1m0-13 |
| 2014-11-08 | 2456969.718 | 19.510 0.110 | *g* | 1m0-08 | 2014-08-14 | 2456884.464 | 16.400 0.020 | *V* | 1m0-13 |
| 2014-11-08 | 2456969.725 | 19.606 0.113 | *g* | 1m0-08 | 2014-08-20 | 2456890.074 | 16.478 0.014 | *V* | 1m0-11 |
| 2014-11-19 | 2456980.681 | 19.968 0.053 | *g* | 1m0-08 | 2014-08-20 | 2456890.076 | 16.458 0.015 | *V* | 1m0-11 |
| 2014-11-19 | 2456980.688 | 19.938 0.053 | *g* | 1m0-08 | 2014-08-20 | 2456890.159 | 16.538 0.015 | *V* | 1m0-03 |
| 2014-11-20 | 2456981.643 | 19.735 0.040 | *g* | 1m0-08 | 2014-08-20 | 2456890.160 | 16.520 0.016 | *V* | 1m0-03 |
| 2014-11-20 | 2456981.650 | 19.759 0.035 | *g* | 1m0-08 | 2014-08-26 | 2456896.475 | 16.560 0.020 | *V* | 1m0-10 |
| 2014-11-28 | 2456989.558 | 19.752 0.045 | *g* | 1m0-08 | 2014-08-26 | 2456896.477 | 16.574 0.020 | *V* | 1m0-10 |
| 2014-11-28 | 2456989.565 | 19.855 0.052 | *g* | 1m0-08 | 2014-09-07 | 2456908.095 | 16.676 0.035 | *V* | 1m0-03 |
| 2014-11-28 | 2456989.671 | 19.935 0.055 | *g* | 1m0-08 | 2014-09-07 | 2456908.096 | 16.738 0.034 | *V* | 1m0-03 |
| 2014-11-28 | 2456989.678 | 19.780 0.046 | *g* | 1m0-08 | 2014-09-07 | 2456908.427 | 16.675 0.054 | *V* | 1m0-10 |
| 2014-11-30 | 2456991.644 | 19.902 0.091 | *g* | 1m0-08 | 2014-09-07 | 2456908.429 | 16.640 0.054 | *V* | 1m0-10 |
| 2014-11-30 | 2456991.651 | 19.948 0.117 | *g* | 1m0-08 | 2014-09-10 | 2456911.426 | 16.756 0.025 | *V* | 1m0-12 |
| 2014-12-02 | 2456993.655 | 20.046 0.136 | *g* | 1m0-08 | 2014-09-10 | 2456911.429 | 16.744 0.022 | *V* | 1m0-12 |
| 2014-12-02 | 2456993.662 | 20.012 0.155 | *g* | 1m0-08 | 2014-09-17 | 2456918.052 | 16.872 0.015 | *V* | 1m0-03 |
| 2014-12-14 | 2457005.573 | 20.044 0.052 | *g* | 1m0-08 | 2014-09-17 | 2456918.055 | 16.861 0.014 | *V* | 1m0-03 |
| 2014-12-14 | 2457005.580 | 20.029 0.052 | *g* | 1m0-08 | 2014-09-23 | 2456924.066 | 16.820 0.017 | *V* | 1m0-11 |
| 2014-12-15 | 2457006.573 | 20.274 0.083 | *g* | 1m0-08 | 2014-09-23 | 2456924.068 | 16.870 0.016 | *V* | 1m0-11 |
| 2014-12-15 | 2457006.580 | 20.063 0.067 | *g* | 1m0-08 | 2014-09-29 | 2456930.061 | 17.109 0.037 | *V* | 1m0-11 |
| 2014-12-16 | 2457007.559 | 19.951 0.047 | *g* | 1m0-08 | 2014-10-03 | 2456934.263 | 17.294 0.023 | *V* | 1m0-10 |
| 2014-12-16 | 2457007.566 | 19.968 0.046 | *g* | 1m0-08 | 2014-10-03 | 2456934.266 | 17.233 0.024 | *V* | 1m0-10 |
| 2014-12-25 | 2457016.581 | 20.111 0.094 | *g* | 1m0-08 | 2014-10-06 | 2456936.981 | 17.393 0.037 | *V* | 1m0-03 |
| 2014-12-25 | 2457016.588 | 20.380 0.103 | *g* | 1m0-08 | 2014-10-06 | 2456936.985 | 17.341 0.028 | *V* | 1m0-03 |
| 2014-12-29 | 2457020.587 | 20.246 0.154 | *g* | 1m0-08 | 2014-10-10 | 2456940.611 | 17.644 0.021 | *V* | 1m0-08 |
| 2014-12-30 | 2457021.574 | 20.167 0.290 | *g* | 1m0-08 | 2014-10-10 | 2456940.614 | 17.637 0.023 | *V* | 1m0-08 |
| 2014-12-30 | 2457021.581 | 20.063 0.159 | *g* | 1m0-08 | 2014-10-12 | 2456942.709 | 17.936 0.025 | *V* | 1m0-08 |
| 2015-05-22 | 2457164.895 | 20.619 0.102 | *g* | 1m0-09 | 2014-10-12 | 2456942.712 | 17.950 0.020 | *V* | 1m0-08 |
| 2015-05-22 | 2457164.901 | 20.564 0.103 | *g* | 1m0-09 | 2014-10-15 | 2456945.642 | 18.283 0.027 | *V* | 1m0-08 |
| 2015-05-22 | 2457164.910 | 20.976 0.108 | *g* | 1m0-05 | 2014-10-15 | 2456945.646 | 18.306 0.029 | *V* | 1m0-08 |
| 2015-05-22 | 2457164.915 | 21.174 0.119 | *g* | 1m0-05 | 2014-10-18 | 2456948.608 | 18.654 0.024 | *V* | 1m0-08 |
| 2015-05-23 | 2457165.906 | 21.569 0.168 | *g* | 1m0-04 | 2014-10-18 | 2456948.611 | 18.669 0.026 | *V* | 1m0-08 |
| 2015-05-23 | 2457165.911 | 21.969 0.228 | *g* | 1m0-04 | 2014-10-21 | 2456952.000 | 18.812 0.049 | *V* | 1m0-11 |
| 2015-06-06 | 2457179.912 | 21.665 0.496 | *g* | 1m0-09 | 2014-10-21 | 2456952.004 | 18.857 0.065 | *V* | 1m0-11 |
| 2015-06-06 | 2457179.917 | 21.030 0.240 | *g* | 1m0-09 | 2014-10-23 | 2456954.336 | 18.902 0.058 | *V* | 1m0-13 |
| 2014-06-27 | 2456836.000 | $< 17.400$ | *V* | Atel/CBAT | 2014-10-24 | 2456955.292 | 18.993 0.063 | *V* | 1m0-13 |
| 2014-07-08 | 2456847.000 | 15.700 0.100 | *V* | Atel/CBAT | 2014-10-24 | 2456955.296 | 18.970 0.056 | *V* | 1m0-13 |
| 2014-07-10 | 2456849.246 | 15.767 0.149 | *V* | 1m0-11 | 2014-10-30 | 2456961.301 | 18.770 0.067 | *V* | 1m0-13 |
| 2014-07-10 | 2456849.248 | 15.830 0.028 | *V* | 1m0-11 | 2014-11-05 | 2456967.263 | 19.287 0.188 | *V* | 1m0-13 |
| 2014-07-12 | 2456850.582 | 15.796 0.019 | *V* | 1m0-12 | 2014-11-05 | 2456967.266 | 19.125 0.171 | *V* | 1m0-13 |
| 2014-07-12 | 2456850.583 | 15.844 0.020 | *V* | 1m0-12 | 2014-11-05 | 2456967.297 | 18.838 0.109 | *V* | 1m0-10 |
| 2014-07-22 | 2456860.559 | 16.057 0.022 | *V* | 1m0-13 | 2014-11-05 | 2456967.301 | 19.035 0.117 | *V* | 1m0-10 |
| 2014-07-22 | 2456860.561 | 16.030 0.017 | *V* | 1m0-13 | 2014-11-08 | 2456969.711 | 19.000 0.100 | *V* | 1m0-08 |
| 2014-07-24 | 2456862.560 | 16.039 0.017 | *V* | 1m0-10 | 2014-11-08 | 2456969.714 | 19.033 0.104 | *V* | 1m0-08 |

(a) Data have not been corrected for extinction
(b) *Swift* Telescope; LSQ (La Silla Quest, Chile); 1m0-08 (McDonald Observatory, USA); 1m0-10, 1m0-12, 1m0-13 (Sutherland, South Africa), 1m0-04, 1m0-05, 1m0-09 (Cerro Tololo, Chile); 1m0-03, 1m0-11 (Siding Spring, Australia).

**Table D1:** ASASSN-14dq: Photometric Data

| Date | JD | mag$^{(a)}$ | Filter | telescope$^{(b)}$ | Date | JD | mag$^{(a)}$ | Filter | telescope$^{(b)}$ |
|---|---|---|---|---|---|---|---|---|---|
| 2014-11-19 | 2456980.673 | 19.449 0.069 | $V$ | 1m0-08 | 2014-09-17 | 2456918.065 | 16.444 0.011 | $r$ | 1m0-03 |
| 2014-11-19 | 2456980.677 | 19.384 0.063 | $V$ | 1m0-08 | 2014-09-17 | 2456918.068 | 16.452 0.012 | $r$ | 1m0-03 |
| 2014-11-20 | 2456981.635 | 19.165 0.048 | $V$ | 1m0-08 | 2014-09-23 | 2456924.078 | 16.549 0.010 | $r$ | 1m0-11 |
| 2014-11-20 | 2456981.639 | 19.139 0.042 | $V$ | 1m0-08 | 2014-09-23 | 2456924.081 | 16.530 0.011 | $r$ | 1m0-11 |
| 2014-11-25 | 2456986.657 | 19.444 0.065 | $V$ | 1m0-08 | 2014-10-03 | 2456934.308 | 16.730 0.013 | $r$ | 1m0-10 |
| 2014-11-25 | 2456986.661 | 19.276 0.063 | $V$ | 1m0-08 | 2014-10-03 | 2456934.312 | 16.745 0.016 | $r$ | 1m0-10 |
| 2014-11-28 | 2456989.550 | 19.386 0.054 | $V$ | 1m0-08 | 2014-10-06 | 2456936.982 | 16.880 0.022 | $r$ | 1m0-11 |
| 2014-11-28 | 2456989.554 | 19.312 0.040 | $V$ | 1m0-08 | 2014-10-06 | 2456936.986 | 16.849 0.021 | $r$ | 1m0-11 |
| 2014-11-28 | 2456989.663 | 19.389 0.073 | $V$ | 1m0-08 | 2014-10-10 | 2456940.629 | 17.112 0.015 | $r$ | 1m0-08 |
| 2014-11-28 | 2456989.667 | 19.344 0.062 | $V$ | 1m0-08 | 2014-10-10 | 2456940.633 | 17.122 0.015 | $r$ | 1m0-08 |
| 2014-11-29 | 2456990.664 | 19.355 0.126 | $V$ | 1m0-08 | 2014-10-12 | 2456942.975 | 17.313 0.022 | $r$ | 1m0-11 |
| 2014-11-29 | 2456990.667 | 19.342 0.120 | $V$ | 1m0-08 | 2014-10-12 | 2456942.979 | 17.356 0.017 | $r$ | 1m0-11 |
| 2014-11-30 | 2456991.636 | 19.310 0.092 | $V$ | 1m0-08 | 2014-10-15 | 2456945.695 | 17.576 0.015 | $r$ | 1m0-08 |
| 2014-11-30 | 2456991.640 | 19.251 0.076 | $V$ | 1m0-08 | 2014-10-15 | 2456945.699 | 17.598 0.013 | $r$ | 1m0-08 |
| 2014-12-01 | 2456992.588 | 19.191 0.153 | $V$ | 1m0-08 | 2014-10-18 | 2456948.625 | 17.834 0.021 | $r$ | 1m0-08 |
| 2014-12-02 | 2456993.648 | 19.625 0.202 | $V$ | 1m0-08 | 2014-10-18 | 2456948.629 | 17.826 0.021 | $r$ | 1m0-08 |
| 2014-12-02 | 2456993.651 | 19.339 0.121 | $V$ | 1m0-08 | 2014-10-21 | 2456952.274 | 17.970 0.022 | $r$ | 1m0-13 |
| 2014-12-14 | 2457005.565 | 19.529 0.077 | $V$ | 1m0-08 | 2014-10-21 | 2456952.278 | 17.987 0.018 | $r$ | 1m0-13 |
| 2014-12-14 | 2457005.569 | 19.511 0.061 | $V$ | 1m0-08 | 2014-10-24 | 2456954.763 | 18.120 0.021 | $r$ | 1m0-08 |
| 2014-12-15 | 2457006.565 | 19.598 0.090 | $V$ | 1m0-08 | 2014-10-24 | 2456954.766 | 18.141 0.029 | $r$ | 1m0-08 |
| 2014-12-15 | 2457006.569 | 19.411 0.084 | $V$ | 1m0-08 | 2014-10-27 | 2456957.759 | 18.312 0.064 | $r$ | 1m0-08 |
| 2014-12-16 | 2457007.552 | 19.521 0.067 | $V$ | 1m0-08 | 2014-10-27 | 2456957.762 | 18.372 0.078 | $r$ | 1m0-08 |
| 2014-12-16 | 2457007.555 | 19.434 0.048 | $V$ | 1m0-08 | 2014-10-30 | 2456960.900 | 18.205 0.021 | $r$ | 1m0-03 |
| 2014-12-25 | 2457016.573 | 19.273 0.095 | $V$ | 1m0-08 | 2014-10-30 | 2456960.904 | 18.171 0.025 | $r$ | 1m0-03 |
| 2014-12-29 | 2457020.579 | 20.118 0.234 | $V$ | 1m0-08 | 2014-11-05 | 2456966.927 | 18.353 0.062 | $r$ | 1m0-11 |
| 2014-12-30 | 2457021.566 | 20.026 0.295 | $V$ | 1m0-08 | 2014-11-05 | 2456966.930 | 18.237 0.055 | $r$ | 1m0-11 |
| 2014-12-30 | 2457021.570 | 19.516 0.302 | $V$ | 1m0-08 | 2014-11-06 | 2456967.928 | 18.356 0.126 | $r$ | 1m0-11 |
| 2014-07-12 | 2456850.590 | 15.755 0.013 | $r$ | 1m0-12 | 2014-11-06 | 2456967.931 | 18.157 0.122 | $r$ | 1m0-11 |
| 2014-07-12 | 2456850.592 | 15.814 0.013 | $r$ | 1m0-12 | 2014-11-08 | 2456969.733 | 18.638 0.074 | $r$ | 1m0-08 |
| 2014-07-22 | 2456860.568 | 15.820 0.012 | $r$ | 1m0-13 | 2014-11-08 | 2456969.737 | 18.455 0.061 | $r$ | 1m0-08 |
| 2014-07-22 | 2456860.569 | 15.783 0.016 | $r$ | 1m0-13 | 2014-11-14 | 2456975.699 | 18.572 0.063 | $r$ | 1m0-08 |
| 2014-07-24 | 2456862.568 | 15.852 0.011 | $r$ | 1m0-10 | 2014-11-19 | 2456980.695 | 18.537 0.029 | $r$ | 1m0-08 |
| 2014-07-24 | 2456862.570 | 15.870 0.013 | $r$ | 1m0-10 | 2014-11-19 | 2456980.699 | 18.534 0.031 | $r$ | 1m0-08 |
| 2014-07-26 | 2456864.844 | 15.884 0.014 | $r$ | 1m0-08 | 2014-11-20 | 2456981.657 | 18.465 0.021 | $r$ | 1m0-08 |
| 2014-07-26 | 2456864.845 | 15.841 0.010 | $r$ | 1m0-08 | 2014-11-20 | 2456981.661 | 18.479 0.023 | $r$ | 1m0-08 |
| 2014-07-28 | 2456867.203 | 15.933 0.009 | $r$ | 1m0-11 | 2014-11-28 | 2456989.572 | 18.552 0.027 | $r$ | 1m0-08 |
| 2014-07-28 | 2456867.204 | 15.892 0.009 | $r$ | 1m0-11 | 2014-11-28 | 2456989.576 | 18.561 0.027 | $r$ | 1m0-08 |
| 2014-07-30 | 2456869.176 | 15.957 0.013 | $r$ | 1m0-03 | 2014-11-28 | 2456989.686 | 18.600 0.033 | $r$ | 1m0-08 |
| 2014-07-30 | 2456869.178 | 15.959 0.011 | $r$ | 1m0-03 | 2014-11-28 | 2456989.689 | 18.585 0.035 | $r$ | 1m0-08 |
| 2014-08-01 | 2456871.193 | 16.007 0.015 | $r$ | 1m0-11 | 2014-11-30 | 2456991.658 | 18.596 0.047 | $r$ | 1m0-08 |
| 2014-08-02 | 2456872.195 | 16.039 0.009 | $r$ | 1m0-03 | 2014-11-30 | 2456991.662 | 18.503 0.034 | $r$ | 1m0-08 |
| 2014-08-02 | 2456872.196 | 16.022 0.009 | $r$ | 1m0-03 | 2014-12-02 | 2456993.670 | 18.710 0.059 | $r$ | 1m0-08 |
| 2014-08-03 | 2456873.480 | 16.087 0.014 | $r$ | 1m0-10 | 2014-12-02 | 2456993.673 | 18.753 0.073 | $r$ | 1m0-08 |
| 2014-08-03 | 2456873.481 | 16.055 0.010 | $r$ | 1m0-10 | 2014-12-14 | 2457005.587 | 18.721 0.035 | $r$ | 1m0-08 |
| 2014-08-05 | 2456875.086 | 15.987 0.009 | $r$ | 1m0-03 | 2014-12-15 | 2457006.588 | 18.724 0.040 | $r$ | 1m0-08 |
| 2014-08-05 | 2456875.088 | 16.034 0.008 | $r$ | 1m0-03 | 2014-12-15 | 2457006.592 | 18.747 0.043 | $r$ | 1m0-08 |
| 2014-08-09 | 2456879.167 | 16.029 0.011 | $r$ | 1m0-11 | 2014-12-16 | 2457007.574 | 18.649 0.033 | $r$ | 1m0-08 |
| 2014-08-09 | 2456879.168 | 16.044 0.013 | $r$ | 1m0-11 | 2014-12-16 | 2457007.577 | 18.613 0.028 | $r$ | 1m0-08 |
| 2014-08-14 | 2456884.471 | 16.133 0.011 | $r$ | 1m0-13 | 2014-12-25 | 2457016.595 | 18.981 0.051 | $r$ | 1m0-08 |
| 2014-08-14 | 2456884.472 | 16.133 0.012 | $r$ | 1m0-13 | 2014-12-25 | 2457016.599 | 18.935 0.052 | $r$ | 1m0-08 |
| 2014-08-20 | 2456890.083 | 16.128 0.010 | $r$ | 1m0-11 | 2014-12-30 | 2457021.588 | 18.641 0.153 | $r$ | 1m0-08 |
| 2014-08-20 | 2456890.084 | 16.140 0.009 | $r$ | 1m0-11 | 2014-12-30 | 2457021.592 | 19.031 0.164 | $r$ | 1m0-08 |
| 2014-08-20 | 2456890.167 | 16.196 0.011 | $r$ | 1m0-03 | 2015-05-22 | 2457164.906 | 19.824 0.073 | $r$ | 1m0-09 |
| 2014-08-20 | 2456890.169 | 16.218 0.010 | $r$ | 1m0-03 | 2015-05-22 | 2457164.910 | 19.745 0.072 | $r$ | 1m0-09 |
| 2014-08-26 | 2456896.484 | 16.223 0.010 | $r$ | 1m0-10 | 2015-05-22 | 2457164.920 | 20.615 0.130 | $r$ | 1m0-05 |
| 2014-08-26 | 2456896.485 | 16.221 0.010 | $r$ | 1m0-10 | 2015-05-22 | 2457164.923 | 20.761 0.105 | $r$ | 1m0-05 |
| 2014-09-07 | 2456908.436 | 16.287 0.028 | $r$ | 1m0-10 | 2015-05-23 | 2457165.917 | 20.568 0.162 | $r$ | 1m0-04 |
| 2014-09-07 | 2456908.437 | 16.330 0.031 | $r$ | 1m0-10 | 2015-05-23 | 2457165.921 | 20.495 0.212 | $r$ | 1m0-04 |
| 2014-09-10 | 2456911.439 | 16.470 0.017 | $r$ | 1m0-12 | 2015-06-05 | 2457178.835 | 20.340 0.263 | $r$ | 1m0-09 |
| 2014-09-10 | 2456911.441 | 16.385 0.015 | $r$ | 1m0-12 | 2015-06-05 | 2457178.839 | 20.334 0.271 | $r$ | 1m0-09 |

(a) Data have not been corrected for extinction
(b) *Swift* Telescope; LSQ (La Silla Quest, Chile); 1m0-08 (McDonald Observatory, USA); 1m0-10, 1m0-12, 1m0-13 (Sutherland, South Africa), 1m0-04, 1m0-05, 1m0-09 (Cerro Tololo, Chile); 1m0-03, 1m0-11 (Siding Spring, Australia).

**Table D1:** ASASSN-14dq: Photometric Data

| Date | JD | mag[(a)] | Filter | telescope[(b)] | Date | JD | mag[(a)] | Filter | telescope[(b)] |
|---|---|---|---|---|---|---|---|---|---|
| 2015-06-06 | 2457179.923 | 19.390 0.126 | *r* | 1m0-09 | 2014-10-12 | 2456942.982 | 17.302 0.095 | *i* | 1m0-11 |
| 2015-06-06 | 2457179.927 | 19.478 0.155 | *r* | 1m0-09 | 2014-10-12 | 2456942.986 | 17.308 0.058 | *i* | 1m0-11 |
| 2015-06-18 | 2457191.913 | 20.599 0.099 | *r* | 1m0-04 | 2014-10-15 | 2456945.703 | 17.551 0.024 | *i* | 1m0-08 |
| 2015-06-18 | 2457191.917 | 20.546 0.091 | *r* | 1m0-04 | 2014-10-15 | 2456945.707 | 17.529 0.023 | *i* | 1m0-08 |
| 2014-07-12 | 2456850.594 | 15.857 0.015 | *i* | 1m0-12 | 2014-10-18 | 2456948.633 | 17.846 0.027 | *i* | 1m0-08 |
| 2014-07-12 | 2456850.595 | 15.909 0.015 | *i* | 1m0-12 | 2014-10-18 | 2456948.637 | 17.838 0.027 | *i* | 1m0-08 |
| 2014-07-22 | 2456860.571 | 15.927 0.018 | *i* | 1m0-13 | 2014-10-21 | 2456952.282 | 17.997 0.241 | *i* | 1m0-13 |
| 2014-07-22 | 2456860.573 | 16.003 0.014 | *i* | 1m0-13 | 2014-10-21 | 2456952.285 | 18.162 0.132 | *i* | 1m0-13 |
| 2014-07-24 | 2456862.572 | 16.102 0.039 | *i* | 1m0-10 | 2014-10-24 | 2456954.770 | 18.142 0.030 | *i* | 1m0-08 |
| 2014-07-24 | 2456862.573 | 16.027 0.014 | *i* | 1m0-10 | 2014-10-24 | 2456954.774 | 18.169 0.033 | *i* | 1m0-08 |
| 2014-07-26 | 2456864.847 | 16.021 0.016 | *i* | 1m0-08 | 2014-10-27 | 2456957.766 | 17.969 0.029 | *i* | 1m0-08 |
| 2014-07-26 | 2456864.849 | 16.001 0.015 | *i* | 1m0-08 | 2014-10-27 | 2456957.770 | 18.013 0.027 | *i* | 1m0-08 |
| 2014-07-28 | 2456867.206 | 16.033 0.011 | *i* | 1m0-11 | 2014-10-30 | 2456960.908 | 18.045 0.034 | *i* | 1m0-03 |
| 2014-07-30 | 2456869.180 | 16.052 0.018 | *i* | 1m0-03 | 2014-10-30 | 2456960.911 | 18.070 0.030 | *i* | 1m0-03 |
| 2014-07-30 | 2456869.181 | 16.033 0.015 | *i* | 1m0-03 | 2014-11-05 | 2456966.934 | 18.133 0.055 | *i* | 1m0-11 |
| 2014-08-02 | 2456872.198 | 16.130 0.013 | *i* | 1m0-03 | 2014-11-05 | 2456966.938 | 18.041 0.073 | *i* | 1m0-11 |
| 2014-08-02 | 2456872.199 | 16.122 0.015 | *i* | 1m0-03 | 2014-11-06 | 2456967.935 | 18.500 0.244 | *i* | 1m0-11 |
| 2014-08-03 | 2456873.483 | 16.146 0.014 | *i* | 1m0-10 | 2014-11-08 | 2456969.741 | 18.408 0.088 | *i* | 1m0-08 |
| 2014-08-03 | 2456873.485 | 16.115 0.015 | *i* | 1m0-10 | 2014-11-08 | 2456969.744 | 18.241 0.087 | *i* | 1m0-08 |
| 2014-08-05 | 2456875.089 | 16.129 0.012 | *i* | 1m0-03 | 2014-11-14 | 2456975.707 | 18.529 0.110 | *i* | 1m0-08 |
| 2014-08-05 | 2456875.091 | 16.121 0.011 | *i* | 1m0-03 | 2014-11-19 | 2456980.703 | 18.519 0.052 | *i* | 1m0-08 |
| 2014-08-09 | 2456879.170 | 16.110 0.014 | *i* | 1m0-11 | 2014-11-20 | 2456981.665 | 18.378 0.043 | *i* | 1m0-08 |
| 2014-08-09 | 2456879.172 | 16.136 0.016 | *i* | 1m0-11 | 2014-11-20 | 2456981.669 | 18.446 0.039 | *i* | 1m0-08 |
| 2014-08-14 | 2456884.474 | 16.176 0.018 | *i* | 1m0-13 | 2014-11-28 | 2456989.580 | 18.565 0.049 | *i* | 1m0-08 |
| 2014-08-14 | 2456884.476 | 16.221 0.020 | *i* | 1m0-13 | 2014-11-28 | 2456989.583 | 18.580 0.040 | *i* | 1m0-08 |
| 2014-08-20 | 2456890.086 | 16.246 0.012 | *i* | 1m0-11 | 2014-11-28 | 2456989.693 | 18.617 0.065 | *i* | 1m0-08 |
| 2014-08-20 | 2456890.087 | 16.225 0.015 | *i* | 1m0-11 | 2014-11-30 | 2456991.666 | 18.456 0.061 | *i* | 1m0-08 |
| 2014-08-20 | 2456890.171 | 16.303 0.015 | *i* | 1m0-03 | 2014-11-30 | 2456991.669 | 18.594 0.078 | *i* | 1m0-08 |
| 2014-08-20 | 2456890.172 | 16.310 0.019 | *i* | 1m0-03 | 2014-12-02 | 2456993.677 | 18.717 0.096 | *i* | 1m0-08 |
| 2014-08-26 | 2456896.487 | 16.321 0.014 | *i* | 1m0-10 | 2014-12-02 | 2456993.681 | 18.513 0.081 | *i* | 1m0-08 |
| 2014-08-26 | 2456896.488 | 16.330 0.015 | *i* | 1m0-10 | 2014-12-15 | 2457006.595 | 18.879 0.068 | *i* | 1m0-08 |
| 2014-09-07 | 2456908.439 | 16.460 0.039 | *i* | 1m0-10 | 2014-12-15 | 2457006.599 | 18.863 0.071 | *i* | 1m0-08 |
| 2014-09-07 | 2456908.440 | 16.447 0.041 | *i* | 1m0-10 | 2014-12-16 | 2457007.581 | 18.829 0.049 | *i* | 1m0-08 |
| 2014-09-10 | 2456911.444 | 16.446 0.020 | *i* | 1m0-12 | 2014-12-16 | 2457007.585 | 18.651 0.043 | *i* | 1m0-08 |
| 2014-09-10 | 2456911.446 | 16.487 0.019 | *i* | 1m0-12 | 2014-12-30 | 2457021.596 | 19.036 0.350 | *i* | 1m0-08 |
| 2014-09-17 | 2456918.070 | 16.434 0.016 | *i* | 1m0-03 | 2014-12-30 | 2457021.599 | 18.746 0.333 | *i* | 1m0-08 |
| 2014-09-17 | 2456918.073 | 16.489 0.016 | *i* | 1m0-03 | 2015-05-22 | 2457164.914 | 18.692 0.094 | *i* | 1m0-09 |
| 2014-09-23 | 2456924.083 | 16.533 0.014 | *i* | 1m0-11 | 2015-05-22 | 2457164.918 | 18.318 0.107 | *i* | 1m0-09 |
| 2014-09-23 | 2456924.086 | 16.576 0.016 | *i* | 1m0-11 | 2015-05-22 | 2457164.927 | 20.041 0.232 | *i* | 1m0-05 |
| 2014-09-29 | 2456930.076 | 16.741 0.135 | *i* | 1m0-11 | 2015-05-22 | 2457164.931 | 19.898 0.219 | *i* | 1m0-05 |
| 2014-09-29 | 2456930.079 | 16.661 0.096 | *i* | 1m0-11 | 2015-05-23 | 2457165.925 | 20.324 0.180 | *i* | 1m0-04 |
| 2014-10-03 | 2456934.315 | 16.739 0.016 | *i* | 1m0-10 | 2015-05-23 | 2457165.929 | 20.376 0.142 | *i* | 1m0-04 |
| 2014-10-03 | 2456934.319 | 16.752 0.012 | *i* | 1m0-10 | 2015-06-05 | 2457178.847 | 20.785 0.434 | *i* | 1m0-09 |
| 2014-10-06 | 2456936.989 | 16.900 0.025 | *i* | 1m0-11 | 2015-06-06 | 2457179.931 | 19.571 0.263 | *i* | 1m0-09 |
| 2014-10-06 | 2456936.993 | 16.861 0.030 | *i* | 1m0-11 | 2015-06-06 | 2457179.935 | 19.452 0.241 | *i* | 1m0-09 |
| 2014-10-10 | 2456940.636 | 17.091 0.022 | *i* | 1m0-08 | 2015-06-18 | 2457191.921 | 19.573 0.127 | *i* | 1m0-04 |
| 2014-10-10 | 2456940.640 | 17.017 0.016 | *i* | 1m0-08 | 2015-06-18 | 2457191.925 | 19.720 0.160 | *i* | 1m0-04 |

(a) Data have not been corrected for extinction

(b) *Swift* Telescope; LSQ (La Silla Quest, Chile); 1m0-08 (McDonald Observatory, USA); 1m0-10, 1m0-12, 1m0-13 (Sutherland, South Africa), 1m0-04, 1m0-05, 1m0-09 (Cerro Tololo, Chile); 1m0-03, 1m0-11 (Siding Spring, Australia).

**Table D1:** ASASSN-14gm: Photometric Data

| Date | JD | mag[(a)] | Filter | telescope[(b)] | Date | JD | mag[(a)] | Filter | telescope[(b)] |
|---|---|---|---|---|---|---|---|---|---|
| 2014-09-03 | 2456903.529 | 13.756 0.070 | *uw2* | *Swift* | 2014-10-24 | 2456955.094 | 16.686 0.069 | *us* | *Swift* |
| 2014-09-04 | 2456905.125 | 13.848 0.070 | *uw2* | *Swift* | 2014-09-03 | 2456903.526 | 15.391 0.047 | *bs* | *Swift* |
| 2014-09-05 | 2456905.758 | 13.959 0.070 | *uw2* | *Swift* | 2014-09-04 | 2456905.123 | 15.121 0.050 | *bs* | *Swift* |
| 2014-09-06 | 2456906.593 | 14.195 0.071 | *uw2* | *Swift* | 2014-09-05 | 2456905.756 | 15.093 0.049 | *bs* | *Swift* |
| 2014-09-07 | 2456907.750 | 14.415 0.071 | *uw2* | *Swift* | 2014-09-06 | 2456906.592 | 15.116 0.050 | *bs* | *Swift* |
| 2014-09-08 | 2456908.813 | 14.655 0.083 | *uw2* | *Swift* | 2014-09-07 | 2456907.747 | 15.065 0.050 | *bs* | *Swift* |
| 2014-09-09 | 2456909.593 | 14.945 0.072 | *uw2* | *Swift* | 2014-09-08 | 2456908.812 | 15.037 0.050 | *bs* | *Swift* |
| 2014-09-12 | 2456913.412 | 15.553 0.073 | *uw2* | *Swift* | 2014-09-09 | 2456909.591 | 15.108 0.049 | *bs* | *Swift* |
| 2014-09-16 | 2456916.775 | 16.303 0.074 | *uw2* | *Swift* | 2014-09-12 | 2456913.411 | 15.080 0.048 | *bs* | *Swift* |
| 2014-09-20 | 2456921.276 | 17.736 0.081 | *uw2* | *Swift* | 2014-09-16 | 2456916.773 | 15.213 0.048 | *bs* | *Swift* |
| 2014-09-24 | 2456925.209 | 18.302 0.089 | *uw2* | *Swift* | 2014-09-20 | 2456921.273 | 15.307 0.048 | *bs* | *Swift* |
| 2014-09-28 | 2456929.101 | 18.767 0.087 | *uw2* | *Swift* | 2014-09-24 | 2456925.206 | 15.392 0.052 | *bs* | *Swift* |
| 2014-10-04 | 2456934.731 | 19.360 0.184 | *uw2* | *Swift* | 2014-09-28 | 2456929.099 | 15.507 0.050 | *bs* | *Swift* |
| 2014-10-11 | 2456941.772 | 21.080 0.581 | *uw2* | *Swift* | 2014-10-04 | 2456934.729 | 15.680 0.048 | *bs* | *Swift* |
| 2014-10-19 | 2456950.406 | 20.202 0.385 | *uw2* | *Swift* | 2014-10-11 | 2456941.769 | 15.869 0.048 | *bs* | *Swift* |
| 2014-10-22 | 2456953.204 | 19.483 0.341 | *uw2* | *Swift* | 2014-10-19 | 2456950.405 | 16.073 0.051 | *bs* | *Swift* |
| 2014-10-24 | 2456955.096 | 20.756 0.481 | *uw2* | *Swift* | 2014-10-22 | 2456953.203 | 16.046 0.088 | *bs* | *Swift* |
| 2014-09-03 | 2456903.502 | 13.822 0.059 | *um2* | *Swift* | 2014-10-24 | 2456955.094 | 16.076 0.050 | *bs* | *Swift* |
| 2014-09-04 | 2456905.129 | 13.808 0.059 | *um2* | *Swift* | 2014-09-03 | 2456903.627 | 15.324 0.084 | *B* | 1m0-10 |
| 2014-09-05 | 2456905.762 | 13.826 0.059 | *um2* | *Swift* | 2014-09-03 | 2456903.630 | 15.327 0.072 | *B* | 1m0-10 |
| 2014-09-06 | 2456906.597 | 13.994 0.059 | *um2* | *Swift* | 2014-09-03 | 2456903.887 | 15.297 0.043 | *B* | 1m0-09 |
| 2014-09-07 | 2456907.757 | 14.160 0.060 | *um2* | *Swift* | 2014-09-03 | 2456903.890 | 15.297 0.047 | *B* | 1m0-09 |
| 2014-09-09 | 2456909.596 | 14.542 0.060 | *um2* | *Swift* | 2014-09-07 | 2456908.186 | 15.061 0.076 | *B* | 1m0-11 |
| 2014-09-12 | 2456913.313 | 15.259 0.062 | *um2* | *Swift* | 2014-09-07 | 2456908.189 | 15.061 0.066 | *B* | 1m0-11 |
| 2014-09-16 | 2456916.781 | 16.338 0.064 | *um2* | *Swift* | 2014-09-07 | 2456908.268 | 15.050 0.086 | *B* | 1m0-03 |
| 2014-09-20 | 2456921.282 | 17.988 0.072 | *um2* | *Swift* | 2014-09-07 | 2456908.270 | 15.067 0.084 | *B* | 1m0-03 |
| 2014-09-24 | 2456925.216 | 18.608 0.091 | *um2* | *Swift* | 2014-09-12 | 2456913.181 | 15.100 0.090 | *B* | 1m0-11 |
| 2014-09-28 | 2456929.105 | 19.467 0.079 | *um2* | *Swift* | 2014-09-12 | 2456913.183 | 15.136 0.079 | *B* | 1m0-11 |
| 2014-09-03 | 2456903.524 | 13.949 0.058 | *uw1* | *Swift* | 2014-09-14 | 2456915.255 | 15.134 0.078 | *B* | 1m0-03 |
| 2014-09-04 | 2456905.121 | 13.786 0.058 | *uw1* | *Swift* | 2014-09-14 | 2456915.257 | 15.135 0.079 | *B* | 1m0-03 |
| 2014-09-05 | 2456905.755 | 13.901 0.058 | *uw1* | *Swift* | 2014-09-16 | 2456917.177 | 15.116 0.067 | *B* | 1m0-11 |
| 2014-09-06 | 2456906.590 | 13.913 0.058 | *uw1* | *Swift* | 2014-09-16 | 2456917.180 | 15.207 0.067 | *B* | 1m0-11 |
| 2014-09-07 | 2456907.744 | 14.037 0.058 | *uw1* | *Swift* | 2014-09-18 | 2456919.184 | 15.176 0.087 | *B* | 1m0-03 |
| 2014-09-08 | 2456908.809 | 14.119 0.058 | *uw1* | *Swift* | 2014-09-18 | 2456919.187 | 15.171 0.085 | *B* | 1m0-03 |
| 2014-09-09 | 2456909.589 | 14.230 0.058 | *uw1* | *Swift* | 2014-09-20 | 2456921.041 | 15.282 0.073 | *B* | 1m0-03 |
| 2014-09-12 | 2456913.410 | 14.774 0.059 | *uw1* | *Swift* | 2014-09-20 | 2456921.043 | 15.298 0.074 | *B* | 1m0-03 |
| 2014-09-16 | 2456916.771 | 15.375 0.060 | *uw1* | *Swift* | 2014-09-23 | 2456924.037 | 15.279 0.069 | *B* | 1m0-11 |
| 2014-09-20 | 2456921.271 | 16.423 0.066 | *uw1* | *Swift* | 2014-09-23 | 2456924.039 | 15.324 0.069 | *B* | 1m0-11 |
| 2014-09-24 | 2456925.203 | 16.908 0.075 | *uw1* | *Swift* | 2014-09-27 | 2456928.044 | 15.426 0.079 | *B* | 1m0-11 |
| 2014-09-28 | 2456929.097 | 17.591 0.076 | *uw1* | *Swift* | 2014-09-29 | 2456929.893 | 15.495 0.082 | *B* | 1m0-08 |
| 2014-10-04 | 2456934.727 | 18.305 0.073 | *uw1* | *Swift* | 2014-10-02 | 2456933.018 | 15.586 0.063 | *B* | 1m0-11 |
| 2014-10-11 | 2456941.767 | 19.165 0.173 | *uw1* | *Swift* | 2014-10-02 | 2456933.020 | 15.584 0.066 | *B* | 1m0-11 |
| 2014-10-19 | 2456950.404 | 18.984 0.177 | *uw1* | *Swift* | 2014-10-03 | 2456934.212 | 15.451 0.138 | *B* | 1m0-11 |
| 2014-10-22 | 2456953.202 | 19.581 0.160 | *uw1* | *Swift* | 2014-10-03 | 2456934.215 | 15.616 0.055 | *B* | 1m0-11 |
| 2014-10-24 | 2456955.092 | 19.368 0.274 | *uw1* | *Swift* | 2014-10-09 | 2456940.185 | 15.652 0.132 | *B* | 1m0-11 |
| 2014-09-04 | 2456905.122 | 13.882 0.053 | *us* | *Swift* | 2014-10-09 | 2456940.187 | 15.737 0.070 | *B* | 1m0-11 |
| 2014-09-05 | 2456905.756 | 13.894 0.053 | *us* | *Swift* | 2014-10-13 | 2456944.326 | 15.813 0.090 | *B* | 1m0-12 |
| 2014-09-06 | 2456906.591 | 13.920 0.053 | *us* | *Swift* | 2014-10-13 | 2456944.329 | 15.791 0.089 | *B* | 1m0-12 |
| 2014-09-07 | 2456907.746 | 13.905 0.053 | *us* | *Swift* | 2014-10-17 | 2456947.972 | 15.892 0.061 | *B* | 1m0-11 |
| 2014-09-08 | 2456908.811 | 13.934 0.053 | *us* | *Swift* | 2014-10-17 | 2456947.974 | 15.910 0.067 | *B* | 1m0-11 |
| 2014-09-09 | 2456909.591 | 13.935 0.053 | *us* | *Swift* | 2014-10-21 | 2456952.054 | 15.707 0.064 | *B* | 1m0-11 |
| 2014-09-12 | 2456913.411 | 14.131 0.052 | *us* | *Swift* | 2014-10-21 | 2456952.057 | 15.748 0.071 | *B* | 1m0-11 |
| 2014-09-16 | 2456916.773 | 14.401 0.052 | *us* | *Swift* | 2014-10-25 | 2456955.904 | 15.959 0.082 | *B* | 1m0-03 |
| 2014-09-20 | 2456921.273 | 14.831 0.054 | *us* | *Swift* | 2014-10-25 | 2456955.905 | 15.952 0.081 | *B* | 1m0-03 |
| 2014-09-24 | 2456925.205 | 15.345 0.062 | *us* | *Swift* | 2014-11-01 | 2456963.063 | 15.958 0.075 | *B* | 1m0-11 |
| 2014-09-28 | 2456929.099 | 15.715 0.063 | *us* | *Swift* | 2014-11-01 | 2456963.064 | 15.823 0.086 | *B* | 1m0-11 |
| 2014-10-04 | 2456934.729 | 15.961 0.060 | *us* | *Swift* | 2014-11-06 | 2456968.477 | 16.166 0.101 | *B* | 1m0-10 |
| 2014-10-11 | 2456941.768 | 16.330 0.062 | *us* | *Swift* | 2014-11-06 | 2456968.478 | 16.040 0.087 | *B* | 1m0-10 |
| 2014-10-19 | 2456950.404 | 16.584 0.071 | *us* | *Swift* | 2014-11-06 | 2456968.493 | 15.885 0.094 | *B* | 1m0-10 |
| 2014-10-22 | 2456953.203 | 16.462 0.140 | *us* | *Swift* | 2014-11-13 | 2456975.130 | 16.075 0.071 | *B* | 1m0-11 |

(a) Data have not been corrected for extinction
(b) *Swift* Telescope; LSQ (La Silla Quest, Chile); 1m0-08 (McDonald Observatory, USA); 1m0-10, 1m0-12, 1m0-13 (Sutherland, South Africa), 1m0-04, 1m0-05, 1m0-09 (Cerro Tololo, Chile); 1m0-03, 1m0-11 (Siding Spring, Australia).

**Table D1:** ASASSN-14gm: Photometric Data

| Date | JD | mag$^{(a)}$ | Filter | telescope$^{(b)}$ | Date | JD | mag$^{(a)}$ | Filter | telescope$^{(b)}$ |
|---|---|---|---|---|---|---|---|---|---|
| 2014-11-13 | 2456975.132 | 16.201 0.080 | *B* | 1m0-11 | 2015-07-17 | 2457220.755 | 19.062 0.056 | *B* | 1m0-09 |
| 2014-11-18 | 2456980.400 | 16.289 0.066 | *B* | 1m0-10 | 2015-07-17 | 2457220.760 | 19.125 0.054 | *B* | 1m0-09 |
| 2014-11-18 | 2456980.401 | 16.229 0.071 | *B* | 1m0-10 | 2014-09-03 | 2456903.636 | 15.233 0.077 | *g* | 1m0-10 |
| 2014-11-25 | 2456986.561 | 16.074 0.070 | *B* | 1m0-08 | 2014-09-03 | 2456903.639 | 15.212 0.049 | *g* | 1m0-10 |
| 2014-11-25 | 2456986.562 | 16.448 0.067 | *B* | 1m0-08 | 2014-09-03 | 2456903.898 | 15.260 0.041 | *g* | 1m0-09 |
| 2014-11-27 | 2456989.389 | 16.132 0.090 | *B* | 1m0-13 | 2014-09-03 | 2456903.901 | 15.218 0.051 | *g* | 1m0-09 |
| 2014-11-27 | 2456989.390 | 16.318 0.078 | *B* | 1m0-13 | 2014-09-07 | 2456908.194 | 14.902 0.070 | *g* | 1m0-11 |
| 2014-11-28 | 2456990.275 | 16.252 0.079 | *B* | 1m0-10 | 2014-09-07 | 2456908.197 | 14.905 0.070 | *g* | 1m0-11 |
| 2014-11-28 | 2456990.276 | 16.502 0.059 | *B* | 1m0-10 | 2014-09-07 | 2456908.276 | 14.910 0.081 | *g* | 1m0-03 |
| 2014-12-04 | 2456996.322 | 16.611 0.075 | *B* | 1m0-10 | 2014-09-07 | 2456908.279 | 14.917 0.079 | *g* | 1m0-03 |
| 2014-12-04 | 2456996.323 | 16.704 0.076 | *B* | 1m0-10 | 2014-09-12 | 2456913.189 | 14.955 0.066 | *g* | 1m0-11 |
| 2014-12-04 | 2456996.328 | 16.664 0.078 | *B* | 1m0-10 | 2014-09-12 | 2456913.192 | 14.945 0.045 | *g* | 1m0-11 |
| 2014-12-04 | 2456996.330 | 16.660 0.072 | *B* | 1m0-10 | 2014-09-14 | 2456915.263 | 14.909 0.084 | *g* | 1m0-03 |
| 2014-12-04 | 2456996.347 | 16.739 0.070 | *B* | 1m0-12 | 2014-09-14 | 2456915.266 | 14.928 0.087 | *g* | 1m0-03 |
| 2014-12-04 | 2456996.349 | 16.669 0.083 | *B* | 1m0-12 | 2014-09-16 | 2456917.186 | 14.980 0.056 | *g* | 1m0-11 |
| 2014-12-04 | 2456996.366 | 16.759 0.068 | *B* | 1m0-10 | 2014-09-16 | 2456917.189 | 14.957 0.054 | *g* | 1m0-11 |
| 2014-12-04 | 2456996.367 | 16.684 0.058 | *B* | 1m0-10 | 2014-09-18 | 2456919.193 | 15.036 0.078 | *g* | 1m0-03 |
| 2014-12-09 | 2457000.620 | 16.907 0.078 | *B* | 1m0-05 | 2014-09-18 | 2456919.195 | 15.010 0.065 | *g* | 1m0-03 |
| 2014-12-09 | 2457000.621 | 16.889 0.085 | *B* | 1m0-05 | 2014-09-20 | 2456921.049 | 15.036 0.093 | *g* | 1m0-03 |
| 2014-12-12 | 2457004.331 | 16.787 0.088 | *B* | 1m0-13 | 2014-09-20 | 2456921.052 | 14.971 0.079 | *g* | 1m0-03 |
| 2014-12-12 | 2457004.332 | 16.850 0.078 | *B* | 1m0-13 | 2014-09-23 | 2456924.045 | 15.024 0.047 | *g* | 1m0-11 |
| 2014-12-16 | 2457008.044 | 17.197 0.078 | *B* | 1m0-11 | 2014-09-23 | 2456924.048 | 15.026 0.067 | *g* | 1m0-11 |
| 2014-12-16 | 2457008.045 | 17.208 0.087 | *B* | 1m0-11 | 2014-09-27 | 2456928.053 | 15.113 0.049 | *g* | 1m0-11 |
| 2014-12-20 | 2457011.978 | 17.445 0.066 | *B* | 1m0-11 | 2014-09-27 | 2456928.055 | 15.103 0.051 | *g* | 1m0-11 |
| 2014-12-20 | 2457011.980 | 17.561 0.068 | *B* | 1m0-11 | 2014-09-29 | 2456929.902 | 15.134 0.051 | *g* | 1m0-08 |
| 2014-12-24 | 2457015.924 | 17.795 0.087 | *B* | 1m0-11 | 2014-09-29 | 2456929.904 | 15.146 0.050 | *g* | 1m0-08 |
| 2014-12-24 | 2457015.926 | 17.771 0.089 | *B* | 1m0-11 | 2014-10-02 | 2456933.026 | 15.215 0.056 | *g* | 1m0-11 |
| 2014-12-30 | 2457021.926 | 18.168 0.107 | *B* | 1m0-03 | 2014-10-02 | 2456933.029 | 15.197 0.055 | *g* | 1m0-11 |
| 2014-12-30 | 2457021.927 | 18.114 0.104 | *B* | 1m0-03 | 2014-10-03 | 2456934.224 | 15.270 0.053 | *g* | 1m0-11 |
| 2015-01-02 | 2457024.974 | 17.914 0.153 | *B* | 1m0-03 | 2014-10-09 | 2456940.193 | 15.209 0.117 | *g* | 1m0-11 |
| 2015-01-02 | 2457024.976 | 17.918 0.226 | *B* | 1m0-03 | 2014-10-09 | 2456940.196 | 15.252 0.078 | *g* | 1m0-11 |
| 2015-01-03 | 2457026.292 | 18.096 0.080 | *B* | 1m0-10 | 2014-10-13 | 2456944.335 | 15.395 0.064 | *g* | 1m0-12 |
| 2015-01-03 | 2457026.295 | 18.079 0.090 | *B* | 1m0-10 | 2014-10-17 | 2456947.980 | 15.337 0.057 | *g* | 1m0-11 |
| 2015-01-07 | 2457030.292 | 18.244 0.075 | *B* | 1m0-12 | 2014-10-17 | 2456947.983 | 15.351 0.058 | *g* | 1m0-11 |
| 2015-01-07 | 2457030.295 | 18.310 0.069 | *B* | 1m0-12 | 2014-10-21 | 2456952.063 | 15.389 0.037 | *g* | 1m0-11 |
| 2015-01-08 | 2457030.940 | 18.343 0.073 | *B* | 1m0-11 | 2014-10-21 | 2456952.065 | 15.371 0.042 | *g* | 1m0-11 |
| 2015-01-08 | 2457030.943 | 18.319 0.075 | *B* | 1m0-11 | 2014-10-25 | 2456955.909 | 15.446 0.069 | *g* | 1m0-03 |
| 2015-01-09 | 2457032.309 | 18.322 0.068 | *B* | 1m0-12 | 2014-10-25 | 2456955.910 | 15.444 0.068 | *g* | 1m0-03 |
| 2015-01-09 | 2457032.312 | 18.378 0.068 | *B* | 1m0-12 | 2014-11-01 | 2456963.067 | 15.512 0.075 | *g* | 1m0-11 |
| 2015-01-10 | 2457032.558 | 18.279 0.083 | *B* | 1m0-05 | 2014-11-01 | 2456963.069 | 15.483 0.058 | *g* | 1m0-11 |
| 2015-01-10 | 2457032.561 | 18.249 0.069 | *B* | 1m0-05 | 2014-11-06 | 2456968.483 | 15.596 0.055 | *g* | 1m0-10 |
| 2015-01-11 | 2457034.297 | 18.364 0.063 | *B* | 1m0-12 | 2014-11-06 | 2456968.485 | 15.489 0.069 | *g* | 1m0-10 |
| 2015-01-14 | 2457036.568 | 18.263 0.072 | *B* | 1m0-05 | 2014-11-06 | 2456968.496 | 15.512 0.062 | *g* | 1m0-10 |
| 2015-01-14 | 2457036.571 | 18.351 0.070 | *B* | 1m0-05 | 2014-11-06 | 2456968.498 | 15.536 0.057 | *g* | 1m0-10 |
| 2015-01-14 | 2457036.957 | 18.027 0.110 | *B* | 1m0-11 | 2014-11-13 | 2456975.135 | 15.532 0.081 | *g* | 1m0-11 |
| 2015-01-16 | 2457039.288 | 18.122 0.089 | *B* | 1m0-12 | 2014-11-18 | 2456980.404 | 15.630 0.051 | *g* | 1m0-10 |
| 2015-01-16 | 2457039.291 | 18.252 0.103 | *B* | 1m0-12 | 2014-11-18 | 2456980.406 | 15.621 0.058 | *g* | 1m0-10 |
| 2015-01-19 | 2457042.283 | 18.038 0.087 | *B* | 1m0-10 | 2014-11-25 | 2456986.566 | 15.762 0.062 | *g* | 1m0-08 |
| 2015-01-19 | 2457042.286 | 18.208 0.091 | *B* | 1m0-10 | 2014-11-25 | 2456986.567 | 15.721 0.043 | *g* | 1m0-08 |
| 2015-01-22 | 2457045.285 | 18.252 0.081 | *B* | 1m0-10 | 2014-11-27 | 2456989.394 | 15.694 0.068 | *g* | 1m0-13 |
| 2015-01-22 | 2457045.288 | 18.269 0.075 | *B* | 1m0-10 | 2014-11-27 | 2456989.395 | 15.648 0.049 | *g* | 1m0-13 |
| 2015-01-28 | 2457050.583 | 18.315 0.099 | *B* | 1m0-08 | 2014-11-28 | 2456990.280 | 15.774 0.046 | *g* | 1m0-10 |
| 2015-01-28 | 2457050.586 | 18.292 0.086 | *B* | 1m0-08 | 2014-11-28 | 2456990.281 | 15.796 0.035 | *g* | 1m0-10 |
| 2015-01-29 | 2457051.578 | 18.222 0.094 | *B* | 1m0-08 | 2014-12-04 | 2456996.327 | 15.963 0.046 | *g* | 1m0-10 |
| 2015-01-29 | 2457051.581 | 18.217 0.114 | *B* | 1m0-08 | 2014-12-04 | 2456996.352 | 15.740 0.068 | *g* | 1m0-12 |
| 2015-02-11 | 2457065.270 | 18.471 0.027 | *B* | 1m0-12 | 2014-12-04 | 2456996.354 | 16.009 0.069 | *g* | 1m0-12 |
| 2015-02-11 | 2457065.273 | 18.485 0.031 | *B* | 1m0-12 | 2014-12-04 | 2456996.371 | 15.875 0.050 | *g* | 1m0-10 |
| 2015-02-20 | 2457073.570 | 18.454 0.117 | *B* | 1m0-08 | 2014-12-04 | 2456996.372 | 15.893 0.050 | *g* | 1m0-10 |
| 2015-06-30 | 2457203.893 | 19.042 0.055 | *B* | 1m0-04 | 2014-12-09 | 2457000.625 | 16.132 0.076 | *g* | 1m0-05 |
| 2015-06-30 | 2457203.899 | 19.055 0.051 | *B* | 1m0-04 | 2014-12-09 | 2457000.626 | 16.117 0.066 | *g* | 1m0-05 |

(a) Data have not been corrected for extinction
(b) *Swift* Telescope; LSQ (La Silla Quest, Chile); 1m0-08 (McDonald Observatory, USA); 1m0-10, 1m0-12, 1m0-13 (Sutherland, South Africa), 1m0-04, 1m0-05, 1m0-09 (Cerro Tololo, Chile); 1m0-03, 1m0-11 (Siding Spring, Australia).

**Table D1:** ASASSN-14gm: Photometric Data

| Date | JD | mag$^{(a)}$ | Filter | telescope$^{(b)}$ | Date | JD | mag$^{(a)}$ | Filter | telescope$^{(b)}$ |
|---|---|---|---|---|---|---|---|---|---|
| 2014-12-12 | 2457004.336 | 16.162 0.066 | $g$ | 1m0-13 | 2014-08-29 | 2456899.470 | $<$ 17.300 | $V$ | Atel/CBAT |
| 2014-12-12 | 2457004.337 | 16.167 0.048 | $g$ | 1m0-13 | 2014-09-01 | 2456902.470 | 15.500 0.100 | $V$ | Atel/CBAT |
| 2014-12-16 | 2457008.048 | 16.338 0.062 | $g$ | 1m0-11 | 2014-09-03 | 2456903.632 | 15.279 0.095 | $V$ | 1m0-10 |
| 2014-12-20 | 2457011.983 | 16.507 0.064 | $g$ | 1m0-11 | 2014-09-03 | 2456903.634 | 15.257 0.095 | $V$ | 1m0-10 |
| 2014-12-20 | 2457011.985 | 16.407 0.092 | $g$ | 1m0-11 | 2014-09-03 | 2456903.893 | 15.259 0.050 | $V$ | 1m0-09 |
| 2014-12-24 | 2457015.929 | 17.168 0.107 | $g$ | 1m0-11 | 2014-09-03 | 2456903.895 | 15.260 0.048 | $V$ | 1m0-09 |
| 2014-12-24 | 2457015.930 | 16.774 0.093 | $g$ | 1m0-11 | 2014-09-07 | 2456908.191 | 14.857 0.085 | $V$ | 1m0-11 |
| 2014-12-30 | 2457021.930 | 17.602 0.080 | $g$ | 1m0-03 | 2014-09-07 | 2456908.193 | 14.839 0.085 | $V$ | 1m0-11 |
| 2014-12-30 | 2457021.932 | 17.553 0.063 | $g$ | 1m0-03 | 2014-09-07 | 2456908.273 | 14.875 0.085 | $V$ | 1m0-03 |
| 2015-01-02 | 2457024.983 | 17.478 0.077 | $g$ | 1m0-03 | 2014-09-07 | 2456908.274 | 14.846 0.085 | $V$ | 1m0-03 |
| 2015-01-02 | 2457024.986 | 17.441 0.087 | $g$ | 1m0-03 | 2014-09-12 | 2456913.186 | 14.869 0.102 | $V$ | 1m0-11 |
| 2015-01-03 | 2457026.302 | 17.553 0.061 | $g$ | 1m0-10 | 2014-09-12 | 2456913.187 | 14.876 0.102 | $V$ | 1m0-11 |
| 2015-01-03 | 2457026.305 | 17.371 0.059 | $g$ | 1m0-10 | 2014-09-14 | 2456915.260 | 14.928 0.088 | $V$ | 1m0-03 |
| 2015-01-05 | 2457028.335 | 17.718 0.061 | $g$ | 1m0-12 | 2014-09-14 | 2456915.261 | 14.917 0.088 | $V$ | 1m0-03 |
| 2015-01-05 | 2457028.338 | 17.575 0.063 | $g$ | 1m0-12 | 2014-09-16 | 2456917.183 | 14.838 0.075 | $V$ | 1m0-11 |
| 2015-01-07 | 2457030.301 | 17.658 0.091 | $g$ | 1m0-12 | 2014-09-16 | 2456917.184 | 14.816 0.075 | $V$ | 1m0-11 |
| 2015-01-07 | 2457030.304 | 17.549 0.152 | $g$ | 1m0-12 | 2014-09-18 | 2456919.189 | 14.904 0.097 | $V$ | 1m0-03 |
| 2015-01-08 | 2457030.950 | 17.663 0.064 | $g$ | 1m0-11 | 2014-09-18 | 2456919.191 | 14.905 0.097 | $V$ | 1m0-03 |
| 2015-01-08 | 2457030.953 | 17.695 0.066 | $g$ | 1m0-11 | 2014-09-20 | 2456921.046 | 14.901 0.083 | $V$ | 1m0-03 |
| 2015-01-09 | 2457032.331 | 17.686 0.075 | $g$ | 1m0-12 | 2014-09-20 | 2456921.048 | 14.905 0.083 | $V$ | 1m0-03 |
| 2015-01-10 | 2457032.567 | 17.712 0.066 | $g$ | 1m0-05 | 2014-09-23 | 2456924.042 | 14.841 0.077 | $V$ | 1m0-11 |
| 2015-01-10 | 2457032.570 | 17.766 0.054 | $g$ | 1m0-05 | 2014-09-23 | 2456924.044 | 14.834 0.077 | $V$ | 1m0-11 |
| 2015-01-11 | 2457034.303 | 17.644 0.059 | $g$ | 1m0-12 | 2014-09-27 | 2456928.050 | 14.931 0.088 | $V$ | 1m0-11 |
| 2015-01-11 | 2457034.306 | 17.702 0.057 | $g$ | 1m0-12 | 2014-09-27 | 2456928.051 | 14.887 0.088 | $V$ | 1m0-11 |
| 2015-01-14 | 2457036.577 | 17.715 0.080 | $g$ | 1m0-05 | 2014-09-29 | 2456929.899 | 14.899 0.092 | $V$ | 1m0-08 |
| 2015-01-14 | 2457036.580 | 17.724 0.077 | $g$ | 1m0-05 | 2014-09-29 | 2456929.900 | 14.915 0.092 | $V$ | 1m0-08 |
| 2015-01-14 | 2457036.964 | 17.589 0.057 | $g$ | 1m0-11 | 2014-10-02 | 2456933.023 | 14.919 0.071 | $V$ | 1m0-11 |
| 2015-01-15 | 2457037.937 | 17.733 0.062 | $g$ | 1m0-11 | 2014-10-02 | 2456933.024 | 14.933 0.071 | $V$ | 1m0-11 |
| 2015-01-15 | 2457037.940 | 17.711 0.059 | $g$ | 1m0-11 | 2014-10-03 | 2456934.219 | 14.988 0.061 | $V$ | 1m0-11 |
| 2015-01-16 | 2457039.297 | 17.678 0.075 | $g$ | 1m0-12 | 2014-10-09 | 2456940.190 | 14.798 0.143 | $V$ | 1m0-11 |
| 2015-01-16 | 2457039.300 | 17.796 0.073 | $g$ | 1m0-12 | 2014-10-09 | 2456940.192 | 14.932 0.143 | $V$ | 1m0-11 |
| 2015-01-19 | 2457042.295 | 17.677 0.039 | $g$ | 1m0-10 | 2014-10-13 | 2456944.332 | 15.024 0.101 | $V$ | 1m0-12 |
| 2015-01-22 | 2457045.295 | 17.732 0.052 | $g$ | 1m0-10 | 2014-10-13 | 2456944.333 | 14.951 0.101 | $V$ | 1m0-12 |
| 2015-01-22 | 2457045.298 | 17.794 0.044 | $g$ | 1m0-10 | 2014-10-17 | 2456947.977 | 14.964 0.068 | $V$ | 1m0-11 |
| 2015-01-28 | 2457050.593 | 17.727 0.071 | $g$ | 1m0-08 | 2014-10-17 | 2456947.979 | 14.925 0.068 | $V$ | 1m0-11 |
| 2015-01-28 | 2457050.595 | 17.768 0.072 | $g$ | 1m0-08 | 2014-10-21 | 2456952.059 | 14.954 0.070 | $V$ | 1m0-11 |
| 2015-01-29 | 2457051.587 | 17.763 0.104 | $g$ | 1m0-08 | 2014-10-21 | 2456952.061 | 14.970 0.070 | $V$ | 1m0-11 |
| 2015-01-29 | 2457051.590 | 17.874 0.068 | $g$ | 1m0-08 | 2014-10-25 | 2456955.907 | 14.954 0.094 | $V$ | 1m0-03 |
| 2015-02-11 | 2457064.576 | 17.766 0.079 | $g$ | 1m0-08 | 2014-10-25 | 2456955.908 | 14.974 0.096 | $V$ | 1m0-03 |
| 2015-02-11 | 2457064.579 | 17.697 0.072 | $g$ | 1m0-08 | 2014-11-01 | 2456963.065 | 15.057 0.082 | $V$ | 1m0-11 |
| 2015-06-30 | 2457203.913 | 18.699 0.093 | $g$ | 1m0-04 | 2014-11-01 | 2456963.066 | 15.099 0.081 | $V$ | 1m0-11 |
| 2015-06-30 | 2457203.918 | 18.762 0.086 | $g$ | 1m0-04 | 2014-11-06 | 2456968.481 | 15.103 0.112 | $V$ | 1m0-10 |
| 2015-07-17 | 2457220.760 | 18.730 0.054 | $g$ | 1m0-04 | 2014-11-06 | 2456968.482 | 14.907 0.113 | $V$ | 1m0-10 |
| 2015-07-17 | 2457220.765 | 18.672 0.059 | $g$ | 1m0-04 | 2014-11-06 | 2456968.495 | 15.087 0.112 | $V$ | 1m0-10 |
| 2014-09-03 | 2456903.531 | 15.488 0.063 | $vs$ | *Swift* | 2014-11-13 | 2456975.133 | 14.889 0.082 | $V$ | 1m0-11 |
| 2014-09-04 | 2456905.126 | 15.169 0.057 | $vs$ | *Swift* | 2014-11-13 | 2456975.134 | 14.901 0.082 | $V$ | 1m0-11 |
| 2014-09-05 | 2456905.760 | 15.146 0.056 | $vs$ | *Swift* | 2014-11-18 | 2456980.403 | 15.149 0.074 | $V$ | 1m0-10 |
| 2014-09-06 | 2456906.595 | 15.079 0.055 | $vs$ | *Swift* | 2014-11-18 | 2456980.403 | 15.123 0.074 | $V$ | 1m0-10 |
| 2014-09-07 | 2456907.753 | 15.065 0.056 | $vs$ | *Swift* | 2014-11-25 | 2456986.564 | 15.231 0.074 | $V$ | 1m0-08 |
| 2014-09-09 | 2456909.595 | 15.020 0.053 | $vs$ | *Swift* | 2014-11-25 | 2456986.565 | 15.213 0.074 | $V$ | 1m0-08 |
| 2014-09-12 | 2456913.413 | 15.025 0.052 | $vs$ | *Swift* | 2014-11-27 | 2456989.392 | 15.123 0.098 | $V$ | 1m0-13 |
| 2014-09-16 | 2456916.778 | 15.061 0.049 | $vs$ | *Swift* | 2014-11-27 | 2456989.393 | 15.122 0.098 | $V$ | 1m0-13 |
| 2014-09-20 | 2456921.278 | 15.015 0.050 | $vs$ | *Swift* | 2014-11-28 | 2456990.278 | 15.270 0.082 | $V$ | 1m0-10 |
| 2014-09-24 | 2456925.212 | 14.990 0.055 | $vs$ | *Swift* | 2014-11-28 | 2456990.279 | 15.267 0.082 | $V$ | 1m0-10 |
| 2014-09-28 | 2456929.103 | 15.022 0.051 | $vs$ | *Swift* | 2014-12-04 | 2456996.325 | 15.407 0.081 | $V$ | 1m0-10 |
| 2014-10-04 | 2456934.666 | 15.012 0.066 | $vs$ | *Swift* | 2014-12-04 | 2456996.326 | 15.389 0.081 | $V$ | 1m0-10 |
| 2014-10-11 | 2456941.773 | 15.155 0.046 | $vs$ | *Swift* | 2014-12-04 | 2456996.331 | 15.399 0.081 | $V$ | 1m0-10 |
| 2014-10-19 | 2456950.337 | 15.181 0.053 | $vs$ | *Swift* | 2014-12-04 | 2456996.332 | 15.447 0.081 | $V$ | 1m0-10 |
| 2014-10-22 | 2456953.205 | 15.136 0.092 | $vs$ | *Swift* | 2014-12-04 | 2456996.350 | 15.481 0.082 | $V$ | 1m0-12 |
| 2014-10-24 | 2456955.099 | 15.152 0.046 | $vs$ | *Swift* | 2014-12-04 | 2456996.351 | 15.425 0.082 | $V$ | 1m0-12 |

(a) Data have not been corrected for extinction
(b) *Swift* Telescope; LSQ (La Silla Quest, Chile); 1m0-08 (McDonald Observatory, USA); 1m0-10, 1m0-12, 1m0-13 (Sutherland, South Africa), 1m0-04, 1m0-05, 1m0-09 (Cerro Tololo, Chile); 1m0-03, 1m0-11 (Siding Spring, Australia).

**Table D1:** ASASSN-14gm: Photometric Data

| Date | JD | mag$^{(a)}$ | Filter | telescope$^{(b)}$ | Date | JD | mag$^{(a)}$ | Filter | telescope$^{(b)}$ |
|---|---|---|---|---|---|---|---|---|---|
| 2014-12-04 | 2456996.370 | 15.322 0.082 | $V$ | 1m0-10 | 2014-09-12 | 2456913.194 | 14.767 0.028 | $r$ | 1m0-11 |
| 2014-12-09 | 2457000.623 | 15.577 0.086 | $V$ | 1m0-05 | 2014-09-12 | 2456913.196 | 14.777 0.033 | $r$ | 1m0-11 |
| 2014-12-09 | 2457000.623 | 15.559 0.086 | $V$ | 1m0-05 | 2014-09-14 | 2456915.268 | 14.735 0.069 | $r$ | 1m0-03 |
| 2014-12-12 | 2457004.333 | 15.631 0.094 | $V$ | 1m0-13 | 2014-09-14 | 2456915.270 | 14.728 0.069 | $r$ | 1m0-03 |
| 2014-12-12 | 2457004.334 | 15.616 0.094 | $V$ | 1m0-13 | 2014-09-16 | 2456917.191 | 14.652 0.040 | $r$ | 1m0-11 |
| 2014-12-16 | 2457008.046 | 15.932 0.082 | $V$ | 1m0-11 | 2014-09-16 | 2456917.193 | 14.703 0.037 | $r$ | 1m0-11 |
| 2014-12-16 | 2457008.047 | 15.667 0.089 | $V$ | 1m0-11 | 2014-09-18 | 2456919.198 | 14.788 0.065 | $r$ | 1m0-03 |
| 2014-12-20 | 2457011.981 | 16.195 0.065 | $V$ | 1m0-11 | 2014-09-18 | 2456919.199 | 14.789 0.066 | $r$ | 1m0-03 |
| 2014-12-20 | 2457011.982 | 16.266 0.065 | $V$ | 1m0-11 | 2014-09-20 | 2456921.055 | 14.694 0.064 | $r$ | 1m0-03 |
| 2014-12-24 | 2457015.927 | 16.331 0.127 | $V$ | 1m0-11 | 2014-09-20 | 2456921.056 | 14.709 0.064 | $r$ | 1m0-03 |
| 2014-12-24 | 2457015.928 | 16.532 0.078 | $V$ | 1m0-11 | 2014-09-23 | 2456924.051 | 14.704 0.053 | $r$ | 1m0-11 |
| 2014-12-30 | 2457021.929 | 17.018 0.094 | $V$ | 1m0-03 | 2014-09-23 | 2456924.052 | 14.677 0.054 | $r$ | 1m0-11 |
| 2014-12-30 | 2457021.929 | 17.005 0.095 | $V$ | 1m0-03 | 2014-09-27 | 2456928.058 | 14.712 0.038 | $r$ | 1m0-11 |
| 2015-01-02 | 2457024.980 | 17.014 0.152 | $V$ | 1m0-03 | 2014-09-29 | 2456929.907 | 14.707 0.039 | $r$ | 1m0-08 |
| 2015-01-02 | 2457024.981 | 16.909 0.137 | $V$ | 1m0-03 | 2014-09-29 | 2456929.909 | 14.690 0.032 | $r$ | 1m0-08 |
| 2015-01-03 | 2457026.299 | 16.825 0.086 | $V$ | 1m0-10 | 2014-10-02 | 2456933.031 | 14.758 0.040 | $r$ | 1m0-11 |
| 2015-01-03 | 2457026.300 | 17.025 0.084 | $V$ | 1m0-10 | 2014-10-02 | 2456933.033 | 14.758 0.036 | $r$ | 1m0-11 |
| 2015-01-05 | 2457028.332 | 17.109 0.148 | $V$ | 1m0-12 | 2014-10-03 | 2456934.227 | 14.770 0.043 | $r$ | 1m0-11 |
| 2015-01-07 | 2457030.298 | 17.124 0.079 | $V$ | 1m0-12 | 2014-10-03 | 2456934.228 | 14.799 0.200 | $r$ | 1m0-11 |
| 2015-01-07 | 2457030.299 | 17.166 0.079 | $V$ | 1m0-12 | 2014-10-09 | 2456940.200 | 14.723 0.037 | $r$ | 1m0-11 |
| 2015-01-08 | 2457030.946 | 17.035 0.078 | $V$ | 1m0-11 | 2014-10-13 | 2456944.340 | 14.818 0.054 | $r$ | 1m0-12 |
| 2015-01-08 | 2457030.948 | 17.114 0.079 | $V$ | 1m0-11 | 2014-10-13 | 2456944.342 | 14.813 0.028 | $r$ | 1m0-12 |
| 2015-01-09 | 2457032.325 | 17.331 0.077 | $V$ | 1m0-12 | 2014-10-17 | 2456947.986 | 14.753 0.039 | $r$ | 1m0-11 |
| 2015-01-09 | 2457032.326 | 17.184 0.069 | $V$ | 1m0-12 | 2014-10-17 | 2456947.987 | 14.778 0.035 | $r$ | 1m0-11 |
| 2015-01-10 | 2457032.564 | 17.140 0.088 | $V$ | 1m0-05 | 2014-10-21 | 2456952.068 | 14.731 0.030 | $r$ | 1m0-11 |
| 2015-01-10 | 2457032.565 | 17.111 0.088 | $V$ | 1m0-05 | 2014-10-21 | 2456952.069 | 14.777 0.035 | $r$ | 1m0-11 |
| 2015-01-11 | 2457034.300 | 17.097 0.080 | $V$ | 1m0-12 | 2014-10-25 | 2456955.912 | 14.773 0.051 | $r$ | 1m0-03 |
| 2015-01-11 | 2457034.302 | 17.264 0.060 | $V$ | 1m0-12 | 2014-10-25 | 2456955.913 | 14.752 0.054 | $r$ | 1m0-03 |
| 2015-01-14 | 2457036.574 | 17.312 0.070 | $V$ | 1m0-05 | 2014-11-01 | 2456963.070 | 14.733 0.047 | $r$ | 1m0-11 |
| 2015-01-14 | 2457036.576 | 17.248 0.069 | $V$ | 1m0-05 | 2014-11-01 | 2456963.071 | 14.813 0.048 | $r$ | 1m0-11 |
| 2015-01-14 | 2457036.961 | 17.079 0.124 | $V$ | 1m0-11 | 2014-11-06 | 2456968.486 | 14.767 0.043 | $r$ | 1m0-10 |
| 2015-01-14 | 2457036.962 | 17.008 0.124 | $V$ | 1m0-11 | 2014-11-06 | 2456968.487 | 14.796 0.038 | $r$ | 1m0-10 |
| 2015-01-16 | 2457039.294 | 17.153 0.089 | $V$ | 1m0-12 | 2014-11-06 | 2456968.499 | 14.744 0.042 | $r$ | 1m0-10 |
| 2015-01-16 | 2457039.296 | 17.150 0.088 | $V$ | 1m0-12 | 2014-11-07 | 2456968.500 | 14.785 0.051 | $r$ | 1m0-10 |
| 2015-01-19 | 2457042.290 | 17.221 0.080 | $V$ | 1m0-10 | 2014-11-13 | 2456975.138 | 14.683 0.061 | $r$ | 1m0-11 |
| 2015-01-22 | 2457045.291 | 17.219 0.084 | $V$ | 1m0-10 | 2014-11-13 | 2456975.139 | 14.751 0.051 | $r$ | 1m0-11 |
| 2015-01-22 | 2457045.293 | 17.161 0.085 | $V$ | 1m0-10 | 2014-11-18 | 2456980.407 | 14.700 0.042 | $r$ | 1m0-10 |
| 2015-01-27 | 2457049.532 | 17.362 0.103 | $V$ | 1m0-05 | 2014-11-18 | 2456980.408 | 14.861 0.040 | $r$ | 1m0-10 |
| 2015-01-27 | 2457049.534 | 17.307 0.107 | $V$ | 1m0-05 | 2014-11-25 | 2456986.568 | 14.951 0.044 | $r$ | 1m0-08 |
| 2015-01-28 | 2457050.589 | 17.186 0.098 | $V$ | 1m0-08 | 2014-11-25 | 2456986.569 | 14.955 0.035 | $r$ | 1m0-08 |
| 2015-01-28 | 2457050.591 | 17.311 0.096 | $V$ | 1m0-08 | 2014-11-27 | 2456989.397 | 14.884 0.044 | $r$ | 1m0-13 |
| 2015-01-29 | 2457051.584 | 17.271 0.090 | $V$ | 1m0-08 | 2014-11-27 | 2456989.398 | 14.828 0.032 | $r$ | 1m0-13 |
| 2015-01-29 | 2457051.585 | 17.378 0.087 | $V$ | 1m0-08 | 2014-11-28 | 2456990.283 | 15.008 0.033 | $r$ | 1m0-10 |
| 2015-02-11 | 2457065.277 | 17.483 0.013 | $V$ | 1m0-12 | 2014-11-28 | 2456990.284 | 15.013 0.037 | $r$ | 1m0-10 |
| 2015-02-11 | 2457065.280 | 17.471 0.013 | $V$ | 1m0-12 | 2014-12-04 | 2456996.355 | 15.133 0.038 | $r$ | 1m0-12 |
| 2015-02-18 | 2457071.576 | 17.304 0.109 | $V$ | 1m0-08 | 2014-12-04 | 2456996.356 | 15.095 0.032 | $r$ | 1m0-12 |
| 2015-02-18 | 2457071.578 | 17.330 0.108 | $V$ | 1m0-08 | 2014-12-04 | 2456996.374 | 15.118 0.041 | $r$ | 1m0-10 |
| 2015-02-20 | 2457073.577 | 17.375 0.089 | $V$ | 1m0-08 | 2014-12-04 | 2456996.374 | 15.072 0.035 | $r$ | 1m0-10 |
| 2015-06-30 | 2457203.904 | 18.643 0.057 | $V$ | 1m0-04 | 2014-12-09 | 2457000.627 | 15.180 0.039 | $r$ | 1m0-05 |
| 2015-06-30 | 2457203.908 | 18.534 0.058 | $V$ | 1m0-04 | 2014-12-09 | 2457000.628 | 15.179 0.045 | $r$ | 1m0-05 |
| 2015-07-17 | 2457220.765 | 18.555 0.059 | $V$ | 1m0-09 | 2014-12-12 | 2457004.339 | 15.256 0.031 | $r$ | 1m0-13 |
| 2015-07-17 | 2457220.769 | 18.544 0.060 | $V$ | 1m0-09 | 2014-12-12 | 2457004.340 | 15.246 0.042 | $r$ | 1m0-13 |
| 2014-09-03 | 2456903.641 | 15.361 0.050 | $r$ | 1m0-10 | 2014-12-16 | 2457008.051 | 15.436 0.056 | $r$ | 1m0-11 |
| 2014-09-03 | 2456903.643 | 15.354 0.041 | $r$ | 1m0-10 | 2014-12-16 | 2457008.052 | 15.463 0.036 | $r$ | 1m0-11 |
| 2014-09-03 | 2456903.905 | 15.351 0.036 | $r$ | 1m0-09 | 2014-12-20 | 2457011.986 | 15.731 0.039 | $r$ | 1m0-11 |
| 2014-09-03 | 2456903.908 | 15.344 0.036 | $r$ | 1m0-09 | 2014-12-20 | 2457011.987 | 15.745 0.035 | $r$ | 1m0-11 |
| 2014-09-07 | 2456908.200 | 14.805 0.031 | $r$ | 1m0-11 | 2014-12-24 | 2457015.932 | 16.050 0.041 | $r$ | 1m0-11 |
| 2014-09-07 | 2456908.201 | 14.788 0.031 | $r$ | 1m0-11 | 2014-12-24 | 2457015.933 | 16.039 0.050 | $r$ | 1m0-11 |
| 2014-09-07 | 2456908.281 | 14.812 0.057 | $r$ | 1m0-03 | 2014-12-30 | 2457021.933 | 16.465 0.046 | $r$ | 1m0-03 |
| 2014-09-07 | 2456908.283 | 14.793 0.059 | $r$ | 1m0-03 | 2014-12-30 | 2457021.934 | 16.412 0.047 | $r$ | 1m0-03 |

(a) Data have not been corrected for extinction
(b) *Swift* Telescope; LSQ (La Silla Quest, Chile); 1m0-08 (McDonald Observatory, USA); 1m0-10, 1m0-12, 1m0-13 (Sutherland, South Africa), 1m0-04, 1m0-05, 1m0-09 (Cerro Tololo, Chile); 1m0-03, 1m0-11 (Siding Spring, Australia).

**Table D1:** ASASSN-14gm: Photometric Data

| Date | JD | mag[a] | Filter | telescope[b] | Date | JD | mag[a] | Filter | telescope[b] |
|---|---|---|---|---|---|---|---|---|---|
| 2015-01-02 | 2457024.989 | 16.496 0.076 | $r$ | 1m0-03 | 2014-09-29 | 2456929.912 | 14.747 0.040 | $i$ | 1m0-08 |
| 2015-01-02 | 2457024.991 | 16.474 0.059 | $r$ | 1m0-03 | 2014-10-02 | 2456933.035 | 14.768 0.040 | $i$ | 1m0-11 |
| 2015-01-03 | 2457026.308 | 16.487 0.041 | $r$ | 1m0-10 | 2014-10-02 | 2456933.036 | 14.767 0.040 | $i$ | 1m0-11 |
| 2015-01-03 | 2457026.310 | 16.363 0.034 | $r$ | 1m0-10 | 2014-10-03 | 2456934.230 | 14.764 0.043 | $i$ | 1m0-11 |
| 2015-01-05 | 2457028.341 | 16.445 0.046 | $r$ | 1m0-12 | 2014-10-03 | 2456934.232 | 14.786 0.043 | $i$ | 1m0-11 |
| 2015-01-05 | 2457028.343 | 16.518 0.038 | $r$ | 1m0-12 | 2014-10-09 | 2456940.202 | 14.744 0.038 | $i$ | 1m0-11 |
| 2015-01-08 | 2457030.956 | 16.515 0.053 | $r$ | 1m0-11 | 2014-10-09 | 2456940.204 | 14.711 0.038 | $i$ | 1m0-11 |
| 2015-01-08 | 2457030.957 | 16.521 0.056 | $r$ | 1m0-11 | 2014-10-13 | 2456944.343 | 14.751 0.055 | $i$ | 1m0-12 |
| 2015-01-10 | 2457032.573 | 16.591 0.033 | $r$ | 1m0-05 | 2014-10-13 | 2456944.345 | 14.793 0.055 | $i$ | 1m0-12 |
| 2015-01-10 | 2457032.575 | 16.541 0.037 | $r$ | 1m0-05 | 2014-10-17 | 2456947.989 | 14.769 0.040 | $i$ | 1m0-11 |
| 2015-01-11 | 2457034.310 | 16.379 0.037 | $r$ | 1m0-12 | 2014-10-17 | 2456947.990 | 14.766 0.040 | $i$ | 1m0-11 |
| 2015-01-11 | 2457034.311 | 16.552 0.035 | $r$ | 1m0-12 | 2014-10-21 | 2456952.071 | 14.753 0.031 | $i$ | 1m0-11 |
| 2015-01-14 | 2457036.584 | 16.556 0.059 | $r$ | 1m0-05 | 2014-10-21 | 2456952.073 | 14.689 0.031 | $i$ | 1m0-11 |
| 2015-01-14 | 2457036.585 | 16.555 0.050 | $r$ | 1m0-05 | 2014-10-25 | 2456955.914 | 14.729 0.052 | $i$ | 1m0-03 |
| 2015-01-14 | 2457036.970 | 16.596 0.056 | $r$ | 1m0-11 | 2014-10-25 | 2456955.914 | 14.719 0.052 | $i$ | 1m0-03 |
| 2015-01-14 | 2457036.972 | 16.558 0.070 | $r$ | 1m0-11 | 2014-11-01 | 2456963.072 | 14.675 0.046 | $i$ | 1m0-11 |
| 2015-01-15 | 2457037.943 | 16.658 0.047 | $r$ | 1m0-11 | 2014-11-01 | 2456963.073 | 14.740 0.046 | $i$ | 1m0-11 |
| 2015-01-15 | 2457037.945 | 16.615 0.041 | $r$ | 1m0-11 | 2014-11-06 | 2456968.488 | 14.787 0.045 | $i$ | 1m0-10 |
| 2015-01-16 | 2457039.303 | 16.634 0.049 | $r$ | 1m0-12 | 2014-11-06 | 2456968.489 | 14.729 0.044 | $i$ | 1m0-10 |
| 2015-01-16 | 2457039.305 | 16.636 0.049 | $r$ | 1m0-12 | 2014-11-07 | 2456968.502 | 14.701 0.047 | $i$ | 1m0-10 |
| 2015-01-19 | 2457042.298 | 16.642 0.053 | $r$ | 1m0-10 | 2014-11-07 | 2456968.503 | 14.724 0.044 | $i$ | 1m0-10 |
| 2015-01-19 | 2457042.300 | 16.534 0.040 | $r$ | 1m0-10 | 2014-11-13 | 2456975.141 | 14.828 0.055 | $i$ | 1m0-11 |
| 2015-01-22 | 2457045.301 | 16.560 0.049 | $r$ | 1m0-10 | 2014-11-18 | 2456980.409 | 14.873 0.045 | $i$ | 1m0-10 |
| 2015-01-22 | 2457045.303 | 16.557 0.059 | $r$ | 1m0-10 | 2014-11-18 | 2456980.410 | 14.786 0.039 | $i$ | 1m0-10 |
| 2015-01-28 | 2457050.599 | 16.642 0.043 | $r$ | 1m0-08 | 2014-11-25 | 2456986.570 | 14.851 0.045 | $i$ | 1m0-08 |
| 2015-01-28 | 2457050.600 | 16.665 0.044 | $r$ | 1m0-08 | 2014-11-25 | 2456986.571 | 14.848 0.044 | $i$ | 1m0-08 |
| 2015-01-29 | 2457051.593 | 16.559 0.043 | $r$ | 1m0-08 | 2014-11-27 | 2456989.399 | 14.812 0.046 | $i$ | 1m0-13 |
| 2015-01-29 | 2457051.595 | 16.580 0.043 | $r$ | 1m0-08 | 2014-11-28 | 2456990.285 | 14.934 0.034 | $i$ | 1m0-10 |
| 2015-02-11 | 2457064.583 | 16.702 0.057 | $r$ | 1m0-08 | 2014-11-28 | 2456990.285 | 14.923 0.035 | $i$ | 1m0-10 |
| 2015-02-11 | 2457064.586 | 16.720 0.051 | $r$ | 1m0-08 | 2014-12-04 | 2456996.357 | 14.957 0.040 | $i$ | 1m0-12 |
| 2015-06-04 | 2457177.919 | 17.806 0.059 | $r$ | 1m0-05 | 2014-12-04 | 2456996.376 | 14.889 0.039 | $i$ | 1m0-10 |
| 2015-06-04 | 2457177.922 | 17.721 0.049 | $r$ | 1m0-05 | 2014-12-09 | 2457000.629 | 15.052 0.041 | $i$ | 1m0-05 |
| 2015-06-22 | 2457196.287 | 17.968 0.072 | $r$ | 1m0-11 | 2014-12-09 | 2457000.630 | 15.082 0.041 | $i$ | 1m0-05 |
| 2015-06-22 | 2457196.291 | 17.991 0.766 | $r$ | 1m0-11 | 2014-12-12 | 2457004.341 | 15.118 0.033 | $i$ | 1m0-13 |
| 2015-06-30 | 2457203.923 | 17.902 0.055 | $r$ | 1m0-04 | 2014-12-12 | 2457004.342 | 15.096 0.033 | $i$ | 1m0-13 |
| 2015-06-30 | 2457203.927 | 17.900 0.054 | $r$ | 1m0-04 | 2014-12-16 | 2457008.053 | 15.415 0.057 | $i$ | 1m0-11 |
| 2015-07-17 | 2457220.771 | 18.067 0.037 | $r$ | 1m0-04 | 2014-12-16 | 2457008.054 | 15.284 0.060 | $i$ | 1m0-11 |
| 2015-07-17 | 2457220.775 | 18.101 0.036 | $r$ | 1m0-04 | 2014-12-20 | 2457011.988 | 15.563 0.039 | $i$ | 1m0-11 |
| 2014-09-03 | 2456903.645 | 15.499 0.050 | $i$ | 1m0-10 | 2014-12-20 | 2457011.989 | 15.530 0.042 | $i$ | 1m0-11 |
| 2014-09-03 | 2456903.646 | 15.479 0.051 | $i$ | 1m0-10 | 2014-12-24 | 2457015.934 | 15.729 0.048 | $i$ | 1m0-11 |
| 2014-09-03 | 2456903.910 | 15.429 0.034 | $i$ | 1m0-09 | 2014-12-24 | 2457015.935 | 15.922 0.043 | $i$ | 1m0-11 |
| 2014-09-03 | 2456903.912 | 15.430 0.034 | $i$ | 1m0-09 | 2014-12-30 | 2457021.935 | 16.330 0.049 | $i$ | 1m0-03 |
| 2014-09-07 | 2456908.203 | 14.873 0.031 | $i$ | 1m0-11 | 2014-12-30 | 2457021.936 | 16.385 0.050 | $i$ | 1m0-03 |
| 2014-09-07 | 2456908.284 | 14.857 0.031 | $i$ | 1m0-03 | 2015-01-02 | 2457024.992 | 16.416 0.065 | $i$ | 1m0-03 |
| 2014-09-07 | 2456908.286 | 14.896 0.031 | $i$ | 1m0-03 | 2015-01-02 | 2457024.994 | 16.356 0.059 | $i$ | 1m0-03 |
| 2014-09-12 | 2456913.198 | 14.919 0.028 | $i$ | 1m0-11 | 2015-01-03 | 2457026.311 | 16.419 0.046 | $i$ | 1m0-10 |
| 2014-09-12 | 2456913.199 | 14.868 0.028 | $i$ | 1m0-11 | 2015-01-05 | 2457028.345 | 16.408 0.046 | $i$ | 1m0-12 |
| 2014-09-14 | 2456915.272 | 14.868 0.070 | $i$ | 1m0-03 | 2015-01-05 | 2457028.346 | 16.527 0.047 | $i$ | 1m0-12 |
| 2014-09-14 | 2456915.273 | 14.917 0.069 | $i$ | 1m0-03 | 2015-01-08 | 2457030.959 | 16.476 0.059 | $i$ | 1m0-11 |
| 2014-09-16 | 2456917.194 | 14.846 0.040 | $i$ | 1m0-11 | 2015-01-08 | 2457030.961 | 16.518 0.055 | $i$ | 1m0-11 |
| 2014-09-16 | 2456917.196 | 14.819 0.040 | $i$ | 1m0-11 | 2015-01-10 | 2457032.577 | 16.481 0.034 | $i$ | 1m0-05 |
| 2014-09-18 | 2456919.201 | 14.862 0.066 | $i$ | 1m0-03 | 2015-01-10 | 2457032.578 | 16.538 0.035 | $i$ | 1m0-05 |
| 2014-09-18 | 2456919.203 | 14.847 0.066 | $i$ | 1m0-03 | 2015-01-11 | 2457034.313 | 16.347 0.044 | $i$ | 1m0-12 |
| 2014-09-20 | 2456921.058 | 14.860 0.064 | $i$ | 1m0-03 | 2015-01-11 | 2457034.315 | 16.531 0.038 | $i$ | 1m0-12 |
| 2014-09-20 | 2456921.059 | 14.897 0.064 | $i$ | 1m0-03 | 2015-01-14 | 2457036.587 | 16.614 0.062 | $i$ | 1m0-05 |
| 2014-09-23 | 2456924.054 | 14.759 0.054 | $i$ | 1m0-11 | 2015-01-15 | 2457037.946 | 16.585 0.050 | $i$ | 1m0-11 |
| 2014-09-23 | 2456924.055 | 14.716 0.054 | $i$ | 1m0-11 | 2015-01-15 | 2457037.948 | 16.622 0.046 | $i$ | 1m0-11 |
| 2014-09-27 | 2456928.061 | 14.801 0.038 | $i$ | 1m0-11 | 2015-01-16 | 2457039.307 | 16.597 0.052 | $i$ | 1m0-12 |
| 2014-09-27 | 2456928.063 | 14.770 0.038 | $i$ | 1m0-11 | 2015-01-16 | 2457039.308 | 16.559 0.051 | $i$ | 1m0-12 |
| 2014-09-29 | 2456929.910 | 14.750 0.040 | $i$ | 1m0-08 | 2015-01-19 | 2457042.302 | 16.496 0.057 | $i$ | 1m0-10 |

(a) Data have not been corrected for extinction
(b) *Swift* Telescope; LSQ (La Silla Quest, Chile); 1m0-08 (McDonald Observatory, USA); 1m0-10, 1m0-12, 1m0-13 (Sutherland, South Africa), 1m0-04, 1m0-05, 1m0-09 (Cerro Tololo, Chile); 1m0-03, 1m0-11 (Siding Spring, Australia).

**Table D1:** ASASSN-14gm: Photometric Data

| Date | JD | mag$^{(a)}$ | Filter | telescope$^{(b)}$ | Date | JD | mag$^{(a)}$ | Filter | telescope$^{(b)}$ |
|---|---|---|---|---|---|---|---|---|---|
| 2015-01-19 | 2457042.303 | 16.555 0.056 | *i* | 1m0-10 | 2015-06-04 | 2457177.924 | 18.017 0.078 | *i* | 1m0-05 |
| 2015-01-22 | 2457045.304 | 16.562 0.051 | *i* | 1m0-10 | 2015-06-04 | 2457177.928 | 18.269 0.112 | *i* | 1m0-05 |
| 2015-01-22 | 2457045.306 | 16.659 0.052 | *i* | 1m0-10 | 2015-06-22 | 2457196.295 | 18.023 0.081 | *i* | 1m0-11 |
| 2015-01-28 | 2457050.602 | 16.652 0.052 | *i* | 1m0-08 | 2015-06-22 | 2457196.302 | 18.053 0.081 | *i* | 1m0-11 |
| 2015-01-29 | 2457051.597 | 16.768 0.059 | *i* | 1m0-08 | 2015-06-30 | 2457203.931 | 18.237 0.061 | *i* | 1m0-04 |
| 2015-01-29 | 2457051.598 | 16.666 0.061 | *i* | 1m0-08 | 2015-06-30 | 2457203.935 | 18.150 0.062 | *i* | 1m0-04 |
| 2015-02-11 | 2457064.588 | 16.794 0.059 | *i* | 1m0-08 | 2015-07-17 | 2457220.779 | 18.049 0.041 | *i* | 1m0-04 |
| 2015-02-11 | 2457064.591 | 16.812 0.058 | *i* | 1m0-08 | 2015-07-17 | 2457220.783 | 18.085 0.041 | *i* | 1m0-04 |

(a) Data have not been corrected for extinction
(b) *Swift* Telescope; LSQ (La Silla Quest, Chile); 1m0-08 (McDonald Observatory, USA); 1m0-10, 1m0-12, 1m0-13 (Sutherland, South Africa), 1m0-04, 1m0-05, 1m0-09 (Cerro Tololo, Chile); 1m0-03, 1m0-11 (Siding Spring, Australia).

**Table D1:** SN 2014cy: Photometric Data

| Date | JD | mag$^{(a)}$ | Filter | telescope$^{(b)}$ | Date | JD | mag$^{(a)}$ | Filter | telescope$^{(b)}$ |
|---|---|---|---|---|---|---|---|---|---|
| 2014-09-03 | 2456903.893 | 16.018 0.025 | *B* | 1m0-08 | 2014-12-27 | 2457018.555 | 19.382 0.185 | *B* | 1m0-08 |
| 2014-09-03 | 2456903.894 | 16.019 0.025 | *B* | 1m0-08 | 2014-12-30 | 2457021.626 | 19.934 0.179 | *B* | 1m0-08 |
| 2014-09-04 | 2456905.433 | 15.972 0.026 | *B* | 1m0-10 | 2014-12-30 | 2457021.631 | 20.543 0.198 | *B* | 1m0-08 |
| 2014-09-04 | 2456905.434 | 16.000 0.026 | *B* | 1m0-10 | 2015-01-07 | 2457029.538 | 20.718 0.519 | *B* | 1m0-05 |
| 2014-09-06 | 2456907.353 | 16.111 0.028 | *B* | 1m0-10 | 2015-01-18 | 2457040.588 | 20.338 0.518 | *B* | 1m0-08 |
| 2014-09-06 | 2456907.354 | 16.073 0.027 | *B* | 1m0-10 | 2015-01-19 | 2457041.594 | 20.398 0.277 | *B* | 1m0-08 |
| 2014-09-11 | 2456912.077 | 16.177 0.025 | *B* | 1m0-11 | 2015-01-19 | 2457041.599 | 20.534 0.404 | *B* | 1m0-08 |
| 2014-09-11 | 2456912.078 | 16.130 0.025 | *B* | 1m0-11 | 2015-02-11 | 2457064.570 | 20.111 0.320 | *B* | 1m0-08 |
| 2014-09-13 | 2456914.197 | 16.239 0.025 | *B* | 1m0-03 | 2014-09-03 | 2456903.897 | 16.164 0.021 | *g* | 1m0-08 |
| 2014-09-13 | 2456914.198 | 16.247 0.025 | *B* | 1m0-03 | 2014-09-03 | 2456903.897 | 16.195 0.027 | *g* | 1m0-08 |
| 2014-09-17 | 2456918.061 | 16.357 0.025 | *B* | 1m0-11 | 2014-09-04 | 2456905.436 | 16.080 0.024 | *g* | 1m0-10 |
| 2014-09-17 | 2456918.062 | 16.360 0.025 | *B* | 1m0-11 | 2014-09-04 | 2456905.437 | 16.102 0.025 | *g* | 1m0-10 |
| 2014-09-20 | 2456920.915 | 16.591 0.026 | *B* | 1m0-08 | 2014-09-06 | 2456907.356 | 16.172 0.040 | *g* | 1m0-10 |
| 2014-09-20 | 2456920.916 | 16.589 0.058 | *B* | 1m0-08 | 2014-09-06 | 2456907.357 | 16.291 0.047 | *g* | 1m0-10 |
| 2014-09-21 | 2456922.463 | 16.574 0.029 | *B* | 1m0-10 | 2014-09-08 | 2456909.436 | 16.369 0.053 | *g* | 1m0-12 |
| 2014-09-21 | 2456922.464 | 16.619 0.039 | *B* | 1m0-10 | 2014-09-08 | 2456909.436 | 16.305 0.042 | *g* | 1m0-12 |
| 2014-09-23 | 2456924.111 | 16.536 0.039 | *B* | 1m0-11 | 2014-09-11 | 2456912.080 | 16.138 0.013 | *g* | 1m0-11 |
| 2014-09-23 | 2456924.112 | 16.621 0.043 | *B* | 1m0-11 | 2014-09-11 | 2456912.081 | 16.146 0.015 | *g* | 1m0-11 |
| 2014-09-27 | 2456928.066 | 16.721 0.055 | *B* | 1m0-11 | 2014-09-13 | 2456914.200 | 16.216 0.031 | *g* | 1m0-03 |
| 2014-10-02 | 2456932.986 | 17.178 0.053 | *B* | 1m0-11 | 2014-09-13 | 2456914.201 | 16.205 0.028 | *g* | 1m0-03 |
| 2014-10-02 | 2456932.987 | 17.130 0.052 | *B* | 1m0-11 | 2014-09-17 | 2456918.064 | 16.268 0.018 | *g* | 1m0-11 |
| 2014-10-09 | 2456940.454 | 17.331 0.031 | *B* | 1m0-12 | 2014-09-17 | 2456918.065 | 16.323 0.021 | *g* | 1m0-11 |
| 2014-10-09 | 2456940.455 | 17.364 0.028 | *B* | 1m0-12 | 2014-09-20 | 2456920.533 | 16.350 0.021 | *g* | 1m0-12 |
| 2014-10-09 | 2456940.483 | 17.523 0.037 | *B* | 1m0-12 | 2014-09-20 | 2456920.918 | 16.460 0.032 | *g* | 1m0-08 |
| 2014-10-09 | 2456940.484 | 17.427 0.033 | *B* | 1m0-12 | 2014-09-20 | 2456920.919 | 16.415 0.029 | *g* | 1m0-08 |
| 2014-10-13 | 2456944.284 | 17.655 0.040 | *B* | 1m0-12 | 2014-09-21 | 2456922.467 | 16.419 0.017 | *g* | 1m0-10 |
| 2014-10-15 | 2456945.620 | 17.584 0.030 | *B* | 1m0-08 | 2014-09-21 | 2456922.467 | 16.405 0.016 | *g* | 1m0-10 |
| 2014-10-15 | 2456945.621 | 17.672 0.119 | *B* | 1m0-08 | 2014-09-23 | 2456924.114 | 16.351 0.020 | *g* | 1m0-11 |
| 2014-10-22 | 2456953.317 | 17.726 0.090 | *B* | 1m0-12 | 2014-09-23 | 2456924.115 | 16.348 0.019 | *g* | 1m0-11 |
| 2014-10-22 | 2456953.317 | 17.684 0.084 | *B* | 1m0-12 | 2014-09-27 | 2456928.069 | 16.443 0.018 | *g* | 1m0-11 |
| 2014-10-30 | 2456961.080 | 17.781 0.033 | *B* | 1m0-03 | 2014-09-27 | 2456928.070 | 16.511 0.018 | *g* | 1m0-11 |
| 2014-10-30 | 2456961.081 | 17.817 0.032 | *B* | 1m0-03 | 2014-10-02 | 2456932.989 | 16.727 0.021 | *g* | 1m0-11 |
| 2014-11-19 | 2456980.556 | 18.237 0.039 | *B* | 1m0-05 | 2014-10-02 | 2456932.990 | 16.721 0.022 | *g* | 1m0-11 |
| 2014-11-19 | 2456980.559 | 18.169 0.035 | *B* | 1m0-05 | 2014-10-09 | 2456940.458 | 17.022 0.065 | *g* | 1m0-12 |
| 2014-11-19 | 2456980.925 | 18.290 0.051 | *B* | 1m0-03 | 2014-10-09 | 2456940.459 | 17.051 0.065 | *g* | 1m0-12 |
| 2014-11-19 | 2456981.272 | 18.274 0.036 | *B* | 1m0-12 | 2014-10-09 | 2456940.487 | 17.139 0.076 | *g* | 1m0-12 |
| 2014-11-19 | 2456981.275 | 18.256 0.045 | *B* | 1m0-12 | 2014-10-09 | 2456940.487 | 17.188 0.063 | *g* | 1m0-12 |
| 2014-11-25 | 2456987.319 | 18.269 0.053 | *B* | 1m0-13 | 2014-10-13 | 2456944.287 | 17.033 0.049 | *g* | 1m0-12 |
| 2014-11-25 | 2456987.324 | 18.291 0.041 | *B* | 1m0-13 | 2014-10-13 | 2456944.288 | 17.006 0.029 | *g* | 1m0-12 |
| 2014-11-28 | 2456989.590 | 18.501 0.043 | *B* | 1m0-05 | 2014-10-15 | 2456945.624 | 16.943 0.013 | *g* | 1m0-08 |
| 2014-11-28 | 2456989.595 | 18.364 0.039 | *B* | 1m0-05 | 2014-10-15 | 2456945.624 | 16.978 0.010 | *g* | 1m0-08 |
| 2014-11-29 | 2456990.535 | 18.347 0.040 | *B* | 1m0-08 | 2014-10-22 | 2456953.320 | 17.124 0.037 | *g* | 1m0-12 |
| 2014-11-29 | 2456990.540 | 18.430 0.044 | *B* | 1m0-08 | 2014-10-22 | 2456953.321 | 17.181 0.037 | *g* | 1m0-12 |
| 2014-12-03 | 2456994.523 | 18.659 0.052 | *B* | 1m0-05 | 2014-10-30 | 2456961.083 | 17.281 0.045 | *g* | 1m0-03 |
| 2014-12-09 | 2457000.942 | 18.455 0.086 | *B* | 1m0-11 | 2014-11-07 | 2456968.908 | 17.299 0.058 | *g* | 1m0-11 |
| 2014-12-09 | 2457000.946 | 18.577 0.096 | *B* | 1m0-11 | 2014-11-07 | 2456968.908 | 17.192 0.015 | *g* | 1m0-11 |
| 2014-12-12 | 2457003.931 | 18.545 0.077 | *B* | 1m0-11 | 2014-11-11 | 2456972.684 | 17.172 0.063 | *g* | 1m0-08 |
| 2014-12-12 | 2457003.936 | 18.659 0.073 | *B* | 1m0-11 | 2014-11-11 | 2456972.686 | 17.212 0.029 | *g* | 1m0-08 |
| 2014-12-14 | 2457006.280 | 18.869 0.103 | *B* | 1m0-12 | 2014-11-19 | 2456980.565 | 17.333 0.014 | *g* | 1m0-05 |
| 2014-12-14 | 2457006.285 | 18.659 0.058 | *B* | 1m0-12 | 2014-11-19 | 2456980.567 | 17.338 0.013 | *g* | 1m0-05 |
| 2014-12-15 | 2457006.921 | 18.900 0.074 | *B* | 1m0-03 | 2014-11-19 | 2456980.936 | 17.392 0.013 | *g* | 1m0-03 |
| 2014-12-15 | 2457006.926 | 18.759 0.065 | *B* | 1m0-03 | 2014-11-19 | 2456981.281 | 17.372 0.026 | *g* | 1m0-12 |
| 2014-12-16 | 2457007.671 | 18.879 0.060 | *B* | 1m0-08 | 2014-11-25 | 2456987.334 | 17.458 0.018 | *g* | 1m0-13 |
| 2014-12-20 | 2457011.642 | 18.968 0.078 | *B* | 1m0-08 | 2014-11-25 | 2456987.339 | 17.450 0.017 | *g* | 1m0-13 |
| 2014-12-20 | 2457011.647 | 18.776 0.069 | *B* | 1m0-08 | 2014-11-28 | 2456989.605 | 17.596 0.050 | *g* | 1m0-05 |
| 2014-12-24 | 2457015.532 | 19.403 0.086 | *B* | 1m0-05 | 2014-11-28 | 2456989.610 | 17.595 0.047 | *g* | 1m0-05 |
| 2014-12-24 | 2457015.537 | 19.605 0.119 | *B* | 1m0-05 | 2014-11-29 | 2456990.555 | 17.522 0.015 | *g* | 1m0-08 |
| 2014-12-25 | 2457016.533 | 19.204 0.141 | *B* | 1m0-05 | 2014-12-03 | 2456994.538 | 17.593 0.014 | *g* | 1m0-05 |
| 2014-12-25 | 2457016.537 | 19.175 0.089 | *B* | 1m0-05 | 2014-12-03 | 2456994.543 | 17.570 0.015 | *g* | 1m0-05 |
| 2014-12-27 | 2457018.550 | 20.120 0.421 | *B* | 1m0-08 | 2014-12-14 | 2457006.297 | 17.647 0.040 | *g* | 1m0-12 |

(a) Data have not been corrected for extinction
(b) *Swift* Telescope; LSQ (La Silla Quest, Chile); 1m0-08 (McDonald Observatory, USA); 1m0-10, 1m0-12, 1m0-13 (Sutherland, South Africa), 1m0-04, 1m0-05, 1m0-09 (Cerro Tololo, Chile); 1m0-03, 1m0-11 (Siding Spring, Australia).

**Table D1:** SN 2014cy: Photometric Data

| Date | JD | mag$^{(a)}$ | Filter | telescope$^{(b)}$ | Date | JD | mag$^{(a)}$ | Filter | telescope$^{(b)}$ |
|---|---|---|---|---|---|---|---|---|---|
| 2014-12-14 | 2457006.302 | 17.686 0.045 | $g$ | 1m0-12 | 2014-11-29 | 2456990.547 | 16.747 0.037 | $V$ | 1m0-08 |
| 2014-12-16 | 2457007.686 | 17.861 0.018 | $g$ | 1m0-08 | 2014-12-03 | 2456994.533 | 16.805 0.025 | $V$ | 1m0-05 |
| 2014-12-16 | 2457007.690 | 18.048 0.058 | $g$ | 1m0-08 | 2014-12-03 | 2456994.535 | 16.828 0.025 | $V$ | 1m0-05 |
| 2014-12-20 | 2457011.657 | 18.064 0.020 | $g$ | 1m0-08 | 2014-12-12 | 2457003.941 | 17.007 0.024 | $V$ | 1m0-11 |
| 2014-12-20 | 2457011.662 | 18.128 0.025 | $g$ | 1m0-08 | 2014-12-12 | 2457003.943 | 16.976 0.032 | $V$ | 1m0-11 |
| 2014-12-25 | 2457016.660 | 18.376 0.044 | $g$ | 1m0-08 | 2014-12-15 | 2457006.931 | 17.085 0.025 | $V$ | 1m0-03 |
| 2014-12-30 | 2457021.648 | 18.731 0.093 | $g$ | 1m0-08 | 2014-12-15 | 2457006.933 | 17.055 0.025 | $V$ | 1m0-03 |
| 2014-12-30 | 2457021.653 | 19.488 0.256 | $g$ | 1m0-08 | 2014-12-16 | 2457007.680 | 17.073 0.025 | $V$ | 1m0-08 |
| 2015-01-05 | 2457027.534 | 19.907 0.192 | $g$ | 1m0-05 | 2014-12-16 | 2457007.683 | 17.133 0.025 | $V$ | 1m0-08 |
| 2015-01-05 | 2457027.539 | 20.249 0.195 | $g$ | 1m0-05 | 2014-12-20 | 2457011.652 | 17.236 0.028 | $V$ | 1m0-08 |
| 2015-01-19 | 2457041.617 | 21.651 0.526 | $g$ | 1m0-08 | 2014-12-20 | 2457011.654 | 17.256 0.031 | $V$ | 1m0-08 |
| 2015-01-21 | 2457043.609 | 21.754 0.517 | $g$ | 1m0-08 | 2014-12-24 | 2457015.542 | 17.390 0.028 | $V$ | 1m0-05 |
| 2015-01-28 | 2457050.557 | 21.326 0.186 | $g$ | 1m0-08 | 2014-12-24 | 2457015.546 | 17.412 0.028 | $V$ | 1m0-05 |
| 2014-09-03 | 2456903.895 | 15.957 0.052 | $V$ | 1m0-08 | 2014-12-25 | 2457016.542 | 17.473 0.030 | $V$ | 1m0-05 |
| 2014-09-03 | 2456903.896 | 15.906 0.023 | $V$ | 1m0-08 | 2014-12-25 | 2457016.546 | 17.462 0.028 | $V$ | 1m0-05 |
| 2014-09-04 | 2456905.435 | 15.918 0.041 | $V$ | 1m0-10 | 2014-12-27 | 2457018.560 | 17.509 0.037 | $V$ | 1m0-08 |
| 2014-09-04 | 2456905.435 | 15.896 0.037 | $V$ | 1m0-10 | 2014-12-30 | 2457021.639 | 18.669 0.279 | $V$ | 1m0-08 |
| 2014-09-06 | 2456907.354 | 16.149 0.027 | $V$ | 1m0-10 | 2015-01-20 | 2457042.571 | 21.069 0.432 | $V$ | 1m0-08 |
| 2014-09-06 | 2456907.355 | 16.034 0.025 | $V$ | 1m0-10 | 2015-01-21 | 2457043.597 | 20.050 0.193 | $V$ | 1m0-08 |
| 2014-09-08 | 2456909.434 | 15.847 0.030 | $V$ | 1m0-12 | 2015-02-03 | 2457056.590 | 19.614 0.524 | $V$ | 1m0-08 |
| 2014-09-08 | 2456909.435 | 15.828 0.032 | $V$ | 1m0-12 | 2015-02-09 | 2457062.567 | 20.677 0.323 | $V$ | 1m0-08 |
| 2014-09-11 | 2456912.078 | 15.975 0.035 | $V$ | 1m0-11 | 2014-08-29 | 2456898.822 | $<$ 19.000 | $r$ | Atel/CBAT |
| 2014-09-11 | 2456912.079 | 16.071 0.038 | $V$ | 1m0-11 | 2014-08-31 | 2456900.822 | 15.800 0.100 | $r$ | Atel/CBAT |
| 2014-09-13 | 2456914.199 | 15.887 0.023 | $V$ | 1m0-03 | 2014-09-03 | 2456903.899 | 15.928 0.011 | $r$ | 1m0-08 |
| 2014-09-13 | 2456914.199 | 15.947 0.022 | $V$ | 1m0-03 | 2014-09-03 | 2456903.899 | 15.972 0.008 | $r$ | 1m0-08 |
| 2014-09-17 | 2456918.063 | 15.922 0.023 | $V$ | 1m0-11 | 2014-09-08 | 2456909.438 | 15.800 0.015 | $r$ | 1m0-12 |
| 2014-09-17 | 2456918.064 | 15.944 0.023 | $V$ | 1m0-11 | 2014-09-08 | 2456909.438 | 15.861 0.011 | $r$ | 1m0-12 |
| 2014-09-20 | 2456920.917 | 16.168 0.067 | $V$ | 1m0-08 | 2014-09-11 | 2456912.082 | 15.845 0.022 | $r$ | 1m0-11 |
| 2014-09-20 | 2456920.917 | 16.010 0.056 | $V$ | 1m0-08 | 2014-09-11 | 2456912.082 | 15.899 0.018 | $r$ | 1m0-11 |
| 2014-09-21 | 2456922.465 | 16.050 0.027 | $V$ | 1m0-10 | 2014-09-17 | 2456918.066 | 15.888 0.027 | $r$ | 1m0-11 |
| 2014-09-21 | 2456922.466 | 16.052 0.027 | $V$ | 1m0-10 | 2014-09-17 | 2456918.067 | 15.947 0.026 | $r$ | 1m0-11 |
| 2014-09-23 | 2456924.113 | 15.994 0.032 | $V$ | 1m0-11 | 2014-09-20 | 2456920.920 | 16.002 0.041 | $r$ | 1m0-08 |
| 2014-09-23 | 2456924.113 | 16.037 0.026 | $V$ | 1m0-11 | 2014-09-20 | 2456920.921 | 16.013 0.050 | $r$ | 1m0-08 |
| 2014-09-27 | 2456928.068 | 16.044 0.035 | $V$ | 1m0-11 | 2014-09-21 | 2456922.468 | 16.022 0.035 | $r$ | 1m0-10 |
| 2014-09-27 | 2456928.068 | 16.153 0.082 | $V$ | 1m0-11 | 2014-09-21 | 2456922.469 | 15.955 0.022 | $r$ | 1m0-10 |
| 2014-10-02 | 2456932.988 | 16.216 0.024 | $V$ | 1m0-11 | 2014-09-23 | 2456924.116 | 15.915 0.030 | $r$ | 1m0-11 |
| 2014-10-02 | 2456932.989 | 16.189 0.038 | $V$ | 1m0-11 | 2014-09-23 | 2456924.117 | 15.922 0.026 | $r$ | 1m0-11 |
| 2014-10-09 | 2456940.456 | 16.283 0.023 | $V$ | 1m0-12 | 2014-09-27 | 2456928.071 | 15.973 0.023 | $r$ | 1m0-11 |
| 2014-10-09 | 2456940.457 | 16.397 0.076 | $V$ | 1m0-12 | 2014-09-27 | 2456928.071 | 15.966 0.010 | $r$ | 1m0-11 |
| 2014-10-09 | 2456940.485 | 16.588 0.085 | $V$ | 1m0-12 | 2014-10-02 | 2456932.991 | 16.046 0.027 | $r$ | 1m0-11 |
| 2014-10-09 | 2456940.486 | 16.439 0.086 | $V$ | 1m0-12 | 2014-10-02 | 2456932.992 | 16.057 0.025 | $r$ | 1m0-11 |
| 2014-10-13 | 2456944.286 | 16.444 0.032 | $V$ | 1m0-12 | 2014-10-06 | 2456936.572 | 16.140 0.046 | $r$ | 1m0-08 |
| 2014-10-13 | 2456944.286 | 16.369 0.056 | $V$ | 1m0-12 | 2014-10-09 | 2456940.460 | 16.099 0.009 | $r$ | 1m0-12 |
| 2014-10-15 | 2456945.622 | 16.491 0.061 | $V$ | 1m0-08 | 2014-10-09 | 2456940.460 | 16.089 0.012 | $r$ | 1m0-12 |
| 2014-10-15 | 2456945.623 | 16.394 0.050 | $V$ | 1m0-08 | 2014-10-09 | 2456940.489 | 16.133 0.049 | $r$ | 1m0-12 |
| 2014-10-22 | 2456953.319 | 16.394 0.025 | $V$ | 1m0-12 | 2014-10-09 | 2456940.489 | 16.320 0.071 | $r$ | 1m0-12 |
| 2014-10-22 | 2456953.319 | 16.502 0.057 | $V$ | 1m0-12 | 2014-10-13 | 2456944.289 | 16.186 0.047 | $r$ | 1m0-12 |
| 2014-10-30 | 2456961.082 | 16.469 0.024 | $V$ | 1m0-03 | 2014-10-13 | 2456944.290 | 16.115 0.045 | $r$ | 1m0-12 |
| 2014-10-30 | 2456961.082 | 16.496 0.025 | $V$ | 1m0-03 | 2014-10-15 | 2456945.625 | 16.109 0.008 | $r$ | 1m0-08 |
| 2014-11-11 | 2456972.682 | 16.429 0.062 | $V$ | 1m0-08 | 2014-10-15 | 2456945.626 | 16.094 0.009 | $r$ | 1m0-08 |
| 2014-11-19 | 2456980.562 | 16.616 0.024 | $V$ | 1m0-05 | 2014-10-22 | 2456953.322 | 16.122 0.015 | $r$ | 1m0-12 |
| 2014-11-19 | 2456980.563 | 16.627 0.024 | $V$ | 1m0-05 | 2014-10-22 | 2456953.322 | 16.117 0.013 | $r$ | 1m0-12 |
| 2014-11-19 | 2456980.932 | 16.595 0.024 | $V$ | 1m0-03 | 2014-10-30 | 2456961.085 | 16.159 0.009 | $r$ | 1m0-03 |
| 2014-11-19 | 2456981.277 | 16.638 0.023 | $V$ | 1m0-12 | 2014-10-30 | 2456961.086 | 16.125 0.014 | $r$ | 1m0-03 |
| 2014-11-19 | 2456981.279 | 16.656 0.023 | $V$ | 1m0-12 | 2014-11-07 | 2456968.910 | 16.183 0.013 | $r$ | 1m0-11 |
| 2014-11-25 | 2456987.329 | 16.695 0.026 | $V$ | 1m0-13 | 2014-11-07 | 2456968.910 | 16.201 0.015 | $r$ | 1m0-11 |
| 2014-11-25 | 2456987.331 | 16.681 0.026 | $V$ | 1m0-13 | 2014-11-11 | 2456972.689 | 16.081 0.029 | $r$ | 1m0-08 |
| 2014-11-28 | 2456989.600 | 16.725 0.024 | $V$ | 1m0-05 | 2014-11-11 | 2456972.690 | 16.205 0.018 | $r$ | 1m0-08 |
| 2014-11-28 | 2456989.603 | 16.714 0.023 | $V$ | 1m0-05 | 2014-11-19 | 2456980.570 | 16.284 0.010 | $r$ | 1m0-05 |
| 2014-11-29 | 2456990.545 | 16.756 0.035 | $V$ | 1m0-08 | 2014-11-19 | 2456980.940 | 16.288 0.008 | $r$ | 1m0-03 |

(a) Data have not been corrected for extinction
(b) *Swift* Telescope; LSQ (La Silla Quest, Chile); 1m0-08 (McDonald Observatory, USA); 1m0-10, 1m0-12, 1m0-13 (Sutherland, South Africa), 1m0-04, 1m0-05, 1m0-09 (Cerro Tololo, Chile); 1m0-03, 1m0-11 (Siding Spring, Australia).

**Table D1:** SN 2014cy: Photometric Data

| Date | JD | mag[(a)] | Filter | telescope[(b)] | Date | JD | mag[(a)] | Filter | telescope[(b)] |
|---|---|---|---|---|---|---|---|---|---|
| 2014-11-19 | 2456981.286 | 16.261 0.010 | *r* | 1m0-12 | 2014-09-27 | 2456928.073 | 15.970 0.016 | *i* | 1m0-11 |
| 2014-11-19 | 2456981.287 | 16.264 0.017 | *r* | 1m0-12 | 2014-10-02 | 2456932.993 | 16.012 0.013 | *i* | 1m0-11 |
| 2014-11-25 | 2456987.344 | 16.319 0.013 | *r* | 1m0-13 | 2014-10-02 | 2456932.993 | 16.056 0.020 | *i* | 1m0-11 |
| 2014-11-25 | 2456987.346 | 16.310 0.013 | *r* | 1m0-13 | 2014-10-06 | 2456936.574 | 16.134 0.024 | *i* | 1m0-08 |
| 2014-11-28 | 2456989.615 | 16.348 0.009 | *r* | 1m0-05 | 2014-10-06 | 2456936.574 | 16.185 0.070 | *i* | 1m0-08 |
| 2014-11-29 | 2456990.560 | 16.373 0.008 | *r* | 1m0-08 | 2014-10-09 | 2456940.461 | 16.028 0.013 | *i* | 1m0-12 |
| 2014-11-29 | 2456990.562 | 16.396 0.008 | *r* | 1m0-08 | 2014-10-09 | 2456940.490 | 16.065 0.015 | *i* | 1m0-12 |
| 2014-12-03 | 2456994.548 | 16.397 0.011 | *r* | 1m0-05 | 2014-10-09 | 2456940.491 | 16.064 0.011 | *i* | 1m0-12 |
| 2014-12-03 | 2456994.550 | 16.400 0.009 | *r* | 1m0-05 | 2014-10-13 | 2456944.290 | 16.178 0.083 | *i* | 1m0-12 |
| 2014-12-16 | 2457007.695 | 16.661 0.009 | *r* | 1m0-08 | 2014-10-13 | 2456944.291 | 16.050 0.064 | *i* | 1m0-12 |
| 2014-12-16 | 2457007.698 | 16.637 0.009 | *r* | 1m0-08 | 2014-10-15 | 2456945.626 | 16.031 0.050 | *i* | 1m0-08 |
| 2014-12-20 | 2457011.666 | 16.785 0.020 | *r* | 1m0-08 | 2014-10-15 | 2456945.627 | 16.063 0.044 | *i* | 1m0-08 |
| 2014-12-20 | 2457011.669 | 16.829 0.018 | *r* | 1m0-08 | 2014-10-22 | 2456953.323 | 16.075 0.016 | *i* | 1m0-12 |
| 2014-12-25 | 2457016.673 | 17.311 0.058 | *r* | 1m0-08 | 2014-10-22 | 2456953.323 | 16.069 0.049 | *i* | 1m0-12 |
| 2014-12-30 | 2457021.658 | 17.757 0.098 | *r* | 1m0-08 | 2014-10-30 | 2456961.086 | 16.069 0.013 | *i* | 1m0-03 |
| 2014-12-30 | 2457021.661 | 17.605 0.084 | *r* | 1m0-08 | 2014-10-30 | 2456961.087 | 16.103 0.014 | *i* | 1m0-03 |
| 2015-01-05 | 2457027.544 | 19.507 0.207 | *r* | 1m0-05 | 2014-11-07 | 2456968.911 | 16.072 0.019 | *i* | 1m0-11 |
| 2015-01-21 | 2457043.614 | 20.417 0.286 | *r* | 1m0-08 | 2014-11-07 | 2456968.911 | 16.149 0.017 | *i* | 1m0-11 |
| 2015-01-21 | 2457043.618 | 19.719 0.161 | *r* | 1m0-08 | 2014-11-11 | 2456972.692 | 16.006 0.030 | *i* | 1m0-08 |
| 2015-01-26 | 2457048.599 | 19.641 0.195 | *r* | 1m0-08 | 2014-11-19 | 2456980.942 | 16.274 0.026 | *i* | 1m0-03 |
| 2015-01-28 | 2457050.567 | 19.998 0.102 | *r* | 1m0-08 | 2014-11-19 | 2456981.289 | 16.176 0.013 | *i* | 1m0-12 |
| 2015-01-28 | 2457050.571 | 19.808 0.097 | *r* | 1m0-08 | 2014-11-19 | 2456981.291 | 16.168 0.015 | *i* | 1m0-12 |
| 2014-09-03 | 2456903.900 | 16.251 0.052 | *i* | 1m0-08 | 2014-11-25 | 2456987.349 | 16.163 0.024 | *i* | 1m0-13 |
| 2014-09-03 | 2456903.900 | 16.198 0.040 | *i* | 1m0-08 | 2014-11-25 | 2456987.352 | 16.282 0.023 | *i* | 1m0-13 |
| 2014-09-04 | 2456905.439 | 16.057 0.044 | *i* | 1m0-10 | 2014-11-28 | 2456989.620 | 16.224 0.007 | *i* | 1m0-05 |
| 2014-09-04 | 2456905.440 | 16.006 0.048 | *i* | 1m0-10 | 2014-11-28 | 2456989.623 | 16.231 0.008 | *i* | 1m0-05 |
| 2014-09-06 | 2456907.359 | 16.087 0.288 | *i* | 1m0-10 | 2014-11-29 | 2456990.565 | 16.244 0.009 | *i* | 1m0-08 |
| 2014-09-08 | 2456909.439 | 16.030 0.018 | *i* | 1m0-12 | 2014-11-29 | 2456990.567 | 16.252 0.008 | *i* | 1m0-08 |
| 2014-09-08 | 2456909.439 | 16.028 0.018 | *i* | 1m0-12 | 2014-12-03 | 2456994.553 | 16.300 0.010 | *i* | 1m0-05 |
| 2014-09-11 | 2456912.083 | 16.026 0.021 | *i* | 1m0-11 | 2014-12-16 | 2457007.700 | 16.546 0.009 | *i* | 1m0-08 |
| 2014-09-11 | 2456912.083 | 16.000 0.018 | *i* | 1m0-11 | 2014-12-16 | 2457007.703 | 16.543 0.012 | *i* | 1m0-08 |
| 2014-09-13 | 2456914.203 | 15.995 0.011 | *i* | 1m0-03 | 2014-12-20 | 2457011.672 | 16.667 0.022 | *i* | 1m0-08 |
| 2014-09-17 | 2456918.067 | 15.983 0.033 | *i* | 1m0-11 | 2014-12-20 | 2457011.674 | 16.678 0.025 | *i* | 1m0-08 |
| 2014-09-17 | 2456918.068 | 16.050 0.042 | *i* | 1m0-11 | 2014-12-25 | 2457016.677 | 17.545 0.086 | *i* | 1m0-08 |
| 2014-09-20 | 2456920.921 | 15.977 0.064 | *i* | 1m0-08 | 2015-01-05 | 2457027.552 | 19.031 0.150 | *i* | 1m0-05 |
| 2014-09-20 | 2456920.922 | 15.911 0.011 | *i* | 1m0-08 | 2015-01-05 | 2457027.555 | 19.177 0.161 | *i* | 1m0-05 |
| 2014-09-21 | 2456922.470 | 16.020 0.036 | *i* | 1m0-10 | 2015-01-19 | 2457041.631 | 19.496 0.205 | *i* | 1m0-08 |
| 2014-09-21 | 2456922.470 | 16.011 0.032 | *i* | 1m0-10 | 2015-01-20 | 2457042.610 | 20.268 0.250 | *i* | 1m0-08 |
| 2014-09-23 | 2456924.117 | 15.884 0.028 | *i* | 1m0-11 | 2015-01-26 | 2457048.603 | 20.897 0.278 | *i* | 1m0-08 |
| 2014-09-23 | 2456924.118 | 15.922 0.035 | *i* | 1m0-11 | 2015-01-28 | 2457050.575 | 19.902 0.130 | *i* | 1m0-08 |
| 2014-09-27 | 2456928.072 | 15.961 0.020 | *i* | 1m0-11 | 2015-01-28 | 2457050.578 | 20.190 0.138 | *i* | 1m0-08 |

(a) Data have not been corrected for extinction
(b) *Swift* Telescope; LSQ (La Silla Quest, Chile); 1m0-08 (McDonald Observatory, USA); 1m0-10, 1m0-12, 1m0-13 (Sutherland, South Africa), 1m0-04, 1m0-05, 1m0-09 (Cerro Tololo, Chile); 1m0-03, 1m0-11 (Siding Spring, Australia).

**Table D1:** ASASSN-14kg: Photometric Data

| Date | JD | mag[(a)] | Filter | telescope[(b)] | Date | JD | mag[(a)] | Filter | telescope[(b)] |
|---|---|---|---|---|---|---|---|---|---|
| 2014-11-27 | 2456988.767 | 16.448 0.020 | *B* | 1m0-08 | 2015-01-28 | 2457050.651 | 18.563 0.037 | *g* | 1m0-08 |
| 2014-11-27 | 2456988.769 | 16.517 0.020 | *B* | 1m0-08 | 2015-01-28 | 2457050.654 | 18.557 0.038 | *g* | 1m0-08 |
| 2014-11-27 | 2456988.832 | 16.458 0.019 | *B* | 1m0-08 | 2015-01-29 | 2457051.655 | 18.497 0.052 | *g* | 1m0-08 |
| 2014-11-27 | 2456988.835 | 16.544 0.019 | *B* | 1m0-08 | 2015-01-29 | 2457051.658 | 18.548 0.052 | *g* | 1m0-08 |
| 2014-11-28 | 2456989.700 | 16.480 0.020 | *B* | 1m0-08 | 2015-02-05 | 2457058.613 | 18.752 0.072 | *g* | 1m0-08 |
| 2014-11-28 | 2456989.703 | 16.478 0.019 | *B* | 1m0-08 | 2015-02-05 | 2457058.616 | 18.770 0.076 | *g* | 1m0-08 |
| 2014-11-30 | 2456991.578 | 16.551 0.021 | *B* | 1m0-08 | 2015-02-09 | 2457062.621 | 19.000 0.076 | *g* | 1m0-08 |
| 2014-11-30 | 2456991.581 | 16.557 0.020 | *B* | 1m0-08 | 2015-02-09 | 2457062.625 | 19.031 0.073 | *g* | 1m0-08 |
| 2014-12-01 | 2456992.642 | 16.652 0.022 | *B* | 1m0-08 | 2015-02-11 | 2457064.642 | 19.026 0.092 | *g* | 1m0-08 |
| 2014-12-01 | 2456992.645 | 16.625 0.023 | *B* | 1m0-08 | 2015-02-11 | 2457064.646 | 18.962 0.076 | *g* | 1m0-08 |
| 2014-12-02 | 2456993.783 | 16.647 0.030 | *B* | 1m0-08 | 2015-02-19 | 2457072.609 | 19.144 0.082 | *g* | 1m0-08 |
| 2014-12-02 | 2456993.785 | 16.625 0.022 | *B* | 1m0-08 | 2015-02-20 | 2457073.618 | 19.340 0.084 | *g* | 1m0-08 |
| 2014-12-12 | 2457003.771 | 17.240 0.029 | *B* | 1m0-08 | 2015-02-22 | 2457075.574 | 19.423 0.102 | *g* | 1m0-08 |
| 2014-12-12 | 2457003.774 | 17.231 0.025 | *B* | 1m0-08 | 2015-03-07 | 2457088.577 | 19.847 0.238 | *g* | 1m0-08 |
| 2014-12-16 | 2457007.728 | 17.479 0.038 | *B* | 1m0-08 | 2015-03-07 | 2457088.581 | 20.061 0.176 | *g* | 1m0-08 |
| 2014-12-16 | 2457007.730 | 17.445 0.036 | *B* | 1m0-08 | 2014-11-11 | 2456972.880 | $< 16.900$ | *V* | Atel/CBAT |
| 2014-12-25 | 2457016.711 | 17.888 0.053 | *B* | 1m0-08 | 2014-11-12 | 2456973.860 | 16.900 0.500 | *V* | Atel/CBAT |
| 2014-12-29 | 2457020.642 | 18.253 0.079 | *B* | 1m0-08 | 2014-11-17 | 2456978.860 | 16.400 0.100 | *V* | Atel/CBAT |
| 2014-12-29 | 2457020.644 | 18.320 0.079 | *B* | 1m0-08 | 2014-11-27 | 2456988.772 | 16.159 0.023 | *V* | 1m0-08 |
| 2015-01-16 | 2457038.686 | 18.972 0.120 | *B* | 1m0-08 | 2014-11-27 | 2456988.774 | 16.166 0.024 | *V* | 1m0-08 |
| 2015-01-21 | 2457043.688 | 19.017 0.083 | *B* | 1m0-08 | 2014-11-27 | 2456988.839 | 16.175 0.022 | *V* | 1m0-08 |
| 2015-01-21 | 2457043.691 | 18.979 0.081 | *B* | 1m0-08 | 2014-11-28 | 2456989.707 | 16.170 0.022 | *V* | 1m0-08 |
| 2015-01-28 | 2457050.638 | 19.364 0.120 | *B* | 1m0-08 | 2014-11-30 | 2456991.583 | 16.165 0.023 | *V* | 1m0-08 |
| 2015-01-28 | 2457050.642 | 19.323 0.157 | *B* | 1m0-08 | 2014-11-30 | 2456991.585 | 16.174 0.024 | *V* | 1m0-08 |
| 2015-01-29 | 2457051.642 | 19.121 0.116 | *B* | 1m0-08 | 2014-12-01 | 2456992.647 | 16.151 0.024 | *V* | 1m0-08 |
| 2015-01-29 | 2457051.646 | 19.379 0.150 | *B* | 1m0-08 | 2014-12-01 | 2456992.649 | 16.158 0.025 | *V* | 1m0-08 |
| 2015-02-05 | 2457058.600 | 19.683 0.225 | *B* | 1m0-08 | 2014-12-02 | 2456993.788 | 16.190 0.028 | *V* | 1m0-08 |
| 2015-02-05 | 2457058.604 | 19.758 0.260 | *B* | 1m0-08 | 2014-12-12 | 2457003.776 | 16.314 0.024 | *V* | 1m0-08 |
| 2015-02-09 | 2457062.609 | 19.533 0.262 | *B* | 1m0-08 | 2014-12-12 | 2457003.778 | 16.321 0.026 | *V* | 1m0-08 |
| 2015-02-09 | 2457062.612 | 19.715 0.208 | *B* | 1m0-08 | 2014-12-16 | 2457007.733 | 16.458 0.023 | *V* | 1m0-08 |
| 2015-02-11 | 2457064.629 | 19.927 0.256 | *B* | 1m0-08 | 2014-12-16 | 2457007.734 | 16.460 0.023 | *V* | 1m0-08 |
| 2015-02-11 | 2457064.632 | 19.908 0.297 | *B* | 1m0-08 | 2014-12-20 | 2457011.739 | 16.587 0.024 | *V* | 1m0-08 |
| 2015-02-19 | 2457072.569 | 20.735 0.467 | *B* | 1m0-08 | 2014-12-20 | 2457011.740 | 16.601 0.028 | *V* | 1m0-08 |
| 2015-02-19 | 2457072.573 | 20.191 0.264 | *B* | 1m0-08 | 2014-12-25 | 2457016.714 | 16.693 0.039 | *V* | 1m0-08 |
| 2014-11-27 | 2456988.775 | 16.211 0.013 | *g* | 1m0-08 | 2014-12-29 | 2457020.647 | 16.783 0.041 | *V* | 1m0-08 |
| 2014-11-27 | 2456988.778 | 16.225 0.013 | *g* | 1m0-08 | 2014-12-29 | 2457020.649 | 16.865 0.035 | *V* | 1m0-08 |
| 2014-11-27 | 2456988.841 | 16.232 0.013 | *g* | 1m0-08 | 2014-12-30 | 2457021.682 | 16.857 0.055 | *V* | 1m0-08 |
| 2014-11-27 | 2456988.843 | 16.219 0.013 | *g* | 1m0-08 | 2014-12-30 | 2457021.683 | 16.886 0.054 | *V* | 1m0-08 |
| 2014-11-28 | 2456989.709 | 16.237 0.013 | *g* | 1m0-08 | 2015-01-16 | 2457038.689 | 17.258 0.035 | *V* | 1m0-08 |
| 2014-11-28 | 2456989.712 | 16.242 0.013 | *g* | 1m0-08 | 2015-01-16 | 2457038.691 | 17.326 0.046 | *V* | 1m0-08 |
| 2014-11-30 | 2456991.587 | 16.270 0.014 | *g* | 1m0-08 | 2015-01-21 | 2457043.695 | 17.395 0.030 | *V* | 1m0-08 |
| 2014-11-30 | 2456991.589 | 16.264 0.015 | *g* | 1m0-08 | 2015-01-21 | 2457043.698 | 17.405 0.028 | *V* | 1m0-08 |
| 2014-12-01 | 2456992.651 | 16.272 0.013 | *g* | 1m0-08 | 2015-01-24 | 2457046.655 | 17.421 0.087 | *V* | 1m0-08 |
| 2014-12-01 | 2456992.653 | 16.299 0.013 | *g* | 1m0-08 | 2015-01-28 | 2457050.645 | 17.576 0.030 | *V* | 1m0-08 |
| 2014-12-02 | 2456993.794 | 16.317 0.013 | *g* | 1m0-08 | 2015-01-28 | 2457050.648 | 17.578 0.033 | *V* | 1m0-08 |
| 2014-12-12 | 2457003.780 | 16.728 0.015 | *g* | 1m0-08 | 2015-01-29 | 2457051.649 | 17.583 0.038 | *V* | 1m0-08 |
| 2014-12-12 | 2457003.782 | 16.731 0.014 | *g* | 1m0-08 | 2015-01-29 | 2457051.652 | 17.590 0.035 | *V* | 1m0-08 |
| 2014-12-16 | 2457007.736 | 16.937 0.016 | *g* | 1m0-08 | 2015-02-05 | 2457058.610 | 17.745 0.033 | *V* | 1m0-08 |
| 2014-12-16 | 2457007.739 | 16.931 0.017 | *g* | 1m0-08 | 2015-02-09 | 2457062.616 | 17.875 0.044 | *V* | 1m0-08 |
| 2014-12-20 | 2457011.745 | 17.136 0.022 | *g* | 1m0-08 | 2015-02-09 | 2457062.619 | 17.846 0.034 | *V* | 1m0-08 |
| 2014-12-25 | 2457016.717 | 17.237 0.032 | *g* | 1m0-08 | 2015-02-11 | 2457064.636 | 17.904 0.035 | *V* | 1m0-08 |
| 2014-12-25 | 2457016.720 | 17.260 0.032 | *g* | 1m0-08 | 2015-02-11 | 2457064.639 | 17.876 0.039 | *V* | 1m0-08 |
| 2014-12-29 | 2457020.650 | 17.474 0.024 | *g* | 1m0-08 | 2015-02-19 | 2457072.576 | 18.012 0.046 | *V* | 1m0-08 |
| 2014-12-29 | 2457020.653 | 17.557 0.026 | *g* | 1m0-08 | 2015-02-19 | 2457072.579 | 18.093 0.063 | *V* | 1m0-08 |
| 2014-12-30 | 2457021.685 | 17.503 0.037 | *g* | 1m0-08 | 2015-02-20 | 2457073.605 | 18.111 0.046 | *V* | 1m0-08 |
| 2014-12-30 | 2457021.688 | 17.475 0.031 | *g* | 1m0-08 | 2015-02-20 | 2457073.607 | 18.169 0.051 | *V* | 1m0-08 |
| 2015-01-16 | 2457038.692 | 18.173 0.040 | *g* | 1m0-08 | 2014-11-27 | 2456988.781 | 16.145 0.015 | *r* | 1m0-08 |
| 2015-01-16 | 2457038.695 | 18.032 0.038 | *g* | 1m0-08 | 2014-11-27 | 2456988.782 | 16.147 0.016 | *r* | 1m0-08 |
| 2015-01-24 | 2457046.658 | 18.355 0.072 | *g* | 1m0-08 | 2014-11-27 | 2456988.846 | 16.136 0.015 | *r* | 1m0-08 |
| 2015-01-24 | 2457046.662 | 18.336 0.057 | *g* | 1m0-08 | 2014-11-27 | 2456988.848 | 16.147 0.015 | *r* | 1m0-08 |

(a) Data have not been corrected for extinction
(b) *Swift* Telescope; LSQ (La Silla Quest, Chile); 1m0-08 (McDonald Observatory, USA); 1m0-10, 1m0-12, 1m0-13 (Sutherland, South Africa), 1m0-04, 1m0-05, 1m0-09 (Cerro Tololo, Chile); 1m0-03, 1m0-11 (Siding Spring, Australia).

**Table D1:** ASASSN-14kg: Photometric Data

| Date | JD | mag$^{(a)}$ | Filter | telescope$^{(b)}$ | Date | JD | mag$^{(a)}$ | Filter | telescope$^{(b)}$ |
|---|---|---|---|---|---|---|---|---|---|
| 2014-11-28 | 2456989.714 | 16.126 0.016 | $r$ | 1m0-08 | 2014-11-27 | 2456988.784 | 16.300 0.018 | $i$ | 1m0-08 |
| 2014-11-28 | 2456989.716 | 16.138 0.015 | $r$ | 1m0-08 | 2014-11-27 | 2456988.786 | 16.293 0.018 | $i$ | 1m0-08 |
| 2014-11-30 | 2456991.592 | 16.118 0.016 | $r$ | 1m0-08 | 2014-11-27 | 2456988.849 | 16.311 0.018 | $i$ | 1m0-08 |
| 2014-11-30 | 2456991.594 | 16.121 0.016 | $r$ | 1m0-08 | 2014-11-27 | 2456988.851 | 16.279 0.018 | $i$ | 1m0-08 |
| 2014-12-01 | 2456992.656 | 16.144 0.016 | $r$ | 1m0-08 | 2014-11-28 | 2456989.718 | 16.271 0.018 | $i$ | 1m0-08 |
| 2014-12-01 | 2456992.657 | 16.098 0.015 | $r$ | 1m0-08 | 2014-11-28 | 2456989.719 | 16.287 0.018 | $i$ | 1m0-08 |
| 2014-12-02 | 2456993.796 | 16.054 0.018 | $r$ | 1m0-08 | 2014-11-30 | 2456991.595 | 16.239 0.018 | $i$ | 1m0-08 |
| 2014-12-02 | 2456993.798 | 16.072 0.020 | $r$ | 1m0-08 | 2014-11-30 | 2456991.597 | 16.266 0.019 | $i$ | 1m0-08 |
| 2014-12-12 | 2457003.785 | 16.095 0.018 | $r$ | 1m0-08 | 2014-12-01 | 2456992.659 | 16.245 0.020 | $i$ | 1m0-08 |
| 2014-12-12 | 2457003.786 | 16.113 0.016 | $r$ | 1m0-08 | 2014-12-01 | 2456992.661 | 16.146 0.021 | $i$ | 1m0-08 |
| 2014-12-16 | 2457007.741 | 16.202 0.016 | $r$ | 1m0-08 | 2014-12-02 | 2456993.800 | 16.209 0.029 | $i$ | 1m0-08 |
| 2014-12-16 | 2457007.743 | 16.204 0.016 | $r$ | 1m0-08 | 2014-12-02 | 2456993.801 | 16.232 0.022 | $i$ | 1m0-08 |
| 2014-12-20 | 2457011.747 | 16.287 0.016 | $r$ | 1m0-08 | 2014-12-12 | 2457003.788 | 16.235 0.023 | $i$ | 1m0-08 |
| 2014-12-20 | 2457011.749 | 16.284 0.017 | $r$ | 1m0-08 | 2014-12-12 | 2457003.790 | 16.226 0.016 | $i$ | 1m0-08 |
| 2014-12-25 | 2457016.724 | 16.657 0.056 | $r$ | 1m0-08 | 2014-12-16 | 2457007.745 | 16.222 0.017 | $i$ | 1m0-08 |
| 2014-12-29 | 2457020.656 | 16.393 0.020 | $r$ | 1m0-08 | 2014-12-16 | 2457007.746 | 16.272 0.046 | $i$ | 1m0-08 |
| 2014-12-29 | 2457020.657 | 16.402 0.018 | $r$ | 1m0-08 | 2014-12-20 | 2457011.751 | 16.335 0.020 | $i$ | 1m0-08 |
| 2014-12-30 | 2457021.690 | 16.388 0.031 | $r$ | 1m0-08 | 2014-12-20 | 2457011.752 | 16.311 0.028 | $i$ | 1m0-08 |
| 2014-12-30 | 2457021.692 | 16.490 0.019 | $r$ | 1m0-08 | 2014-12-25 | 2457016.727 | 16.553 0.052 | $i$ | 1m0-08 |
| 2015-01-16 | 2457038.697 | 16.783 0.018 | $r$ | 1m0-08 | 2014-12-29 | 2457020.659 | 16.558 0.029 | $i$ | 1m0-08 |
| 2015-01-16 | 2457038.699 | 16.769 0.020 | $r$ | 1m0-08 | 2014-12-29 | 2457020.661 | 16.468 0.027 | $i$ | 1m0-08 |
| 2015-01-24 | 2457046.666 | 16.677 0.029 | $r$ | 1m0-08 | 2014-12-30 | 2457021.694 | 16.461 0.034 | $i$ | 1m0-08 |
| 2015-01-24 | 2457046.668 | 16.787 0.035 | $r$ | 1m0-08 | 2014-12-30 | 2457021.695 | 16.498 0.033 | $i$ | 1m0-08 |
| 2015-01-28 | 2457050.658 | 16.988 0.019 | $r$ | 1m0-08 | 2015-01-16 | 2457038.701 | 16.776 0.029 | $i$ | 1m0-08 |
| 2015-01-28 | 2457050.661 | 16.993 0.021 | $r$ | 1m0-08 | 2015-01-16 | 2457038.702 | 16.799 0.028 | $i$ | 1m0-08 |
| 2015-01-29 | 2457051.662 | 17.015 0.021 | $r$ | 1m0-08 | 2015-01-24 | 2457046.671 | 16.685 0.044 | $i$ | 1m0-08 |
| 2015-02-05 | 2457058.620 | 17.129 0.026 | $r$ | 1m0-08 | 2015-01-24 | 2457046.673 | 16.611 0.042 | $i$ | 1m0-08 |
| 2015-02-05 | 2457058.623 | 17.118 0.025 | $r$ | 1m0-08 | 2015-01-28 | 2457050.663 | 16.963 0.022 | $i$ | 1m0-08 |
| 2015-02-09 | 2457062.629 | 17.172 0.022 | $r$ | 1m0-08 | 2015-02-05 | 2457058.625 | 17.095 0.030 | $i$ | 1m0-08 |
| 2015-02-09 | 2457062.631 | 17.194 0.023 | $r$ | 1m0-08 | 2015-02-05 | 2457058.628 | 17.298 0.094 | $i$ | 1m0-08 |
| 2015-02-11 | 2457064.650 | 17.225 0.023 | $r$ | 1m0-08 | 2015-02-09 | 2457062.634 | 17.212 0.022 | $i$ | 1m0-08 |
| 2015-02-11 | 2457064.652 | 17.221 0.020 | $r$ | 1m0-08 | 2015-02-09 | 2457062.637 | 17.186 0.029 | $i$ | 1m0-08 |
| 2015-02-19 | 2457072.616 | 17.414 0.027 | $r$ | 1m0-08 | 2015-02-11 | 2457064.655 | 17.213 0.027 | $i$ | 1m0-08 |
| 2015-02-19 | 2457072.619 | 17.419 0.062 | $r$ | 1m0-08 | 2015-02-11 | 2457064.658 | 17.243 0.029 | $i$ | 1m0-08 |
| 2015-02-20 | 2457073.622 | 17.428 0.025 | $r$ | 1m0-08 | 2015-02-20 | 2457073.627 | 17.438 0.033 | $i$ | 1m0-08 |
| 2015-02-20 | 2457073.625 | 17.424 0.025 | $r$ | 1m0-08 | 2015-02-20 | 2457073.630 | 17.407 0.030 | $i$ | 1m0-08 |
| 2015-02-22 | 2457075.578 | 17.422 0.032 | $r$ | 1m0-08 | 2015-02-22 | 2457075.583 | 17.443 0.029 | $i$ | 1m0-08 |
| 2015-02-22 | 2457075.580 | 17.425 0.027 | $r$ | 1m0-08 | 2015-02-22 | 2457075.586 | 17.498 0.035 | $i$ | 1m0-08 |
| 2015-03-07 | 2457088.587 | 17.909 0.050 | $r$ | 1m0-08 | 2015-03-07 | 2457088.592 | 17.951 0.069 | $i$ | 1m0-08 |
| 2015-03-07 | 2457088.589 | 17.877 0.049 | $r$ | 1m0-08 | 2015-03-07 | 2457088.594 | 17.834 0.068 | $i$ | 1m0-08 |

(a) Data have not been corrected for extinction
(b) *Swift* Telescope; LSQ (La Silla Quest, Chile); 1m0-08 (McDonald Observatory, USA); 1m0-10, 1m0-12, 1m0-13 (Sutherland, South Africa), 1m0-04, 1m0-05, 1m0-09 (Cerro Tololo, Chile); 1m0-03, 1m0-11 (Siding Spring, Australia).

**Table D1:** SN2013ai: Photometric Data

| Date | JD | mag$^{(a)}$ | Filter | telescope$^{(b)}$ | Date | JD | mag$^{(a)}$ | Filter | telescope$^{(b)}$ |
|---|---|---|---|---|---|---|---|---|---|
| 2013-03-05 | 2456356.563 | 18.061 0.020 | *B* | 1m0-04 | 2013-05-09 | 2456422.470 | 20.536 0.184 | *B* | 1m0-05 |
| 2013-03-05 | 2456356.564 | 18.093 0.017 | *B* | 1m0-04 | 2013-03-05 | 2456356.567 | 17.701 0.012 | *g* | 1m0-04 |
| 2013-03-06 | 2456357.563 | 18.067 0.019 | *B* | 1m0-04 | 2013-03-05 | 2456356.568 | 17.723 0.010 | *g* | 1m0-04 |
| 2013-03-06 | 2456357.564 | 18.002 0.017 | *B* | 1m0-04 | 2013-03-06 | 2456357.567 | 17.624 0.013 | *g* | 1m0-04 |
| 2013-03-14 | 2456365.604 | 18.104 0.020 | *B* | 1m0-09 | 2013-03-06 | 2456357.568 | 17.669 0.017 | *g* | 1m0-04 |
| 2013-03-14 | 2456365.605 | 18.160 0.018 | *B* | 1m0-09 | 2013-03-14 | 2456365.609 | 17.567 0.014 | *g* | 1m0-09 |
| 2013-03-15 | 2456366.604 | 17.962 0.028 | *B* | 1m0-09 | 2013-03-14 | 2456365.610 | 17.558 0.015 | *g* | 1m0-09 |
| 2013-03-15 | 2456366.606 | 18.183 0.053 | *B* | 1m0-09 | 2013-03-15 | 2456366.609 | 17.711 0.017 | *g* | 1m0-09 |
| 2013-03-16 | 2456367.604 | 18.125 0.022 | *B* | 1m0-09 | 2013-03-15 | 2456366.610 | 17.572 0.013 | *g* | 1m0-09 |
| 2013-03-16 | 2456367.606 | 18.086 0.018 | *B* | 1m0-09 | 2013-03-16 | 2456367.609 | 17.591 0.013 | *g* | 1m0-09 |
| 2013-03-17 | 2456368.605 | 18.176 0.022 | *B* | 1m0-09 | 2013-03-16 | 2456367.610 | 17.636 0.016 | *g* | 1m0-09 |
| 2013-03-17 | 2456368.606 | 18.148 0.022 | *B* | 1m0-09 | 2013-03-17 | 2456368.609 | 17.671 0.010 | *g* | 1m0-09 |
| 2013-03-18 | 2456369.605 | 18.159 0.019 | *B* | 1m0-09 | 2013-03-17 | 2456368.610 | 17.651 0.009 | *g* | 1m0-09 |
| 2013-03-18 | 2456369.606 | 18.249 0.020 | *B* | 1m0-09 | 2013-03-18 | 2456369.609 | 17.639 0.012 | *g* | 1m0-09 |
| 2013-03-19 | 2456370.605 | 18.287 0.021 | *B* | 1m0-09 | 2013-03-18 | 2456369.611 | 17.621 0.014 | *g* | 1m0-09 |
| 2013-03-19 | 2456370.606 | 18.305 0.033 | *B* | 1m0-09 | 2013-03-19 | 2456370.609 | 17.664 0.014 | *g* | 1m0-09 |
| 2013-03-24 | 2456375.573 | 18.611 0.029 | *B* | 1m0-09 | 2013-03-19 | 2456370.611 | 17.678 0.014 | *g* | 1m0-09 |
| 2013-03-24 | 2456375.575 | 18.551 0.031 | *B* | 1m0-09 | 2013-03-24 | 2456375.579 | 17.875 0.016 | *g* | 1m0-09 |
| 2013-03-27 | 2456378.575 | 18.635 0.033 | *B* | 1m0-09 | 2013-03-24 | 2456375.581 | 17.784 0.017 | *g* | 1m0-09 |
| 2013-03-28 | 2456379.575 | 18.790 0.107 | *B* | 1m0-09 | 2013-03-26 | 2456377.581 | 17.956 0.031 | *g* | 1m0-09 |
| 2013-03-28 | 2456380.261 | 18.939 0.031 | *B* | 1m0-12 | 2013-03-27 | 2456378.581 | 17.952 0.030 | *g* | 1m0-09 |
| 2013-03-28 | 2456380.262 | 19.034 0.050 | *B* | 1m0-12 | 2013-03-28 | 2456380.266 | 18.019 0.015 | *g* | 1m0-12 |
| 2013-03-29 | 2456380.566 | 18.851 0.046 | *B* | 1m0-09 | 2013-03-28 | 2456380.268 | 18.014 0.015 | *g* | 1m0-12 |
| 2013-03-29 | 2456380.568 | 18.784 0.029 | *B* | 1m0-09 | 2013-03-29 | 2456380.572 | 17.995 0.019 | *g* | 1m0-09 |
| 2013-04-03 | 2456385.500 | 19.220 0.041 | *B* | 1m0-09 | 2013-03-29 | 2456380.574 | 17.994 0.015 | *g* | 1m0-09 |
| 2013-04-03 | 2456385.502 | 19.066 0.047 | *B* | 1m0-09 | 2013-04-03 | 2456385.507 | 18.224 0.017 | *g* | 1m0-09 |
| 2013-04-04 | 2456387.230 | 19.213 0.046 | *B* | 1m0-13 | 2013-04-03 | 2456385.508 | 18.162 0.015 | *g* | 1m0-09 |
| 2013-04-04 | 2456387.231 | 18.955 0.033 | *B* | 1m0-13 | 2013-04-04 | 2456387.236 | 18.291 0.024 | *g* | 1m0-13 |
| 2013-04-05 | 2456387.500 | 19.251 0.045 | *B* | 1m0-09 | 2013-04-04 | 2456387.237 | 18.272 0.020 | *g* | 1m0-13 |
| 2013-04-05 | 2456388.229 | 19.144 0.049 | *B* | 1m0-13 | 2013-04-05 | 2456387.507 | 18.262 0.018 | *g* | 1m0-09 |
| 2013-04-05 | 2456388.231 | 19.304 0.041 | *B* | 1m0-13 | 2013-04-05 | 2456387.509 | 18.257 0.017 | *g* | 1m0-09 |
| 2013-04-06 | 2456388.500 | 19.186 0.057 | *B* | 1m0-09 | 2013-04-05 | 2456388.236 | 18.255 0.016 | *g* | 1m0-13 |
| 2013-04-06 | 2456388.502 | 19.288 0.048 | *B* | 1m0-09 | 2013-04-05 | 2456388.237 | 18.345 0.020 | *g* | 1m0-13 |
| 2013-04-06 | 2456389.230 | 19.299 0.049 | *B* | 1m0-13 | 2013-04-06 | 2456388.507 | 18.340 0.017 | *g* | 1m0-09 |
| 2013-04-06 | 2456389.232 | 19.403 0.042 | *B* | 1m0-13 | 2013-04-06 | 2456388.509 | 18.312 0.021 | *g* | 1m0-09 |
| 2013-04-11 | 2456393.500 | 19.531 0.073 | *B* | 1m0-09 | 2013-04-06 | 2456389.236 | 18.336 0.018 | *g* | 1m0-13 |
| 2013-04-11 | 2456393.502 | 19.433 0.075 | *B* | 1m0-09 | 2013-04-06 | 2456389.238 | 18.382 0.018 | *g* | 1m0-13 |
| 2013-04-11 | 2456394.210 | 19.274 0.103 | *B* | 1m0-13 | 2013-04-11 | 2456393.506 | 18.469 0.021 | *g* | 1m0-09 |
| 2013-04-11 | 2456394.211 | 19.179 0.086 | *B* | 1m0-13 | 2013-04-11 | 2456393.508 | 18.437 0.025 | *g* | 1m0-09 |
| 2013-04-12 | 2456394.504 | 19.458 0.080 | *B* | 1m0-09 | 2013-04-11 | 2456394.217 | 18.532 0.029 | *g* | 1m0-13 |
| 2013-04-13 | 2456395.500 | 19.705 0.083 | *B* | 1m0-09 | 2013-04-12 | 2456394.510 | 18.543 0.027 | *g* | 1m0-09 |
| 2013-04-13 | 2456396.209 | 19.574 0.136 | *B* | 1m0-13 | 2013-04-12 | 2456394.512 | 18.472 0.028 | *g* | 1m0-09 |
| 2013-04-15 | 2456397.500 | 19.602 0.055 | *B* | 1m0-09 | 2013-04-13 | 2456395.506 | 18.406 0.030 | *g* | 1m0-09 |
| 2013-04-15 | 2456397.502 | 19.564 0.079 | *B* | 1m0-09 | 2013-04-13 | 2456395.508 | 18.483 0.024 | *g* | 1m0-09 |
| 2013-04-15 | 2456398.209 | 19.534 0.077 | *B* | 1m0-13 | 2013-04-15 | 2456397.507 | 18.520 0.022 | *g* | 1m0-09 |
| 2013-04-15 | 2456398.211 | 19.474 0.090 | *B* | 1m0-13 | 2013-04-15 | 2456397.508 | 18.564 0.024 | *g* | 1m0-09 |
| 2013-04-18 | 2456400.500 | 19.772 0.080 | *B* | 1m0-09 | 2013-04-15 | 2456398.218 | 18.465 0.037 | *g* | 1m0-13 |
| 2013-04-18 | 2456400.505 | 19.808 0.063 | *B* | 1m0-09 | 2013-04-18 | 2456400.515 | 18.634 0.043 | *g* | 1m0-09 |
| 2013-04-20 | 2456402.500 | 19.808 0.092 | *B* | 1m0-09 | 2013-04-18 | 2456400.519 | 18.610 0.027 | *g* | 1m0-09 |
| 2013-04-20 | 2456402.505 | 19.810 0.072 | *B* | 1m0-09 | 2013-04-20 | 2456402.514 | 18.784 0.032 | *g* | 1m0-09 |
| 2013-04-22 | 2456404.500 | 20.083 0.072 | *B* | 1m0-09 | 2013-04-20 | 2456402.519 | 18.715 0.022 | *g* | 1m0-09 |
| 2013-04-22 | 2456404.505 | 19.722 0.083 | *B* | 1m0-09 | 2013-04-22 | 2456404.515 | 18.766 0.033 | *g* | 1m0-09 |
| 2013-04-23 | 2456405.505 | 19.711 0.088 | *B* | 1m0-09 | 2013-04-22 | 2456404.520 | 18.817 0.032 | *g* | 1m0-09 |
| 2013-04-24 | 2456407.476 | 19.762 0.096 | *B* | 1m0-05 | 2013-04-23 | 2456405.514 | 18.739 0.025 | *g* | 1m0-09 |
| 2013-04-28 | 2456411.473 | 19.985 0.142 | *B* | 1m0-09 | 2013-04-23 | 2456405.519 | 18.681 0.032 | *g* | 1m0-09 |
| 2013-04-29 | 2456412.476 | 20.118 0.110 | *B* | 1m0-09 | 2013-04-24 | 2456407.483 | 18.956 0.048 | *g* | 1m0-05 |
| 2013-05-03 | 2456416.461 | 20.432 0.230 | *B* | 1m0-05 | 2013-04-24 | 2456407.486 | 18.919 0.031 | *g* | 1m0-05 |
| 2013-05-03 | 2456416.465 | 20.233 0.167 | *B* | 1m0-05 | 2013-04-26 | 2456409.482 | 18.965 0.030 | *g* | 1m0-09 |
| 2013-05-07 | 2456420.444 | 20.947 0.192 | *B* | 1m0-09 | 2013-04-28 | 2456411.483 | 18.981 0.036 | *g* | 1m0-09 |
| 2013-05-09 | 2456422.467 | 20.755 0.235 | *B* | 1m0-05 | 2013-04-28 | 2456411.486 | 18.970 0.041 | *g* | 1m0-09 |

(a) Data have not been corrected for extinction
(b) *Swift* Telescope; LSQ (La Silla Quest, Chile); 1m0-08 (McDonald Observatory, USA); 1m0-10, 1m0-12, 1m0-13 (Sutherland, South Africa), 1m0-04, 1m0-05, 1m0-09 (Cerro Tololo, Chile); 1m0-03, 1m0-11 (Siding Spring, Australia).

**Table D1:** SN2013ai: Photometric Data

| Date | JD | mag[(a)] | Filter | telescope[(b)] | Date | JD | mag[(a)] | Filter | telescope[(b)] |
|---|---|---|---|---|---|---|---|---|---|
| 2013-04-29 | 2456412.484 | 18.999 0.028 | *g* | 1m0-09 | 2013-04-20 | 2456402.509 | 17.958 0.014 | *V* | 1m0-09 |
| 2013-04-29 | 2456412.487 | 18.988 0.032 | *g* | 1m0-09 | 2013-04-20 | 2456402.512 | 17.930 0.014 | *V* | 1m0-09 |
| 2013-05-03 | 2456416.474 | 19.149 0.039 | *g* | 1m0-05 | 2013-04-22 | 2456404.510 | 18.035 0.015 | *V* | 1m0-09 |
| 2013-05-03 | 2456416.479 | 19.165 0.038 | *g* | 1m0-05 | 2013-04-22 | 2456404.512 | 18.022 0.015 | *V* | 1m0-09 |
| 2013-05-08 | 2456421.453 | 19.406 0.100 | *g* | 1m0-09 | 2013-04-23 | 2456405.509 | 18.044 0.021 | *V* | 1m0-09 |
| 2013-05-09 | 2456422.477 | 19.320 0.043 | *g* | 1m0-05 | 2013-04-23 | 2456405.512 | 18.091 0.026 | *V* | 1m0-09 |
| 2013-05-09 | 2456422.480 | 19.467 0.070 | *g* | 1m0-05 | 2013-04-24 | 2456407.479 | 18.000 0.015 | *V* | 1m0-05 |
| 2013-05-10 | 2456423.451 | 19.287 0.051 | *g* | 1m0-09 | 2013-04-24 | 2456407.481 | 18.058 0.018 | *V* | 1m0-05 |
| 2013-05-10 | 2456423.454 | 19.220 0.057 | *g* | 1m0-09 | 2013-04-27 | 2456410.479 | 18.133 0.077 | *V* | 1m0-09 |
| 2013-05-14 | 2456427.449 | 19.128 0.065 | *g* | 1m0-09 | 2013-04-28 | 2456411.479 | 18.143 0.064 | *V* | 1m0-09 |
| 2013-05-14 | 2456427.452 | 19.335 0.080 | *g* | 1m0-09 | 2013-04-28 | 2456411.481 | 18.155 0.020 | *V* | 1m0-09 |
| 2013-03-05 | 2456356.565 | 17.375 0.009 | *V* | 1m0-04 | 2013-04-29 | 2456412.479 | 18.141 0.018 | *V* | 1m0-09 |
| 2013-03-05 | 2456356.566 | 17.352 0.011 | *V* | 1m0-04 | 2013-04-29 | 2456412.482 | 18.150 0.019 | *V* | 1m0-09 |
| 2013-03-06 | 2456357.565 | 17.395 0.008 | *V* | 1m0-04 | 2013-05-03 | 2456416.472 | 18.279 0.021 | *V* | 1m0-05 |
| 2013-03-06 | 2456357.566 | 17.357 0.011 | *V* | 1m0-04 | 2013-05-07 | 2456420.447 | 18.534 0.040 | *V* | 1m0-09 |
| 2013-03-14 | 2456365.607 | 17.239 0.009 | *V* | 1m0-09 | 2013-05-07 | 2456420.449 | 18.436 0.041 | *V* | 1m0-09 |
| 2013-03-14 | 2456365.608 | 17.214 0.008 | *V* | 1m0-09 | 2013-05-09 | 2456422.473 | 18.346 0.019 | *V* | 1m0-05 |
| 2013-03-15 | 2456366.607 | 17.110 0.018 | *V* | 1m0-09 | 2013-05-09 | 2456422.475 | 18.332 0.020 | *V* | 1m0-05 |
| 2013-03-15 | 2456366.608 | 17.095 0.015 | *V* | 1m0-09 | 2013-05-10 | 2456423.449 | 18.521 0.200 | *V* | 1m0-09 |
| 2013-03-16 | 2456367.607 | 17.247 0.010 | *V* | 1m0-09 | 2013-05-20 | 2456433.195 | 18.546 0.200 | *V* | 1m0-10 |
| 2013-03-16 | 2456367.608 | 17.226 0.012 | *V* | 1m0-09 | 2013-05-20 | 2456433.197 | 18.404 0.200 | *V* | 1m0-10 |
| 2013-03-17 | 2456368.607 | 17.244 0.010 | *V* | 1m0-09 | 2013-05-20 | 2456433.451 | 18.545 0.200 | *V* | 1m0-05 |
| 2013-03-17 | 2456368.608 | 17.208 0.009 | *V* | 1m0-09 | 2013-05-22 | 2456435.453 | 18.541 0.200 | *V* | 1m0-05 |
| 2013-03-18 | 2456369.607 | 17.274 0.010 | *V* | 1m0-09 | 2013-05-27 | 2456440.195 | 18.561 0.200 | *V* | 1m0-10 |
| 2013-03-18 | 2456369.608 | 17.259 0.009 | *V* | 1m0-09 | 2013-02-06 | 2456330.000 | < 19.000 | *r* | Atel/CBAT |
| 2013-03-19 | 2456370.607 | 17.256 0.013 | *V* | 1m0-09 | 2013-02-26 | 2456350.000 | 18.300 0.000 | *r* | Atel/CBAT |
| 2013-03-19 | 2456370.608 | 17.273 0.010 | *V* | 1m0-09 | 2013-03-01 | 2456352.567 | 17.600 0.000 | *r* | Atel/CBAT |
| 2013-03-24 | 2456375.577 | 17.349 0.009 | *V* | 1m0-09 | 2013-03-05 | 2456356.569 | 17.156 0.019 | *r* | 1m0-04 |
| 2013-03-24 | 2456375.578 | 17.385 0.010 | *V* | 1m0-09 | 2013-03-05 | 2456356.570 | 17.186 0.018 | *r* | 1m0-04 |
| 2013-03-27 | 2456378.577 | 17.413 0.009 | *V* | 1m0-09 | 2013-03-06 | 2456357.569 | 17.089 0.016 | *r* | 1m0-04 |
| 2013-03-27 | 2456378.578 | 17.386 0.066 | *V* | 1m0-09 | 2013-03-06 | 2456357.570 | 17.106 0.020 | *r* | 1m0-04 |
| 2013-03-28 | 2456380.264 | 17.440 0.015 | *V* | 1m0-12 | 2013-03-14 | 2456365.611 | 16.862 0.010 | *r* | 1m0-09 |
| 2013-03-28 | 2456380.265 | 17.491 0.014 | *V* | 1m0-12 | 2013-03-14 | 2456365.612 | 16.905 0.012 | *r* | 1m0-09 |
| 2013-03-29 | 2456380.570 | 17.474 0.011 | *V* | 1m0-09 | 2013-03-15 | 2456366.611 | 16.816 0.016 | *r* | 1m0-09 |
| 2013-03-29 | 2456380.571 | 17.460 0.009 | *V* | 1m0-09 | 2013-03-15 | 2456366.612 | 16.871 0.021 | *r* | 1m0-09 |
| 2013-04-03 | 2456385.504 | 17.617 0.012 | *V* | 1m0-09 | 2013-03-16 | 2456367.611 | 16.855 0.039 | *r* | 1m0-09 |
| 2013-04-03 | 2456385.505 | 17.586 0.013 | *V* | 1m0-09 | 2013-03-16 | 2456367.612 | 16.857 0.036 | *r* | 1m0-09 |
| 2013-04-04 | 2456387.233 | 17.604 0.012 | *V* | 1m0-13 | 2013-03-17 | 2456368.612 | 16.875 0.013 | *r* | 1m0-09 |
| 2013-04-05 | 2456387.505 | 17.691 0.071 | *V* | 1m0-09 | 2013-03-17 | 2456368.613 | 16.854 0.013 | *r* | 1m0-09 |
| 2013-04-05 | 2456387.506 | 17.620 0.012 | *V* | 1m0-09 | 2013-03-18 | 2456369.612 | 16.898 0.011 | *r* | 1m0-09 |
| 2013-04-05 | 2456388.233 | 17.677 0.011 | *V* | 1m0-13 | 2013-03-18 | 2456369.613 | 16.895 0.010 | *r* | 1m0-09 |
| 2013-04-05 | 2456388.234 | 17.644 0.014 | *V* | 1m0-13 | 2013-03-19 | 2456370.613 | 16.881 0.015 | *r* | 1m0-09 |
| 2013-04-06 | 2456388.504 | 17.779 0.019 | *V* | 1m0-09 | 2013-03-24 | 2456375.582 | 16.916 0.012 | *r* | 1m0-09 |
| 2013-04-06 | 2456388.505 | 17.681 0.015 | *V* | 1m0-09 | 2013-03-28 | 2456380.270 | 16.930 0.017 | *r* | 1m0-12 |
| 2013-04-06 | 2456389.234 | 17.654 0.013 | *V* | 1m0-13 | 2013-03-29 | 2456380.575 | 16.953 0.012 | *r* | 1m0-09 |
| 2013-04-06 | 2456389.235 | 17.605 0.014 | *V* | 1m0-13 | 2013-03-29 | 2456380.576 | 16.936 0.024 | *r* | 1m0-09 |
| 2013-04-11 | 2456393.505 | 17.721 0.016 | *V* | 1m0-09 | 2013-04-03 | 2456385.510 | 17.018 0.013 | *r* | 1m0-09 |
| 2013-04-11 | 2456394.213 | 17.675 0.021 | *V* | 1m0-13 | 2013-04-03 | 2456385.511 | 17.023 0.011 | *r* | 1m0-09 |
| 2013-04-11 | 2456394.214 | 17.770 0.020 | *V* | 1m0-13 | 2013-04-04 | 2456387.239 | 17.105 0.014 | *r* | 1m0-13 |
| 2013-04-12 | 2456394.507 | 17.821 0.022 | *V* | 1m0-09 | 2013-04-04 | 2456387.240 | 17.084 0.014 | *r* | 1m0-13 |
| 2013-04-12 | 2456394.509 | 17.783 0.018 | *V* | 1m0-09 | 2013-04-05 | 2456387.511 | 17.093 0.015 | *r* | 1m0-09 |
| 2013-04-13 | 2456395.504 | 17.747 0.014 | *V* | 1m0-09 | 2013-04-05 | 2456388.239 | 17.096 0.017 | *r* | 1m0-13 |
| 2013-04-13 | 2456395.505 | 17.710 0.018 | *V* | 1m0-09 | 2013-04-05 | 2456388.240 | 17.081 0.013 | *r* | 1m0-13 |
| 2013-04-13 | 2456396.213 | 17.744 0.021 | *V* | 1m0-13 | 2013-04-06 | 2456388.511 | 17.087 0.020 | *r* | 1m0-09 |
| 2013-04-13 | 2456396.214 | 17.830 0.022 | *V* | 1m0-13 | 2013-04-06 | 2456388.512 | 17.106 0.013 | *r* | 1m0-09 |
| 2013-04-15 | 2456397.504 | 17.850 0.018 | *V* | 1m0-09 | 2013-04-06 | 2456389.240 | 17.149 0.015 | *r* | 1m0-13 |
| 2013-04-15 | 2456397.505 | 17.839 0.009 | *V* | 1m0-09 | 2013-04-06 | 2456389.241 | 17.146 0.015 | *r* | 1m0-13 |
| 2013-04-15 | 2456398.213 | 17.881 0.043 | *V* | 1m0-13 | 2013-04-11 | 2456393.509 | 17.192 0.025 | *r* | 1m0-09 |
| 2013-04-18 | 2456400.510 | 17.912 0.018 | *V* | 1m0-09 | 2013-04-11 | 2456393.511 | 17.140 0.024 | *r* | 1m0-09 |
| 2013-04-18 | 2456400.512 | 17.901 0.013 | *V* | 1m0-09 | 2013-04-11 | 2456394.219 | 17.225 0.027 | *r* | 1m0-13 |

(a) Data have not been corrected for extinction
(b) *Swift* Telescope; LSQ (La Silla Quest, Chile); 1m0-08 (McDonald Observatory, USA); 1m0-10, 1m0-12, 1m0-13 (Sutherland, South Africa), 1m0-04, 1m0-05, 1m0-09 (Cerro Tololo, Chile); 1m0-03, 1m0-11 (Siding Spring, Australia).

**Table D1:** SN2013ai: Photometric Data

| Date | JD | mag[(a)] | Filter | telescope[(b)] | Date | JD | mag[(a)] | Filter | telescope[(b)] |
|---|---|---|---|---|---|---|---|---|---|
| 2013-04-12 | 2456394.514 | 17.169 0.034 | *r* | 1m0-09 | 2013-04-04 | 2456387.241 | 16.719 0.008 | *i* | 1m0-13 |
| 2013-04-12 | 2456394.515 | 17.132 0.037 | *r* | 1m0-09 | 2013-04-05 | 2456388.242 | 16.726 0.010 | *i* | 1m0-13 |
| 2013-04-13 | 2456395.511 | 17.193 0.033 | *r* | 1m0-09 | 2013-04-11 | 2456393.513 | 16.800 0.012 | *i* | 1m0-09 |
| 2013-04-15 | 2456397.510 | 17.206 0.014 | *r* | 1m0-09 | 2013-04-11 | 2456394.221 | 16.785 0.014 | *i* | 1m0-13 |
| 2013-04-15 | 2456397.512 | 17.222 0.016 | *r* | 1m0-09 | 2013-04-11 | 2456394.222 | 16.781 0.013 | *i* | 1m0-13 |
| 2013-04-15 | 2456398.222 | 17.196 0.029 | *r* | 1m0-13 | 2013-04-12 | 2456394.516 | 16.798 0.012 | *i* | 1m0-09 |
| 2013-04-18 | 2456400.524 | 17.262 0.012 | *r* | 1m0-09 | 2013-04-13 | 2456395.512 | 16.823 0.013 | *i* | 1m0-09 |
| 2013-04-18 | 2456400.527 | 17.275 0.014 | *r* | 1m0-09 | 2013-04-13 | 2456395.513 | 16.793 0.011 | *i* | 1m0-09 |
| 2013-04-20 | 2456402.523 | 17.306 0.015 | *r* | 1m0-09 | 2013-04-15 | 2456397.513 | 16.723 0.014 | *i* | 1m0-09 |
| 2013-04-20 | 2456402.526 | 17.286 0.013 | *r* | 1m0-09 | 2013-04-15 | 2456397.514 | 16.819 0.012 | *i* | 1m0-09 |
| 2013-04-22 | 2456404.524 | 17.337 0.017 | *r* | 1m0-09 | 2013-04-15 | 2456398.223 | 16.765 0.015 | *i* | 1m0-13 |
| 2013-04-22 | 2456404.527 | 17.349 0.029 | *r* | 1m0-09 | 2013-04-15 | 2456398.225 | 16.847 0.009 | *i* | 1m0-13 |
| 2013-04-23 | 2456405.523 | 17.346 0.017 | *r* | 1m0-09 | 2013-04-18 | 2456400.529 | 16.826 0.011 | *i* | 1m0-09 |
| 2013-04-23 | 2456405.526 | 17.324 0.013 | *r* | 1m0-09 | 2013-04-18 | 2456400.532 | 16.900 0.012 | *i* | 1m0-09 |
| 2013-04-24 | 2456407.489 | 17.421 0.031 | *r* | 1m0-05 | 2013-04-20 | 2456402.528 | 16.901 0.014 | *i* | 1m0-09 |
| 2013-04-24 | 2456407.491 | 17.402 0.024 | *r* | 1m0-05 | 2013-04-20 | 2456402.531 | 16.925 0.010 | *i* | 1m0-09 |
| 2013-04-28 | 2456411.490 | 17.452 0.029 | *r* | 1m0-09 | 2013-04-22 | 2456404.530 | 16.910 0.014 | *i* | 1m0-09 |
| 2013-04-28 | 2456411.492 | 17.409 0.026 | *r* | 1m0-09 | 2013-04-22 | 2456404.532 | 16.936 0.012 | *i* | 1m0-09 |
| 2013-04-29 | 2456412.490 | 17.423 0.018 | *r* | 1m0-09 | 2013-04-23 | 2456405.528 | 16.915 0.012 | *i* | 1m0-09 |
| 2013-04-29 | 2456412.492 | 17.417 0.028 | *r* | 1m0-09 | 2013-04-23 | 2456405.531 | 17.025 0.018 | *i* | 1m0-09 |
| 2013-05-03 | 2456416.483 | 17.536 0.025 | *r* | 1m0-05 | 2013-04-24 | 2456407.493 | 16.997 0.016 | *i* | 1m0-05 |
| 2013-05-04 | 2456417.456 | 17.586 0.053 | *r* | 1m0-09 | 2013-04-24 | 2456407.494 | 17.026 0.012 | *i* | 1m0-05 |
| 2013-05-04 | 2456417.457 | 17.609 0.039 | *r* | 1m0-09 | 2013-04-27 | 2456410.493 | 16.964 0.021 | *i* | 1m0-09 |
| 2013-05-06 | 2456419.455 | 17.567 0.025 | *r* | 1m0-09 | 2013-04-27 | 2456410.495 | 16.990 0.020 | *i* | 1m0-09 |
| 2013-05-06 | 2456419.457 | 17.563 0.020 | *r* | 1m0-09 | 2013-04-28 | 2456411.494 | 17.029 0.013 | *i* | 1m0-09 |
| 2013-05-07 | 2456420.457 | 17.659 0.022 | *r* | 1m0-09 | 2013-04-28 | 2456411.496 | 17.045 0.019 | *i* | 1m0-09 |
| 2013-05-07 | 2456420.459 | 17.535 0.024 | *r* | 1m0-09 | 2013-04-29 | 2456412.494 | 17.049 0.013 | *i* | 1m0-09 |
| 2013-05-08 | 2456421.456 | 17.736 0.035 | *r* | 1m0-09 | 2013-04-29 | 2456412.497 | 17.066 0.016 | *i* | 1m0-09 |
| 2013-05-08 | 2456421.458 | 17.650 0.038 | *r* | 1m0-09 | 2013-05-03 | 2456416.488 | 17.131 0.014 | *i* | 1m0-05 |
| 2013-05-09 | 2456422.483 | 17.613 0.016 | *r* | 1m0-05 | 2013-05-03 | 2456416.490 | 17.134 0.012 | *i* | 1m0-05 |
| 2013-05-09 | 2456422.485 | 17.765 0.045 | *r* | 1m0-05 | 2013-05-04 | 2456417.459 | 17.092 0.014 | *i* | 1m0-09 |
| 2013-05-10 | 2456423.457 | 17.600 0.036 | *r* | 1m0-09 | 2013-05-04 | 2456417.461 | 17.115 0.021 | *i* | 1m0-09 |
| 2013-05-10 | 2456423.459 | 17.708 0.057 | *r* | 1m0-09 | 2013-05-06 | 2456419.458 | 17.174 0.021 | *i* | 1m0-09 |
| 2013-05-14 | 2456427.455 | 17.632 0.066 | *r* | 1m0-09 | 2013-05-06 | 2456419.460 | 17.167 0.013 | *i* | 1m0-09 |
| 2013-05-14 | 2456427.457 | 17.664 0.041 | *r* | 1m0-09 | 2013-05-07 | 2456420.461 | 17.192 0.014 | *i* | 1m0-09 |
| 2013-03-05 | 2456356.572 | 16.932 0.015 | *i* | 1m0-04 | 2013-05-07 | 2456420.462 | 17.189 0.018 | *i* | 1m0-09 |
| 2013-03-06 | 2456357.572 | 16.805 0.009 | *i* | 1m0-04 | 2013-05-08 | 2456421.459 | 17.213 0.024 | *i* | 1m0-09 |
| 2013-03-14 | 2456365.613 | 16.585 0.010 | *i* | 1m0-09 | 2013-05-08 | 2456421.461 | 17.283 0.018 | *i* | 1m0-09 |
| 2013-03-15 | 2456366.613 | 16.615 0.009 | *i* | 1m0-09 | 2013-05-09 | 2456422.487 | 17.244 0.017 | *i* | 1m0-05 |
| 2013-03-16 | 2456367.614 | 16.599 0.011 | *i* | 1m0-09 | 2013-05-09 | 2456422.488 | 17.271 0.023 | *i* | 1m0-05 |
| 2013-03-29 | 2456380.578 | 16.603 0.009 | *i* | 1m0-09 | 2013-05-10 | 2456423.461 | 17.242 0.017 | *i* | 1m0-09 |
| 2013-03-29 | 2456380.579 | 16.627 0.011 | *i* | 1m0-09 | 2013-05-10 | 2456423.463 | 17.170 0.015 | *i* | 1m0-09 |
| 2013-04-03 | 2456385.513 | 16.788 0.013 | *i* | 1m0-09 | 2013-05-14 | 2456427.459 | 17.294 0.015 | *i* | 1m0-09 |

(a) Data have not been corrected for extinction
(b) *Swift* Telescope; LSQ (La Silla Quest, Chile); 1m0-08 (McDonald Observatory, USA); 1m0-10, 1m0-12, 1m0-13 (Sutherland, South Africa), 1m0-04, 1m0-05, 1m0-09 (Cerro Tololo, Chile); 1m0-03, 1m0-11 (Siding Spring, Australia).

**Table D1:** SN 2014dw: Photometric Data

| Date | JD | mag[(a)] | Filter | telescope[(b)] | Date | JD | mag[(a)] | Filter | telescope[(b)] |
|---|---|---|---|---|---|---|---|---|---|
| 2014-11-10 | 2456972.225 | 16.480 0.025 | *B* | 1m0-11 | 2014-11-10 | 2456972.236 | 16.069 0.015 | *g* | 1m0-11 |
| 2014-11-10 | 2456972.227 | 16.497 0.026 | *B* | 1m0-11 | 2014-11-12 | 2456974.228 | 16.220 0.014 | *g* | 1m0-11 |
| 2014-11-12 | 2456974.219 | 16.658 0.020 | *B* | 1m0-11 | 2014-11-12 | 2456974.231 | 16.185 0.014 | *g* | 1m0-11 |
| 2014-11-12 | 2456974.222 | 16.600 0.020 | *B* | 1m0-11 | 2014-11-14 | 2456975.569 | 16.342 0.016 | *g* | 1m0-10 |
| 2014-11-14 | 2456975.569 | 16.711 0.022 | *B* | 1m0-12 | 2014-11-14 | 2456975.572 | 16.336 0.015 | *g* | 1m0-10 |
| 2014-11-14 | 2456975.569 | 16.759 0.016 | *B* | 1m0-13 | 2014-11-14 | 2456975.578 | 16.352 0.014 | *g* | 1m0-12 |
| 2014-11-14 | 2456975.572 | 16.721 0.024 | *B* | 1m0-12 | 2014-11-14 | 2456975.580 | 16.349 0.014 | *g* | 1m0-12 |
| 2014-11-14 | 2456975.572 | 16.770 0.018 | *B* | 1m0-13 | 2014-11-16 | 2456978.216 | 16.453 0.017 | *g* | 1m0-11 |
| 2014-11-16 | 2456978.219 | 16.922 0.022 | *B* | 1m0-03 | 2014-11-16 | 2456978.218 | 16.462 0.017 | *g* | 1m0-11 |
| 2014-11-16 | 2456978.221 | 16.797 0.021 | *B* | 1m0-03 | 2014-11-18 | 2456979.559 | 16.541 0.014 | *g* | 1m0-12 |
| 2014-11-18 | 2456979.559 | 16.932 0.020 | *B* | 1m0-10 | 2014-11-18 | 2456979.561 | 16.530 0.014 | *g* | 1m0-12 |
| 2014-11-18 | 2456979.562 | 16.973 0.021 | *B* | 1m0-10 | 2014-11-20 | 2456981.577 | 16.628 0.020 | *g* | 1m0-12 |
| 2014-11-20 | 2456981.553 | 17.118 0.019 | *B* | 1m0-12 | 2014-11-20 | 2456981.579 | 16.769 0.039 | *g* | 1m0-12 |
| 2014-11-20 | 2456981.555 | 17.162 0.026 | *B* | 1m0-12 | 2014-11-22 | 2456983.549 | 16.716 0.026 | *g* | 1m0-12 |
| 2014-11-22 | 2456983.549 | 17.181 0.025 | *B* | 1m0-10 | 2014-11-25 | 2456986.793 | 16.915 0.017 | *g* | 1m0-05 |
| 2014-11-22 | 2456983.552 | 17.184 0.023 | *B* | 1m0-10 | 2014-11-25 | 2456986.795 | 16.962 0.025 | *g* | 1m0-05 |
| 2014-11-24 | 2456985.818 | 17.423 0.016 | *B* | 1m0-05 | 2014-11-27 | 2456988.561 | 16.988 0.021 | *g* | 1m0-12 |
| 2014-11-24 | 2456985.821 | 17.412 0.017 | *B* | 1m0-05 | 2014-11-27 | 2456988.564 | 16.955 0.021 | *g* | 1m0-12 |
| 2014-11-24 | 2456985.843 | 17.429 0.018 | *B* | 1m0-05 | 2014-11-28 | 2456990.184 | 17.059 0.021 | *g* | 1m0-03 |
| 2014-11-24 | 2456985.846 | 17.408 0.016 | *B* | 1m0-05 | 2014-11-28 | 2456990.187 | 17.042 0.020 | *g* | 1m0-03 |
| 2014-11-25 | 2456986.827 | 17.549 0.018 | *B* | 1m0-05 | 2014-12-04 | 2456996.189 | 17.265 0.039 | *g* | 1m0-11 |
| 2014-11-25 | 2456986.829 | 17.533 0.018 | *B* | 1m0-05 | 2014-12-04 | 2456996.191 | 17.209 0.031 | *g* | 1m0-11 |
| 2014-11-27 | 2456988.555 | 17.529 0.030 | *B* | 1m0-12 | 2014-12-09 | 2457000.787 | 17.416 0.031 | *g* | 1m0-05 |
| 2014-11-28 | 2456990.175 | 17.619 0.045 | *B* | 1m0-03 | 2014-12-09 | 2457000.789 | 17.459 0.017 | *g* | 1m0-05 |
| 2014-11-28 | 2456990.178 | 17.609 0.039 | *B* | 1m0-03 | 2014-12-14 | 2457005.512 | 17.587 0.027 | *g* | 1m0-12 |
| 2014-12-04 | 2456996.180 | 17.932 0.098 | *B* | 1m0-11 | 2014-12-14 | 2457005.515 | 17.538 0.025 | *g* | 1m0-12 |
| 2014-12-04 | 2456996.183 | 17.959 0.103 | *B* | 1m0-11 | 2014-12-15 | 2457007.138 | 17.562 0.019 | *g* | 1m0-11 |
| 2014-12-09 | 2457000.778 | 18.247 0.026 | *B* | 1m0-05 | 2014-12-15 | 2457007.140 | 17.553 0.022 | *g* | 1m0-11 |
| 2014-12-09 | 2457000.781 | 18.250 0.022 | *B* | 1m0-05 | 2014-12-20 | 2457012.124 | 17.812 0.026 | *g* | 1m0-11 |
| 2014-12-14 | 2457005.504 | 18.343 0.033 | *B* | 1m0-12 | 2014-12-20 | 2457012.126 | 17.677 0.026 | *g* | 1m0-11 |
| 2014-12-14 | 2457005.506 | 18.400 0.028 | *B* | 1m0-12 | 2014-12-25 | 2457017.472 | 18.026 0.026 | *g* | 1m0-10 |
| 2014-12-15 | 2457007.129 | 18.469 0.068 | *B* | 1m0-11 | 2014-12-25 | 2457017.475 | 18.216 0.050 | *g* | 1m0-10 |
| 2014-12-15 | 2457007.132 | 18.376 0.049 | *B* | 1m0-11 | 2014-12-30 | 2457021.839 | 18.149 0.019 | *g* | 1m0-05 |
| 2014-12-20 | 2457012.115 | 18.610 0.061 | *B* | 1m0-11 | 2014-12-30 | 2457021.841 | 18.155 0.021 | *g* | 1m0-05 |
| 2014-12-20 | 2457012.118 | 18.579 0.077 | *B* | 1m0-11 | 2015-01-04 | 2457026.546 | 18.217 0.045 | *g* | 1m0-10 |
| 2014-12-25 | 2457017.464 | 18.907 0.044 | *B* | 1m0-10 | 2015-01-04 | 2457026.549 | 18.266 0.064 | *g* | 1m0-10 |
| 2014-12-30 | 2457021.830 | 19.059 0.039 | *B* | 1m0-05 | 2015-01-13 | 2457036.462 | 18.720 0.070 | *g* | 1m0-12 |
| 2014-12-30 | 2457021.833 | 19.043 0.040 | *B* | 1m0-05 | 2015-01-13 | 2457036.464 | 18.600 0.057 | *g* | 1m0-12 |
| 2015-01-04 | 2457026.537 | 19.377 0.077 | *B* | 1m0-10 | 2015-01-18 | 2457041.400 | 18.938 0.038 | *g* | 1m0-12 |
| 2015-01-04 | 2457026.540 | 19.270 0.112 | *B* | 1m0-10 | 2015-01-18 | 2457041.403 | 19.011 0.062 | *g* | 1m0-12 |
| 2015-01-18 | 2457041.392 | 19.808 0.146 | *B* | 1m0-12 | 2015-01-22 | 2457045.426 | 18.892 0.082 | *g* | 1m0-12 |
| 2015-01-18 | 2457041.394 | 19.809 0.185 | *B* | 1m0-12 | 2015-01-22 | 2457045.430 | 19.116 0.039 | *g* | 1m0-12 |
| 2015-01-22 | 2457045.413 | 20.272 0.124 | *B* | 1m0-12 | 2015-01-29 | 2457051.540 | 19.891 0.075 | *g* | 1m0-13 |
| 2015-01-22 | 2457045.417 | 20.068 0.145 | *B* | 1m0-12 | 2015-01-29 | 2457051.584 | 19.946 0.076 | *g* | 1m0-10 |
| 2015-01-29 | 2457051.527 | 20.812 0.393 | *B* | 1m0-13 | 2015-01-29 | 2457051.587 | 19.894 0.083 | *g* | 1m0-10 |
| 2015-01-29 | 2457051.530 | 20.924 0.184 | *B* | 1m0-13 | 2015-01-29 | 2457051.667 | 19.743 0.068 | *g* | 1m0-05 |
| 2015-01-29 | 2457051.570 | 21.235 0.246 | *B* | 1m0-10 | 2015-01-29 | 2457051.671 | 19.931 0.082 | *g* | 1m0-05 |
| 2015-01-29 | 2457051.574 | 20.835 0.167 | *B* | 1m0-10 | 2015-01-29 | 2457051.746 | 20.037 0.068 | *g* | 1m0-05 |
| 2015-01-29 | 2457051.654 | 20.926 0.175 | *B* | 1m0-05 | 2015-02-02 | 2457056.456 | 20.085 0.100 | *g* | 1m0-12 |
| 2015-01-29 | 2457051.658 | 20.979 0.227 | *B* | 1m0-05 | 2015-02-02 | 2457056.460 | 19.942 0.095 | *g* | 1m0-12 |
| 2015-01-29 | 2457051.729 | 20.867 0.193 | *B* | 1m0-05 | 2015-02-04 | 2457057.504 | 20.673 0.109 | *g* | 1m0-10 |
| 2015-01-29 | 2457051.733 | 20.899 0.221 | *B* | 1m0-05 | 2015-02-07 | 2457061.461 | 20.450 0.107 | *g* | 1m0-12 |
| 2015-02-02 | 2457056.443 | 21.415 0.144 | *B* | 1m0-12 | 2015-02-07 | 2457061.465 | 20.580 0.107 | *g* | 1m0-12 |
| 2015-02-02 | 2457056.447 | 21.429 0.167 | *B* | 1m0-12 | 2015-02-12 | 2457066.000 | 20.463 0.087 | *g* | 2m0 |
| 2015-02-07 | 2457061.452 | 21.716 0.234 | *B* | 1m0-12 | 2015-02-19 | 2457073.013 | 20.862 0.109 | *g* | 2m0 |
| 2015-02-12 | 2457065.983 | 21.519 0.221 | *B* | 2m0 | 2014-11-10 | 2456972.230 | 15.950 0.020 | *V* | 1m0-11 |
| 2015-02-12 | 2457065.987 | 21.707 0.277 | *B* | 2m0 | 2014-11-10 | 2456972.232 | 16.000 0.019 | *V* | 1m0-11 |
| 2015-02-16 | 2457069.927 | 21.905 0.313 | *B* | 2m0 | 2014-11-12 | 2456974.225 | 16.019 0.022 | *V* | 1m0-11 |
| 2014-11-08 | 2456969.597 | 16.178 0.016 | *g* | 1m0-12 | 2014-11-12 | 2456974.226 | 16.036 0.021 | *V* | 1m0-11 |
| 2014-11-10 | 2456972.233 | 16.117 0.015 | *g* | 1m0-11 | 2014-11-14 | 2456975.574 | 16.094 0.021 | *V* | 1m0-12 |

(a) Data have not been corrected for extinction
(b) *Swift* Telescope; LSQ (La Silla Quest, Chile); 1m0-08 (McDonald Observatory, USA); 1m0-10, 1m0-12, 1m0-13 (Sutherland, South Africa), 1m0-04, 1m0-05, 1m0-09 (Cerro Tololo, Chile); 1m0-03, 1m0-11 (Siding Spring, Australia).

**Table D1:** SN 2014dw: Photometric Data

| Date | JD | mag[(a)] | Filter | telescope[(b)] | Date | JD | mag[(a)] | Filter | telescope[(b)] |
|---|---|---|---|---|---|---|---|---|---|
| 2014-11-14 | 2456975.575 | 16.152 0.021 | *V* | 1m0-13 | 2015-02-12 | 2457065.993 | 20.426 0.115 | *V* | 2m0 |
| 2014-11-14 | 2456975.576 | 16.073 0.021 | *V* | 1m0-12 | 2015-02-16 | 2457069.930 | 20.459 0.119 | *V* | 2m0 |
| 2014-11-14 | 2456975.576 | 16.090 0.020 | *V* | 1m0-13 | 2015-02-27 | 2457080.898 | 20.614 0.245 | *V* | 2m0 |
| 2014-11-16 | 2456978.224 | 16.045 0.021 | *V* | 1m0-03 | 2014-11-08 | 2456969.599 | 15.937 0.024 | *r* | 1m0-12 |
| 2014-11-16 | 2456978.226 | 16.036 0.021 | *V* | 1m0-03 | 2014-11-08 | 2456969.601 | 15.916 0.021 | *r* | 1m0-12 |
| 2014-11-18 | 2456979.566 | 16.153 0.019 | *V* | 1m0-10 | 2014-11-10 | 2456972.239 | 15.901 0.018 | *r* | 1m0-11 |
| 2014-11-20 | 2456981.558 | 16.221 0.026 | *V* | 1m0-12 | 2014-11-10 | 2456972.240 | 15.882 0.017 | *r* | 1m0-11 |
| 2014-11-20 | 2456981.559 | 16.226 0.024 | *V* | 1m0-12 | 2014-11-12 | 2456974.233 | 15.922 0.016 | *r* | 1m0-11 |
| 2014-11-22 | 2456983.554 | 16.155 0.019 | *V* | 1m0-10 | 2014-11-12 | 2456974.235 | 15.945 0.015 | *r* | 1m0-11 |
| 2014-11-22 | 2456983.556 | 16.195 0.022 | *V* | 1m0-10 | 2014-11-14 | 2456975.575 | 15.947 0.015 | *r* | 1m0-10 |
| 2014-11-24 | 2456985.823 | 16.371 0.022 | *V* | 1m0-05 | 2014-11-14 | 2456975.576 | 15.970 0.019 | *r* | 1m0-10 |
| 2014-11-24 | 2456985.848 | 16.348 0.019 | *V* | 1m0-05 | 2014-11-14 | 2456975.583 | 15.970 0.016 | *r* | 1m0-12 |
| 2014-11-24 | 2456985.850 | 16.388 0.021 | *V* | 1m0-05 | 2014-11-14 | 2456975.584 | 15.975 0.016 | *r* | 1m0-12 |
| 2014-11-25 | 2456986.832 | 16.398 0.028 | *V* | 1m0-05 | 2014-11-16 | 2456978.223 | 15.966 0.015 | *r* | 1m0-11 |
| 2014-11-25 | 2456986.834 | 16.441 0.021 | *V* | 1m0-05 | 2014-11-18 | 2456979.564 | 15.986 0.016 | *r* | 1m0-12 |
| 2014-11-27 | 2456988.558 | 16.347 0.039 | *V* | 1m0-12 | 2014-11-18 | 2456979.566 | 16.015 0.016 | *r* | 1m0-12 |
| 2014-11-27 | 2456988.560 | 16.453 0.024 | *V* | 1m0-12 | 2014-11-20 | 2456981.582 | 16.174 0.029 | *r* | 1m0-12 |
| 2014-11-28 | 2456990.181 | 16.578 0.028 | *V* | 1m0-03 | 2014-11-20 | 2456981.584 | 16.030 0.017 | *r* | 1m0-12 |
| 2014-11-28 | 2456990.182 | 16.592 0.024 | *V* | 1m0-03 | 2014-11-22 | 2456983.555 | 16.020 0.018 | *r* | 1m0-12 |
| 2014-12-04 | 2456996.185 | 16.646 0.041 | *V* | 1m0-11 | 2014-11-22 | 2456983.556 | 15.985 0.018 | *r* | 1m0-12 |
| 2014-12-04 | 2456996.187 | 16.646 0.035 | *V* | 1m0-11 | 2014-11-25 | 2456986.798 | 16.102 0.024 | *r* | 1m0-05 |
| 2014-12-09 | 2457000.783 | 16.835 0.026 | *V* | 1m0-05 | 2014-11-25 | 2456986.800 | 16.183 0.016 | *r* | 1m0-05 |
| 2014-12-09 | 2457000.785 | 16.818 0.024 | *V* | 1m0-05 | 2014-11-28 | 2456990.189 | 16.238 0.021 | *r* | 1m0-03 |
| 2014-12-14 | 2457005.509 | 16.918 0.028 | *V* | 1m0-12 | 2014-11-28 | 2456990.191 | 16.273 0.023 | *r* | 1m0-03 |
| 2014-12-14 | 2457005.510 | 16.903 0.028 | *V* | 1m0-12 | 2014-12-04 | 2456996.194 | 16.249 0.020 | *r* | 1m0-11 |
| 2014-12-15 | 2457007.134 | 16.924 0.024 | *V* | 1m0-11 | 2014-12-04 | 2456996.195 | 16.294 0.021 | *r* | 1m0-11 |
| 2014-12-15 | 2457007.136 | 16.996 0.030 | *V* | 1m0-11 | 2014-12-09 | 2457000.792 | 16.457 0.023 | *r* | 1m0-05 |
| 2014-12-20 | 2457012.121 | 17.127 0.031 | *V* | 1m0-11 | 2014-12-09 | 2457000.794 | 16.415 0.015 | *r* | 1m0-05 |
| 2014-12-20 | 2457012.122 | 17.064 0.027 | *V* | 1m0-11 | 2014-12-14 | 2457005.518 | 16.494 0.019 | *r* | 1m0-12 |
| 2014-12-25 | 2457017.469 | 17.190 0.025 | *V* | 1m0-10 | 2014-12-14 | 2457005.519 | 16.509 0.018 | *r* | 1m0-12 |
| 2014-12-25 | 2457017.470 | 17.206 0.024 | *V* | 1m0-10 | 2014-12-15 | 2457007.143 | 16.506 0.018 | *r* | 1m0-11 |
| 2014-12-30 | 2457021.835 | 17.349 0.034 | *V* | 1m0-05 | 2014-12-15 | 2457007.144 | 16.482 0.018 | *r* | 1m0-11 |
| 2014-12-30 | 2457021.837 | 17.426 0.022 | *V* | 1m0-05 | 2014-12-20 | 2457012.131 | 16.629 0.021 | *r* | 1m0-11 |
| 2015-01-04 | 2457026.543 | 17.434 0.041 | *V* | 1m0-10 | 2014-12-25 | 2457017.478 | 16.703 0.029 | *r* | 1m0-10 |
| 2015-01-04 | 2457026.544 | 17.518 0.044 | *V* | 1m0-10 | 2014-12-25 | 2457017.479 | 16.759 0.017 | *r* | 1m0-10 |
| 2015-01-13 | 2457036.459 | 17.845 0.091 | *V* | 1m0-12 | 2014-12-30 | 2457021.844 | 16.873 0.015 | *r* | 1m0-05 |
| 2015-01-13 | 2457036.460 | 17.840 0.131 | *V* | 1m0-12 | 2014-12-30 | 2457021.845 | 16.875 0.016 | *r* | 1m0-05 |
| 2015-01-18 | 2457041.397 | 18.175 0.054 | *V* | 1m0-12 | 2015-01-04 | 2457026.551 | 16.951 0.026 | *r* | 1m0-10 |
| 2015-01-18 | 2457041.398 | 18.142 0.048 | *V* | 1m0-12 | 2015-01-04 | 2457026.553 | 16.963 0.025 | *r* | 1m0-10 |
| 2015-01-22 | 2457045.421 | 18.322 0.035 | *V* | 1m0-12 | 2015-01-08 | 2457031.478 | 17.314 0.089 | *r* | 1m0-10 |
| 2015-01-22 | 2457045.424 | 18.303 0.039 | *V* | 1m0-12 | 2015-01-08 | 2457031.479 | 17.213 0.079 | *r* | 1m0-10 |
| 2015-01-29 | 2457051.537 | 19.523 0.124 | *V* | 1m0-13 | 2015-01-13 | 2457036.467 | 17.145 0.046 | *r* | 1m0-12 |
| 2015-01-29 | 2457051.581 | 19.229 0.096 | *V* | 1m0-10 | 2015-01-13 | 2457036.469 | 17.186 0.037 | *r* | 1m0-12 |
| 2015-01-29 | 2457051.662 | 19.342 0.054 | *V* | 1m0-05 | 2015-01-18 | 2457041.405 | 17.435 0.030 | *r* | 1m0-12 |
| 2015-01-29 | 2457051.664 | 19.346 0.072 | *V* | 1m0-05 | 2015-01-18 | 2457041.407 | 17.499 0.035 | *r* | 1m0-12 |
| 2015-01-29 | 2457051.737 | 19.348 0.120 | *V* | 1m0-05 | 2015-01-22 | 2457045.434 | 17.701 0.022 | *r* | 1m0-12 |
| 2015-01-29 | 2457051.740 | 19.260 0.036 | *V* | 1m0-05 | 2015-01-22 | 2457045.436 | 17.707 0.022 | *r* | 1m0-12 |
| 2015-02-02 | 2457056.451 | 20.097 0.119 | *V* | 1m0-12 | 2015-01-29 | 2457051.750 | 18.462 0.025 | *r* | 1m0-05 |
| 2015-02-02 | 2457056.453 | 19.809 0.071 | *V* | 1m0-12 | 2015-01-29 | 2457051.752 | 18.505 0.026 | *r* | 1m0-05 |
| 2015-02-04 | 2457057.521 | 20.395 0.351 | *V* | 1m0-13 | 2015-02-02 | 2457056.464 | 19.127 0.050 | *r* | 1m0-12 |
| 2015-02-04 | 2457057.525 | 20.072 0.173 | *V* | 1m0-13 | 2015-02-02 | 2457056.466 | 18.956 0.046 | *r* | 1m0-12 |
| 2015-02-07 | 2457061.456 | 19.972 0.079 | *V* | 1m0-12 | 2015-02-04 | 2457057.509 | 18.905 0.048 | *r* | 1m0-10 |
| 2015-02-07 | 2457061.458 | 20.071 0.093 | *V* | 1m0-12 | 2015-02-04 | 2457057.513 | 19.258 0.066 | *r* | 1m0-10 |
| 2015-02-08 | 2457062.470 | 20.047 0.154 | *V* | 1m0-10 | 2015-02-07 | 2457061.469 | 19.079 0.028 | *r* | 1m0-12 |
| 2015-02-08 | 2457062.473 | 19.962 0.195 | *V* | 1m0-10 | 2015-02-07 | 2457061.471 | 19.241 0.041 | *r* | 1m0-12 |
| 2015-02-09 | 2457062.516 | 19.987 0.094 | *V* | 1m0-12 | 2015-02-10 | 2457064.254 | 19.294 0.080 | *r* | 1m0-03 |
| 2015-02-09 | 2457062.520 | 20.119 0.112 | *V* | 1m0-12 | 2015-02-10 | 2457064.257 | 19.180 0.065 | *r* | 1m0-03 |
| 2015-02-12 | 2457066.333 | 20.252 0.142 | *V* | 1m0-12 | 2015-02-12 | 2457066.354 | 19.349 0.126 | *r* | 1m0-12 |
| 2015-02-12 | 2457066.337 | 19.956 0.183 | *V* | 1m0-12 | 2015-02-11 | 2457064.987 | 19.060 0.080 | *r* | 2m0 |
| 2015-02-12 | 2457065.991 | 20.520 0.152 | *V* | 2m0 | 2015-02-11 | 2457064.990 | 18.980 0.052 | *r* | 2m0 |

(a) Data have not been corrected for extinction
(b) *Swift* Telescope; LSQ (La Silla Quest, Chile); 1m0-08 (McDonald Observatory, USA); 1m0-10, 1m0-12, 1m0-13 (Sutherland, South Africa), 1m0-04, 1m0-05, 1m0-09 (Cerro Tololo, Chile); 1m0-03, 1m0-11 (Siding Spring, Australia).

**Table D1:** SN 2014dw: Photometric Data

| Date | JD | mag[(a)] | Filter | telescope[(b)] | Date | JD | mag[(a)] | Filter | telescope[(b)] |
|---|---|---|---|---|---|---|---|---|---|
| 2015-02-12 | 2457066.004 | 19.193 0.057 | $r$ | 2m0 | 2014-12-20 | 2457012.132 | 16.456 0.027 | $i$ | 1m0-11 |
| 2015-02-12 | 2457066.006 | 19.141 0.053 | $r$ | 2m0 | 2014-12-20 | 2457012.134 | 16.492 0.026 | $i$ | 1m0-11 |
| 2015-02-16 | 2457069.937 | 19.157 0.043 | $r$ | 2m0 | 2014-12-25 | 2457017.482 | 16.629 0.024 | $i$ | 1m0-10 |
| 2015-02-19 | 2457073.017 | 19.555 0.053 | $r$ | 2m0 | 2014-12-25 | 2457017.483 | 16.648 0.031 | $i$ | 1m0-10 |
| 2015-02-23 | 2457076.934 | 19.298 0.030 | $r$ | 2m0 | 2014-12-30 | 2457021.847 | 16.764 0.024 | $i$ | 1m0-05 |
| 2015-03-15 | 2457096.945 | 19.922 0.063 | $r$ | 2m0 | 2014-12-30 | 2457021.849 | 16.758 0.022 | $i$ | 1m0-05 |
| 2015-03-21 | 2457102.876 | 20.221 0.074 | $r$ | 2m0 | 2015-01-04 | 2457026.555 | 16.824 0.036 | $i$ | 1m0-10 |
| 2015-03-29 | 2457110.852 | 20.515 0.084 | $r$ | 2m0 | 2015-01-04 | 2457026.556 | 16.783 0.031 | $i$ | 1m0-10 |
| 2014-11-08 | 2456969.603 | 15.972 0.035 | $i$ | 1m0-12 | 2015-01-08 | 2457031.481 | 17.047 0.044 | $i$ | 1m0-10 |
| 2014-11-08 | 2456969.604 | 16.004 0.042 | $i$ | 1m0-12 | 2015-01-13 | 2457036.470 | 17.297 0.084 | $i$ | 1m0-12 |
| 2014-11-10 | 2456972.242 | 15.823 0.019 | $i$ | 1m0-11 | 2015-01-13 | 2457036.472 | 17.164 0.075 | $i$ | 1m0-12 |
| 2014-11-10 | 2456972.243 | 15.871 0.019 | $i$ | 1m0-11 | 2015-01-18 | 2457041.409 | 17.475 0.060 | $i$ | 1m0-12 |
| 2014-11-12 | 2456974.237 | 15.886 0.022 | $i$ | 1m0-11 | 2015-01-18 | 2457041.410 | 17.431 0.051 | $i$ | 1m0-12 |
| 2014-11-12 | 2456974.238 | 15.873 0.023 | $i$ | 1m0-11 | 2015-01-22 | 2457045.439 | 17.838 0.096 | $i$ | 1m0-12 |
| 2014-11-14 | 2456975.578 | 15.922 0.026 | $i$ | 1m0-10 | 2015-01-22 | 2457045.442 | 17.525 0.027 | $i$ | 1m0-12 |
| 2014-11-14 | 2456975.586 | 15.950 0.022 | $i$ | 1m0-12 | 2015-01-29 | 2457051.597 | 18.418 0.050 | $i$ | 1m0-10 |
| 2014-11-14 | 2456975.588 | 15.943 0.024 | $i$ | 1m0-12 | 2015-01-29 | 2457051.755 | 18.440 0.053 | $i$ | 1m0-05 |
| 2014-11-16 | 2456978.224 | 15.907 0.018 | $i$ | 1m0-11 | 2015-01-29 | 2457051.757 | 18.517 0.037 | $i$ | 1m0-05 |
| 2014-11-16 | 2456978.226 | 15.900 0.019 | $i$ | 1m0-11 | 2015-02-02 | 2457056.469 | 18.772 0.086 | $i$ | 1m0-12 |
| 2014-11-18 | 2456979.567 | 15.995 0.023 | $i$ | 1m0-12 | 2015-02-02 | 2457056.471 | 18.842 0.129 | $i$ | 1m0-12 |
| 2014-11-18 | 2456979.569 | 15.980 0.021 | $i$ | 1m0-12 | 2015-02-04 | 2457057.517 | 18.988 0.062 | $i$ | 1m0-10 |
| 2014-11-20 | 2456981.586 | 15.988 0.025 | $i$ | 1m0-12 | 2015-02-04 | 2457057.520 | 18.907 0.060 | $i$ | 1m0-10 |
| 2014-11-20 | 2456981.587 | 15.988 0.027 | $i$ | 1m0-12 | 2015-02-07 | 2457061.474 | 19.068 0.056 | $i$ | 1m0-12 |
| 2014-11-22 | 2456983.558 | 15.955 0.019 | $i$ | 1m0-12 | 2015-02-07 | 2457061.476 | 18.924 0.070 | $i$ | 1m0-12 |
| 2014-11-22 | 2456983.559 | 15.966 0.021 | $i$ | 1m0-12 | 2015-02-10 | 2457064.261 | 19.108 0.137 | $i$ | 1m0-03 |
| 2014-11-25 | 2456986.801 | 16.093 0.027 | $i$ | 1m0-05 | 2015-02-12 | 2457066.358 | 19.290 0.149 | $i$ | 1m0-12 |
| 2014-11-25 | 2456986.803 | 16.015 0.025 | $i$ | 1m0-05 | 2015-02-12 | 2457066.362 | 19.054 0.142 | $i$ | 1m0-12 |
| 2014-11-28 | 2456990.192 | 16.150 0.030 | $i$ | 1m0-03 | 2015-02-11 | 2457064.992 | 18.935 0.071 | $i$ | 2m0 |
| 2014-11-28 | 2456990.194 | 16.286 0.031 | $i$ | 1m0-03 | 2015-02-12 | 2457066.009 | 19.415 0.054 | $i$ | 2m0 |
| 2014-12-04 | 2456996.197 | 16.104 0.027 | $i$ | 1m0-11 | 2015-02-12 | 2457066.011 | 19.435 0.054 | $i$ | 2m0 |
| 2014-12-04 | 2456996.199 | 16.153 0.025 | $i$ | 1m0-11 | 2015-02-16 | 2457069.940 | 19.531 0.058 | $i$ | 2m0 |
| 2014-12-09 | 2457000.795 | 16.330 0.021 | $i$ | 1m0-05 | 2015-02-19 | 2457073.020 | 19.805 0.082 | $i$ | 2m0 |
| 2014-12-09 | 2457000.797 | 16.319 0.021 | $i$ | 1m0-05 | 2015-02-23 | 2457076.936 | 19.824 0.096 | $i$ | 2m0 |
| 2014-12-14 | 2457005.521 | 16.368 0.023 | $i$ | 1m0-12 | 2015-02-27 | 2457080.908 | 19.875 0.117 | $i$ | 2m0 |
| 2014-12-14 | 2457005.522 | 16.386 0.024 | $i$ | 1m0-12 | 2015-03-02 | 2457083.993 | 20.051 0.205 | $i$ | 2m0 |
| 2014-12-15 | 2457007.146 | 16.367 0.027 | $i$ | 1m0-11 | 2015-03-10 | 2457091.946 | 20.560 0.152 | $i$ | 2m0 |
| 2014-12-15 | 2457007.148 | 16.380 0.025 | $i$ | 1m0-11 | 2015-03-10 | 2457091.951 | 20.570 0.123 | $i$ | 2m0 |

(a) Data have not been corrected for extinction
(b) *Swift* Telescope; LSQ (La Silla Quest, Chile); 1m0-08 (McDonald Observatory, USA); 1m0-10, 1m0-12, 1m0-13 (Sutherland, South Africa), 1m0-04, 1m0-05, 1m0-09 (Cerro Tololo, Chile); 1m0-03, 1m0-11 (Siding Spring, Australia).

**Table D1:** SN 2015W: Photometric Data

| Date | JD | mag[(a)] | Filter | telescope[(b)] | Date | JD | mag[(a)] | Filter | telescope[(b)] |
|---|---|---|---|---|---|---|---|---|---|
| 2015-01-12 | 2457035.423 | 17.238 0.014 | *B* | 1m0-10 | 2015-03-03 | 2457085.315 | 18.480 0.216 | *g* | 1m0-12 |
| 2015-01-14 | 2457037.412 | 17.379 0.034 | *B* | 1m0-10 | 2015-03-07 | 2457089.265 | 18.614 0.030 | *g* | 1m0-10 |
| 2015-01-16 | 2457039.127 | 17.461 0.023 | *B* | 1m0-11 | 2015-03-07 | 2457089.300 | 18.535 0.010 | *g* | 1m0-12 |
| 2015-01-18 | 2457041.324 | 17.927 0.079 | *B* | 1m0-12 | 2015-03-09 | 2457090.937 | 18.577 0.041 | *g* | 1m0-03 |
| 2015-01-22 | 2457045.314 | 17.945 0.026 | *B* | 1m0-12 | 2015-03-14 | 2457095.989 | 18.712 0.051 | *g* | 1m0-03 |
| 2015-01-28 | 2457051.429 | 18.247 0.088 | *B* | 1m0-12 | 2015-03-18 | 2457099.951 | 18.799 0.037 | *g* | 1m0-11 |
| 2015-01-30 | 2457053.037 | 18.305 0.025 | *B* | 1m0-11 | 2015-03-19 | 2457101.284 | 18.779 0.014 | *g* | 1m0-10 |
| 2015-01-30 | 2457053.279 | 18.380 0.019 | *B* | 1m0-10 | 2015-03-19 | 2457101.328 | 18.830 0.015 | *g* | 1m0-12 |
| 2015-02-03 | 2457056.997 | 18.511 0.026 | *B* | 1m0-03 | 2015-03-20 | 2457101.909 | 18.897 0.026 | *g* | 1m0-11 |
| 2015-02-07 | 2457060.708 | 18.483 0.051 | *B* | 1m0-08 | 2015-03-24 | 2457105.610 | 18.943 0.229 | *g* | 1m0-08 |
| 2015-02-11 | 2457065.061 | 18.901 0.021 | *B* | 1m0-03 | 2015-03-29 | 2457111.302 | 19.082 0.243 | *g* | 1m0-12 |
| 2015-02-11 | 2457065.400 | 18.815 0.123 | *B* | 1m0-10 | 2015-03-30 | 2457112.280 | 18.960 0.111 | *g* | 1m0-12 |
| 2015-02-12 | 2457065.613 | 18.753 0.036 | *B* | 1m0-05 | 2015-04-01 | 2457114.499 | 19.219 0.045 | *g* | 1m0-05 |
| 2015-02-12 | 2457066.405 | 18.649 0.051 | *B* | 1m0-13 | 2015-04-03 | 2457115.526 | 19.125 0.023 | *g* | 1m0-05 |
| 2015-02-16 | 2457070.291 | 19.076 0.013 | *B* | 1m0-10 | 2015-04-04 | 2457117.230 | 19.226 0.064 | *g* | 1m0-10 |
| 2015-02-18 | 2457072.310 | 19.142 0.043 | *B* | 1m0-12 | 2015-04-05 | 2457117.564 | 19.222 0.092 | *g* | 1m0-05 |
| 2015-02-22 | 2457076.340 | 19.428 0.012 | *B* | 1m0-13 | 2015-04-06 | 2457118.868 | 19.071 0.085 | *g* | 1m0-11 |
| 2015-02-26 | 2457079.927 | 19.207 0.084 | *B* | 1m0-11 | 2015-04-06 | 2457119.230 | 19.425 0.055 | *g* | 1m0-13 |
| 2015-03-02 | 2457083.948 | 19.576 0.350 | *B* | 1m0-11 | 2015-04-07 | 2457119.598 | 19.248 0.019 | *g* | 1m0-08 |
| 2015-03-03 | 2457085.304 | 19.360 0.100 | *B* | 1m0-12 | 2015-04-08 | 2457120.668 | 19.273 0.040 | *g* | 1m0-08 |
| 2015-03-07 | 2457089.251 | 19.488 0.011 | *B* | 1m0-10 | 2015-04-09 | 2457121.879 | 19.325 0.028 | *g* | 1m0-03 |
| 2015-03-07 | 2457089.288 | 19.358 0.067 | *B* | 1m0-12 | 2015-04-11 | 2457123.896 | 19.422 0.015 | *g* | 1m0-03 |
| 2015-03-09 | 2457090.924 | 19.585 0.039 | *B* | 1m0-03 | 2015-04-12 | 2457125.220 | 19.663 0.059 | *g* | 1m0-12 |
| 2015-03-13 | 2457095.355 | 19.484 0.203 | *B* | 1m0-12 | 2015-04-13 | 2457126.219 | 19.594 0.147 | *g* | 1m0-12 |
| 2015-03-14 | 2457095.976 | 19.583 0.211 | *B* | 1m0-03 | 2015-04-15 | 2457127.863 | 19.662 0.020 | *g* | 1m0-03 |
| 2015-03-19 | 2457101.270 | 19.772 0.088 | *B* | 1m0-10 | 2015-04-15 | 2457128.229 | 20.037 0.097 | *g* | 1m0-10 |
| 2015-03-19 | 2457101.314 | 19.831 0.056 | *B* | 1m0-12 | 2015-04-16 | 2457129.254 | 19.818 0.141 | *g* | 1m0-12 |
| 2015-03-20 | 2457101.896 | 19.907 0.036 | *B* | 1m0-11 | 2015-04-19 | 2457132.257 | 19.753 0.080 | *g* | 1m0-13 |
| 2015-03-24 | 2457105.596 | 19.694 0.207 | *B* | 1m0-08 | 2015-04-20 | 2457133.492 | 19.897 0.136 | *g* | 1m0-05 |
| 2015-03-29 | 2457111.240 | 19.747 0.149 | *B* | 1m0-12 | 2015-04-22 | 2457135.237 | 20.034 0.054 | *g* | 1m0-10 |
| 2015-04-01 | 2457114.340 | 19.893 0.473 | *B* | 1m0-10 | 2015-04-27 | 2457140.469 | 19.977 0.122 | *g* | 1m0-05 |
| 2015-04-03 | 2457115.514 | 20.057 0.204 | *B* | 1m0-05 | 2015-05-02 | 2457144.612 | 20.107 0.314 | *g* | 1m0-08 |
| 2015-04-04 | 2457117.228 | 20.219 0.450 | *B* | 1m0-13 | 2015-05-05 | 2457148.469 | 20.812 0.125 | *g* | 1m0-05 |
| 2015-04-04 | 2457117.247 | 20.109 0.117 | *B* | 1m0-12 | 2015-05-06 | 2457148.615 | 20.526 0.262 | *g* | 1m0-08 |
| 2015-04-07 | 2457119.614 | 20.056 0.089 | *B* | 1m0-08 | 2015-05-07 | 2457150.465 | 20.609 0.024 | *g* | 1m0-05 |
| 2015-04-08 | 2457120.622 | 20.065 0.106 | *B* | 1m0-08 | 2015-05-10 | 2457153.215 | 20.719 0.096 | *g* | 1m0-12 |
| 2015-04-09 | 2457121.864 | 20.189 0.188 | *B* | 1m0-03 | 2015-01-12 | 2457035.426 | 16.714 0.016 | *V* | 1m0-10 |
| 2015-04-11 | 2457123.896 | 20.157 0.110 | *B* | 1m0-11 | 2015-01-14 | 2457037.415 | 16.726 0.027 | *V* | 1m0-10 |
| 2015-04-12 | 2457124.929 | 20.342 0.429 | *B* | 1m0-03 | 2015-01-16 | 2457039.130 | 16.715 0.021 | *V* | 1m0-11 |
| 2015-04-13 | 2457126.219 | 20.189 0.192 | *B* | 1m0-10 | 2015-01-22 | 2457045.317 | 16.893 0.030 | *V* | 1m0-12 |
| 2015-01-12 | 2457035.429 | 16.934 0.015 | *g* | 1m0-10 | 2015-01-28 | 2457051.432 | 17.077 0.016 | *V* | 1m0-12 |
| 2015-01-14 | 2457037.418 | 17.008 0.044 | *g* | 1m0-10 | 2015-01-30 | 2457053.041 | 17.093 0.041 | *V* | 1m0-11 |
| 2015-01-16 | 2457039.133 | 17.004 0.032 | *g* | 1m0-11 | 2015-01-30 | 2457053.284 | 17.061 0.030 | *V* | 1m0-10 |
| 2015-01-18 | 2457041.329 | 17.195 0.027 | *g* | 1m0-12 | 2015-02-03 | 2457057.002 | 17.260 0.059 | *V* | 1m0-03 |
| 2015-01-19 | 2457042.428 | 17.201 0.014 | *g* | 1m0-12 | 2015-02-07 | 2457060.713 | 17.195 0.023 | *V* | 1m0-08 |
| 2015-01-22 | 2457045.321 | 17.392 0.023 | *g* | 1m0-12 | 2015-02-11 | 2457065.067 | 17.418 0.038 | *V* | 1m0-03 |
| 2015-01-28 | 2457051.436 | 17.604 0.066 | *g* | 1m0-12 | 2015-02-11 | 2457065.408 | 17.442 0.031 | *V* | 1m0-10 |
| 2015-01-30 | 2457053.044 | 17.638 0.038 | *g* | 1m0-11 | 2015-02-12 | 2457065.618 | 17.372 0.013 | *V* | 1m0-05 |
| 2015-01-30 | 2457053.288 | 17.575 0.020 | *g* | 1m0-10 | 2015-02-12 | 2457066.410 | 17.367 0.079 | *V* | 1m0-13 |
| 2015-02-03 | 2457057.006 | 17.850 0.068 | *g* | 1m0-03 | 2015-02-16 | 2457070.296 | 17.526 0.017 | *V* | 1m0-10 |
| 2015-02-07 | 2457060.717 | 17.929 0.012 | *g* | 1m0-08 | 2015-02-18 | 2457072.314 | 17.551 0.018 | *V* | 1m0-12 |
| 2015-02-11 | 2457065.071 | 18.054 0.038 | *g* | 1m0-03 | 2015-02-22 | 2457076.367 | 17.765 0.058 | *V* | 1m0-13 |
| 2015-02-11 | 2457065.429 | 18.289 0.027 | *g* | 1m0-10 | 2015-02-26 | 2457079.932 | 17.751 0.041 | *V* | 1m0-11 |
| 2015-02-12 | 2457065.623 | 18.036 0.028 | *g* | 1m0-05 | 2015-03-02 | 2457083.954 | 17.720 0.010 | *V* | 1m0-11 |
| 2015-02-12 | 2457066.414 | 18.230 0.016 | *g* | 1m0-13 | 2015-03-03 | 2457085.311 | 17.686 0.010 | *V* | 1m0-12 |
| 2015-02-16 | 2457070.300 | 18.154 0.064 | *g* | 1m0-10 | 2015-03-07 | 2457089.259 | 17.863 0.031 | *V* | 1m0-10 |
| 2015-02-18 | 2457072.318 | 18.244 0.013 | *g* | 1m0-12 | 2015-03-07 | 2457089.294 | 17.940 0.046 | *V* | 1m0-12 |
| 2015-02-22 | 2457076.394 | 18.562 0.042 | *g* | 1m0-13 | 2015-03-09 | 2457090.931 | 17.997 0.021 | *V* | 1m0-03 |
| 2015-02-26 | 2457079.936 | 18.427 0.036 | *g* | 1m0-11 | 2015-03-13 | 2457095.360 | 18.052 0.030 | *V* | 1m0-12 |
| 2015-03-02 | 2457083.959 | 18.649 0.116 | *g* | 1m0-11 | 2015-03-14 | 2457095.983 | 18.083 0.029 | *V* | 1m0-03 |

(a) Data have not been corrected for extinction
(b) *Swift* Telescope; LSQ (La Silla Quest, Chile); 1m0-08 (McDonald Observatory, USA); 1m0-10, 1m0-12, 1m0-13 (Sutherland, South Africa), 1m0-04, 1m0-05, 1m0-09 (Cerro Tololo, Chile); 1m0-03, 1m0-11 (Siding Spring, Australia).

**Table D1:** SN 2015W: Photometric Data

| Date | JD | mag[(a)] | Filter | telescope[(b)] | Date | JD | mag[(a)] | Filter | telescope[(b)] |
|---|---|---|---|---|---|---|---|---|---|
| 2015-03-18 | 2457099.946 | 18.080 0.033 | *V* | 1m0-11 | 2015-03-19 | 2457101.335 | 17.319 0.015 | *r* | 1m0-12 |
| 2015-03-19 | 2457101.277 | 18.090 0.026 | *V* | 1m0-10 | 2015-03-20 | 2457101.916 | 17.474 0.021 | *r* | 1m0-11 |
| 2015-03-19 | 2457101.322 | 18.143 0.044 | *V* | 1m0-12 | 2015-03-24 | 2457105.617 | 17.470 0.068 | *r* | 1m0-08 |
| 2015-03-20 | 2457101.903 | 18.257 0.013 | *V* | 1m0-11 | 2015-03-29 | 2457111.307 | 17.597 0.017 | *r* | 1m0-12 |
| 2015-03-24 | 2457105.605 | 18.261 0.141 | *V* | 1m0-08 | 2015-03-30 | 2457112.287 | 17.532 0.043 | *r* | 1m0-12 |
| 2015-03-29 | 2457111.246 | 18.166 0.014 | *V* | 1m0-12 | 2015-04-02 | 2457114.506 | 17.532 0.027 | *r* | 1m0-05 |
| 2015-03-30 | 2457112.275 | 18.319 0.134 | *V* | 1m0-13 | 2015-04-03 | 2457115.533 | 17.354 0.015 | *r* | 1m0-05 |
| 2015-04-01 | 2457114.491 | 18.479 0.015 | *V* | 1m0-05 | 2015-04-04 | 2457117.238 | 17.609 0.020 | *r* | 1m0-10 |
| 2015-04-03 | 2457115.519 | 18.453 0.018 | *V* | 1m0-05 | 2015-04-05 | 2457117.573 | 17.541 0.045 | *r* | 1m0-05 |
| 2015-04-04 | 2457117.236 | 18.892 0.138 | *V* | 1m0-13 | 2015-04-06 | 2457119.238 | 17.809 0.032 | *r* | 1m0-13 |
| 2015-04-04 | 2457117.254 | 18.562 0.031 | *V* | 1m0-12 | 2015-04-07 | 2457119.604 | 17.579 0.024 | *r* | 1m0-08 |
| 2015-04-05 | 2457117.558 | 18.645 0.066 | *V* | 1m0-05 | 2015-04-08 | 2457120.675 | 17.580 0.017 | *r* | 1m0-08 |
| 2015-04-06 | 2457118.669 | 18.400 0.015 | *V* | 1m0-08 | 2015-04-09 | 2457121.886 | 17.722 0.051 | *r* | 1m0-03 |
| 2015-04-07 | 2457119.623 | 18.521 0.018 | *V* | 1m0-08 | 2015-04-11 | 2457123.903 | 17.734 0.022 | *r* | 1m0-03 |
| 2015-04-08 | 2457120.629 | 18.548 0.073 | *V* | 1m0-08 | 2015-04-12 | 2457125.228 | 17.740 0.042 | *r* | 1m0-12 |
| 2015-04-09 | 2457121.872 | 18.707 0.026 | *V* | 1m0-03 | 2015-04-13 | 2457126.228 | 17.893 0.044 | *r* | 1m0-12 |
| 2015-04-11 | 2457123.904 | 18.529 0.046 | *V* | 1m0-11 | 2015-04-15 | 2457127.872 | 17.865 0.015 | *r* | 1m0-03 |
| 2015-04-12 | 2457124.940 | 18.899 0.047 | *V* | 1m0-03 | 2015-04-15 | 2457128.245 | 18.070 0.012 | *r* | 1m0-10 |
| 2015-04-13 | 2457126.228 | 18.834 0.030 | *V* | 1m0-10 | 2015-04-16 | 2457129.237 | 18.141 0.064 | *r* | 1m0-12 |
| 2015-04-15 | 2457128.221 | 19.050 0.067 | *V* | 1m0-10 | 2015-04-18 | 2457131.219 | 17.971 0.116 | *r* | 1m0-10 |
| 2015-04-16 | 2457129.248 | 19.184 0.063 | *V* | 1m0-12 | 2015-04-19 | 2457132.246 | 17.841 0.032 | *r* | 1m0-12 |
| 2015-04-17 | 2457129.916 | 19.111 0.445 | *V* | 1m0-03 | 2015-04-20 | 2457133.268 | 18.417 0.021 | *r* | 1m0-13 |
| 2015-04-18 | 2457131.227 | 19.262 0.125 | *V* | 1m0-12 | 2015-04-20 | 2457133.474 | 18.251 0.039 | *r* | 1m0-05 |
| 2015-04-19 | 2457132.253 | 19.387 0.166 | *V* | 1m0-13 | 2015-04-22 | 2457134.515 | 18.087 0.015 | *r* | 1m0-05 |
| 2015-04-20 | 2457132.599 | 19.261 0.076 | *V* | 1m0-08 | 2015-04-27 | 2457139.513 | 18.968 0.021 | *r* | 1m0-05 |
| 2015-04-20 | 2457133.485 | 19.273 0.050 | *V* | 1m0-05 | 2015-04-28 | 2457141.207 | 18.499 0.142 | *r* | 1m0-12 |
| 2015-04-22 | 2457135.230 | 19.452 0.045 | *V* | 1m0-10 | 2015-05-01 | 2457144.461 | 18.916 0.030 | *r* | 1m0-05 |
| 2015-04-27 | 2457140.463 | 19.671 0.102 | *V* | 1m0-05 | 2015-05-03 | 2457146.203 | 18.882 0.138 | *r* | 1m0-13 |
| 2015-05-02 | 2457144.607 | 19.898 0.286 | *V* | 1m0-08 | 2015-05-03 | 2457146.227 | 18.599 0.202 | *r* | 1m0-10 |
| 2015-05-03 | 2457146.211 | 20.082 0.249 | *V* | 1m0-10 | 2015-05-05 | 2457148.208 | 19.187 0.404 | *r* | 1m0-13 |
| 2015-05-04 | 2457147.204 | 20.199 0.037 | *V* | 1m0-13 | 2015-05-06 | 2457148.500 | 18.870 0.144 | *r* | 1m0-05 |
| 2015-05-04 | 2457147.234 | 19.939 0.060 | *V* | 1m0-12 | 2015-05-07 | 2457150.202 | 18.903 0.178 | *r* | 1m0-13 |
| 2015-05-05 | 2457148.464 | 19.676 0.169 | *V* | 1m0-05 | 2015-05-10 | 2457152.610 | 19.057 0.143 | *r* | 1m0-08 |
| 2015-05-06 | 2457148.607 | 20.289 0.230 | *V* | 1m0-08 | 2015-09-06 | 2457272.096 | 19.806 0.172 | *r* | 2m0 |
| 2015-05-07 | 2457150.460 | 20.190 0.240 | *V* | 1m0-05 | 2015-09-06 | 2457272.100 | 19.952 0.187 | *r* | 2m0 |
| 2015-05-10 | 2457153.207 | 20.499 0.282 | *V* | 1m0-12 | 2015-09-10 | 2457276.115 | 20.254 0.074 | *r* | 2m0 |
| 2015-01-12 | 2457034.776 | 16.500 0.000 | *r* | Atel/CBAT | 2015-09-10 | 2457276.119 | 20.306 0.057 | *r* | 2m0 |
| 2015-01-12 | 2457035.432 | 16.528 0.022 | *r* | 1m0-10 | 2015-10-13 | 2457309.086 | 20.571 0.060 | *r* | 2m0 |
| 2015-01-14 | 2457037.421 | 16.574 0.053 | *r* | 1m0-10 | 2015-10-13 | 2457309.090 | 20.676 0.065 | *r* | 2m0 |
| 2015-01-16 | 2457039.136 | 16.496 0.029 | *r* | 1m0-11 | 2015-01-12 | 2457035.434 | 16.608 0.033 | *i* | 1m0-10 |
| 2015-01-22 | 2457045.326 | 16.665 0.012 | *r* | 1m0-12 | 2015-01-14 | 2457037.423 | 16.590 0.034 | *i* | 1m0-10 |
| 2015-01-28 | 2457051.441 | 16.665 0.041 | *r* | 1m0-12 | 2015-01-16 | 2457039.138 | 16.506 0.030 | *i* | 1m0-11 |
| 2015-01-30 | 2457053.049 | 16.669 0.025 | *r* | 1m0-11 | 2015-01-18 | 2457041.335 | 16.539 0.039 | *i* | 1m0-12 |
| 2015-01-30 | 2457053.292 | 16.656 0.017 | *r* | 1m0-10 | 2015-01-22 | 2457045.329 | 16.543 0.037 | *i* | 1m0-12 |
| 2015-02-03 | 2457057.010 | 16.844 0.023 | *r* | 1m0-03 | 2015-01-28 | 2457051.444 | 16.606 0.042 | *i* | 1m0-12 |
| 2015-02-07 | 2457060.722 | 16.752 0.044 | *r* | 1m0-08 | 2015-01-30 | 2457053.053 | 16.591 0.012 | *i* | 1m0-11 |
| 2015-02-11 | 2457065.435 | 16.972 0.015 | *r* | 1m0-10 | 2015-01-30 | 2457053.296 | 16.649 0.037 | *i* | 1m0-10 |
| 2015-02-12 | 2457065.628 | 16.802 0.041 | *r* | 1m0-05 | 2015-02-03 | 2457057.014 | 16.880 0.025 | *i* | 1m0-03 |
| 2015-02-12 | 2457066.419 | 16.984 0.033 | *r* | 1m0-13 | 2015-02-07 | 2457060.726 | 16.736 0.018 | *i* | 1m0-08 |
| 2015-02-16 | 2457070.305 | 16.852 0.015 | *r* | 1m0-10 | 2015-02-12 | 2457065.631 | 16.775 0.021 | *i* | 1m0-05 |
| 2015-02-18 | 2457072.323 | 16.884 0.025 | *r* | 1m0-12 | 2015-02-12 | 2457066.423 | 16.956 0.014 | *i* | 1m0-13 |
| 2015-02-22 | 2457076.376 | 17.228 0.075 | *r* | 1m0-13 | 2015-02-16 | 2457070.309 | 16.892 0.020 | *i* | 1m0-10 |
| 2015-02-26 | 2457079.940 | 17.026 0.015 | *r* | 1m0-11 | 2015-02-18 | 2457072.326 | 16.931 0.021 | *i* | 1m0-12 |
| 2015-03-02 | 2457083.963 | 17.195 0.123 | *r* | 1m0-11 | 2015-02-22 | 2457076.386 | 17.136 0.051 | *i* | 1m0-13 |
| 2015-03-07 | 2457089.272 | 17.117 0.010 | *r* | 1m0-10 | 2015-02-26 | 2457079.944 | 17.050 0.031 | *i* | 1m0-11 |
| 2015-03-07 | 2457089.307 | 17.118 0.035 | *r* | 1m0-12 | 2015-03-02 | 2457083.966 | 17.276 0.021 | *i* | 1m0-11 |
| 2015-03-09 | 2457090.944 | 17.247 0.026 | *r* | 1m0-03 | 2015-03-07 | 2457089.276 | 17.217 0.020 | *i* | 1m0-10 |
| 2015-03-14 | 2457095.996 | 17.222 0.021 | *r* | 1m0-03 | 2015-03-07 | 2457089.313 | 17.167 0.020 | *i* | 1m0-12 |
| 2015-03-18 | 2457099.958 | 17.281 0.058 | *r* | 1m0-11 | 2015-03-09 | 2457090.949 | 17.148 0.049 | *i* | 1m0-03 |
| 2015-03-19 | 2457101.291 | 17.259 0.032 | *r* | 1m0-10 | 2015-03-14 | 2457096.001 | 17.319 0.018 | *i* | 1m0-03 |

(a) Data have not been corrected for extinction
(b) *Swift* Telescope; LSQ (La Silla Quest, Chile); 1m0-08 (McDonald Observatory, USA); 1m0-10, 1m0-12, 1m0-13 (Sutherland, South Africa), 1m0-04, 1m0-05, 1m0-09 (Cerro Tololo, Chile); 1m0-03, 1m0-11 (Siding Spring, Australia).

**Table D1:** SN 2015W: Photometric Data

| Date | JD | mag[(a)] | Filter | telescope[(b)] | Date | JD | mag[(a)] | Filter | telescope[(b)] |
|---|---|---|---|---|---|---|---|---|---|
| 2015-03-18 | 2457099.963 | 17.284 0.032 | *i* | 1m0-11 | 2015-04-18 | 2457131.224 | 18.035 0.040 | *i* | 1m0-10 |
| 2015-03-19 | 2457101.295 | 17.369 0.021 | *i* | 1m0-10 | 2015-04-19 | 2457132.251 | 18.017 0.018 | *i* | 1m0-12 |
| 2015-03-19 | 2457101.339 | 17.259 0.025 | *i* | 1m0-12 | 2015-04-20 | 2457133.273 | 18.547 0.034 | *i* | 1m0-13 |
| 2015-03-20 | 2457101.921 | 17.380 0.012 | *i* | 1m0-11 | 2015-04-20 | 2457133.479 | 18.167 0.019 | *i* | 1m0-05 |
| 2015-03-24 | 2457105.621 | 17.663 0.053 | *i* | 1m0-08 | 2015-04-22 | 2457134.520 | 18.250 0.031 | *i* | 1m0-05 |
| 2015-03-29 | 2457111.311 | 17.679 0.079 | *i* | 1m0-12 | 2015-04-27 | 2457139.519 | 18.805 0.089 | *i* | 1m0-05 |
| 2015-03-30 | 2457112.292 | 17.574 0.019 | *i* | 1m0-12 | 2015-04-28 | 2457141.212 | 18.715 0.118 | *i* | 1m0-12 |
| 2015-04-02 | 2457114.511 | 17.569 0.035 | *i* | 1m0-05 | 2015-05-01 | 2457144.466 | 18.954 0.100 | *i* | 1m0-05 |
| 2015-04-03 | 2457115.538 | 17.535 0.039 | *i* | 1m0-05 | 2015-05-03 | 2457146.210 | 18.496 0.124 | *i* | 1m0-13 |
| 2015-04-04 | 2457117.244 | 17.636 0.024 | *i* | 1m0-10 | 2015-05-03 | 2457146.232 | 19.144 0.077 | *i* | 1m0-10 |
| 2015-04-06 | 2457119.244 | 17.634 0.033 | *i* | 1m0-13 | 2015-05-05 | 2457148.211 | 18.152 0.394 | *i* | 1m0-13 |
| 2015-04-07 | 2457119.610 | 17.681 0.012 | *i* | 1m0-08 | 2015-05-06 | 2457148.505 | 18.926 0.043 | *i* | 1m0-05 |
| 2015-04-08 | 2457120.680 | 17.734 0.018 | *i* | 1m0-08 | 2015-05-07 | 2457150.207 | 19.335 0.128 | *i* | 1m0-13 |
| 2015-04-09 | 2457121.891 | 17.730 0.046 | *i* | 1m0-03 | 2015-05-10 | 2457152.616 | 19.063 0.062 | *i* | 1m0-08 |
| 2015-04-11 | 2457123.909 | 17.591 0.062 | *i* | 1m0-03 | 2015-05-11 | 2457154.219 | 19.676 0.413 | *i* | 1m0-13 |
| 2015-04-12 | 2457125.234 | 17.743 0.099 | *i* | 1m0-12 | 2015-05-12 | 2457154.867 | 18.971 0.018 | *i* | 1m0-11 |
| 2015-04-13 | 2457126.233 | 18.008 0.051 | *i* | 1m0-12 | 2015-09-06 | 2457272.104 | 20.334 0.277 | *i* | 2m0 |
| 2015-04-15 | 2457127.877 | 17.942 0.029 | *i* | 1m0-03 | 2015-09-06 | 2457272.107 | 20.577 0.318 | *i* | 2m0 |
| 2015-04-15 | 2457128.250 | 17.985 0.058 | *i* | 1m0-10 | 2015-09-10 | 2457276.126 | 20.527 0.107 | *i* | 2m0 |
| 2015-04-16 | 2457129.242 | 18.271 0.033 | *i* | 1m0-12 | 2015-10-13 | 2457309.093 | 20.945 0.087 | *i* | 2m0 |

(a) Data have not been corrected for extinction
(b) *Swift* Telescope; LSQ (La Silla Quest, Chile); 1m0-08 (McDonald Observatory, USA); 1m0-10, 1m0-12, 1m0-13 (Sutherland, South Africa), 1m0-04, 1m0-05, 1m0-09 (Cerro Tololo, Chile); 1m0-03, 1m0-11 (Siding Spring, Australia).

**Table D1:** LSQ14gv: Photometric Data

| Date | JD | mag[(a)] | Filter | telescope[(b)] | Date | JD | mag[(a)] | Filter | telescope[(b)] |
|---|---|---|---|---|---|---|---|---|---|
| 2014-01-25 | 2456682.596 | 18.119 0.069 | B | 1m0-10 | 2014-01-29 | 2456686.810 | 18.071 0.012 | g + r | LSQ |
| 2014-02-01 | 2456689.907 | 18.312 0.029 | B | 1m0-08 | 2014-01-29 | 2456686.847 | 18.078 0.012 | g + r | LSQ |
| 2014-02-04 | 2456693.365 | 18.485 0.046 | B | 1m0-13 | 2014-01-31 | 2456688.830 | 18.059 0.118 | g + r | LSQ |
| 2014-02-07 | 2456696.070 | 18.749 0.018 | B | 1m0-03 | 2014-02-02 | 2456690.832 | 17.949 0.170 | g + r | LSQ |
| 2014-02-08 | 2456697.011 | 18.799 0.023 | B | 1m0-11 | 2014-02-26 | 2456714.572 | 18.736 0.025 | g + r | LSQ |
| 2014-02-11 | 2456700.337 | 18.896 0.041 | B | 1m0-10 | 2014-02-26 | 2456714.654 | 18.735 0.018 | g + r | LSQ |
| 2014-02-26 | 2456715.424 | 19.770 0.096 | B | 1m0-10 | 2014-02-28 | 2456716.586 | 18.747 0.022 | g + r | LSQ |
| 2014-03-09 | 2456726.295 | 20.001 0.163 | B | 1m0-12 | 2014-02-28 | 2456716.669 | 18.757 0.018 | g + r | LSQ |
| 2014-03-27 | 2456744.231 | 20.760 0.154 | B | 1m0-13 | 2014-03-02 | 2456718.594 | 18.879 0.025 | g + r | LSQ |
| 2014-04-02 | 2456750.132 | 20.811 0.199 | B | 1m0-11 | 2014-03-02 | 2456718.679 | 18.798 0.020 | g + r | LSQ |
| 2014-04-19 | 2456767.256 | 21.168 0.187 | B | 1m0-13 | 2014-03-04 | 2456720.540 | 18.809 0.020 | g + r | LSQ |
| 2014-01-25 | 2456682.608 | 17.851 0.037 | g | 1m0-10 | 2014-03-04 | 2456720.625 | 18.849 0.020 | g + r | LSQ |
| 2014-02-01 | 2456689.916 | 18.101 0.035 | g | 1m0-08 | 2014-03-06 | 2456722.564 | 18.854 0.021 | g + r | LSQ |
| 2014-02-04 | 2456693.375 | 18.178 0.031 | g | 1m0-13 | 2014-03-06 | 2456722.649 | 18.913 0.018 | g + r | LSQ |
| 2014-02-07 | 2456696.081 | 18.199 0.015 | g | 1m0-03 | 2014-03-08 | 2456724.562 | 18.958 0.023 | g + r | LSQ |
| 2014-02-08 | 2456697.022 | 18.264 0.028 | g | 1m0-11 | 2014-03-08 | 2456724.647 | 18.915 0.020 | g + r | LSQ |
| 2014-02-11 | 2456700.347 | 18.364 0.015 | g | 1m0-10 | 2014-03-10 | 2456726.565 | 18.944 0.026 | g + r | LSQ |
| 2014-02-15 | 2456704.360 | 18.538 0.150 | g | 1m0-13 | 2014-03-10 | 2456726.648 | 18.911 0.026 | g + r | LSQ |
| 2014-02-20 | 2456709.318 | 18.769 0.022 | g | 1m0-13 | 2014-03-12 | 2456728.559 | 19.015 0.033 | g + r | LSQ |
| 2014-02-21 | 2456710.338 | 18.726 0.011 | g | 1m0-13 | 2014-03-12 | 2456728.643 | 18.957 0.029 | g + r | LSQ |
| 2014-02-26 | 2456715.433 | 18.784 0.052 | g | 1m0-10 | 2014-03-14 | 2456730.542 | 18.978 0.078 | g + r | LSQ |
| 2014-03-01 | 2456718.455 | 19.115 0.017 | g | 1m0-13 | 2014-03-14 | 2456730.628 | 18.973 0.060 | g + r | LSQ |
| 2014-03-05 | 2456722.269 | 19.153 0.080 | g | 1m0-12 | 2014-03-18 | 2456734.556 | 19.109 0.064 | g + r | LSQ |
| 2014-03-06 | 2456723.268 | 19.158 0.021 | g | 1m0-13 | 2014-03-18 | 2456734.640 | 19.122 0.057 | g + r | LSQ |
| 2014-03-09 | 2456726.264 | 19.233 0.194 | g | 1m0-10 | 2014-03-20 | 2456736.557 | 19.290 0.048 | g + r | LSQ |
| 2014-03-29 | 2456746.273 | 19.808 0.021 | g | 1m0-12 | 2014-03-20 | 2456736.642 | 19.277 0.062 | g + r | LSQ |
| 2014-04-07 | 2456755.274 | 20.477 0.023 | g | 1m0-10 | 2014-03-22 | 2456738.559 | 19.313 0.027 | g + r | LSQ |
| 2014-04-19 | 2456767.264 | 21.281 0.030 | g | 1m0-13 | 2014-03-22 | 2456738.642 | 19.181 0.033 | g + r | LSQ |
| 2014-01-17 | 2456674.801 | 18.270 0.060 | g + r | LSQ | 2014-03-24 | 2456740.549 | 19.298 0.026 | g + r | LSQ |
| 2014-01-17 | 2456674.838 | 18.330 0.060 | g + r | LSQ | 2014-03-24 | 2456740.631 | 19.409 0.026 | g + r | LSQ |
| 2014-01-21 | 2456678.642 | 17.930 0.040 | g + r | LSQ | 2014-03-26 | 2456742.548 | 19.369 0.027 | g + r | LSQ |
| 2014-01-21 | 2456678.738 | 18.160 0.040 | g + r | LSQ | 2014-03-26 | 2456742.633 | 19.419 0.025 | g + r | LSQ |
| 2014-01-25 | 2456682.602 | 17.909 0.010 | V | 1m0-10 | 2014-03-28 | 2456744.545 | 19.487 0.030 | g + r | LSQ |
| 2014-02-01 | 2456689.912 | 17.843 0.086 | V | 1m0-08 | 2014-03-28 | 2456744.630 | 19.492 0.035 | g + r | LSQ |
| 2014-02-04 | 2456693.370 | 18.007 0.100 | V | 1m0-13 | 2014-03-30 | 2456746.537 | 19.577 0.036 | g + r | LSQ |
| 2014-02-07 | 2456696.076 | 18.181 0.016 | V | 1m0-03 | 2014-03-30 | 2456746.621 | 19.677 0.039 | g + r | LSQ |
| 2014-02-08 | 2456697.018 | 18.189 0.038 | V | 1m0-11 | 2014-04-03 | 2456750.531 | 19.748 0.036 | g + r | LSQ |
| 2014-02-11 | 2456700.342 | 18.339 0.029 | V | 1m0-10 | 2014-04-03 | 2456750.614 | 19.781 0.044 | g + r | LSQ |
| 2014-02-15 | 2456704.356 | 18.172 0.064 | V | 1m0-13 | 2014-04-05 | 2456752.530 | 19.784 0.071 | g + r | LSQ |
| 2014-02-21 | 2456710.334 | 18.428 0.070 | V | 1m0-13 | 2014-04-05 | 2456752.615 | 19.937 0.046 | g + r | LSQ |
| 2014-02-26 | 2456715.430 | 18.698 0.054 | V | 1m0-10 | 2014-04-07 | 2456754.519 | 19.955 0.057 | g + r | LSQ |
| 2014-03-01 | 2456718.449 | 18.709 0.023 | V | 1m0-13 | 2014-04-07 | 2456754.599 | 19.956 0.070 | g + r | LSQ |
| 2014-03-09 | 2456726.301 | 18.756 0.152 | V | 1m0-12 | 2014-04-09 | 2456756.528 | 19.954 0.066 | g + r | LSQ |
| 2014-03-12 | 2456729.258 | 18.993 0.063 | V | 1m0-13 | 2014-04-09 | 2456756.611 | 20.018 0.072 | g + r | LSQ |
| 2014-03-27 | 2456744.243 | 19.402 0.159 | V | 1m0-13 | 2014-04-11 | 2456758.514 | 20.723 0.444 | g + r | LSQ |
| 2014-03-28 | 2456745.365 | 19.389 0.137 | V | 1m0-12 | 2014-04-11 | 2456758.598 | 20.088 0.220 | g + r | LSQ |
| 2014-04-02 | 2456750.112 | 19.656 0.065 | V | 1m0-11 | 2014-04-13 | 2456760.524 | 20.393 0.216 | g + r | LSQ |
| 2014-04-19 | 2456767.259 | 21.490 0.162 | V | 1m0-13 | 2014-04-13 | 2456760.607 | 20.382 0.198 | g + r | LSQ |
| 2014-01-09 | 2456666.682 | < 23.629 | V | 1m0-30 | 2014-04-15 | 2456762.523 | 20.973 0.332 | g + r | LSQ |
| 2014-01-13 | 2456670.673 | < 24.207 | V | 1m0-30 | 2014-04-15 | 2456762.608 | 20.657 0.253 | g + r | LSQ |
| 2014-01-17 | 2456674.801 | 18.209 0.041 | g + r | LSQ | 2014-04-17 | 2456764.519 | 21.754 0.417 | g + r | LSQ |
| 2014-01-17 | 2456674.838 | 18.377 0.045 | g + r | LSQ | 2014-04-17 | 2456764.602 | 21.569 0.394 | g + r | LSQ |
| 2014-01-21 | 2456678.642 | 17.933 0.022 | g + r | LSQ | 2014-04-19 | 2456766.513 | 21.981 0.250 | g + r | LSQ |
| 2014-01-21 | 2456678.738 | 18.034 0.022 | g + r | LSQ | 2014-04-19 | 2456766.596 | 21.468 0.253 | g + r | LSQ |
| 2014-01-23 | 2456680.638 | 18.027 0.014 | g + r | LSQ | 2014-04-21 | 2456768.506 | 21.753 0.210 | g + r | LSQ |
| 2014-01-23 | 2456680.722 | 18.351 0.027 | g + r | LSQ | 2014-04-21 | 2456768.591 | 21.552 0.188 | g + r | LSQ |
| 2014-01-25 | 2456682.644 | 18.168 0.114 | g + r | LSQ | 2014-04-23 | 2456770.504 | 21.886 0.260 | g + r | LSQ |
| 2014-01-25 | 2456682.729 | 17.898 0.138 | g + r | LSQ | 2014-04-23 | 2456770.587 | 22.035 0.278 | g + r | LSQ |
| 2014-01-27 | 2456684.710 | 17.971 0.011 | g + r | LSQ | 2014-04-25 | 2456772.539 | 22.021 0.248 | g + r | LSQ |
| 2014-01-27 | 2456684.794 | 17.977 0.013 | g + r | LSQ | 2014-04-25 | 2456772.623 | 22.420 0.368 | g + r | LSQ |

(a) Data have not been corrected for extinction
(b) *Swift* Telescope; LSQ (La Silla Quest, Chile); 1m0-08 (McDonald Observatory, USA); 1m0-10, 1m0-12, 1m0-13 (Sutherland, South Africa), 1m0-04, 1m0-05, 1m0-09 (Cerro Tololo, Chile); 1m0-03, 1m0-11 (Siding Spring, Australia).

**Table D1:** LSQ14gv: Photometric Data

| Date | JD | mag[(a)] | Filter | telescope[(b)] | Date | JD | mag[(a)] | Filter | telescope[(b)] |
|---|---|---|---|---|---|---|---|---|---|
| 2014-01-25 | 2456682.612 | 17.843 0.068 | $r$ | 1m0-10 | 2014-01-25 | 2456682.614 | 17.947 0.040 | $i$ | 1m0-10 |
| 2014-02-01 | 2456689.921 | 18.085 0.029 | $r$ | 1m0-08 | 2014-02-01 | 2456689.925 | 17.865 0.092 | $i$ | 1m0-08 |
| 2014-02-04 | 2456693.381 | 17.891 0.047 | $r$ | 1m0-13 | 2014-02-04 | 2456693.387 | 18.000 0.090 | $i$ | 1m0-13 |
| 2014-02-07 | 2456696.088 | 17.955 0.017 | $r$ | 1m0-03 | 2014-02-07 | 2456696.092 | 18.079 0.018 | $i$ | 1m0-03 |
| 2014-02-08 | 2456697.029 | 17.987 0.012 | $r$ | 1m0-11 | 2014-02-08 | 2456697.033 | 17.972 0.041 | $i$ | 1m0-11 |
| 2014-02-11 | 2456700.354 | 17.878 0.041 | $r$ | 1m0-10 | 2014-02-11 | 2456700.358 | 17.982 0.036 | $i$ | 1m0-10 |
| 2014-02-15 | 2456704.367 | 17.958 0.037 | $r$ | 1m0-13 | 2014-02-15 | 2456704.370 | 18.155 0.109 | $i$ | 1m0-13 |
| 2014-02-20 | 2456709.327 | 18.189 0.066 | $r$ | 1m0-13 | 2014-02-20 | 2456709.331 | 18.164 0.093 | $i$ | 1m0-13 |
| 2014-02-21 | 2456710.346 | 18.293 0.036 | $r$ | 1m0-13 | 2014-02-21 | 2456710.351 | 18.287 0.125 | $i$ | 1m0-13 |
| 2014-03-01 | 2456718.463 | 18.491 0.056 | $r$ | 1m0-13 | 2014-02-26 | 2456715.448 | 18.359 0.052 | $i$ | 1m0-10 |
| 2014-03-05 | 2456722.280 | 18.322 0.059 | $r$ | 1m0-12 | 2014-03-01 | 2456718.468 | 18.392 0.084 | $i$ | 1m0-13 |
| 2014-03-06 | 2456723.275 | 18.454 0.045 | $r$ | 1m0-13 | 2014-03-05 | 2456722.283 | 18.340 0.066 | $i$ | 1m0-12 |
| 2014-03-09 | 2456726.296 | 18.431 0.154 | $r$ | 1m0-10 | 2014-03-06 | 2456723.280 | 18.369 0.059 | $i$ | 1m0-13 |
| 2014-03-29 | 2456746.282 | 18.812 0.046 | $r$ | 1m0-12 | 2014-03-09 | 2456726.314 | 18.470 0.163 | $i$ | 1m0-10 |
| 2014-04-06 | 2456754.263 | 19.290 0.105 | $r$ | 1m0-10 | 2014-03-29 | 2456746.287 | 18.826 0.060 | $i$ | 1m0-12 |
| 2014-04-07 | 2456755.283 | 19.240 0.087 | $r$ | 1m0-10 | 2014-04-06 | 2456754.267 | 19.316 0.107 | $i$ | 1m0-10 |
| 2014-04-09 | 2456757.258 | 19.145 0.110 | $r$ | 1m0-12 | 2014-04-07 | 2456755.289 | 19.365 0.081 | $i$ | 1m0-10 |
| 2014-04-19 | 2456767.275 | 20.422 0.297 | $r$ | 1m0-13 | 2014-04-09 | 2456757.266 | 19.638 0.077 | $i$ | 1m0-12 |

(a) Data have not been corrected for extinction
(b) *Swift* Telescope; LSQ (La Silla Quest, Chile); 1m0-08 (McDonald Observatory, USA); 1m0-10, 1m0-12, 1m0-13 (Sutherland, South Africa), 1m0-04, 1m0-05, 1m0-09 (Cerro Tololo, Chile); 1m0-03, 1m0-11 (Siding Spring, Australia).

**Table D1:** LSQ13dpa: Photometric Data

| Date | JD | mag$^{(a)}$ | Filter | telescope$^{(b)}$ | Date | JD | mag$^{(a)}$ | Filter | telescope$^{(b)}$ |
|---|---|---|---|---|---|---|---|---|---|
| 2013-12-20 | 2456646.752 | 18.355 0.065 | $B$ | 1m0-09 | 2014-04-16 | 2456764.104 | 19.929 0.227 | $g$ | 1m0-03 |
| 2013-12-21 | 2456648.196 | 18.161 0.145 | $B$ | 1m0-03 | 2014-04-17 | 2456764.684 | 19.566 0.048 | $g$ | 1m0-08 |
| 2013-12-30 | 2456657.024 | 18.361 0.016 | $B$ | 1m0-08 | 2014-04-19 | 2456767.276 | 19.980 0.051 | $g$ | 1m0-12 |
| 2014-01-01 | 2456658.994 | 18.781 0.130 | $B$ | 1m0-08 | 2014-04-21 | 2456769.067 | 19.979 0.013 | $g$ | 1m0-11 |
| 2014-01-13 | 2456671.244 | 18.984 0.117 | $B$ | 1m0-11 | 2014-04-23 | 2456770.907 | 20.018 0.087 | $g$ | 1m0-03 |
| 2014-01-17 | 2456675.238 | 19.008 0.141 | $B$ | 1m0-03 | 2014-04-24 | 2456772.323 | 20.379 0.049 | $g$ | 1m0-12 |
| 2014-01-20 | 2456678.234 | 19.194 0.048 | $B$ | 1m0-11 | 2014-04-25 | 2456772.957 | 20.050 0.030 | $g$ | 1m0-11 |
| 2014-01-22 | 2456679.608 | 19.292 0.131 | $B$ | 1m0-13 | 2014-04-28 | 2456776.226 | 20.449 0.213 | $g$ | 1m0-13 |
| 2014-01-28 | 2456686.072 | 19.371 0.146 | $B$ | 1m0-03 | 2014-04-28 | 2456776.323 | 20.751 0.059 | $g$ | 1m0-12 |
| 2014-02-03 | 2456692.416 | 19.439 0.073 | $B$ | 1m0-10 | 2014-05-12 | 2456790.223 | 21.090 0.033 | $g$ | 1m0-12 |
| 2014-02-07 | 2456696.118 | 19.692 0.180 | $B$ | 1m0-03 | 2014-05-17 | 2456794.973 | 20.984 0.105 | $g$ | 1m0-11 |
| 2014-02-08 | 2456697.039 | 19.570 0.106 | $B$ | 1m0-11 | 2014-05-20 | 2456797.954 | 20.530 0.211 | $g$ | 1m0-11 |
| 2014-02-08 | 2456697.055 | 19.516 0.053 | $B$ | 1m0-03 | 2014-05-21 | 2456798.927 | 21.229 0.139 | $g$ | 1m0-11 |
| 2014-02-23 | 2456711.965 | 19.596 0.040 | $B$ | 1m0-03 | 2014-05-29 | 2456806.855 | 20.945 0.123 | $g$ | 1m0-03 |
| 2014-02-23 | 2456711.979 | 19.326 0.137 | $B$ | 1m0-11 | 2014-06-07 | 2456816.238 | 20.950 0.076 | $g$ | 1m0-13 |
| 2014-03-05 | 2456722.493 | 19.742 0.069 | $B$ | 1m0-13 | 2013-12-14 | 2456640.700 | $< 22.000$ | $V$ | 1m0-30 |
| 2014-03-07 | 2456724.308 | 19.743 0.120 | $B$ | 1m0-13 | 2013-12-18 | 2456644.782 | 18.580 0.050 | $g+r$ | LSQ |
| 2014-04-04 | 2456752.150 | 20.449 0.142 | $B$ | 1m0-03 | 2013-12-22 | 2456648.813 | 18.320 0.050 | $g+r$ | LSQ |
| 2014-04-07 | 2456755.343 | 20.225 0.138 | $B$ | 1m0-10 | 2013-12-20 | 2456646.758 | 18.393 0.051 | $V$ | 1m0-09 |
| 2014-04-09 | 2456756.944 | 20.030 0.189 | $B$ | 1m0-11 | 2013-12-21 | 2456648.203 | 18.341 0.015 | $V$ | 1m0-03 |
| 2014-04-09 | 2456757.392 | 20.160 0.254 | $B$ | 1m0-13 | 2013-12-30 | 2456657.032 | 18.191 0.138 | $V$ | 1m0-08 |
| 2014-04-12 | 2456760.327 | 20.038 0.250 | $B$ | 1m0-13 | 2014-01-01 | 2456658.999 | 18.454 0.141 | $V$ | 1m0-08 |
| 2014-04-17 | 2456764.672 | 20.463 0.184 | $B$ | 1m0-08 | 2014-01-13 | 2456671.237 | 18.426 0.131 | $V$ | 1m0-03 |
| 2014-04-19 | 2456767.264 | 21.172 0.250 | $B$ | 1m0-12 | 2014-01-13 | 2456671.250 | 18.228 0.130 | $V$ | 1m0-11 |
| 2014-04-21 | 2456769.052 | 20.992 0.121 | $B$ | 1m0-11 | 2014-01-15 | 2456672.608 | 18.336 0.025 | $V$ | 1m0-10 |
| 2014-04-23 | 2456770.892 | 20.924 0.061 | $B$ | 1m0-03 | 2014-01-17 | 2456675.224 | 18.252 0.148 | $V$ | 1m0-11 |
| 2014-04-24 | 2456772.308 | 20.630 0.087 | $B$ | 1m0-12 | 2014-01-17 | 2456675.245 | 18.157 0.057 | $V$ | 1m0-03 |
| 2014-04-25 | 2456772.942 | 21.079 0.061 | $B$ | 1m0-11 | 2014-01-20 | 2456678.241 | 18.376 0.011 | $V$ | 1m0-11 |
| 2014-04-28 | 2456776.205 | 21.754 0.330 | $B$ | 1m0-13 | 2014-01-22 | 2456679.612 | 18.272 0.131 | $V$ | 1m0-13 |
| 2014-04-28 | 2456776.306 | 21.381 0.216 | $B$ | 1m0-12 | 2014-01-28 | 2456686.076 | 18.377 0.141 | $V$ | 1m0-03 |
| 2014-05-12 | 2456790.208 | 21.325 0.077 | $B$ | 1m0-12 | 2014-02-03 | 2456692.424 | 18.419 0.035 | $V$ | 1m0-10 |
| 2014-05-17 | 2456794.956 | 21.272 0.257 | $B$ | 1m0-11 | 2014-02-08 | 2456697.046 | 18.398 0.129 | $V$ | 1m0-11 |
| 2014-05-21 | 2456798.910 | 21.877 0.414 | $B$ | 1m0-11 | 2014-02-08 | 2456697.061 | 18.407 0.130 | $V$ | 1m0-03 |
| 2014-06-07 | 2456816.221 | 21.703 0.238 | $B$ | 1m0-13 | 2014-02-23 | 2456711.989 | 18.408 0.135 | $V$ | 1m0-11 |
| 2013-12-20 | 2456646.763 | 18.389 0.059 | $g$ | 1m0-09 | 2014-03-06 | 2456722.503 | 18.386 0.129 | $V$ | 1m0-13 |
| 2013-12-21 | 2456648.208 | 18.259 0.024 | $g$ | 1m0-03 | 2014-03-07 | 2456724.322 | 18.458 0.090 | $V$ | 1m0-13 |
| 2013-12-30 | 2456657.008 | 18.161 0.022 | $g$ | 1m0-08 | 2014-04-07 | 2456755.353 | 18.704 0.130 | $V$ | 1m0-10 |
| 2014-01-01 | 2456658.957 | 18.138 0.022 | $g$ | 1m0-08 | 2014-04-07 | 2456755.372 | 18.507 0.015 | $V$ | 1m0-12 |
| 2014-01-07 | 2456665.009 | 18.343 0.036 | $g$ | 1m0-08 | 2014-04-09 | 2456756.952 | 18.631 0.010 | $V$ | 1m0-11 |
| 2014-01-15 | 2456672.593 | 18.623 0.016 | $g$ | 1m0-13 | 2014-04-09 | 2456757.401 | 18.659 0.017 | $V$ | 1m0-13 |
| 2014-01-17 | 2456675.022 | 18.700 0.072 | $g$ | 1m0-08 | 2014-04-17 | 2456764.678 | 19.033 0.018 | $V$ | 1m0-08 |
| 2014-01-25 | 2456682.515 | 18.767 0.018 | $g$ | 1m0-12 | 2014-04-19 | 2456767.271 | 19.014 0.136 | $V$ | 1m0-12 |
| 2014-01-31 | 2456689.407 | 18.660 0.161 | $g$ | 1m0-10 | 2014-04-21 | 2456769.061 | 19.311 0.022 | $V$ | 1m0-11 |
| 2014-02-01 | 2456689.558 | 18.778 0.160 | $g$ | 1m0-12 | 2014-04-23 | 2456770.900 | 19.367 0.081 | $V$ | 1m0-03 |
| 2014-02-03 | 2456692.013 | 18.701 0.156 | $g$ | 1m0-11 | 2014-04-24 | 2456772.317 | 19.610 0.055 | $V$ | 1m0-12 |
| 2014-02-03 | 2456692.429 | 18.689 0.152 | $g$ | 1m0-12 | 2014-04-25 | 2456772.952 | 19.534 0.181 | $V$ | 1m0-11 |
| 2014-02-07 | 2456696.216 | 18.839 0.153 | $g$ | 1m0-11 | 2014-04-28 | 2456776.216 | 19.847 0.160 | $V$ | 1m0-13 |
| 2014-02-08 | 2456697.029 | 18.740 0.050 | $g$ | 1m0-03 | 2014-04-28 | 2456776.317 | 20.030 0.201 | $V$ | 1m0-12 |
| 2014-02-11 | 2456700.364 | 18.831 0.111 | $g$ | 1m0-10 | 2014-05-12 | 2456790.217 | 20.441 0.117 | $V$ | 1m0-12 |
| 2014-02-17 | 2456705.988 | 18.980 0.087 | $g$ | 1m0-03 | 2014-05-17 | 2456794.967 | 20.525 0.092 | $V$ | 1m0-11 |
| 2014-02-20 | 2456709.325 | 18.695 0.020 | $g$ | 1m0-12 | 2014-05-21 | 2456798.920 | 20.462 0.166 | $V$ | 1m0-11 |
| 2014-02-24 | 2456713.367 | 18.870 0.022 | $g$ | 1m0-13 | 2014-05-29 | 2456806.849 | 20.339 0.157 | $V$ | 1m0-03 |
| 2014-03-05 | 2456722.310 | 18.864 0.031 | $g$ | 1m0-13 | 2014-06-07 | 2456816.233 | 20.639 0.252 | $V$ | 1m0-13 |
| 2014-03-07 | 2456724.294 | 18.864 0.088 | $g$ | 1m0-12 | 2013-12-18 | 2456644.782 | 18.497 0.036 | $g+r$ | LSQ |
| 2014-03-12 | 2456729.283 | 18.839 0.049 | $g$ | 1m0-13 | 2013-12-18 | 2456644.830 | 18.456 0.028 | $g+r$ | LSQ |
| 2014-03-27 | 2456743.609 | 19.009 0.154 | $g$ | 1m0-08 | 2013-12-22 | 2456648.765 | 18.352 0.028 | $g+r$ | LSQ |
| 2014-04-07 | 2456755.320 | 19.128 0.053 | $g$ | 1m0-10 | 2013-12-22 | 2456648.813 | 18.296 0.029 | $g+r$ | LSQ |
| 2014-04-10 | 2456758.262 | 19.283 0.011 | $g$ | 1m0-12 | 2013-12-30 | 2456656.857 | 18.281 0.021 | $g+r$ | LSQ |
| 2014-04-11 | 2456759.388 | 19.394 0.157 | $g$ | 1m0-13 | 2013-12-30 | 2456656.862 | 18.307 0.021 | $g+r$ | LSQ |
| 2014-04-11 | 2456759.426 | 19.028 0.059 | $g$ | 1m0-12 | 2014-01-03 | 2456660.846 | 18.333 0.014 | $g+r$ | LSQ |

(a) Data have not been corrected for extinction
(b) *Swift* Telescope; LSQ (La Silla Quest, Chile); 1m0-08 (McDonald Observatory, USA); 1m0-10, 1m0-12, 1m0-13 (Sutherland, South Africa), 1m0-04, 1m0-05, 1m0-09 (Cerro Tololo, Chile); 1m0-03, 1m0-11 (Siding Spring, Australia).

**Table D1:** LSQ13dpa: Photometric Data

| Date | JD | mag[(a)] | Filter | telescope[(b)] | Date | JD | mag[(a)] | Filter | telescope[(b)] |
|---|---|---|---|---|---|---|---|---|---|
| 2014-01-05 | 2456662.771 | 18.391 0.015 | $g + r$ | LSQ | 2014-04-19 | 2456767.285 | 18.475 0.048 | $r$ | 1m0-12 |
| 2014-01-05 | 2456662.822 | 18.339 0.015 | $g + r$ | LSQ | 2014-04-21 | 2456769.076 | 18.756 0.028 | $r$ | 1m0-11 |
| 2014-01-07 | 2456664.711 | 18.374 0.016 | $g + r$ | LSQ | 2014-04-23 | 2456770.915 | 18.620 0.028 | $r$ | 1m0-03 |
| 2014-01-07 | 2456664.796 | 18.391 0.014 | $g + r$ | LSQ | 2014-04-24 | 2456772.332 | 19.080 0.066 | $r$ | 1m0-12 |
| 2014-01-09 | 2456666.705 | 18.445 0.018 | $g + r$ | LSQ | 2014-04-25 | 2456772.965 | 18.827 0.027 | $r$ | 1m0-11 |
| 2014-01-09 | 2456666.799 | 18.412 0.019 | $g + r$ | LSQ | 2014-04-28 | 2456776.232 | 19.074 0.047 | $r$ | 1m0-13 |
| 2014-02-19 | 2456707.784 | 18.561 0.027 | $g + r$ | LSQ | 2014-04-28 | 2456776.332 | 19.480 0.326 | $r$ | 1m0-12 |
| 2014-02-19 | 2456707.841 | 18.526 0.033 | $g + r$ | LSQ | 2014-05-12 | 2456790.232 | 19.966 0.119 | $r$ | 1m0-12 |
| 2014-02-21 | 2456709.789 | 18.510 0.020 | $g + r$ | LSQ | 2014-05-17 | 2456794.983 | 19.803 0.125 | $r$ | 1m0-11 |
| 2014-02-21 | 2456709.869 | 18.536 0.024 | $g + r$ | LSQ | 2014-05-21 | 2456798.937 | 19.839 0.131 | $r$ | 1m0-11 |
| 2014-03-01 | 2456717.708 | 18.621 0.020 | $g + r$ | LSQ | 2014-05-29 | 2456806.864 | 19.865 0.012 | $r$ | 1m0-03 |
| 2014-03-03 | 2456719.702 | 18.529 0.016 | $g + r$ | LSQ | 2014-06-07 | 2456816.247 | 20.161 0.023 | $r$ | 1m0-13 |
| 2014-03-03 | 2456719.785 | 18.508 0.016 | $g + r$ | LSQ | 2014-06-27 | 2456836.202 | 20.221 0.268 | $r$ | 1m0-13 |
| 2014-03-05 | 2456721.697 | 18.538 0.016 | $g + r$ | LSQ | 2014-06-27 | 2456836.281 | 20.118 0.177 | $r$ | 1m0-10 |
| 2014-03-05 | 2456721.781 | 18.510 0.016 | $g + r$ | LSQ | 2013-12-20 | 2456646.774 | 18.657 0.086 | $i$ | 1m0-09 |
| 2014-03-13 | 2456729.587 | 18.460 0.027 | $g + r$ | LSQ | 2013-12-21 | 2456648.218 | 18.591 0.120 | $i$ | 1m0-03 |
| 2014-03-13 | 2456729.671 | 18.497 0.025 | $g + r$ | LSQ | 2013-12-30 | 2456657.019 | 18.242 0.097 | $i$ | 1m0-08 |
| 2014-03-21 | 2456737.653 | 18.519 0.020 | $g + r$ | LSQ | 2014-01-01 | 2456658.967 | 18.303 0.233 | $i$ | 1m0-08 |
| 2014-03-21 | 2456737.736 | 18.504 0.021 | $g + r$ | LSQ | 2014-01-03 | 2456661.021 | 18.256 0.029 | $i$ | 1m0-08 |
| 2014-03-23 | 2456739.624 | 18.546 0.016 | $g + r$ | LSQ | 2014-01-07 | 2456665.019 | 18.251 0.024 | $i$ | 1m0-08 |
| 2014-03-23 | 2456739.709 | 18.526 0.019 | $g + r$ | LSQ | 2014-01-15 | 2456672.604 | 18.324 0.079 | $i$ | 1m0-13 |
| 2014-03-25 | 2456741.614 | 18.591 0.017 | $g + r$ | LSQ | 2014-01-17 | 2456675.033 | 18.429 0.100 | $i$ | 1m0-08 |
| 2014-03-25 | 2456741.698 | 18.547 0.016 | $g + r$ | LSQ | 2014-01-21 | 2456679.082 | 18.165 0.026 | $i$ | 1m0-03 |
| 2014-12-16 | 2457007.764 | 21.492 0.261 | $g + r$ | LSQ | 2014-01-25 | 2456682.529 | 18.345 0.019 | $i$ | 1m0-12 |
| 2014-12-16 | 2457007.836 | 22.200 0.427 | $g + r$ | LSQ | 2014-02-03 | 2456692.026 | 18.208 0.111 | $i$ | 1m0-11 |
| 2013-12-20 | 2456646.770 | 18.501 0.044 | $r$ | 1m0-09 | 2014-02-03 | 2456692.442 | 18.105 0.122 | $i$ | 1m0-12 |
| 2013-12-21 | 2456648.214 | 18.241 0.061 | $r$ | 1m0-03 | 2014-02-07 | 2456696.231 | 18.174 0.067 | $i$ | 1m0-11 |
| 2013-12-30 | 2456657.015 | 18.046 0.015 | $r$ | 1m0-08 | 2014-02-08 | 2456697.037 | 18.078 0.060 | $i$ | 1m0-03 |
| 2014-01-01 | 2456658.964 | 17.917 0.109 | $r$ | 1m0-08 | 2014-02-11 | 2456700.376 | 18.289 0.044 | $i$ | 1m0-10 |
| 2014-01-03 | 2456661.017 | 18.055 0.026 | $r$ | 1m0-08 | 2014-02-17 | 2456706.000 | 18.107 0.221 | $i$ | 1m0-03 |
| 2014-01-07 | 2456665.016 | 18.113 0.031 | $r$ | 1m0-08 | 2014-02-20 | 2456709.337 | 18.047 0.033 | $i$ | 1m0-12 |
| 2014-01-15 | 2456672.600 | 18.202 0.048 | $r$ | 1m0-13 | 2014-02-24 | 2456713.380 | 18.185 0.025 | $i$ | 1m0-13 |
| 2014-01-17 | 2456675.029 | 18.110 0.070 | $r$ | 1m0-08 | 2014-03-05 | 2456722.323 | 18.009 0.012 | $i$ | 1m0-13 |
| 2014-01-25 | 2456682.524 | 18.226 0.026 | $r$ | 1m0-12 | 2014-03-07 | 2456724.319 | 18.167 0.033 | $i$ | 1m0-12 |
| 2014-02-03 | 2456692.439 | 17.959 0.050 | $r$ | 1m0-12 | 2014-03-12 | 2456729.297 | 18.081 0.014 | $i$ | 1m0-13 |
| 2014-02-07 | 2456696.226 | 18.177 0.028 | $r$ | 1m0-11 | 2014-03-27 | 2456743.620 | 18.180 0.026 | $i$ | 1m0-08 |
| 2014-02-08 | 2456697.032 | 18.025 0.042 | $r$ | 1m0-03 | 2014-04-07 | 2456755.334 | 18.430 0.110 | $i$ | 1m0-10 |
| 2014-02-11 | 2456700.372 | 18.211 0.025 | $r$ | 1m0-10 | 2014-04-09 | 2456756.878 | 18.101 0.113 | $i$ | 1m0-03 |
| 2014-02-17 | 2456705.995 | 18.051 0.193 | $r$ | 1m0-03 | 2014-04-10 | 2456758.276 | 18.357 0.031 | $i$ | 1m0-12 |
| 2014-02-20 | 2456709.334 | 18.057 0.112 | $r$ | 1m0-12 | 2014-04-11 | 2456759.440 | 18.190 0.064 | $i$ | 1m0-12 |
| 2014-02-24 | 2456713.375 | 18.089 0.059 | $r$ | 1m0-13 | 2014-04-17 | 2456764.698 | 18.458 0.132 | $i$ | 1m0-08 |
| 2014-03-05 | 2456722.318 | 18.026 0.011 | $r$ | 1m0-13 | 2014-04-19 | 2456767.290 | 18.504 0.071 | $i$ | 1m0-12 |
| 2014-03-07 | 2456724.318 | 18.106 0.015 | $r$ | 1m0-12 | 2014-04-21 | 2456769.081 | 18.763 0.031 | $i$ | 1m0-11 |
| 2014-03-12 | 2456729.292 | 18.077 0.038 | $r$ | 1m0-13 | 2014-04-23 | 2456770.920 | 18.798 0.028 | $i$ | 1m0-03 |
| 2014-03-27 | 2456743.614 | 17.998 0.103 | $r$ | 1m0-08 | 2014-04-24 | 2456772.337 | 19.099 0.103 | $i$ | 1m0-12 |
| 2014-04-07 | 2456755.329 | 18.423 0.095 | $r$ | 1m0-10 | 2014-04-25 | 2456772.971 | 19.049 0.159 | $i$ | 1m0-11 |
| 2014-04-10 | 2456758.271 | 18.149 0.073 | $r$ | 1m0-12 | 2014-04-28 | 2456776.237 | 19.070 0.373 | $i$ | 1m0-13 |
| 2014-04-11 | 2456759.435 | 18.099 0.146 | $r$ | 1m0-12 | 2014-05-12 | 2456790.236 | 19.852 0.202 | $i$ | 1m0-12 |
| 2014-04-16 | 2456764.110 | 18.811 0.073 | $r$ | 1m0-03 | 2014-05-17 | 2456794.987 | 19.981 0.050 | $i$ | 1m0-11 |
| 2014-04-17 | 2456764.693 | 18.574 0.102 | $r$ | 1m0-08 | 2014-05-21 | 2456798.941 | 20.042 0.094 | $i$ | 1m0-11 |

(a) Data have not been corrected for extinction

(b) *Swift* Telescope; LSQ (La Silla Quest, Chile); 1m0-08 (McDonald Observatory, USA); 1m0-10, 1m0-12, 1m0-13 (Sutherland, South Africa), 1m0-04, 1m0-05, 1m0-09 (Cerro Tololo, Chile); 1m0-03, 1m0-11 (Siding Spring, Australia).

**Table D2:** Slope Data

| SN | $M(V)$ * $\Delta M$ | $s50(V)$ $(V)$ | $\Delta$ s50(V) | $ph\_start$ | $ph\_stop$ $(V)$ | $M(R)$ $(V)$ | $\Delta M$ | s50$(R)$ $(R)$ | $\Delta s50(R)$ | $ph\_start$ | $ph\_stop$ $(R)$ | $M(I)$ $(R)$ | $\Delta M$ | $s50(I)$ $(I)$ | $\Delta s50(I)$ | $ph\_start$ | $ph\_stop$ | $(I)$ |
|---|---|---|---|---|---|---|---|---|---|---|---|---|---|---|---|---|---|---|
| 2013ai | 16.80 | 0.02 | 0.0209 | 0.0006 | 17.6 | 54.5 | 16.59 | 0.02 | 0.0129 | 0.0004 | 17.6 | 64.5 | 16.29 | 0.05 | 0.0112 | 0.0009 | 19.6 | 63.5 |
| 2013bu | 16.33 | 0.04 | 0.0053 | 0.0013 | 6.2 | 48.1 | 15.61 | 0.02 | 0.0014 | 0.0005 | 6.2 | 57.1 | 15.63 | 0.01 | -0.0027 | 0.0004 | 6.2 | 55.1 |
| 2013fs | 16.03 | 0.04 | 0.0158 | 0.0014 | 4.5 | 58.4 | 15.98 | 0.03 | 0.0075 | 0.0009 | 14.5 | 60.4 | 15.80 | 0.03 | 0.0065 | 0.0008 | 14.5 | 69.6 |
| LSQ13dpa | 18.31 | 0.03 | 0.0011 | 0.0011 | 5.5 | 54.4 | 18.05 | 0.07 | 0.0008 | 0.0017 | 14.3 | 66.6 | 18.36 | 0.07 | -0.0032 | 0.0017 | 14.3 | 63.3 |
| 2014cy | 15.81 | 0.04 | 0.0124 | 0.0012 | 5.4 | 61.1 | 15.83 | 0.03 | 0.0064 | 0.0008 | 0.8 | 61.1 | 15.97 | 0.02 | 0.0019 | 0.0007 | 5.4 | 61.1 |
| 2014dw | 15.55 | 0.03 | 0.0291 | 0.0009 | 14.2 | 54.1 | 15.63 | 0.02 | 0.0185 | 0.0006 | 11.6 | 63.8 | 15.59 | 0.03 | 0.0170 | 0.0007 | 14.2 | 63.8 |
| LSQ14gv | 17.71 | 0.04 | 0.0239 | 0.0012 | 7.8 | 51.8 | 17.65 | 0.07 | 0.0157 | 0.0019 | 7.8 | 71.5 | 17.71 | 0.04 | 0.0148 | 0.0012 | 7.8 | 71.5 |
| ASASSN-14dq | 15.69 | 0.02 | 0.0170 | 0.0006 | 5.5 | 55.0 | 15.67 | 0.02 | 0.0101 | 0.0005 | 9.1 | 66.9 | 15.80 | 0.02 | 0.0096 | 0.0004 | 9.1 | 66.9 |
| ASASSN-14gm | 14.83 | 0.02 | 0.0026 | 0.0005 | 7.2 | 62.1 | 14.74 | 0.02 | 0.0003 | 0.0005 | 7.2 | 62.1 | 14.90 | 0.01 | -0.0034 | 0.0004 | 7.2 | 62.1 |
| ASASSN-14kg | 15.67 | 0.04 | 0.0223 | 0.0012 | 18.8 | 51.7 | 15.73 | 0.07 | 0.0143 | 0.0016 | 21.6 | 68.7 | 15.80 | 0.07 | 0.0138 | 0.0015 | 23.8 | 68.7 |
| ASASSN-14ha | 14.89 | 0.01 | 0.0070 | 0.0005 | 3.1 | 60.4 | 15.00 | 0.02 | -0.0005 | 0.0006 | 3.1 | 72.2 | 15.19 | 0.01 | -0.0043 | 0.0005 | 1.8 | 72.2 |
| 2015W | 16.40 | 0.03 | 0.0247 | 0.0010 | 10.4 | 54.9 | 16.37 | 0.04 | 0.0127 | 0.0011 | 9.8 | 65.9 | 16.29 | 0.05 | 0.0145 | 0.0013 | 12.4 | 64.3 |
| 2013ab | 14.64 | 0.02 | 0.0149 | 0.0006 | 8.8 | 53.4 | 14.63 | 0.02 | 0.0075 | 0.0005 | 8.3 | 66.3 | 14.58 | 0.01 | 0.0033 | 0.0003 | 11.3 | 66.3 |
| 2013by | 12.87 | 0.02 | 0.0290 | 0.0007 | 11.8 | 48.8 | 12.97 | 0.02 | 0.0176 | 0.0005 | 7.9 | 61.6 | 12.91 | 0.03 | 0.0194 | 0.0012 | 7.5 | 51.8 |
| 2013ej | 12.14 | 0.03 | 0.0236 | 0.0009 | 14.9 | 51.4 | 12.02 | 0.04 | 0.0161 | 0.0011 | 14.9 | 66.3 | 11.97 | 0.06 | 0.0124 | 0.0017 | 14.9 | 63.3 |
| 2014G | 13.89 | 0.03 | 0.0335 | 0.0008 | 14.4 | 53.6 | 13.97 | 0.03 | 0.0233 | 0.0009 | 14.4 | 65.3 | 13.90 | 0.05 | 0.0227 | 0.0013 | 14.4 | 65.3 |
| 1986L | 13.53 | 0.05 | 0.0209 | 0.0015 | 8.2 | 62.3 | – | – | – | – | – | – | – | – | – | – | – | – |
| 1987A | 4.57 | 0.01 | -0.0189 | 0.0004 | 3.5 | 34.5 | 4.22 | 0.01 | -0.0299 | 0.0002 | 6.5 | 56.5 | 3.99 | 0.02 | -0.0344 | 0.0008 | 4.6 | 49.4 |
| 1979C | 11.73 | 0.04 | 0.0282 | 0.0012 | 16.7 | 50.7 | – | – | – | – | – | – | – | – | – | – | – | – |
| 1990E | 15.73 | 0.02 | -0.0082 | 0.0013 | 7.6 | 27.3 | – | – | – | – | – | – | – | – | – | – | – | – |
| 1991al | 16.35 | 0.03 | 0.0151 | 0.0008 | 15.3 | 56.1 | 16.10 | 0.02 | 0.0113 | 0.0006 | 12.2 | 65.1 | 16.01 | 0.03 | 0.0085 | 0.0008 | 15.3 | 65.1 |
| 1992af | 17.11 | 0.07 | 0.0047 | 0.0029 | 14.3 | 40.3 | – | – | – | – | – | – | 15.66 | 0.34 | 0.0239 | 0.0061 | 16.1 | 81.1 |
| 1992ba | 15.13 | 0.03 | 0.0072 | 0.0007 | 16.3 | 68.3 | – | – | – | – | – | – | – | – | – | – | – | – |
| 1993A | – | – | – | – | – | – | – | – | – | – | – | – | 18.88 | 0.06 | 0.0008 | 0.0015 | 16.7 | 77.7 |
| 1993K | – | – | – | – | – | – | 14.82 | inf | 0.0151 | inf | 12.6 | 43.5 | – | – | – | – | – | – |
| 1993S | – | – | – | – | – | – | – | – | – | – | – | – | 17.60 | 0.06 | 0.0129 | 0.0013 | 13.4 | 57.4 |
| 1999ca | – | – | – | – | – | – | – | – | – | – | – | – | 14.88 | 0.04 | 0.0169 | 0.0008 | 28.0 | 63.0 |
| 1999cr | 17.95 | 0.02 | 0.0138 | 0.0005 | 9.3 | 54.0 | 17.69 | 0.01 | 0.0091 | 0.0003 | 9.3 | 55.3 | 17.46 | 0.02 | 0.0069 | 0.0005 | 10.4 | 57.2 |
| 1999em | 13.80 | 0.01 | 0.0032 | 0.0004 | 5.4 | 55.2 | 13.64 | 0.01 | -0.0016 | 0.0003 | 8.3 | 70.3 | 13.64 | 0.01 | -0.0074 | 0.0003 | 5.3 | 62.1 |
| 1999gi | 14.53 | 0.03 | 0.0064 | 0.0006 | 11.8 | 71.7 | 14.39 | 0.04 | -0.0003 | 0.0013 | 4.1 | 60.4 | 14.14 | 0.01 | -0.0031 | 0.0004 | 9.8 | 63.6 |
| 1999br | 17.56 | 0.02 | 0.0004 | 0.0006 | 7.0 | 59.0 | 17.35 | 0.01 | -0.0053 | 0.0004 | 8.5 | 57.5 | 17.26 | 0.02 | -0.0112 | 0.0005 | 7.7 | 67.5 |
| 2000dc | 15.78 | 0.04 | 0.0257 | 0.0014 | 11.2 | 50.2 | 15.61 | 0.02 | 0.0153 | 0.0007 | 11.2 | 58.2 | 15.36 | 0.02 | 0.0128 | 0.0005 | 11.2 | 58.2 |
| 2001fa | 15.62 | 0.07 | 0.0513 | 0.0032 | 8.4 | 33.3 | 15.84 | 0.13 | 0.0282 | 0.0035 | 11.4 | 80.2 | 15.72 | 0.08 | 0.0248 | 0.0033 | 7.3 | 52.3 |
| 2001do | 15.54 | 0.03 | 0.0246 | 0.0008 | 8.0 | 52.9 | 15.25 | 0.02 | 0.0174 | 0.0006 | 11.0 | 58.9 | 15.05 | 0.02 | 0.0136 | 0.0007 | 11.0 | 55.9 |
| 2001cy | 15.76 | 0.03 | 0.0209 | 0.0011 | 9.4 | 56.3 | 15.72 | 0.01 | 0.0123 | 0.0005 | 6.4 | 61.3 | 15.71 | 0.01 | 0.0084 | 0.0004 | 6.4 | 66.3 |
| 2001X | 15.12 | 0.02 | 0.0044 | 0.0005 | 13.1 | 63.9 | 14.93 | 0.02 | 0.0005 | 0.0005 | 13.1 | 68.9 | 14.96 | 0.04 | -0.0038 | 0.0008 | 13.1 | 68.9 |
| 2002gd | 17.01 | 0.04 | 0.0149 | 0.0014 | 8.0 | 47.5 | 16.93 | 0.03 | 0.0038 | 0.0008 | 6.7 | 65.6 | 16.89 | 0.04 | 0.0006 | 0.0012 | 8.0 | 63.6 |
| 2002gw | 17.29 | 0.02 | 0.0035 | 0.0007 | 8.3 | 56.3 | – | – | – | – | – | – | 16.92 | 0.02 | -0.0052 | 0.0007 | 9.2 | 56.3 |
| 2002hj | 17.91 | 0.04 | 0.0166 | 0.0010 | 23.2 | 53.2 | – | – | – | – | – | – | 17.46 | 0.03 | 0.0098 | 0.0007 | 23.2 | 57.1 |
| 2002hh | 16.15 | 0.05 | 0.0055 | 0.0021 | 3.1 | 43.1 | – | – | – | – | – | – | 13.61 | 0.03 | 0.0005 | 0.0013 | 4.1 | 43.1 |
| 2003B | 15.65 | 0.02 | 0.0062 | 0.0005 | 29.2 | 56.1 | – | – | – | – | – | – | – | – | – | – | – | – |
| 2003E | 18.38 | 0.04 | 0.0010 | 0.0009 | 14.2 | 67.1 | – | – | – | – | – | – | 17.68 | 0.03 | -0.0037 | 0.0008 | 13.7 | 59.6 |
| 2003T | 18.79 | 0.03 | 0.0087 | 0.0010 | 14.2 | 56.2 | – | – | – | – | – | – | 18.50 | 0.02 | -0.0018 | 0.0006 | 14.2 | 56.2 |
| 2003Z | 17.17 | 0.05 | 0.0031 | 0.0012 | 4.8 | 61.7 | 16.94 | 0.04 | -0.0000 | 0.0008 | 8.9 | 74.5 | 16.96 | 0.02 | -0.0067 | 0.0005 | 8.9 | 61.7 |
| 2003bl | 18.81 | 0.02 | 0.0043 | 0.0005 | 2.0 | 65.2 | – | – | – | – | – | – | 18.64 | 0.03 | -0.0073 | 0.0007 | 2.8 | 54.7 |
| 2003bn | 17.13 | 0.03 | 0.0063 | 0.0007 | 10.1 | 70.1 | – | – | – | – | – | – | 16.95 | 0.02 | -0.0029 | 0.0005 | 12.0 | 66.0 |
| 2003cn | 18.11 | 0.04 | 0.0151 | 0.0012 | 14.4 | 45.2 | – | – | – | – | – | – | 17.89 | 0.06 | 0.0060 | 0.0016 | 13.9 | 62.7 |
| 2003cx | 19.35 | 0.06 | 0.0070 | 0.0018 | 11.4 | 54.3 | – | – | – | – | – | – | – | – | – | – | – | – |
| 2003ef | 17.40 | 0.03 | 0.0083 | 0.0008 | 13.2 | 61.1 | – | – | – | – | – | – | 16.83 | 0.04 | 0.0001 | 0.0010 | 22.6 | 66.6 |
| 2003fb | 19.30 | 0.09 | 0.0060 | 0.0018 | 21.3 | 66.1 | – | – | – | – | – | – | – | – | – | – | – | – |
| 2003hd | 18.65 | 0.05 | 0.0138 | 0.0013 | 9.3 | 51.2 | 18.60 | 0.04 | 0.0050 | 0.0008 | 13.2 | 72.2 | 18.48 | 0.04 | 0.0020 | 0.0009 | 13.2 | 57.2 |
| 2003hf | 16.62 | 0.05 | 0.0392 | 0.0017 | 13.2 | 49.1 | 16.65 | 0.04 | 0.0291 | 0.0013 | 13.2 | 55.1 | 16.60 | 0.06 | 0.0229 | 0.0016 | 15.2 | 52.1 |
| 2003hg | 17.43 | 0.05 | 0.0113 | 0.0011 | 6.2 | 64.1 | 16.84 | 0.04 | 0.0065 | 0.0010 | 13.8 | 63.6 | 16.48 | 0.03 | 0.0026 | 0.0009 | 5.7 | 63.6 |
| 2003hl | 16.40 | 0.09 | 0.0070 | 0.0024 | 12.9 | 61.7 | 16.23 | 0.05 | 0.0003 | 0.0012 | 10.9 | 59.7 | 15.83 | 0.06 | -0.0038 | 0.0014 | 14.0 | 63.8 |
| 2003hn | 14.10 | 0.06 | 0.0157 | 0.0012 | 22.8 | 61.8 | 13.93 | 0.03 | 0.0099 | 0.0008 | 20.8 | 61.8 | 13.93 | 0.02 | 0.0055 | 0.0004 | 20.8 | 76.7 |
| 2003ib | 17.72 | 0.02 | 0.0177 | 0.0007 | 15.0 | 61.1 | 17.54 | 0.05 | 0.0123 | 0.0012 | 16.6 | 62.5 | 17.51 | 0.02 | 0.0077 | 0.0005 | 14.5 | 62.5 |
| 2003ip | 16.24 | 0.04 | 0.0210 | 0.0008 | 19.2 | 63.1 | 16.04 | 0.05 | 0.0137 | 0.0011 | 18.7 | 62.6 | 15.84 | 0.04 | 0.0126 | 0.0008 | 18.7 | 69.6 |
| 2003iq | 15.63 | 0.01 | 0.0066 | 0.0004 | 6.9 | 51.8 | 15.41 | 0.06 | 0.0033 | 0.0014 | 7.4 | 72.2 | 15.38 | 0.05 | -0.0011 | 0.0014 | 7.4 | 68.1 |
| 2004du | 16.60 | 0.02 | 0.0124 | 0.0005 | 9.8 | 60.7 | 16.39 | 0.01 | 0.0086 | 0.0005 | 9.8 | 41.7 | 16.42 | 0.02 | 0.0032 | 0.0005 | 16.7 | 60.7 |
| 2004et | 12.44 | 0.04 | 0.0093 | 0.0010 | 9.4 | 59.3 | 12.18 | 0.03 | 0.0034 | 0.0008 | 9.4 | 59.3 | 11.95 | 0.02 | -0.0004 | 0.0004 | 18.4 | 84.3 |
| 2004er | 16.94 | 0.02 | 0.0103 | 0.0005 | 10.1 | 77.0 | – | – | – | – | – | – | – | – | – | – | – | – |
| 2004fx | 17.53 | 0.02 | 0.0007 | 0.0007 | 18.4 | 59.2 | – | – | – | – | – | – | – | – | – | – | – | – |
| 2005J | 16.63 | 0.02 | 0.0144 | 0.0005 | 7.1 | 64.0 | – | – | – | – | – | – | – | – | – | – | – | – |
| 2005dq | 17.27 | 0.07 | 0.0256 | 0.0021 | 7.3 | 57.2 | 17.39 | 0.06 | 0.0157 | 0.0015 | 19.2 | 57.2 | 16.89 | 0.06 | 0.0220 | 0.0019 | 9.3 | 49.2 |
| 2005cs | 14.52 | 0.01 | 0.0063 | 0.0006 | 1.4 | 51.4 | 14.43 | 0.01 | -0.0039 | 0.0004 | 5.5 | 61.4 | 14.42 | 0.01 | -0.0086 | 0.0004 | 5.5 | 63.3 |
| 2005dx | 19.03 | 0.03 | 0.0161 | 0.0010 | 10.1 | 51.1 | – | – | – | – | – | – | – | – | – | – | – | – |
| 2005dz | 17.87 | 0.01 | 0.0114 | 0.0004 | 9.3 | 56.1 | – | – | – | – | – | – | – | – | – | – | – | – |
| 2006Y | 17.68 | 0.10 | 0.0500 | 0.0053 | 9.0 | 32.1 | – | – | – | – | – | – | – | – | – | – | – | – |
| 2006iw | 18.52 | 0.02 | 0.0118 | 0.0008 | 8.0 | 65.0 | – | – | – | – | – | – | – | – | – | – | – | – |
| 2006ai | 16.13 | 0.04 | 0.0285 | 0.0014 | 5.0 | 53.7 | – | – | – | – | – | – | – | – | – | – | – | – |
| 2006bp | 15.08 | 0.02 | 0.0081 | 0.0008 | 6.8 | 51.5 | 14.77 | 0.03 | 0.0017 | 0.0015 | 4.1 | 30.2 | – | – | – | – | – | – |
| 2007W | 17.55 | 0.02 | 0.0030 | 0.0006 | 11.0 | 70.9 | – | – | – | – | – | – | – | – | – | – | – | – |
| 2007U | 17.13 | 0.07 | 0.0225 | 0.0023 | 9.0 | 50.9 | – | – | – | – | – | – | – | – | – | – | – | – |
| 2007X | 15.19 | 0.04 | 0.0183 | 0.0012 | 10.1 | 54.0 | – | – | – | – | – | – | – | – | – | – | – | – |
| 2007ab | 17.67 | 0.09 | 0.0286 | 0.0021 | 35.1 | 56.1 | – | – | – | – | – | – | – | – | – | – | – | – |

* the slope is computed with the following equation: mag = M + $s50$ × t

**Table D2:** Slope Data

| SN | $M(V)$ * $\Delta M$ | $s50(V)$ $(V)$ | $\Delta$ s50(V) | $ph\_start$ | $ph\_stop$ $(V)$ | $M(R)$ $(V)$ | $\Delta M$ | $s50(R)$ $(R)$ | $\Delta s50(R)$ | $ph\_start$ | $ph\_stop$ $(R)$ | $M(I)$ $(R)$ | $\Delta M$ | $s50(I)$ $(I)$ | $\Delta s50(I)$ | $ph\_start$ | $ph\_stop$ $(I)$ | $(I)$ |
|---|---|---|---|---|---|---|---|---|---|---|---|---|---|---|---|---|---|---|
| 2007it | 18.80 | 0.02 | 0.0083 | 0.0006 | 14.2 | 79.1 | – | – | – | – | – | – | – | – | – | – | – | – |
| 2007ld | 17.86 | 0.04 | 0.0196 | 0.0015 | 6.0 | 48.0 | – | – | – | – | – | – | – | – | – | – | – | – |
| 2007od | 14.16 | 0.02 | 0.0146 | 0.0007 | 5.5 | 55.5 | 13.92 | 0.03 | 0.0100 | 0.0008 | 6.6 | 58.2 | 13.71 | 0.06 | 0.0103 | 0.0018 | 6.6 | 58.2 |
| 2008M | 15.91 | 0.04 | 0.0122 | 0.0013 | 13.0 | 55.8 | – | – | – | – | – | – | – | – | – | – | – | – |
| 2008K | 17.70 | 0.03 | 0.0278 | 0.0009 | 7.1 | 61.1 | – | – | – | – | – | – | – | – | – | – | – | – |
| 2008aw | 15.30 | 0.05 | 0.0285 | 0.0015 | 13.1 | 45.1 | – | – | – | – | – | – | – | – | – | – | – | – |
| 2008fq | 15.35 | 0.06 | 0.0333 | 0.0020 | 12.6 | 46.5 | – | – | – | – | – | – | – | – | – | – | – | – |
| 2008if | 15.38 | 0.03 | 0.0306 | 0.0012 | 11.0 | 48.0 | – | – | – | – | – | – | – | – | – | – | – | – |
| 2008in | 15.45 | 0.08 | 0.0271 | 0.0019 | 7.9 | 57.8 | 15.10 | 0.03 | 0.0082 | 0.0006 | 4.9 | 63.7 | 14.77 | 0.06 | 0.0055 | 0.0012 | 4.9 | 69.7 |
| 2009N | 16.28 | 0.02 | 0.0032 | 0.0004 | 13.1 | 71.1 | 16.03 | 0.02 | -0.0026 | 0.0005 | 11.6 | 55.6 | 15.87 | 0.02 | -0.0079 | 0.0004 | 11.7 | 62.4 |
| 2009bw | 14.74 | 0.02 | 0.0206 | 0.0008 | 9.0 | 53.8 | 14.51 | 0.02 | 0.0127 | 0.0006 | 9.7 | 56.9 | 14.33 | 0.02 | 0.0065 | 0.0007 | 9.0 | 66.1 |
| 2009dd | 14.58 | 0.05 | 0.0184 | 0.0021 | 11.2 | 46.1 | – | – | – | – | – | – | – | – | – | – | – | – |
| 2009ib | 15.73 | 0.02 | 0.0089 | 0.0006 | 13.1 | 55.0 | 15.52 | 0.02 | 0.0035 | 0.0005 | 13.1 | 63.0 | 15.46 | 0.01 | -0.0016 | 0.0003 | 13.1 | 80.0 |
| 2009js | 17.27 | 0.02 | 0.0045 | 0.0006 | 8.8 | 56.5 | 16.77 | 0.01 | 0.0016 | 0.0004 | 11.6 | 61.6 | 16.56 | 0.02 | -0.0043 | 0.0004 | 11.6 | 61.6 |
| 2009kr | 15.25 | 0.02 | 0.0272 | 0.0006 | 9.1 | 54.3 | 15.02 | 0.03 | 0.0175 | 0.0008 | 11.2 | 62.3 | 14.61 | 0.02 | 0.0183 | 0.0007 | 11.2 | 62.3 |
| 2009md | 16.98 | 0.04 | 0.0059 | 0.0009 | 22.0 | 57.7 | 16.72 | 0.03 | 0.0011 | 0.0007 | 18.0 | 62.5 | 16.66 | 0.05 | -0.0023 | 0.0009 | 19.6 | 74.5 |
| 2010id | 18.83 | 0.05 | 0.0056 | 0.0014 | 4.0 | 79.8 | 18.86 | 0.04 | -0.0001 | 0.0011 | 6.0 | 79.8 | 18.58 | 0.05 | -0.0082 | 0.0016 | 6.0 | 76.8 |
| 2012A | 13.72 | 0.03 | 0.0146 | 0.0009 | 9.5 | 53.5 | 13.56 | 0.03 | 0.0077 | 0.0007 | 8.4 | 65.6 | 13.51 | 0.03 | 0.0038 | 0.0008 | 11.6 | 65.6 |
| 2012aw | 13.25 | 0.02 | 0.0051 | 0.0006 | 9.8 | 54.6 | 13.11 | 0.01 | -0.0003 | 0.0003 | 12.9 | 62.6 | 13.14 | 0.01 | -0.0065 | 0.0003 | 6.1 | 67.0 |
| 2012ec | 14.79 | 0.03 | 0.0073 | 0.0009 | 12.2 | 51.9 | 14.64 | 0.04 | 0.0023 | 0.0010 | 15.3 | 59.2 | 14.62 | 0.03 | -0.0034 | 0.0008 | 14.6 | 69.2 |
| LSQ13cuw | – | – | – | – | – | – | 17.90 | 0.08 | 0.0467 | 0.0020 | 13.4 | 59.4 | 18.10 | 0.18 | 0.0384 | 0.0035 | 27.8 | 75.6 |
| OGLE13-005 | – | – | – | – | – | – | – | – | – | – | – | – | -18.09 | 0.06 | 0.0031 | 0.0015 | 8.9 | 62.9 |
| OGLE13-011 | – | – | – | – | – | – | – | – | – | – | – | – | -18.02 | 0.08 | 0.0076 | 0.0017 | 12.4 | 64.3 |
| OGLE13-045 | – | – | – | – | – | – | – | – | – | – | – | – | -18.62 | 0.10 | 0.0077 | 0.0018 | 17.4 | 78.3 |
| OGLE13-046 | – | – | – | – | – | – | – | – | – | – | – | – | -17.97 | 0.08 | 0.0040 | 0.0020 | 9.0 | 57.8 |
| OGLE13-047 | – | – | – | – | – | – | – | – | – | – | – | – | -19.09 | 0.05 | 0.0155 | 0.0011 | 10.5 | 67.3 |
| OGLE13-048 | – | – | – | – | – | – | – | – | – | – | – | – | -17.55 | 0.08 | 0.0013 | 0.0014 | 19.4 | 92.3 |
| OGLE13-135 | – | – | – | – | – | – | – | – | – | – | – | – | -18.42 | 0.05 | 0.0023 | 0.0012 | 13.0 | 68.9 |
| OGLE13-144 | – | – | – | – | – | – | – | – | – | – | – | – | -17.84 | 0.06 | 0.0096 | 0.0014 | 6.0 | 63.9 |
| OGLE14-004 | – | – | – | – | – | – | – | – | – | – | – | – | -17.07 | 0.05 | 0.0027 | 0.0016 | 2.5 | 53.3 |
| OGLE14-009 | – | – | – | – | – | – | – | – | – | – | – | – | -18.05 | 0.07 | 0.0124 | 0.0018 | 6.5 | 61.3 |
| OGLE14-018 | – | – | – | – | – | – | – | – | – | – | – | – | -17.36 | 0.06 | 0.0006 | 0.0013 | 8.5 | 91.3 |

* the slope is computed with the following equation: mag = M + $s50$ $\times$ t

**Table D3:** Bolometric light curve parameters

| SN | $Log10(Lum1(0))$ | $S1$ | $\Delta S1$ | $ph\_start$ [days] | $ph\_stop$ [days] | $Log10(Lum2(0))$ | $S2$ | $\Delta S2$ | $ph\_start$ [days] | $ph\_stop$ [days] | Ni $M_\odot$ | $\Delta$ $Ni$ $M_\odot$ |
|---|---|---|---|---|---|---|---|---|---|---|---|---|
| 2013ai | 41.62 | -0.0081 | 0.0001 | 18.6 | 49.5 | 41.47 | -0.0057 | 0.0005 | 54.5 | 92.2 | – | – |
| 2013bu | 41.24 | -0.0044 | 0.0003 | 6.2 | 35.1 | 41.18 | -0.0020 | 0.0003 | 35.1 | 78.1 | 0.0021 | 0.0007 |
| 2013fs | 42.47 | -0.0146 | 0.0009 | 4.5 | 27.6 | 42.19 | -0.0054 | 0.0002 | 31.5 | 75.5 | 0.0545 | 0.0003 |
| LSQ13dpa | 42.02 | -0.0042 | 0.0006 | 5.5 | 36.9 | 41.99 | -0.0021 | 0.0004 | 43.4 | 114.3 | 0.0714 | 0.0127 |
| 2014cy | 41.66 | -0.0060 | 0.0005 | 5.4 | 33.0 | 41.51 | -0.0031 | 0.0002 | 44.3 | 94.5 | 0.0037 | 0.0038 |
| 2014dw | 42.23 | -0.0135 | 0.0005 | 14.2 | 38.2 | 42.18 | -0.0113 | 0.0003 | 47.5 | 78.5 | 0.0094 | 0.0008 |
| LSQ14gv | 42.19 | -0.0081 | 0.0014 | 3.8 | 40.6 | 42.17 | -0.0087 | 0.0007 | 35.5 | 70.6 | – | – |
| ASASSN-14dq | 42.36 | -0.0098 | 0.0004 | 7.7 | 33.6 | 42.18 | -0.0048 | 0.0003 | 48.7 | 82.6 | 0.0461 | 0.0079 |
| ASASSN-14gm | 42.10 | -0.0030 | 0.0003 | 12.2 | 43.3 | 42.07 | -0.0021 | 0.0004 | 43.3 | 85.6 | 0.0767 | 0.0102 |
| ASASSN-14ha | 41.28 | -0.0093 | 0.0003 | 1.8 | 37.5 | 41.02 | -0.0020 | 0.0002 | 42.9 | 121.5 | 0.0014 | 0.0002 |
| 2015W | 42.26 | -0.0096 | 0.0005 | 9.8 | 45.3 | 42.08 | -0.0061 | 0.0006 | 51.4 | 92.2 | 0.0314 | 0.0098 |
| 2013ab | 42.36 | -0.0120 | 0.0002 | 8.8 | 36.4 | 42.00 | -0.0027 | 0.0001 | 42.4 | 82.2 | 0.0588 | 0.0100 |
| 2013by | 42.80 | -0.0167 | 0.0007 | 8.5 | 39.7 | 42.48 | -0.0083 | 0.0002 | 39.7 | 67.6 | 0.0320 | 0.0043 |
| 2013ej | 42.46 | -0.0136 | 0.0004 | 9.9 | 38.4 | 42.25 | -0.0079 | 0.0005 | 43.4 | 83.0 | 0.0207 | 0.0019 |
| 2014G | 42.68 | -0.0151 | 0.0006 | 15.4 | 36.4 | 42.39 | -0.0091 | 0.0005 | 49.3 | 78.4 | 0.0341 | 0.0006 |
| 1987A | – | – | – | – | – | – | – | – | – | – | 0.0750 | 0.0007 |
| 1990E | – | – | – | – | – | – | – | – | – | – | 0.0653 | 0.0134 |
| 1999em | 42.21 | -0.0109 | 0.0004 | 3.0 | 34.4 | 41.91 | -0.0014 | 0.0002 | 32.4 | 82.2 | 0.0536 | 0.0119 |
| 1999gi | 42.02 | -0.0090 | 0.0001 | 8.6 | 38.2 | 41.72 | -0.0020 | 0.0002 | 50.2 | 100.5 | 0.0320 | 0.0023 |
| 2001X | 42.02 | -0.0053 | 0.0008 | 13.1 | 41.9 | 41.89 | -0.0018 | 0.0001 | 49.0 | 86.8 | 0.0550 | 0.0047 |
| 2002hh | – | – | – | – | – | – | – | – | – | – | 0.0316 | 0.0102 |
| 2003Z | 41.19 | -0.0071 | 0.0005 | 5.8 | 29.4 | 41.13 | -0.0031 | 0.0003 | 56.7 | 100.7 | 0.0047 | 0.0002 |
| 2003hd | 42.18 | -0.0068 | 0.0010 | 9.3 | 44.3 | 42.02 | -0.0030 | 0.0009 | 44.3 | 72.2 | 0.0361 | 0.0040 |
| 2003hn | 42.53 | -0.0152 | 0.0007 | 20.8 | 42.8 | 42.08 | -0.0048 | 0.0002 | 48.9 | 83.8 | 0.0324 | 0.0046 |
| 2004et | 42.19 | -0.0064 | inf | 18.4 | 53.4 | 42.00 | -0.0028 | 0.0002 | 53.4 | 84.3 | 0.0414 | 0.0086 |
| 2005cs | 41.48 | -0.0192 | 0.0005 | 4.3 | 22.3 | 41.03 | 0.0004 | 0.0001 | 28.4 | 79.2 | 0.0021 | 0.0002 |
| 2007it | – | – | – | – | – | – | – | – | – | – | 0.0721 | 0.0175 |
| 2007od | 42.59 | -0.0148 | 0.0010 | 6.6 | 21.5 | 42.43 | -0.0074 | 0.0002 | 28.5 | 69.2 | 0.0032 | 0.0006 |
| 2008fq | 43.13 | -0.0168 | 0.0013 | 12.6 | 33.6 | 42.80 | -0.0077 | 0.0006 | 39.6 | 70.5 | – | – |
| 2008in | 41.68 | -0.0201 | 0.0021 | 4.9 | 34.7 | 41.23 | -0.0056 | 0.0005 | 38.8 | 89.7 | 0.0037 | 0.0007 |
| 2009N | 41.71 | -0.0127 | 0.0007 | 10.7 | 26.6 | 41.43 | -0.0012 | 0.0001 | 31.6 | 79.3 | 0.0165 | 0.0021 |
| 2009bw | 42.51 | -0.0164 | 0.0010 | 9.7 | 33.8 | 42.01 | -0.0034 | 0.0004 | 53.8 | 116.2 | 0.0234 | 0.0017 |
| 2009dd | 42.50 | -0.0130 | 0.0008 | 11.2 | 46.1 | 42.18 | -0.0055 | nan | 46.1 | 107.9 | 0.0466 | 0.0116 |
| 2009ib | 41.77 | -0.0069 | 0.0005 | 13.1 | 38.1 | 41.50 | -0.0004 | 0.0002 | 59.0 | 109.8 | 0.0520 | 0.0162 |
| 2009kr | 42.23 | -0.0168 | 0.0011 | 9.1 | 27.0 | 41.98 | -0.0093 | 0.0010 | 49.1 | 75.8 | 0.0085 | 0.0002 |
| 2009md | 41.36 | -0.0069 | 0.0006 | 18.0 | 35.5 | 41.26 | -0.0030 | 0.0002 | 49.6 | 100.7 | 0.0044 | 0.0033 |
| 2012A | 41.96 | -0.0139 | 0.0012 | 9.5 | 28.4 | 41.66 | -0.0042 | 0.0003 | 35.6 | 71.5 | 0.0087 | 0.0012 |
| 2012aw | 42.23 | -0.0096 | 0.0002 | 9.0 | 36.6 | 41.97 | -0.0021 | 0.0001 | 41.0 | 102.9 | 0.0497 | 0.0059 |
| 2012ec | 42.21 | -0.0102 | 0.0007 | 11.2 | 36.3 | 41.93 | -0.0020 | 0.0003 | 37.9 | 78.1 | 0.0394 | 0.0051 |

* the slope is computed with the following equation: Log10(Lum(t)) = Log10(Lum(0)) + S1 × t

**Table D4:** Bolometric MCMC light curve parameters

| SN | $T_{pt}$ | $\Delta T_{pt}$ | $A0$ | $A0+$ | $A0-$ | $W0$ | $W0+$ | $W0-$ | $M0$ | $M0+$ | $M0-$ | P0 |
|---|---|---|---|---|---|---|---|---|---|---|---|---|
| 2013bu | 102.8 | 4.5 | -1.14330 | 0.00008 | 0.00011 | 3.85663 | 0.00011 | 0.00011 | 39.73643 | 0.00011 | 0.00010 | -0.0038 |
| 2013fs | 86.2 | 0.5 | -0.60601 | 0.00010 | 0.00009 | 4.85452 | 0.00010 | 0.00010 | 41.17148 | 0.00010 | 0.00009 | -0.0038 |
| LSQ13dpa | 129.9 | 2.0 | -0.52529 | 0.00010 | 0.00009 | 4.60926 | 0.00010 | 0.00010 | 41.16555 | 0.00007 | 0.00010 | -0.0038 |
| 2014cy | 122.6 | 1.0 | -1.17027 | 0.00009 | 0.00010 | 4.68129 | 0.00010 | 0.00010 | 39.92448 | 0.00010 | 0.00010 | -0.0038 |
| 2014dw | 90.8 | 10.0 | -0.75675 | 0.00011 | 0.00009 | 4.17129 | 0.00009 | 0.00009 | 40.51770 | 0.00011 | 0.00010 | -0.0058 |
| ASASSN-14dq | 101.5 | 5.5 | -0.65170 | 0.00010 | 0.00010 | 4.48552 | 0.00011 | 0.00011 | 41.06156 | 0.00011 | 0.00010 | -0.0038 |
| ASASSN-14gm | 110.6 | 1.5 | -0.58317 | 0.00012 | 0.00009 | 5.09893 | 0.00009 | 0.00009 | 41.21063 | 0.00011 | 0.00010 | -0.0028 |
| ASASSN-14ha | 136.9 | 1.5 | -1.29399 | 0.00010 | 0.00010 | 1.67183 | 0.00010 | 0.00010 | 39.38707 | 0.00011 | 0.00010 | -0.0038 |
| 2015W | 109.2 | 10.0 | -0.50126 | 0.00009 | 0.00010 | 6.75293 | 0.00010 | 0.00010 | 40.97968 | 0.00012 | 0.00007 | -0.0038 |
| 2013ab | 102.0 | 1.0 | -0.51427 | 0.00010 | 0.00008 | 3.78071 | 0.00010 | 0.00010 | 41.17435 | 0.00009 | 0.00010 | -0.0038 |
| 2013by | 85.8 | 2.0 | -0.91657 | 0.00009 | 0.00010 | 5.65613 | 0.00009 | 0.00009 | 40.96187 | 0.00011 | 0.00010 | -0.0038 |
| 2013ej | 99.4 | 1.0 | -0.72281 | 0.00010 | 0.00010 | 2.94088 | 0.00009 | 0.00009 | 40.75374 | 0.00010 | 0.00009 | -0.0048 |
| 2014G | 87.8 | 1.0 | -0.71244 | 0.00010 | 0.00009 | 4.51613 | 0.00010 | 0.00010 | 40.99829 | 0.00011 | 0.00009 | -0.0038 |
| 1999em | 117.9 | 1.0 | -0.57741 | 0.00008 | 0.00009 | 3.41479 | 0.00010 | 0.00010 | 41.06099 | 0.00009 | 0.00008 | -0.0038 |
| 1999gi | 126.6 | 3.1 | -0.62125 | 0.00010 | 0.00010 | 4.55976 | 0.00010 | 0.00010 | 40.79945 | 0.00009 | 0.00009 | -0.0038 |
| 2001X | 114.5 | 5.0 | -0.53832 | 0.00009 | 0.00010 | 4.38129 | 0.00010 | 0.00010 | 41.08004 | 0.00009 | 0.00009 | -0.0038 |
| 2003Z | 124.2 | 4.5 | -0.71998 | 0.00009 | 0.00010 | 3.26323 | 0.00011 | 0.00011 | 39.99370 | 0.00010 | 0.00011 | -0.0038 |
| 2003hn | 107.3 | 4.0 | -0.65753 | 0.00010 | 0.00009 | 2.53678 | 0.00012 | 0.00012 | 40.89828 | 0.00010 | 0.00009 | -0.0038 |
| 2004et | 123.5 | 4.0 | -0.64942 | 0.00009 | 0.00011 | 6.01467 | 0.00011 | 0.00011 | 40.96975 | 0.00011 | 0.00009 | -0.0038 |
| 2005cs | 125.8 | 0.5 | -1.22037 | 0.00010 | 0.00010 | 1.93610 | 0.00010 | 0.00010 | 39.64530 | 0.00011 | 0.00011 | -0.0038 |
| 2008in | 107.6 | 1.0 | -0.71691 | 0.00009 | 0.00011 | 1.94207 | 0.00010 | 0.00010 | 39.94404 | 0.00009 | 0.00010 | -0.0038 |
| 2009N | 108.1 | 1.2 | -0.60762 | 0.00008 | 0.00009 | 2.34563 | 0.00010 | 0.00010 | 40.59108 | 0.00010 | 0.00011 | -0.0038 |
| 2009bw | 135.5 | 3.0 | -0.85874 | 0.00011 | 0.00010 | 1.51075 | 0.00009 | 0.00009 | 40.63664 | 0.00009 | 0.00010 | -0.0038 |
| 2009dd | 118.3 | 5.0 | -0.56500 | 0.00011 | 0.00010 | 4.44222 | 0.00009 | 0.00009 | 41.02448 | 0.00010 | 0.00010 | -0.0038 |
| 2009ib | 140.2 | 2.0 | -0.35851 | 0.00010 | 0.00010 | 2.69334 | 0.00009 | 0.00009 | 40.96322 | 0.00010 | 0.00010 | -0.0038 |
| 2009kr | 90.0 | 2.0 | -0.87569 | 0.00010 | 0.00010 | 4.34359 | 0.00012 | 0.00012 | 40.36315 | 0.00008 | 0.00011 | -0.0054 |
| 2009md | 117.8 | 8.0 | -0.93139 | 0.00010 | 0.00009 | 2.61584 | 0.00010 | 0.00010 | 39.93533 | 0.00011 | 0.00011 | -0.0038 |
| 2012A | 106.2 | 2.0 | -0.90870 | 0.00009 | 0.00008 | 4.45165 | 0.00010 | 0.00010 | 40.29491 | 0.00010 | 0.00011 | -0.0038 |
| 2012aw | 135.2 | 4.0 | -0.60089 | 0.00011 | 0.00011 | 7.49323 | 0.00011 | 0.00011 | 41.02130 | 0.00011 | 0.00011 | -0.0038 |
| 2012ec | 110.6 | 5.0 | -0.67027 | 0.00010 | 0.00010 | 9.74179 | 0.00010 | 0.00010 | 40.98082 | 0.00010 | 0.00010 | -0.0038 |

*

**Table D5:** MCMC parameters on V band light curves

| SN | $t_{pt}$ | $\Delta t_{pt}$ | $a0$ | $a0+$ | $a0-$ | $w0$ | $w0+$ | $w0-$ | $m0$ | $m0+$ | $m0-$ | p0 |
|---|---|---|---|---|---|---|---|---|---|---|---|---|
| 2013bu | 103.1 | 4.5 | 3.08170 | 0.15800 | 0.14293 | 3.51516 | 0.60600 | 0.60607 | 20.27520 | 0.14960 | 0.13669 | 0.0120 |
| 2013fs | 82.7 | 0.5 | 1.59863 | 0.09900 | 0.07214 | 2.27769 | 2.47320 | 2.47329 | 18.76480 | 0.13160 | 0.08128 | 0.0120 |
| LSQ13dpa | 128.7 | 2.0 | 1.71574 | 0.07200 | 0.07241 | 4.67327 | 0.54640 | 0.54648 | 20.36860 | 0.07000 | 0.07038 | 0.0042 |
| 2014dw | 91.3 | 10.0 | 1.75577 | 0.05500 | 0.05470 | 3.37373 | 0.38760 | 0.38763 | 19.83370 | 0.05320 | 0.05096 | 0.0260 |
| ASASSN-14dq | 101.0 | 5.5 | 1.58685 | 0.02900 | 0.03044 | 3.34375 | 0.27780 | 0.27782 | 18.73570 | 0.01990 | 0.01985 | 0.0127 |
| ASASSN-14gm | 110.6 | 1.5 | 1.65492 | 0.03800 | 0.04032 | 5.95449 | 0.51220 | 0.51228 | 17.02060 | 0.01440 | 0.02153 | 0.0082 |
| ASASSN-14ha | 136.8 | 1.5 | 3.35748 | 0.11900 | 0.11385 | 1.36023 | 0.16640 | 0.16644 | 19.12990 | 0.11430 | 0.11078 | 0.0120 |
| 2013ab | 101.8 | 1.0 | 1.42075 | 0.01300 | 0.01308 | 3.28386 | 0.13770 | 0.13777 | 17.18670 | 0.01040 | 0.01022 | 0.0107 |
| 2013by | 85.4 | 2.0 | 2.38699 | 0.04500 | 0.04446 | 4.59398 | 0.41810 | 0.41813 | 17.19440 | 0.02940 | 0.02951 | 0.0120 |
| 2013ej | 98.8 | 1.0 | 2.23773 | 0.03900 | 0.03937 | 3.41156 | 0.32750 | 0.32756 | 16.35470 | 0.03240 | 0.03192 | 0.0134 |
| 2014G | 87.5 | 1.0 | 1.34118 | 0.04700 | 0.04464 | 2.66318 | 0.30360 | 0.30361 | 17.82740 | 0.04240 | 0.04137 | 0.0238 |
| 1986L | 110.8 | 6.0 | 0.97384 | 0.13400 | 0.10437 | 3.52309 | 3.70490 | 3.70490 | 16.72320 | 0.17090 | 0.12274 | 0.0301 |
| 1979C | 55.6 | 15.0 | 0.54948 | 0.02400 | 0.02351 | 2.55671 | 0.59640 | 0.59649 | 13.82830 | 0.03410 | 0.03110 | 0.0277 |
| 1992ba | 125.5 | 8.0 | 1.87475 | 0.03700 | 0.03395 | 5.33330 | 0.76550 | 0.76551 | 17.97920 | 0.02590 | 0.02509 | 0.0086 |
| 1999em | 118.1 | 1.0 | 1.60486 | 0.04100 | 0.04035 | 2.82646 | 0.79980 | 0.79981 | 16.14400 | 0.03590 | 0.03409 | 0.0115 |
| 1999gi | 127.8 | 3.1 | 1.95904 | 0.10200 | 0.08906 | 5.56184 | 1.06340 | 1.06342 | 17.36290 | 0.06980 | 0.06503 | 0.0092 |
| 2001X | 114.7 | 5.0 | 1.40032 | 0.03300 | 0.03216 | 4.10216 | 0.31090 | 0.31096 | 17.27810 | 0.03370 | 0.03265 | 0.0131 |
| 2002hj | 99.7 | 7.0 | 2.13250 | 0.00000 | 0.00010 | 6.56108 | 0.00010 | 0.00012 | 21.58200 | 9.00910 | 9.84051 | 0.0141 |
| 2003T | 103.9 | 10.0 | 1.30859 | 0.04900 | 0.04860 | 2.56083 | 0.26960 | 0.26961 | 21.22110 | 0.05040 | 0.05285 | 0.0202 |
| 2003bn | 118.9 | 3.0 | 1.84879 | 0.00000 | 0.00010 | 4.44229 | 9.67260 | 9.67267 | 19.85290 | 0.00010 | 0.00010 | 0.0120 |
| 2003cx | 92.4 | 5.0 | 1.05701 | 9.52700 | 0.00010 | 0.19338 | 8.95750 | 8.95759 | 21.19450 | 0.00010 | 9.46331 | 0.0120 |
| 2003hd | 96.5 | 5.0 | 2.31035 | 0.07900 | 0.07446 | 3.02649 | 1.39710 | 1.39714 | 21.96160 | 0.07550 | 0.07225 | 0.0072 |
| 2003hn | 106.9 | 4.0 | 1.76998 | 9.55500 | 9.30409 | 2.33249 | 9.58090 | 9.58092 | 17.37200 | 9.53970 | 9.72347 | 0.0128 |
| 2003iq | 102.1 | 2.0 | 1.61370 | 0.00000 | 8.35990 | 4.52065 | 9.80470 | 9.80473 | 18.11550 | 0.00010 | 9.40875 | 0.0120 |
| 2004er | 146.6 | 2.0 | 1.34839 | 0.10800 | 0.09203 | 7.68156 | 1.10760 | 1.10763 | 19.65000 | 0.10810 | 0.09462 | 0.0120 |
| 2004fx | 102.8 | 4.0 | 1.90191 | 0.04700 | 0.04804 | 4.12092 | 0.34660 | 0.34666 | 19.98650 | 0.02290 | 0.02374 | 0.0088 |
| 2005cs | 126.0 | 0.5 | 3.83298 | 0.04800 | 0.04709 | 2.31455 | 0.24890 | 0.24892 | 19.12080 | 0.04790 | 0.04634 | 0.0086 |
| 2006Y | 66.8 | 4.0 | 1.74803 | 0.23000 | 0.15203 | 4.28711 | 1.10340 | 1.10348 | 21.22620 | 0.23080 | 0.15381 | 0.0120 |
| 2006ai | 72.4 | 5.0 | 1.49117 | 0.00000 | 8.95440 | 3.46120 | 0.00010 | 0.00010 | 19.36580 | 0.00010 | 9.82648 | 0.0177 |
| 2007ab | 78.6 | 10.0 | 0.77127 | 0.00000 | 0.00010 | 3.37229 | 0.00010 | 0.00010 | 20.72720 | 9.22350 | 0.00011 | 0.0231 |
| 2007it | 113.1 | 10.0 | 1.23574 | 0.01300 | 0.01291 | 4.29137 | 0.20570 | 0.20571 | 15.58930 | 0.00560 | 0.00492 | 0.0100 |
| 2008M | 85.7 | 9.0 | 2.05115 | 0.03200 | 0.03193 | 2.67883 | 0.39460 | 0.39467 | 18.95140 | 0.02770 | 0.02715 | 0.0116 |
| 2008K | 95.3 | 4.0 | 1.55800 | 9.32200 | 0.00010 | 6.73933 | 9.84710 | 9.84717 | 21.51660 | 0.00010 | 0.00010 | 0.0186 |
| 2008aw | 87.6 | 10.0 | 1.40924 | 0.01800 | 0.01873 | 5.31038 | 0.50340 | 0.50345 | 18.85360 | 0.03400 | 0.03501 | 0.0197 |
| 2008if | 84.5 | 5.0 | 1.67851 | 0.02800 | 0.02772 | 4.79672 | 0.23640 | 0.23641 | 18.90100 | 0.02550 | 0.02617 | 0.0120 |
| 2008in | 108.0 | 1.0 | 2.81272 | 0.09100 | 0.08935 | 3.38508 | 0.56450 | 0.56458 | 20.17500 | 0.07820 | 0.07636 | 0.0047 |
| 2009N | 108.3 | 1.2 | 1.89538 | 0.02700 | 0.02757 | 2.83898 | 0.21080 | 0.21085 | 18.72150 | 0.02440 | 0.02376 | 0.0084 |
| 2009bw | 135.2 | 3.0 | 2.27081 | 0.03700 | 0.03802 | 1.51786 | 0.19190 | 0.19193 | 18.84930 | 0.02970 | 0.02921 | 0.0133 |
| 2009ib | 140.1 | 2.0 | 1.23238 | 0.02900 | 0.03036 | 4.16122 | 0.23340 | 0.23340 | 17.76620 | 0.02900 | 0.02901 | 0.0080 |
| 2009kr | 88.2 | 2.0 | 2.25729 | 0.10700 | 0.11373 | 3.76747 | 0.56320 | 0.56321 | 19.67400 | 0.10680 | 0.10148 | 0.0200 |
| 2009md | 118.0 | 8.0 | 2.60711 | 8.84000 | 9.73449 | 1.93493 | 9.63880 | 9.63883 | 20.55390 | 9.99120 | 9.81924 | 0.0120 |
| 2012A | 106.5 | 2.0 | 2.71621 | 0.08500 | 0.08451 | 4.77539 | 0.45080 | 0.45089 | 17.67180 | 0.08000 | 0.07854 | 0.0081 |
| 2012aw | 135.2 | 4.0 | 1.74817 | 0.02300 | 0.02105 | 7.49308 | 1.42810 | 1.42813 | 15.87580 | 0.01600 | 0.01438 | 0.0095 |
| 2012ec | 107.9 | 5.0 | 1.57489 | 9.62000 | 8.10385 | 4.81188 | 9.68530 | 9.68539 | 17.30550 | 8.60480 | 9.96944 | 0.0135 |

*

## REFERENCES


Anderson J. P. et al., 2014, The Astrophysical Journal, 786, 67
Andrews J. E. et al., 2011, The Astrophysical Journal, 731, 47
Barbarino C. et al., 2015, Monthly Notices of the Royal Astronomical Society, 448, 2312
Benetti ., Cappellaro ., Turatto ., dellaValle ., Mazzali ., Gouiffes ., 1994, Astronomy and Astrophysics 285
Bose S., Kumar B., 2014, The Astrophysical Journal, 782, 98
Bose S. et al., 2015, Monthly Notices of the Royal Astronomical Society, 450, 2373
Brown P. J. et al., 2010, The Astrophysical Journal, 721, 1608
Dall'Ora M. et al., 2014, The Astrophysical Journal, 787, 139
de Vaucouleurs G., de Vaucouleurs A., Buta R., Ables H. D., Hewitt A. V., 1981, Publications of the Astronomical Society of the Pacific, 93, 36
Dessart L. et al., 2008, The Astrophysical Journal, 675, 644
Elias-Rosa N. et al., 2010, The Astrophysical Journal, 714, L254
Elias-Rosa N. et al., 2011, The Astrophysical Journal, 742, 6
Faran T. et al., 2014a, Monthly Notices of the Royal Astronomical Society, 442, 844
Faran T. et al., 2014b, Monthly Notices of the Royal Astronomical Society, 445, 554
Ferrarese L. et al., 1996, The Astrophysical Journal, 464, 568
Fraser M. et al., 2011, Monthly Notices of the Royal Astronomical Society, 417, 1417
Fraser M. et al., 2014, Monthly Notices of the Royal Astronomical Society: Letters, 439, 5
Freedman W. L. et al., 2001, The Astrophysical Journal, 553, 47
Gal-Yam A. et al., 2011, The Astrophysical Journal, 736, 159
Gall E. E. E. et al., 2015, Astronomy & Astrophysics, 582, A3
Gandhi P. et al., 2013, The Astrophysical Journal, 767, 166
Inserra C. et al., 2013, Astronomy & Astrophysics, 555, A142
Inserra C. et al., 2011, Monthly Notices of the Royal Astronomical Society, 417, 261
Inserra C. et al., 2012, Monthly Notices of the Royal Astronomical Society, 422, 1122
Jones M. I. et al., 2009, The Astrophysical Journal, 696, 1176
Kanbur S. M., Ngeow C., Nikolaev S., Tanvir N. R., Hendry M. A., 2003, Astronomy and Astrophysics, 411, 361
Leonard D. C. et al., 2002, The Astronomical Journal, 124, 2490
Leonard D. C., Kanbur S. M., Ngeow C. C., Tanvir N. R., 2003, The Astrophysical Journal, 594, 247
Maguire K. et al., 2010, Monthly Notices of the Royal Astronomical Society, 404, 981
Mould J., Sakai S., 2008, The Astrophysical Journal, 686, L75
Olivares F. et al., 2010, The Astrophysical Journal, 715, 833
Pastorello a. et al., 2009, Monthly Notices of the Royal Astronomical Society, 394, 2266
Pastorello a. et al., 2004, Monthly Notices of the Royal Astronomical Society, 347, 74
Poznanski D. et al., 2009, The Astrophysical Journal, 694, 1067
Poznanski D., Kostrzewa-Rutkowska Z., Wyrzykowski L., Blagorodnova N., 2015, Monthly Notices of the Royal Astronomical Society, 449, 1753
Pozzo M. et al., 2006, Monthly Notices of the Royal Astronomical Society, 368, 1169
Quimby R. M., Wheeler J. C., Hoflich P., Akerlof C. W., Brown P. J., Rykoff E. S., 2007, The Astrophysical Journal, 666, 1093
Rest A. et al., 2014, The Astrophysical Journal, 795, 44
Schmidt B. P., Kirshner R. P., Eastman R. G., 1992, The Astrophysical Journal, 395, 366
Spiro S. et al., 2014, Monthly Notices of the Royal Astronomical Society, 439, 2873
Taddia F. et al., 2013, Astronomy & Astrophysics, 555, A10
Takats K. et al., 2015, Monthly Notices of the Royal Astronomical Society, 450, 18
Takáts K. et al., 2014, Monthly Notices of the Royal Astronomical Society, 438, 368
Takats K., Vinko J., 2006, Monthly Notices of the Royal Astronomical Society, 372, 1735
Takáts K., Vinkó J., 2012, Monthly Notices of the Royal Astronomical Society, 419, 2783
Tomasella L. et al., 2013, Monthly Notices of the Royal Astronomical Society, 434, 1636
Valenti S. et al., 2014, Monthly Notices of the Royal Astronomical Society: Letters, 438, L101
Valenti S. et al., 2015, Monthly Notices of the Royal Astronomical Society, 448, 2608
Wang X., Wang L., Pain R., Zhou X., Li Z., 2006, The Astrophysical Journal, 645, 488
Zwitter ., Munari ., Moretti ., 2004, IAU Circ.
